# Supplementary material for: Effective pseudopotential for energy density functionals with higher order derivatives
Source: arXiv:1103.0682 ancillary file (2011-04-17)
Supplement: Supplementary file 1 [file Suppl_T_Section_III.tex.pdf]

**90 fourth-order (isoscalar and isovector) EDF coupling constants expressed by 15 fourth-order pseudopotential parameters.**

$$C^{2000,0}_{00,2000} = \frac{5}{64}C^{40}_{00,00} + \frac{5C^{40}_{00,20}}{64\sqrt{3}} + \frac{25}{192}C^{31}_{11,00} - \frac{5C^{31}_{11,20}}{64\sqrt{3}} + \frac{5}{64}C^{20}_{20,00} + \frac{5C^{20}_{20,20}}{64\sqrt{3}} + \frac{1}{32}\sqrt{5}C^{22}_{22,00} + \frac{1}{32}\sqrt{\frac{5}{3}}C^{22}_{22,20},$$

$$C^{2000,1}_{00,2000} = -\frac{5C^{40}_{00,00}}{64\sqrt{3}} + \frac{5}{64}C^{40}_{00,20} + \frac{5C^{31}_{11,00}}{64\sqrt{3}} - \frac{5}{64}C^{31}_{11,20} - \frac{5C^{20}_{20,00}}{64\sqrt{3}} + \frac{5}{64}C^{20}_{20,20} - \frac{1}{32}\sqrt{\frac{5}{3}}C^{22}_{22,00} + \frac{1}{32}\sqrt{5}C^{22}_{22,20},$$

$$C^{2011,0}_{00,2011} = -\frac{5C^{40}_{00,00}}{64\sqrt{3}} - \frac{25}{192}C^{40}_{00,20} + \frac{5C^{31}_{11,00}}{64\sqrt{3}} - \frac{5}{64}C^{31}_{11,20} - \frac{5C^{20}_{20,00}}{64\sqrt{3}} - \frac{25}{192}C^{20}_{20,20} - \frac{1}{32}\sqrt{\frac{5}{3}}C^{22}_{22,00} - \frac{5}{96}\sqrt{5}C^{22}_{22,20},$$

$$C^{2011,1}_{00,2011} = -\frac{5}{64}C^{40}_{00,00} - \frac{5C^{40}_{00,20}}{64\sqrt{3}} + \frac{5}{64}C^{31}_{11,00} + \frac{5C^{31}_{11,20}}{64\sqrt{3}} - \frac{5}{64}C^{20}_{20,00} - \frac{5C^{20}_{20,20}}{64\sqrt{3}} - \frac{1}{32}\sqrt{5}C^{22}_{22,00} - \frac{1}{32}\sqrt{\frac{5}{3}}C^{22}_{22,20},$$

$$C^{2202,0}_{00,2202} = \frac{1}{32}\sqrt{5}C^{40}_{00,00} + \frac{1}{32}\sqrt{\frac{5}{3}}C^{40}_{00,20} + \frac{5}{96}\sqrt{5}C^{31}_{11,00} - \frac{1}{32}\sqrt{\frac{5}{3}}C^{31}_{11,20} + \frac{1}{32}\sqrt{5}C^{20}_{20,00} + \frac{1}{32}\sqrt{\frac{5}{3}}C^{20}_{20,20} + \frac{1}{16}C^{22}_{22,00} + \frac{C^{22}_{22,20}}{16\sqrt{3}},$$

$$C^{2202,1}_{00,2202} = -\frac{1}{32}\sqrt{\frac{5}{3}}C^{40}_{00,00} + \frac{1}{32}\sqrt{5}C^{40}_{00,20} + \frac{1}{32}\sqrt{\frac{5}{3}}C^{31}_{11,00} - \frac{1}{32}\sqrt{5}C^{31}_{11,20} - \frac{1}{32}\sqrt{\frac{5}{3}}C^{20}_{20,00} + \frac{1}{32}\sqrt{5}C^{20}_{20,20} - \frac{C^{22}_{22,00}}{16\sqrt{3}} + \frac{1}{16}C^{22}_{22,20},$$

$$C^{2011,0}_{00,2211} = -\frac{7}{96}C^{42}_{00,22} - \frac{7}{32}C^{31}_{11,22} - \frac{3}{32}\sqrt{\frac{21}{5}}C^{33}_{11,22} - \frac{7}{96}C^{22}_{20,22} - \frac{1}{48}\sqrt{7}C^{22}_{22,22},$$

$$C^{2011,1}_{00,2211} = \frac{7C^{42}_{00,22}}{32\sqrt{3}} - \frac{7C^{31}_{11,22}}{32\sqrt{3}} - \frac{3}{32}\sqrt{\frac{7}{5}}C^{33}_{11,22} + \frac{7C^{22}_{20,22}}{32\sqrt{3}} + \frac{1}{16}\sqrt{\frac{7}{3}}C^{22}_{22,22},$$

$$C^{2211,0}_{00,2211} = -\frac{C^{40}_{00,00}}{32\sqrt{3}} - \frac{5}{96}C^{40}_{00,20} - \frac{7C^{42}_{00,22}}{192\sqrt{5}} + \frac{C^{31}_{11,00}}{32\sqrt{3}} - \frac{1}{32}C^{31}_{11,20} - \frac{7C^{31}_{11,22}}{64\sqrt{5}} - \frac{3}{320}\sqrt{21}C^{33}_{11,22} - \frac{C^{20}_{20,00}}{32\sqrt{3}} - \frac{5}{96}C^{20}_{20,20} - \frac{7C^{22}_{20,22}}{192\sqrt{5}} - \frac{C^{22}_{22,00}}{16\sqrt{15}} - \frac{1}{48}\sqrt{5}C^{22}_{22,20} - \frac{1}{96}\sqrt{\frac{7}{5}}C^{22}_{22,22},$$

$$C^{2211,1}_{00,2211} = -\frac{1}{32}C^{40}_{00,00} - \frac{C^{40}_{00,20}}{32\sqrt{3}} + \frac{7C^{42}_{00,22}}{64\sqrt{15}} + \frac{1}{32}C^{31}_{11,00} + \frac{C^{31}_{11,20}}{32\sqrt{3}} - \frac{7C^{31}_{11,22}}{64\sqrt{15}} - \frac{3}{320}\sqrt{7}C^{33}_{11,22} - \frac{1}{32}C^{20}_{20,00} - \frac{C^{20}_{20,20}}{32\sqrt{3}} + \frac{7C^{22}_{20,22}}{64\sqrt{15}} - \frac{C^{22}_{22,00}}{16\sqrt{5}} - \frac{C^{22}_{22,20}}{16\sqrt{15}} + \frac{1}{32}\sqrt{\frac{7}{15}}C^{22}_{22,22},$$

$$C^{2212,0}_{00,2212} = -\frac{1}{96}\sqrt{5}C^{40}_{00,00} - \frac{5}{96}\sqrt{\frac{5}{3}}C^{40}_{00,20} + \frac{7C^{42}_{00,22}}{192\sqrt{3}} + \frac{1}{96}\sqrt{5}C^{31}_{11,00} - \frac{1}{32}\sqrt{\frac{5}{3}}C^{31}_{11,20} + \frac{7C^{31}_{11,22}}{64\sqrt{3}} + \frac{3}{64}\sqrt{\frac{7}{5}}C^{33}_{11,22} - \frac{1}{96}\sqrt{5}C^{20}_{20,00} - \frac{5}{96}\sqrt{\frac{5}{3}}C^{20}_{20,20} + \frac{7C^{22}_{20,22}}{192\sqrt{3}} - \frac{1}{48}C^{22}_{22,00} - \frac{5C^{22}_{22,20}}{48\sqrt{3}} + \frac{1}{96}\sqrt{\frac{7}{3}}C^{22}_{22,22},$$

$$C^{2212,1}_{00,2212} = -\frac{1}{32}\sqrt{\frac{5}{3}}C^{40}_{00,00} - \frac{1}{96}\sqrt{5}C^{40}_{00,20} - \frac{7}{192}C^{42}_{00,22} + \frac{1}{32}\sqrt{\frac{5}{3}}C^{31}_{11,00} + \frac{1}{96}\sqrt{5}C^{31}_{11,20} + \frac{7}{192}C^{31}_{11,22} + \frac{1}{64}\sqrt{\frac{21}{5}}C^{33}_{11,22} - \frac{1}{32}\sqrt{\frac{5}{3}}C^{20}_{20,00} - \frac{1}{96}\sqrt{5}C^{20}_{20,20} - \frac{7}{192}C^{22}_{20,22} - \frac{C^{22}_{22,00}}{16\sqrt{3}} - \frac{1}{48}C^{22}_{22,20} - \frac{1}{96}\sqrt{7}C^{22}_{22,22},$$

$$C^{2213,0}_{00,2213} = -\frac{1}{96}\sqrt{7}C^{40}_{00,00} - \frac{5}{96}\sqrt{\frac{7}{3}}C^{40}_{00,20} - \frac{1}{96}\sqrt{\frac{7}{15}}C^{42}_{00,22} + \frac{1}{96}\sqrt{7}C^{31}_{11,00} - \frac{1}{32}\sqrt{\frac{7}{3}}C^{31}_{11,20} - \frac{1}{32}\sqrt{\frac{7}{15}}C^{31}_{11,22} - \frac{3}{160}C^{33}_{11,22} - \frac{1}{96}\sqrt{7}C^{20}_{20,00} - \frac{5}{96}\sqrt{\frac{7}{3}}C^{20}_{20,20} - \frac{1}{96}\sqrt{\frac{7}{15}}C^{22}_{20,22} - \frac{1}{48}\sqrt{\frac{7}{5}}C^{22}_{22,00} - \frac{1}{48}\sqrt{\frac{35}{3}}C^{22}_{22,20} - \frac{C^{22}_{22,22}}{48\sqrt{15}},$$

$C^{2213,1}_{00,2213} = -\frac{1}{32}\sqrt{\frac{7}{3}}C^{40}_{00,00} - \frac{1}{96}\sqrt{7}C^{40}_{00,20} + \frac{1}{96}\sqrt{\frac{7}{5}}C^{42}_{00,22} + \frac{1}{32}\sqrt{\frac{7}{3}}C^{31}_{11,00} + \frac{1}{96}\sqrt{7}C^{31}_{11,20} - \frac{1}{96}\sqrt{\frac{7}{5}}C^{31}_{11,22} - \frac{1}{160}\sqrt{3}C^{33}_{11,22} - \frac{1}{32}\sqrt{\frac{7}{3}}C^{20}_{20,00} - \frac{1}{96}\sqrt{7}C^{20}_{20,20} + \frac{1}{96}\sqrt{\frac{7}{5}}C^{22}_{20,22} - \frac{1}{16}\sqrt{\frac{7}{15}}C^{22}_{22,00} - \frac{1}{48}\sqrt{\frac{7}{5}}C^{22}_{22,20} + \frac{C^{22}_{22,22}}{48\sqrt{5}}$,

$C^{1101,0}_{00,3101} = -\frac{3}{16}C^{40}_{00,00} - \frac{1}{16}\sqrt{3}C^{40}_{00,20} - \frac{5}{16}C^{31}_{11,00} + \frac{1}{16}\sqrt{3}C^{31}_{11,20} - \frac{3}{16}C^{20}_{20,00} - \frac{1}{16}\sqrt{3}C^{20}_{20,20} - \frac{3C^{22}_{22,00}}{8\sqrt{5}} - \frac{1}{8}\sqrt{\frac{3}{5}}C^{22}_{22,20}$,

$C^{1101,1}_{00,3101} = \frac{1}{16}\sqrt{3}C^{40}_{00,00} - \frac{3}{16}C^{40}_{00,20} - \frac{1}{16}\sqrt{3}C^{31}_{11,00} + \frac{3}{16}C^{31}_{11,20} + \frac{1}{16}\sqrt{3}C^{20}_{20,00} - \frac{3}{16}C^{20}_{20,20} + \frac{1}{8}\sqrt{\frac{3}{5}}C^{22}_{22,00} - \frac{3C^{22}_{22,20}}{8\sqrt{5}}$,

$C^{1110,0}_{00,3110} = \frac{C^{40}_{00,00}}{16\sqrt{3}} + \frac{5}{48}C^{40}_{00,20} + \frac{7C^{42}_{00,22}}{48\sqrt{5}} - \frac{C^{31}_{11,00}}{16\sqrt{3}} + \frac{1}{16}C^{31}_{11,20} + \frac{7C^{31}_{11,22}}{16\sqrt{5}} + \frac{3}{80}\sqrt{21}C^{33}_{11,22} + \frac{C^{20}_{20,00}}{16\sqrt{3}} + \frac{5}{48}C^{20}_{20,20} + \frac{7C^{22}_{20,22}}{48\sqrt{5}} + \frac{C^{22}_{22,00}}{8\sqrt{15}} + \frac{1}{24}\sqrt{5}C^{22}_{22,20} + \frac{1}{24}\sqrt{\frac{7}{5}}C^{22}_{22,22}$,

$C^{1110,1}_{00,3110} = \frac{1}{16}C^{40}_{00,00} + \frac{C^{40}_{00,20}}{16\sqrt{3}} - \frac{7C^{42}_{00,22}}{16\sqrt{15}} - \frac{1}{16}C^{31}_{11,00} - \frac{C^{31}_{11,20}}{16\sqrt{3}} + \frac{7C^{31}_{11,22}}{16\sqrt{15}} + \frac{3}{80}\sqrt{7}C^{33}_{11,22} + \frac{1}{16}C^{20}_{20,00} + \frac{C^{20}_{20,20}}{16\sqrt{3}} - \frac{7C^{22}_{20,22}}{16\sqrt{15}} + \frac{C^{22}_{22,00}}{8\sqrt{5}} + \frac{C^{22}_{22,20}}{8\sqrt{15}} - \frac{1}{8}\sqrt{\frac{7}{15}}C^{22}_{22,22}$,

$C^{1111,0}_{00,3111} = \frac{1}{16}C^{40}_{00,00} + \frac{5C^{40}_{00,20}}{16\sqrt{3}} - \frac{7C^{42}_{00,22}}{32\sqrt{15}} - \frac{1}{16}C^{31}_{11,00} + \frac{1}{16}\sqrt{3}C^{31}_{11,20} - \frac{7}{32}\sqrt{\frac{3}{5}}C^{31}_{11,22} - \frac{9}{160}\sqrt{7}C^{33}_{11,22} + \frac{1}{16}C^{20}_{20,00} + \frac{5C^{20}_{20,20}}{16\sqrt{3}} - \frac{7C^{22}_{20,22}}{32\sqrt{15}} + \frac{C^{22}_{22,00}}{8\sqrt{5}} + \frac{1}{8}\sqrt{\frac{5}{3}}C^{22}_{22,20} - \frac{1}{16}\sqrt{\frac{7}{15}}C^{22}_{22,22}$,

$C^{1111,1}_{00,3111} = \frac{1}{16}\sqrt{3}C^{40}_{00,00} + \frac{1}{16}C^{40}_{00,20} + \frac{7C^{42}_{00,22}}{32\sqrt{5}} - \frac{1}{16}\sqrt{3}C^{31}_{11,00} - \frac{1}{16}C^{31}_{11,20} - \frac{7C^{31}_{11,22}}{32\sqrt{5}} - \frac{3}{160}\sqrt{21}C^{33}_{11,22} + \frac{1}{16}\sqrt{3}C^{20}_{20,00} + \frac{1}{16}C^{20}_{20,20} + \frac{7C^{22}_{20,22}}{32\sqrt{5}} + \frac{1}{8}\sqrt{\frac{3}{5}}C^{22}_{22,00} + \frac{C^{22}_{22,20}}{8\sqrt{5}} + \frac{1}{16}\sqrt{\frac{7}{5}}C^{22}_{22,22}$,

$C^{1112,0}_{00,3112} = \frac{1}{16}\sqrt{\frac{5}{3}}C^{40}_{00,00} + \frac{5}{48}\sqrt{5}C^{40}_{00,20} + \frac{7}{480}C^{42}_{00,22} - \frac{1}{16}\sqrt{\frac{5}{3}}C^{31}_{11,00} + \frac{1}{16}\sqrt{5}C^{31}_{11,20} + \frac{7}{160}C^{31}_{11,22} + \frac{3}{160}\sqrt{\frac{21}{5}}C^{33}_{11,22} + \frac{1}{16}\sqrt{\frac{5}{3}}C^{20}_{20,00} + \frac{5}{48}\sqrt{5}C^{20}_{20,20} + \frac{7}{480}C^{22}_{20,22} + \frac{C^{22}_{22,00}}{8\sqrt{3}} + \frac{5}{24}C^{22}_{22,20} + \frac{1}{240}\sqrt{7}C^{22}_{22,22}$,

$C^{1112,1}_{00,3112} = \frac{1}{16}\sqrt{5}C^{40}_{00,00} + \frac{1}{16}\sqrt{\frac{5}{3}}C^{40}_{00,20} - \frac{7C^{42}_{00,22}}{160\sqrt{3}} - \frac{1}{16}\sqrt{5}C^{31}_{11,00} - \frac{1}{16}\sqrt{\frac{5}{3}}C^{31}_{11,20} + \frac{7C^{31}_{11,22}}{160\sqrt{3}} + \frac{3}{160}\sqrt{\frac{7}{5}}C^{33}_{11,22} + \frac{1}{16}\sqrt{5}C^{20}_{20,00} + \frac{1}{16}\sqrt{\frac{5}{3}}C^{20}_{20,20} - \frac{7C^{22}_{20,22}}{160\sqrt{3}} + \frac{1}{8}C^{22}_{22,00} + \frac{C^{22}_{22,20}}{8\sqrt{3}} - \frac{1}{80}\sqrt{\frac{7}{3}}C^{22}_{22,22}$,

$C^{1112,0}_{00,3312} = \frac{1}{16}\sqrt{\frac{7}{15}}C^{42}_{00,22} + \frac{1}{16}\sqrt{\frac{21}{5}}C^{31}_{11,22} + \frac{9}{80}C^{33}_{11,22} + \frac{1}{16}\sqrt{\frac{7}{15}}C^{22}_{20,22} + \frac{C^{22}_{22,22}}{8\sqrt{15}}$,

$C^{1112,1}_{00,3312} = -\frac{1}{16}\sqrt{\frac{7}{5}}C^{42}_{00,22} + \frac{1}{16}\sqrt{\frac{7}{5}}C^{31}_{11,22} + \frac{3}{80}\sqrt{3}C^{33}_{11,22} - \frac{1}{16}\sqrt{\frac{7}{5}}C^{22}_{20,22} - \frac{C^{22}_{22,22}}{8\sqrt{5}}$,

$C^{0000,0}_{00,4000} = \frac{3}{64}C^{40}_{00,00} + \frac{1}{64}\sqrt{3}C^{40}_{00,20} + \frac{5}{64}C^{31}_{11,00} - \frac{1}{64}\sqrt{3}C^{31}_{11,20} + \frac{3}{64}C^{20}_{20,00} + \frac{1}{64}\sqrt{3}C^{20}_{20,20} + \frac{3C^{22}_{22,00}}{32\sqrt{5}} + \frac{1}{32}\sqrt{\frac{3}{5}}C^{22}_{22,20}$,

$C^{0000,1}_{00,4000} = -\frac{1}{64}\sqrt{3}C^{40}_{00,00} + \frac{3}{64}C^{40}_{00,20} + \frac{1}{64}\sqrt{3}C^{31}_{11,00} - \frac{3}{64}C^{31}_{11,20} - \frac{1}{64}\sqrt{3}C^{20}_{20,00} + \frac{3}{64}C^{20}_{20,20} - \frac{1}{32}\sqrt{\frac{3}{5}}C^{22}_{22,00} + \frac{3C^{22}_{22,20}}{32\sqrt{5}}$,

$C^{0011,0}_{00,4011} = -\frac{1}{64}\sqrt{3}C^{40}_{00,00} - \frac{5}{64}C^{40}_{00,20} + \frac{1}{64}\sqrt{3}C^{31}_{11,00} - \frac{3}{64}C^{31}_{11,20} - \frac{1}{64}\sqrt{3}C^{20}_{20,00} - \frac{5}{64}C^{20}_{20,20} - \frac{1}{32}\sqrt{\frac{3}{5}}C^{22}_{22,00} - \frac{1}{32}\sqrt{5}C^{22}_{22,20}$,

$C^{0011,1}_{00,4011} = -\frac{3}{64}C^{40}_{00,00} - \frac{1}{64}\sqrt{3}C^{40}_{00,20} + \frac{3}{64}C^{31}_{11,00} + \frac{1}{64}\sqrt{3}C^{31}_{11,20} - \frac{3}{64}C^{20}_{20,00} - \frac{1}{64}\sqrt{3}C^{20}_{20,20} -$

$\frac{3C^{22}_{22,00}}{32\sqrt{5}} - \frac{1}{32}\sqrt{\frac{3}{5}}C^{22}_{22,20},$

$C^{0011,0}_{00,4211} = -\frac{1}{32}C^{42}_{00,22} - \frac{3}{32}C^{31}_{11,22} - \frac{9}{32}\sqrt{\frac{3}{35}}C^{33}_{11,22} - \frac{1}{32}C^{22}_{20,22} - \frac{C^{22}_{22,22}}{16\sqrt{7}},$

$C^{0011,1}_{00,4211} = \frac{1}{32}\sqrt{3}C^{42}_{00,22} - \frac{1}{32}\sqrt{3}C^{31}_{11,22} - \frac{9C^{33}_{11,22}}{32\sqrt{35}} + \frac{1}{32}\sqrt{3}C^{22}_{20,22} + \frac{1}{16}\sqrt{\frac{3}{7}}C^{22}_{22,22},$

$C^{3101,0}_{11,0011} = -\frac{3}{16}C^{31}_{11,11} - \frac{1}{8}\sqrt{\frac{3}{5}}C^{22}_{22,11},$

$C^{3101,1}_{11,0011} = -\frac{1}{16}\sqrt{3}C^{31}_{11,11} + \frac{3C^{22}_{22,11}}{8\sqrt{5}},$

$C^{2000,0}_{11,1111} = -\frac{5}{16}C^{31}_{11,11} - \frac{1}{8}\sqrt{\frac{5}{3}}C^{22}_{22,11},$

$C^{2000,1}_{11,1111} = -\frac{5C^{31}_{11,11}}{16\sqrt{3}} + \frac{1}{8}\sqrt{5}C^{22}_{22,11},$

$C^{2202,0}_{11,1111} = \frac{1}{16}\sqrt{5}C^{31}_{11,11} + \frac{C^{22}_{22,11}}{8\sqrt{3}},$

$C^{2202,1}_{11,1111} = \frac{1}{16}\sqrt{\frac{5}{3}}C^{31}_{11,11} - \frac{1}{8}C^{22}_{22,11},$

$C^{2202,0}_{11,1112} = \frac{1}{16}\sqrt{15}C^{31}_{11,11} + \frac{1}{8}C^{22}_{22,11},$

$C^{2202,1}_{11,1112} = \frac{1}{16}\sqrt{5}C^{31}_{11,11} - \frac{1}{8}\sqrt{3}C^{22}_{22,11},$

$C^{1101,0}_{11,2011} = -\frac{5}{16}C^{31}_{11,11} - \frac{1}{8}\sqrt{\frac{5}{3}}C^{22}_{22,11},$

$C^{1101,1}_{11,2011} = -\frac{5C^{31}_{11,11}}{16\sqrt{3}} + \frac{1}{8}\sqrt{5}C^{22}_{22,11},$

$C^{1101,0}_{11,2211} = \frac{1}{16}\sqrt{5}C^{31}_{11,11} + \frac{C^{22}_{22,11}}{8\sqrt{3}},$

$C^{1101,1}_{11,2211} = \frac{1}{16}\sqrt{\frac{5}{3}}C^{31}_{11,11} - \frac{1}{8}C^{22}_{22,11},$

$C^{1101,0}_{11,2212} = \frac{1}{16}\sqrt{15}C^{31}_{11,11} + \frac{1}{8}C^{22}_{22,11},$

$C^{1101,1}_{11,2212} = \frac{1}{16}\sqrt{5}C^{31}_{11,11} - \frac{1}{8}\sqrt{3}C^{22}_{22,11},$

$C^{0000,0}_{11,3111} = -\frac{3}{16}C^{31}_{11,11} - \frac{1}{8}\sqrt{\frac{3}{5}}C^{22}_{22,11},$

$C^{0000,1}_{11,3111} = -\frac{1}{16}\sqrt{3}C^{31}_{11,11} + \frac{3C^{22}_{22,11}}{8\sqrt{5}},$

$C^{1101,0}_{20,1101} = \frac{5}{32}C^{40}_{00,00} + \frac{5C^{40}_{00,20}}{32\sqrt{3}} + \frac{1}{32}C^{20}_{20,00} + \frac{C^{20}_{20,20}}{32\sqrt{3}} - \frac{1}{16}\sqrt{5}C^{22}_{22,00} - \frac{1}{16}\sqrt{\frac{5}{3}}C^{22}_{22,20},$

$C^{1101,1}_{20,1101} = -\frac{5C^{40}_{00,00}}{32\sqrt{3}} + \frac{5}{32}C^{40}_{00,20} - \frac{C^{20}_{20,00}}{32\sqrt{3}} + \frac{1}{32}C^{20}_{20,20} + \frac{1}{16}\sqrt{\frac{5}{3}}C^{22}_{22,00} - \frac{1}{16}\sqrt{5}C^{22}_{22,20},$

$C^{1110,0}_{20,1110} = -\frac{5C^{40}_{00,00}}{96\sqrt{3}} - \frac{25}{288}C^{40}_{00,20} - \frac{7}{288}\sqrt{5}C^{42}_{00,22} - \frac{1}{32}\sqrt{5}C^{31}_{11,22} + \frac{1}{32}\sqrt{21}C^{33}_{11,22} -$
$\frac{C^{20}_{20,00}}{96\sqrt{3}} - \frac{5}{288}C^{20}_{20,20} + \frac{1}{288}\sqrt{5}C^{22}_{20,22} + \frac{1}{48}\sqrt{\frac{5}{3}}C^{22}_{22,00} + \frac{5}{144}\sqrt{5}C^{22}_{22,20} + \frac{1}{144}\sqrt{35}C^{22}_{22,22},$

$C^{1110,1}_{20,1110} = -\frac{5}{96}C^{40}_{00,00} - \frac{5C^{40}_{00,20}}{96\sqrt{3}} + \frac{7}{96}\sqrt{\frac{5}{3}}C^{42}_{00,22} - \frac{1}{32}\sqrt{\frac{5}{3}}C^{31}_{11,22} + \frac{1}{32}\sqrt{7}C^{33}_{11,22} -$
$\frac{1}{96}C^{20}_{20,00} - \frac{C^{20}_{20,20}}{96\sqrt{3}} - \frac{1}{96}\sqrt{\frac{5}{3}}C^{22}_{20,22} + \frac{1}{48}\sqrt{5}C^{22}_{22,00} + \frac{1}{48}\sqrt{\frac{5}{3}}C^{22}_{22,20} - \frac{1}{48}\sqrt{\frac{35}{3}}C^{22}_{22,22},$

$C^{1111,0}_{20,1111} = -\frac{5}{96}C^{40}_{00,00} - \frac{25C^{40}_{00,20}}{96\sqrt{3}} + \frac{7}{192}\sqrt{\frac{5}{3}}C^{42}_{00,22} + \frac{1}{64}\sqrt{15}C^{31}_{11,22} - \frac{3}{64}\sqrt{7}C^{33}_{11,22} -$
$\frac{1}{96}C^{20}_{20,00} - \frac{5C^{20}_{20,20}}{96\sqrt{3}} - \frac{1}{192}\sqrt{\frac{5}{3}}C^{22}_{20,22} + \frac{1}{48}\sqrt{5}C^{22}_{22,00} + \frac{5}{48}\sqrt{\frac{5}{3}}C^{22}_{22,20} - \frac{1}{96}\sqrt{\frac{35}{3}}C^{22}_{22,22},$

$C^{1111,1}_{20,1111} = -\frac{5C^{40}_{00,00}}{32\sqrt{3}} - \frac{5}{96}C^{40}_{00,20} - \frac{7}{192}\sqrt{5}C^{42}_{00,22} + \frac{1}{64}\sqrt{5}C^{31}_{11,22} - \frac{1}{64}\sqrt{21}C^{33}_{11,22} -$
$\frac{C^{20}_{20,00}}{32\sqrt{3}} - \frac{1}{96}C^{20}_{20,20} + \frac{1}{192}\sqrt{5}C^{22}_{20,22} + \frac{1}{16}\sqrt{\frac{5}{3}}C^{22}_{22,00} + \frac{1}{48}\sqrt{5}C^{22}_{22,20} + \frac{1}{96}\sqrt{35}C^{22}_{22,22},$

$C^{1112,0}_{20,1112} = -\frac{5}{96}\sqrt{\frac{5}{3}}C^{40}_{00,00} - \frac{25}{288}\sqrt{5}C^{40}_{00,20} - \frac{7}{576}C^{42}_{00,22} - \frac{1}{64}C^{31}_{11,22} + \frac{1}{64}\sqrt{\frac{21}{5}}C^{33}_{11,22} - \frac{1}{96}\sqrt{\frac{5}{3}}C^{20}_{20,00} - \frac{5}{288}\sqrt{5}C^{20}_{20,20} + \frac{1}{576}C^{22}_{20,22} + \frac{5C^{22}_{22,00}}{48\sqrt{3}} + \frac{25}{144}C^{22}_{22,20} + \frac{1}{288}\sqrt{7}C^{22}_{22,22}$,

$C^{1112,1}_{20,1112} = -\frac{5}{96}\sqrt{5}C^{40}_{00,00} - \frac{5}{96}\sqrt{\frac{5}{3}}C^{40}_{00,20} + \frac{7C^{42}_{00,22}}{192\sqrt{3}} - \frac{C^{31}_{11,22}}{64\sqrt{3}} + \frac{1}{64}\sqrt{\frac{7}{5}}C^{33}_{11,22} - \frac{1}{96}\sqrt{5}C^{20}_{20,00} - \frac{1}{96}\sqrt{\frac{5}{3}}C^{20}_{20,20} - \frac{C^{22}_{20,22}}{192\sqrt{3}} + \frac{5}{48}C^{22}_{22,00} + \frac{5C^{22}_{22,20}}{48\sqrt{3}} - \frac{1}{96}\sqrt{\frac{7}{3}}C^{22}_{22,22}$,

$C^{0000,0}_{20,2000} = -\frac{5}{32}C^{40}_{00,00} - \frac{5C^{40}_{00,20}}{32\sqrt{3}} - \frac{1}{32}C^{20}_{20,00} - \frac{C^{20}_{20,20}}{32\sqrt{3}} + \frac{1}{16}\sqrt{5}C^{22}_{22,00} + \frac{1}{16}\sqrt{\frac{5}{3}}C^{22}_{22,20}$,

$C^{0000,1}_{20,2000} = \frac{5C^{40}_{00,00}}{32\sqrt{3}} - \frac{5}{32}C^{40}_{00,20} + \frac{C^{20}_{20,00}}{32\sqrt{3}} - \frac{1}{32}C^{20}_{20,20} - \frac{1}{16}\sqrt{\frac{5}{3}}C^{22}_{22,00} + \frac{1}{16}\sqrt{5}C^{22}_{22,20}$,

$C^{0011,0}_{20,2011} = \frac{5C^{40}_{00,00}}{32\sqrt{3}} + \frac{25}{96}C^{40}_{00,20} + \frac{C^{20}_{20,00}}{32\sqrt{3}} + \frac{5}{96}C^{20}_{20,20} - \frac{1}{16}\sqrt{\frac{5}{3}}C^{22}_{22,00} - \frac{5}{48}\sqrt{5}C^{22}_{22,20}$,

$C^{0011,1}_{20,2011} = \frac{5}{32}C^{40}_{00,00} + \frac{5C^{40}_{00,20}}{32\sqrt{3}} + \frac{1}{32}C^{20}_{20,00} + \frac{C^{20}_{20,20}}{32\sqrt{3}} - \frac{1}{16}\sqrt{5}C^{22}_{22,00} - \frac{1}{16}\sqrt{\frac{5}{3}}C^{22}_{22,20}$,

$C^{0011,0}_{20,2211} = \frac{7}{96}C^{42}_{00,22} + \frac{3}{32}C^{31}_{11,22} - \frac{3}{32}\sqrt{\frac{21}{5}}C^{33}_{11,22} - \frac{1}{96}C^{22}_{20,22} - \frac{1}{48}\sqrt{7}C^{22}_{22,22}$,

$C^{0011,1}_{20,2211} = -\frac{7C^{42}_{00,22}}{32\sqrt{3}} + \frac{1}{32}\sqrt{3}C^{31}_{11,22} - \frac{3}{32}\sqrt{\frac{7}{5}}C^{33}_{11,22} + \frac{C^{22}_{20,22}}{32\sqrt{3}} + \frac{1}{16}\sqrt{\frac{7}{3}}C^{22}_{22,22}$,

$C^{1101,0}_{22,1101} = \frac{1}{16}\sqrt{5}C^{40}_{00,00} + \frac{1}{16}\sqrt{\frac{5}{3}}C^{40}_{00,20} - \frac{1}{16}\sqrt{5}C^{20}_{20,00} - \frac{1}{16}\sqrt{\frac{5}{3}}C^{20}_{20,20} + \frac{1}{16}C^{22}_{22,00} + \frac{C^{22}_{22,20}}{16\sqrt{3}}$,

$C^{1101,1}_{22,1101} = -\frac{1}{16}\sqrt{\frac{5}{3}}C^{40}_{00,00} + \frac{1}{16}\sqrt{5}C^{40}_{00,20} + \frac{1}{16}\sqrt{\frac{5}{3}}C^{20}_{20,00} - \frac{1}{16}\sqrt{5}C^{20}_{20,20} - \frac{C^{22}_{22,00}}{16\sqrt{3}} + \frac{1}{16}C^{22}_{22,20}$,

$C^{1111,0}_{22,1111} = \frac{1}{96}\sqrt{5}C^{40}_{00,00} + \frac{5}{96}\sqrt{\frac{5}{3}}C^{40}_{00,20} - \frac{7C^{42}_{00,22}}{192\sqrt{3}} - \frac{1}{64}\sqrt{3}C^{31}_{11,22} + \frac{3}{64}\sqrt{\frac{7}{5}}C^{33}_{11,22} - \frac{1}{96}\sqrt{5}C^{20}_{20,00} - \frac{5}{96}\sqrt{\frac{5}{3}}C^{20}_{20,20} + \frac{13C^{22}_{20,22}}{192\sqrt{3}} + \frac{1}{96}C^{22}_{22,00} + \frac{5C^{22}_{22,20}}{96\sqrt{3}} - \frac{5}{96}\sqrt{\frac{7}{3}}C^{22}_{22,22}$,

$C^{1111,1}_{22,1111} = \frac{1}{32}\sqrt{\frac{5}{3}}C^{40}_{00,00} + \frac{1}{96}\sqrt{5}C^{40}_{00,20} + \frac{7}{192}C^{42}_{00,22} - \frac{1}{64}C^{31}_{11,22} + \frac{1}{64}\sqrt{\frac{21}{5}}C^{33}_{11,22} - \frac{1}{32}\sqrt{\frac{5}{3}}C^{20}_{20,00} - \frac{1}{96}\sqrt{5}C^{20}_{20,20} - \frac{13}{192}C^{22}_{20,22} + \frac{C^{22}_{22,00}}{32\sqrt{3}} + \frac{1}{96}C^{22}_{22,20} + \frac{5}{96}\sqrt{7}C^{22}_{22,22}$,

$C^{1110,0}_{22,1112} = -\frac{1}{24}\sqrt{\frac{5}{3}}C^{40}_{00,00} - \frac{5}{72}\sqrt{5}C^{40}_{00,20} - \frac{7}{72}C^{42}_{00,22} + \frac{1}{16}C^{31}_{11,22} - \frac{1}{16}\sqrt{\frac{21}{5}}C^{33}_{11,22} + \frac{1}{24}\sqrt{\frac{5}{3}}C^{20}_{20,00} + \frac{5}{72}\sqrt{5}C^{20}_{20,20} + \frac{1}{18}C^{22}_{20,22} - \frac{C^{22}_{22,00}}{24\sqrt{3}} - \frac{5}{72}C^{22}_{22,20} - \frac{1}{72}\sqrt{7}C^{22}_{22,22}$,

$C^{1110,1}_{22,1112} = -\frac{1}{24}\sqrt{5}C^{40}_{00,00} - \frac{1}{24}\sqrt{\frac{5}{3}}C^{40}_{00,20} + \frac{7C^{42}_{00,22}}{24\sqrt{3}} + \frac{C^{31}_{11,22}}{16\sqrt{3}} - \frac{1}{16}\sqrt{\frac{7}{5}}C^{33}_{11,22} + \frac{1}{24}\sqrt{5}C^{20}_{20,00} + \frac{1}{24}\sqrt{\frac{5}{3}}C^{20}_{20,20} - \frac{C^{22}_{20,22}}{6\sqrt{3}} - \frac{1}{24}C^{22}_{22,00} - \frac{C^{22}_{22,20}}{24\sqrt{3}} + \frac{1}{24}\sqrt{\frac{7}{3}}C^{22}_{22,22}$,

$C^{1111,0}_{22,1112} = -\frac{1}{16}\sqrt{\frac{5}{3}}C^{40}_{00,00} - \frac{5}{48}\sqrt{5}C^{40}_{00,20} + \frac{7}{96}C^{42}_{00,22} - \frac{3}{32}C^{31}_{11,22} + \frac{3}{32}\sqrt{\frac{21}{5}}C^{33}_{11,22} + \frac{1}{16}\sqrt{\frac{5}{3}}C^{20}_{20,00} + \frac{5}{48}\sqrt{5}C^{20}_{20,20} - \frac{1}{96}C^{22}_{20,22} - \frac{C^{22}_{22,00}}{16\sqrt{3}} - \frac{5}{48}C^{22}_{22,20} - \frac{1}{48}\sqrt{7}C^{22}_{22,22}$,

$C^{1111,1}_{22,1112} = -\frac{1}{16}\sqrt{5}C^{40}_{00,00} - \frac{1}{16}\sqrt{\frac{5}{3}}C^{40}_{00,20} - \frac{7C^{42}_{00,22}}{32\sqrt{3}} - \frac{1}{32}\sqrt{3}C^{31}_{11,22} + \frac{3}{32}\sqrt{\frac{7}{5}}C^{33}_{11,22} + \frac{1}{16}\sqrt{5}C^{20}_{20,00} + \frac{1}{16}\sqrt{\frac{5}{3}}C^{20}_{20,20} + \frac{C^{22}_{20,22}}{32\sqrt{3}} - \frac{1}{16}C^{22}_{22,00} - \frac{C^{22}_{22,20}}{16\sqrt{3}} + \frac{1}{16}\sqrt{\frac{7}{3}}C^{22}_{22,22}$,

$C^{1112,0}_{22,1112} = -\frac{1}{96}\sqrt{\frac{35}{3}}C^{40}_{00,00} - \frac{5}{288}\sqrt{35}C^{40}_{00,20} - \frac{5}{576}\sqrt{7}C^{42}_{00,22} + \frac{1}{64}\sqrt{7}C^{31}_{11,22} - \frac{7}{64}\sqrt{\frac{3}{5}}C^{33}_{11,22} + \frac{1}{96}\sqrt{\frac{35}{3}}C^{20}_{20,00} + \frac{5}{288}\sqrt{35}C^{20}_{20,20} - \frac{1}{576}\sqrt{7}C^{22}_{20,22} - \frac{1}{96}\sqrt{\frac{7}{3}}C^{22}_{22,00} - \frac{5}{288}\sqrt{7}C^{22}_{22,20} + \frac{11}{288}C^{22}_{22,22}$,

$C_{22,1112}^{1112,1} = -\frac{1}{96}\sqrt{35}C_{00,00}^{40} - \frac{1}{96}\sqrt{\frac{35}{3}}C_{00,20}^{40} + \frac{5}{192}\sqrt{\frac{7}{3}}C_{00,22}^{42} + \frac{1}{64}\sqrt{\frac{7}{3}}C_{11,22}^{31} - \frac{7C_{11,22}^{33}}{64\sqrt{5}} + \frac{1}{96}\sqrt{35}C_{20,00}^{20} + \frac{1}{96}\sqrt{\frac{35}{3}}C_{20,20}^{20} + \frac{1}{192}\sqrt{\frac{7}{3}}C_{20,22}^{22} - \frac{1}{96}\sqrt{7}C_{22,00}^{22} - \frac{1}{96}\sqrt{\frac{7}{3}}C_{22,20}^{22} - \frac{11C_{22,22}^{22}}{96\sqrt{3}}$,

$C_{22,2011}^{0011,0} = \frac{7}{96}C_{00,22}^{42} - \frac{3}{32}C_{11,22}^{31} + \frac{3}{32}\sqrt{\frac{21}{5}}C_{11,22}^{33} - \frac{1}{96}C_{20,22}^{22} - \frac{1}{48}\sqrt{7}C_{22,22}^{22}$,

$C_{22,2011}^{0011,1} = -\frac{7C_{00,22}^{42}}{32\sqrt{3}} - \frac{1}{32}\sqrt{3}C_{11,22}^{31} + \frac{3}{32}\sqrt{\frac{7}{5}}C_{11,22}^{33} + \frac{C_{20,22}^{22}}{32\sqrt{3}} + \frac{1}{16}\sqrt{\frac{7}{3}}C_{22,22}^{22}$,

$C_{22,2202}^{0000,0} = -\frac{1}{16}\sqrt{5}C_{00,00}^{40} - \frac{1}{16}\sqrt{\frac{5}{3}}C_{00,20}^{40} + \frac{1}{16}\sqrt{5}C_{20,00}^{20} + \frac{1}{16}\sqrt{\frac{5}{3}}C_{20,20}^{20} - \frac{1}{16}C_{22,00}^{22} - \frac{C_{22,20}^{22}}{16\sqrt{3}}$,

$C_{22,2202}^{0000,1} = \frac{1}{16}\sqrt{\frac{5}{3}}C_{00,00}^{40} - \frac{1}{16}\sqrt{5}C_{00,20}^{40} - \frac{1}{16}\sqrt{\frac{5}{3}}C_{20,00}^{20} + \frac{1}{16}\sqrt{5}C_{20,20}^{20} + \frac{C_{22,00}^{22}}{16\sqrt{3}} - \frac{1}{16}C_{22,20}^{22}$,

$C_{22,2211}^{0011,0} = \frac{C_{00,00}^{40}}{16\sqrt{3}} + \frac{5}{48}C_{00,20}^{40} + \frac{7C_{00,22}^{42}}{96\sqrt{5}} - \frac{C_{20,00}^{20}}{16\sqrt{3}} - \frac{5}{48}C_{20,20}^{20} - \frac{7C_{20,22}^{22}}{96\sqrt{5}} + \frac{C_{22,00}^{22}}{16\sqrt{15}} + \frac{1}{48}\sqrt{5}C_{22,20}^{22} + \frac{1}{24}\sqrt{\frac{7}{5}}C_{22,22}^{22}$,

$C_{22,2211}^{0011,1} = \frac{1}{16}C_{00,00}^{40} + \frac{C_{00,20}^{40}}{16\sqrt{3}} - \frac{7C_{00,22}^{42}}{32\sqrt{15}} - \frac{1}{16}C_{20,00}^{20} - \frac{C_{20,20}^{20}}{16\sqrt{3}} + \frac{7C_{20,22}^{22}}{32\sqrt{15}} + \frac{C_{22,00}^{22}}{16\sqrt{5}} + \frac{C_{22,20}^{22}}{16\sqrt{15}} - \frac{1}{8}\sqrt{\frac{7}{15}}C_{22,22}^{22}$,

$C_{22,2212}^{0011,0} = -\frac{1}{48}\sqrt{5}C_{00,00}^{40} - \frac{5}{48}\sqrt{\frac{5}{3}}C_{00,20}^{40} + \frac{7C_{00,22}^{42}}{96\sqrt{3}} + \frac{1}{48}\sqrt{5}C_{20,00}^{20} + \frac{5}{48}\sqrt{\frac{5}{3}}C_{20,20}^{20} - \frac{7C_{20,22}^{22}}{96\sqrt{3}} - \frac{1}{48}C_{22,00}^{22} - \frac{5C_{22,20}^{22}}{48\sqrt{3}} + \frac{1}{24}\sqrt{\frac{7}{3}}C_{22,22}^{22}$,

$C_{22,2212}^{0011,1} = -\frac{1}{16}\sqrt{\frac{5}{3}}C_{00,00}^{40} - \frac{1}{48}\sqrt{5}C_{00,20}^{40} - \frac{7}{96}C_{00,22}^{42} + \frac{1}{16}\sqrt{\frac{5}{3}}C_{20,00}^{20} + \frac{1}{48}\sqrt{5}C_{20,20}^{20} + \frac{7}{96}C_{20,22}^{22} - \frac{C_{22,00}^{22}}{16\sqrt{3}} - \frac{1}{48}C_{22,20}^{22} - \frac{1}{24}\sqrt{7}C_{22,22}^{22}$,

$C_{22,2213}^{0011,0} = \frac{1}{48}\sqrt{7}C_{00,00}^{40} + \frac{5}{48}\sqrt{\frac{7}{3}}C_{00,20}^{40} + \frac{1}{48}\sqrt{\frac{7}{15}}C_{00,22}^{42} - \frac{1}{48}\sqrt{7}C_{20,00}^{20} - \frac{5}{48}\sqrt{\frac{7}{3}}C_{20,20}^{20} - \frac{1}{48}\sqrt{\frac{7}{15}}C_{20,22}^{22} + \frac{1}{48}\sqrt{\frac{7}{5}}C_{22,00}^{22} + \frac{1}{48}\sqrt{\frac{35}{3}}C_{22,20}^{22} + \frac{C_{22,22}^{22}}{12\sqrt{15}}$,

$C_{22,2213}^{0011,1} = \frac{1}{16}\sqrt{\frac{7}{3}}C_{00,00}^{40} + \frac{1}{48}\sqrt{7}C_{00,20}^{40} - \frac{1}{48}\sqrt{\frac{7}{5}}C_{00,22}^{42} - \frac{1}{16}\sqrt{\frac{7}{3}}C_{20,00}^{20} - \frac{1}{48}\sqrt{7}C_{20,20}^{20} + \frac{1}{48}\sqrt{\frac{7}{5}}C_{20,22}^{22} + \frac{1}{16}\sqrt{\frac{7}{15}}C_{22,00}^{22} + \frac{1}{48}\sqrt{\frac{7}{5}}C_{22,20}^{22} - \frac{C_{22,22}^{22}}{12\sqrt{5}}$,

$C_{31,0011}^{1101,0} = \frac{3}{16}C_{11,11}^{31} - \frac{1}{8}\sqrt{\frac{3}{5}}C_{22,11}^{22}$,

$C_{31,0011}^{1101,1} = \frac{1}{16}\sqrt{3}C_{11,11}^{31} + \frac{3C_{22,11}^{22}}{8\sqrt{5}}$,

$C_{31,1111}^{0000,0} = \frac{3}{16}C_{11,11}^{31} - \frac{1}{8}\sqrt{\frac{3}{5}}C_{22,11}^{22}$,

$C_{31,1111}^{0000,1} = \frac{1}{16}\sqrt{3}C_{11,11}^{31} + \frac{3C_{22,11}^{22}}{8\sqrt{5}}$,

$C_{40,0000}^{0000,0} = \frac{3}{128}C_{00,00}^{40} + \frac{1}{128}\sqrt{3}C_{00,20}^{40} - \frac{5}{128}C_{11,00}^{31} + \frac{1}{128}\sqrt{3}C_{11,20}^{31} + \frac{3}{128}C_{20,00}^{20} + \frac{1}{128}\sqrt{3}C_{20,20}^{20} + \frac{3C_{22,00}^{22}}{64\sqrt{5}} + \frac{1}{64}\sqrt{\frac{3}{5}}C_{22,20}^{22}$,

$C_{40,0000}^{0000,1} = -\frac{1}{128}\sqrt{3}C_{00,00}^{40} + \frac{3}{128}C_{00,20}^{40} - \frac{1}{128}\sqrt{3}C_{11,00}^{31} + \frac{3}{128}C_{11,20}^{31} - \frac{1}{128}\sqrt{3}C_{20,00}^{20} + \frac{3}{128}C_{20,20}^{20} - \frac{1}{64}\sqrt{\frac{3}{5}}C_{22,00}^{22} + \frac{3C_{22,20}^{22}}{64\sqrt{5}}$,

$C_{40,0011}^{0011,0} = -\frac{1}{128}\sqrt{3}C_{00,00}^{40} - \frac{5}{128}C_{00,20}^{40} - \frac{1}{128}\sqrt{3}C_{11,00}^{31} + \frac{3}{128}C_{11,20}^{31} - \frac{1}{128}\sqrt{3}C_{20,00}^{20} -$

$\frac{5}{128}C^{20}_{20,20} - \frac{1}{64}\sqrt{\frac{3}{5}}C^{22}_{22,00} - \frac{1}{64}\sqrt{5}C^{22}_{22,20}$,

$C^{0011,1}_{40,0011} = -\frac{3}{128}C^{40}_{00,00} - \frac{1}{128}\sqrt{3}C^{40}_{00,20} - \frac{3}{128}C^{31}_{11,00} - \frac{1}{128}\sqrt{3}C^{31}_{11,20} - \frac{3}{128}C^{20}_{20,00} - \frac{1}{128}\sqrt{3}C^{20}_{20,20} - \frac{3C^{22}_{22,00}}{64\sqrt{5}} - \frac{1}{64}\sqrt{\frac{3}{5}}C^{22}_{22,20}$,

$C^{0011,0}_{42,0011} = -\frac{1}{64}C^{42}_{00,22} + \frac{3}{64}C^{31}_{11,22} + \frac{9}{64}\sqrt{\frac{3}{35}}C^{33}_{11,22} - \frac{1}{64}C^{22}_{20,22} - \frac{C^{22}_{22,22}}{32\sqrt{7}}$,

$C^{0011,1}_{42,0011} = \frac{1}{64}\sqrt{3}C^{42}_{00,22} + \frac{1}{64}\sqrt{3}C^{31}_{11,22} + \frac{9C^{33}_{11,22}}{64\sqrt{35}} + \frac{1}{64}\sqrt{3}C^{22}_{20,22} + \frac{1}{32}\sqrt{\frac{3}{7}}C^{22}_{22,22}$,

**258 sixth-order (isoscalar and isovector) EDF coupling constants expressed by 26 sixth-order pseudopotential parameters.**

$C^{3101,0}_{00,3101} = -\frac{63}{640}C^{60}_{00,00} - \frac{21}{640}\sqrt{3}C^{60}_{00,20} - \frac{21}{128}C^{51}_{11,00} + \frac{21}{640}\sqrt{3}C^{51}_{11,20} - \frac{63}{640}C^{40}_{20,00} - \frac{21}{640}\sqrt{3}C^{40}_{20,20} - \frac{63C^{42}_{22,00}}{320\sqrt{5}} - \frac{21}{320}\sqrt{\frac{3}{5}}C^{42}_{22,20} - \frac{21}{128}C^{31}_{31,00} + \frac{21}{640}\sqrt{3}C^{31}_{31,20} - \frac{9}{320}\sqrt{21}C^{33}_{33,00} + \frac{27\sqrt{7}C^{33}_{33,20}}{1600}$,

$C^{3101,1}_{00,3101} = \frac{21}{640}\sqrt{3}C^{60}_{00,00} - \frac{63}{640}C^{60}_{00,20} - \frac{21}{640}\sqrt{3}C^{51}_{11,00} + \frac{63}{640}C^{51}_{11,20} + \frac{21}{640}\sqrt{3}C^{40}_{20,00} - \frac{63}{640}C^{40}_{20,20} + \frac{21}{320}\sqrt{\frac{3}{5}}C^{42}_{22,00} - \frac{63C^{42}_{22,20}}{320\sqrt{5}} - \frac{21}{640}\sqrt{3}C^{31}_{31,00} + \frac{63}{640}C^{31}_{31,20} - \frac{27\sqrt{7}C^{33}_{33,00}}{1600} + \frac{27\sqrt{21}C^{33}_{33,20}}{1600}$,

$C^{3110,0}_{00,3110} = \frac{7}{640}\sqrt{3}C^{60}_{00,00} + \frac{7}{128}C^{60}_{00,20} + \frac{21C^{62}_{00,22}}{320\sqrt{5}} - \frac{7}{640}\sqrt{3}C^{51}_{11,00} + \frac{21}{640}C^{51}_{11,20} + \frac{63C^{51}_{11,22}}{320\sqrt{5}} + \frac{27\sqrt{21}C^{53}_{11,22}}{1600} + \frac{7}{640}\sqrt{3}C^{40}_{20,00} + \frac{7}{128}C^{40}_{20,20} + \frac{21C^{42}_{20,22}}{320\sqrt{5}} + \frac{7}{320}\sqrt{\frac{3}{5}}C^{42}_{22,00} + \frac{7C^{42}_{22,20}}{64\sqrt{5}} + \frac{21C^{40}_{22,22}}{320\sqrt{5}} + \frac{3}{160}\sqrt{\frac{7}{5}}C^{42}_{22,22} + \frac{9}{400}C^{44}_{22,22} - \frac{7}{640}\sqrt{3}C^{31}_{31,00} + \frac{21}{640}C^{31}_{31,20} + \frac{63C^{31}_{31,22}}{320\sqrt{5}} + \frac{27\sqrt{21}C^{33}_{31,22}}{1600} - \frac{9\sqrt{7}C^{33}_{33,00}}{1600} + \frac{9\sqrt{21}C^{33}_{33,20}}{1600} + \frac{27}{400}\sqrt{\frac{7}{10}}C^{33}_{33,22}$,

$C^{3110,1}_{00,3110} = \frac{21}{640}C^{60}_{00,00} + \frac{7}{640}\sqrt{3}C^{60}_{00,20} - \frac{21}{320}\sqrt{\frac{3}{5}}C^{62}_{00,22} - \frac{21}{640}C^{51}_{11,00} - \frac{7}{640}\sqrt{3}C^{51}_{11,20} + \frac{21}{320}\sqrt{\frac{3}{5}}C^{51}_{11,22} + \frac{27\sqrt{7}C^{53}_{11,22}}{1600} + \frac{21}{640}C^{40}_{20,00} + \frac{7}{640}\sqrt{3}C^{40}_{20,20} - \frac{21}{320}\sqrt{\frac{3}{5}}C^{42}_{20,22} + \frac{21C^{42}_{22,00}}{320\sqrt{5}} + \frac{7}{320}\sqrt{\frac{3}{5}}C^{42}_{22,20} - \frac{21}{320}\sqrt{\frac{3}{5}}C^{40}_{22,22} - \frac{3}{160}\sqrt{\frac{21}{5}}C^{42}_{22,22} - \frac{9}{400}\sqrt{3}C^{44}_{22,22} - \frac{21}{640}C^{31}_{31,00} - \frac{7}{640}\sqrt{3}C^{31}_{31,20} + \frac{21}{320}\sqrt{\frac{3}{5}}C^{31}_{31,22} + \frac{27\sqrt{7}C^{33}_{31,22}}{1600} - \frac{9\sqrt{21}C^{33}_{33,00}}{1600} - \frac{9\sqrt{7}C^{33}_{33,20}}{1600} + \frac{9}{400}\sqrt{\frac{21}{10}}C^{33}_{33,22}$,

$C^{3111,0}_{00,3111} = \frac{21}{640}C^{60}_{00,00} + \frac{7}{128}\sqrt{3}C^{60}_{00,20} - \frac{21}{640}\sqrt{\frac{3}{5}}C^{62}_{00,22} - \frac{21}{640}C^{51}_{11,00} + \frac{21}{640}\sqrt{3}C^{51}_{11,20} - \frac{63}{640}\sqrt{\frac{3}{5}}C^{51}_{11,22} - \frac{81\sqrt{7}C^{53}_{11,22}}{3200} + \frac{21}{640}C^{40}_{20,00} + \frac{7}{128}\sqrt{3}C^{40}_{20,20} - \frac{21}{640}\sqrt{\frac{3}{5}}C^{42}_{20,22} + \frac{21C^{42}_{22,00}}{320\sqrt{5}} + \frac{7}{64}\sqrt{\frac{3}{5}}C^{42}_{22,20} - \frac{21}{640}\sqrt{\frac{3}{5}}C^{40}_{22,22} - \frac{3}{320}\sqrt{\frac{21}{5}}C^{42}_{22,22} - \frac{9}{800}\sqrt{3}C^{44}_{22,22} - \frac{21}{640}C^{31}_{31,00} + \frac{21}{640}\sqrt{3}C^{31}_{31,20} - \frac{63}{640}\sqrt{\frac{3}{5}}C^{31}_{31,22} - \frac{81\sqrt{7}C^{33}_{31,22}}{3200} - \frac{9\sqrt{21}C^{33}_{33,00}}{1600} + \frac{27\sqrt{7}C^{33}_{33,20}}{1600} - \frac{27}{800}\sqrt{\frac{21}{10}}C^{33}_{33,22}$,

$C^{3111,1}_{00,3111} = \frac{21}{640}\sqrt{3}C^{60}_{00,00} + \frac{21}{640}C^{60}_{00,20} + \frac{63C^{62}_{00,22}}{640\sqrt{5}} - \frac{21}{640}\sqrt{3}C^{51}_{11,00} - \frac{21}{640}C^{51}_{11,20} - \frac{63C^{51}_{11,22}}{640\sqrt{5}} - \frac{27\sqrt{21}C^{53}_{11,22}}{3200} + \frac{21}{640}\sqrt{3}C^{40}_{20,00} + \frac{21}{640}C^{40}_{20,20} + \frac{63C^{42}_{20,22}}{640\sqrt{5}} + \frac{21}{320}\sqrt{\frac{3}{5}}C^{42}_{22,00} + \frac{21C^{42}_{22,20}}{320\sqrt{5}} + \frac{63C^{40}_{22,22}}{640\sqrt{5}} + \frac{9}{320}\sqrt{\frac{7}{5}}C^{42}_{22,22} + \frac{27}{800}C^{44}_{22,22} - \frac{21}{640}\sqrt{3}C^{31}_{31,00} - \frac{21}{640}C^{31}_{31,20} - \frac{63C^{31}_{31,22}}{640\sqrt{5}} - \frac{27\sqrt{21}C^{33}_{31,22}}{3200} - \frac{27\sqrt{7}C^{33}_{33,00}}{1600} - \frac{9\sqrt{21}C^{33}_{33,20}}{1600} - \frac{27}{800}\sqrt{\frac{7}{10}}C^{33}_{33,22}$,

$$C^{3112,0}_{00,3112} = \frac{7}{128}\sqrt{\frac{3}{5}}C^{60}_{00,00} + \frac{7}{128}\sqrt{5}C^{60}_{00,20} + \frac{21C^{62}_{00,22}}{3200} - \frac{7}{128}\sqrt{\frac{3}{5}}C^{51}_{11,00} + \frac{21C^{51}_{11,20}}{128\sqrt{5}} + \frac{63C^{51}_{11,22}}{3200} + \frac{27\sqrt{\frac{21}{5}}C^{53}_{11,22}}{3200} + \frac{7}{128}\sqrt{\frac{3}{5}}C^{40}_{20,00} + \frac{7}{128}\sqrt{5}C^{40}_{20,20} + \frac{21C^{42}_{20,22}}{3200} + \frac{7}{320}\sqrt{3}C^{42}_{22,00} + \frac{7}{64}C^{42}_{22,20} + \frac{21C^{40}_{22,22}}{3200} + \frac{3\sqrt{7}C^{42}_{22,22}}{1600} + \frac{9C^{44}_{22,22}}{800\sqrt{5}} - \frac{7}{128}\sqrt{\frac{3}{5}}C^{31}_{31,00} + \frac{21C^{31}_{31,20}}{128\sqrt{5}} + \frac{63C^{31}_{31,22}}{3200} + \frac{27\sqrt{\frac{21}{5}}C^{33}_{31,22}}{3200} - \frac{9}{320}\sqrt{\frac{7}{5}}C^{33}_{33,00} + \frac{9}{320}\sqrt{\frac{21}{5}}C^{33}_{33,20} + \frac{27\sqrt{\frac{7}{2}}C^{33}_{33,22}}{4000},$$

$$C^{3112,1}_{00,3112} = \frac{21C^{60}_{00,00}}{128\sqrt{5}} + \frac{7}{128}\sqrt{\frac{3}{5}}C^{60}_{00,20} - \frac{21\sqrt{3}C^{62}_{00,22}}{3200} - \frac{21C^{51}_{11,00}}{128\sqrt{5}} - \frac{7}{128}\sqrt{\frac{3}{5}}C^{51}_{11,20} + \frac{21\sqrt{3}C^{51}_{11,22}}{3200} + \frac{27\sqrt{\frac{7}{5}}C^{53}_{11,22}}{3200} + \frac{21C^{40}_{20,00}}{128\sqrt{5}} + \frac{7}{128}\sqrt{\frac{3}{5}}C^{40}_{20,20} - \frac{21\sqrt{3}C^{42}_{20,22}}{3200} + \frac{21}{320}C^{42}_{22,00} + \frac{7}{320}\sqrt{3}C^{42}_{22,20} - \frac{21\sqrt{3}C^{40}_{22,22}}{3200} - \frac{3\sqrt{21}C^{42}_{22,22}}{1600} - \frac{9}{800}\sqrt{\frac{3}{5}}C^{44}_{22,22} - \frac{21C^{31}_{31,00}}{128\sqrt{5}} - \frac{7}{128}\sqrt{\frac{3}{5}}C^{31}_{31,20} + \frac{21\sqrt{3}C^{31}_{31,22}}{3200} + \frac{27\sqrt{\frac{7}{5}}C^{33}_{31,22}}{3200} - \frac{9}{320}\sqrt{\frac{21}{5}}C^{33}_{33,00} - \frac{9}{320}\sqrt{\frac{7}{5}}C^{33}_{33,20} + \frac{9\sqrt{\frac{21}{2}}C^{33}_{33,22}}{4000},$$

$$C^{3303,0}_{00,3303} = -\frac{1}{64}\sqrt{\frac{7}{3}}C^{60}_{00,00} - \frac{1}{192}\sqrt{7}C^{60}_{00,20} - \frac{5}{192}\sqrt{\frac{7}{3}}C^{51}_{11,00} + \frac{1}{192}\sqrt{7}C^{51}_{11,20} - \frac{1}{64}\sqrt{\frac{7}{3}}C^{40}_{20,00} - \frac{1}{192}\sqrt{7}C^{40}_{20,20} - \frac{1}{32}\sqrt{\frac{7}{15}}C^{42}_{22,00} - \frac{1}{96}\sqrt{\frac{7}{5}}C^{42}_{22,20} - \frac{5}{192}\sqrt{\frac{7}{3}}C^{31}_{31,00} + \frac{1}{192}\sqrt{7}C^{31}_{31,20} - \frac{1}{32}C^{33}_{33,00} + \frac{1}{160}\sqrt{3}C^{33}_{33,20},$$

$$C^{3303,1}_{00,3303} = \frac{1}{192}\sqrt{7}C^{60}_{00,00} - \frac{1}{64}\sqrt{\frac{7}{3}}C^{60}_{00,20} - \frac{1}{192}\sqrt{7}C^{51}_{11,00} + \frac{1}{64}\sqrt{\frac{7}{3}}C^{51}_{11,20} + \frac{1}{192}\sqrt{7}C^{40}_{20,00} - \frac{1}{64}\sqrt{\frac{7}{3}}C^{40}_{20,20} + \frac{1}{96}\sqrt{\frac{7}{5}}C^{42}_{22,00} - \frac{1}{32}\sqrt{\frac{7}{15}}C^{42}_{22,20} - \frac{1}{192}\sqrt{7}C^{31}_{31,00} + \frac{1}{64}\sqrt{\frac{7}{3}}C^{31}_{31,20} - \frac{1}{160}\sqrt{3}C^{33}_{33,00} + \frac{3}{160}C^{33}_{33,20},$$

$$C^{3112,0}_{00,3312} = \frac{3}{160}\sqrt{\frac{21}{5}}C^{62}_{00,22} + \frac{9}{160}\sqrt{\frac{21}{5}}C^{51}_{11,22} + \frac{81}{800}C^{53}_{11,22} + \frac{3}{160}\sqrt{\frac{21}{5}}C^{42}_{20,22} + \frac{3}{160}\sqrt{\frac{21}{5}}C^{40}_{22,22} + \frac{3}{80}\sqrt{\frac{3}{5}}C^{42}_{22,22} + \frac{9}{200}\sqrt{\frac{3}{7}}C^{44}_{22,22} + \frac{9}{160}\sqrt{\frac{21}{5}}C^{31}_{31,22} + \frac{81}{800}C^{33}_{31,22} + \frac{27}{200}\sqrt{\frac{3}{10}}C^{33}_{33,22},$$

$$C^{3112,1}_{00,3312} = -\frac{9}{160}\sqrt{\frac{7}{5}}C^{62}_{00,22} + \frac{9}{160}\sqrt{\frac{7}{5}}C^{51}_{11,22} + \frac{27}{800}\sqrt{3}C^{53}_{11,22} - \frac{9}{160}\sqrt{\frac{7}{5}}C^{42}_{20,22} - \frac{9}{160}\sqrt{\frac{7}{5}}C^{40}_{22,22} - \frac{9C^{42}_{22,22}}{80\sqrt{5}} - \frac{27C^{44}_{22,22}}{200\sqrt{7}} + \frac{9}{160}\sqrt{\frac{7}{5}}C^{31}_{31,22} + \frac{27}{800}\sqrt{3}C^{33}_{31,22} + \frac{27C^{33}_{33,22}}{200\sqrt{10}},$$

$$C^{3312,0}_{00,3312} = \frac{1}{192}\sqrt{\frac{5}{3}}C^{60}_{00,00} + \frac{5}{576}\sqrt{5}C^{60}_{00,20} + \frac{1}{240}C^{62}_{00,22} - \frac{1}{192}\sqrt{\frac{5}{3}}C^{51}_{11,00} + \frac{1}{192}\sqrt{5}C^{51}_{11,20} + \frac{1}{80}C^{51}_{11,22} + \frac{3}{80}\sqrt{\frac{3}{35}}C^{53}_{11,22} + \frac{1}{192}\sqrt{\frac{5}{3}}C^{40}_{20,00} + \frac{5}{576}\sqrt{5}C^{40}_{20,20} + \frac{1}{240}C^{42}_{20,22} + \frac{C^{42}_{22,00}}{96\sqrt{3}} + \frac{5}{288}C^{42}_{22,20} + \frac{1}{240}C^{40}_{22,22} + \frac{C^{42}_{22,22}}{120\sqrt{7}} + \frac{C^{44}_{22,22}}{140\sqrt{5}} - \frac{1}{192}\sqrt{\frac{5}{3}}C^{31}_{31,00} + \frac{1}{192}\sqrt{5}C^{31}_{31,20} + \frac{1}{80}C^{31}_{31,22} + \frac{3}{80}\sqrt{\frac{3}{35}}C^{33}_{31,22} - \frac{C^{33}_{33,00}}{32\sqrt{35}} + \frac{1}{32}\sqrt{\frac{3}{35}}C^{33}_{33,20} + \frac{3C^{33}_{33,22}}{100\sqrt{14}},$$

$$C^{3312,1}_{00,3312} = \frac{1}{192}\sqrt{5}C^{60}_{00,00} + \frac{1}{192}\sqrt{\frac{5}{3}}C^{60}_{00,20} - \frac{C^{62}_{00,22}}{80\sqrt{3}} - \frac{1}{192}\sqrt{5}C^{51}_{11,00} - \frac{1}{192}\sqrt{\frac{5}{3}}C^{51}_{11,20} + \frac{C^{51}_{11,22}}{80\sqrt{3}} + \frac{3C^{53}_{11,22}}{80\sqrt{35}} + \frac{1}{192}\sqrt{5}C^{40}_{20,00} + \frac{1}{192}\sqrt{\frac{5}{3}}C^{40}_{20,20} - \frac{C^{42}_{20,22}}{80\sqrt{3}} + \frac{1}{96}C^{42}_{22,00} + \frac{C^{42}_{22,20}}{96\sqrt{3}} - \frac{C^{40}_{22,22}}{80\sqrt{3}} - \frac{C^{42}_{22,22}}{40\sqrt{21}} - \frac{1}{140}\sqrt{\frac{3}{5}}C^{44}_{22,22} - \frac{1}{192}\sqrt{5}C^{31}_{31,00} - \frac{1}{192}\sqrt{\frac{5}{3}}C^{31}_{31,20} + \frac{C^{31}_{31,22}}{80\sqrt{3}} + \frac{3C^{33}_{31,22}}{80\sqrt{35}} - \frac{1}{32}\sqrt{\frac{3}{35}}C^{33}_{33,00} - \frac{C^{33}_{33,20}}{32\sqrt{35}} + \frac{1}{100}\sqrt{\frac{3}{14}}C^{33}_{33,22},$$

$$C^{3313,0}_{00,3313} = \frac{1}{192}\sqrt{\frac{7}{3}}C^{60}_{00,00} + \frac{5}{576}\sqrt{7}C^{60}_{00,20} - \frac{1}{192}\sqrt{\frac{7}{5}}C^{62}_{00,22} - \frac{1}{192}\sqrt{\frac{7}{3}}C^{51}_{11,00} + \frac{1}{192}\sqrt{7}C^{51}_{11,20} - \frac{1}{64}\sqrt{\frac{7}{5}}C^{51}_{11,22} - \frac{3}{320}\sqrt{3}C^{53}_{11,22} + \frac{1}{192}\sqrt{\frac{7}{3}}C^{40}_{20,00} + \frac{5}{576}\sqrt{7}C^{40}_{20,20} - \frac{1}{192}\sqrt{\frac{7}{5}}C^{42}_{20,22} + \frac{1}{96}\sqrt{\frac{7}{15}}C^{42}_{22,00} +$$

$$\tfrac{1}{288}\sqrt{35}C^{42}_{22,20} - \tfrac{1}{192}\sqrt{\tfrac{7}{5}}C^{40}_{22,22} - \frac{C^{42}_{22,22}}{96\sqrt{5}} - \frac{C^{44}_{22,22}}{80\sqrt{7}} - \tfrac{1}{192}\sqrt{\tfrac{7}{3}}C^{31}_{31,00} + \tfrac{1}{192}\sqrt{7}C^{31}_{31,20} - \tfrac{1}{64}\sqrt{\tfrac{7}{5}}C^{31}_{31,22} - \tfrac{3}{320}\sqrt{3}C^{33}_{31,22} - \tfrac{1}{160}C^{33}_{33,00} + \tfrac{1}{160}\sqrt{3}C^{33}_{33,20} - \frac{3C^{33}_{33,22}}{80\sqrt{10}},$$

$$C^{3313,1}_{00,3313} = \tfrac{1}{192}\sqrt{7}C^{60}_{00,00} + \tfrac{1}{192}\sqrt{\tfrac{7}{3}}C^{60}_{00,20} + \tfrac{1}{64}\sqrt{\tfrac{7}{15}}C^{62}_{00,22} - \tfrac{1}{192}\sqrt{7}C^{51}_{11,00} - \tfrac{1}{192}\sqrt{\tfrac{7}{3}}C^{51}_{11,20} - \tfrac{1}{64}\sqrt{\tfrac{7}{15}}C^{51}_{11,22} - \tfrac{3}{320}C^{53}_{11,22} + \tfrac{1}{192}\sqrt{7}C^{40}_{20,00} + \tfrac{1}{192}\sqrt{\tfrac{7}{3}}C^{40}_{20,20} + \tfrac{1}{64}\sqrt{\tfrac{7}{15}}C^{42}_{20,22} + \tfrac{1}{96}\sqrt{\tfrac{7}{5}}C^{42}_{22,00} + \tfrac{1}{96}\sqrt{\tfrac{7}{15}}C^{42}_{22,20} + \tfrac{1}{64}\sqrt{\tfrac{7}{15}}C^{40}_{22,22} + \frac{C^{42}_{22,22}}{32\sqrt{15}} + \tfrac{1}{80}\sqrt{\tfrac{3}{7}}C^{44}_{22,22} - \tfrac{1}{192}\sqrt{7}C^{31}_{31,00} - \tfrac{1}{192}\sqrt{\tfrac{7}{3}}C^{31}_{31,20} - \tfrac{1}{64}\sqrt{\tfrac{7}{15}}C^{31}_{31,22} - \tfrac{3}{320}C^{33}_{31,22} - \tfrac{1}{160}\sqrt{3}C^{33}_{33,00} - \tfrac{1}{160}C^{33}_{33,20} - \tfrac{1}{80}\sqrt{\tfrac{3}{10}}C^{33}_{33,22},$$

$$C^{3314,0}_{00,3314} = \frac{C^{60}_{00,00}}{64\sqrt{3}} + \tfrac{5}{192}C^{60}_{00,20} + \frac{C^{62}_{00,22}}{192\sqrt{5}} - \frac{C^{51}_{11,00}}{64\sqrt{3}} + \tfrac{1}{64}C^{51}_{11,20} + \frac{C^{51}_{11,22}}{64\sqrt{5}} + \tfrac{3}{320}\sqrt{\tfrac{3}{7}}C^{53}_{11,22} + \frac{C^{40}_{20,00}}{64\sqrt{3}} + \tfrac{5}{192}C^{40}_{20,20} + \frac{C^{42}_{20,22}}{192\sqrt{5}} + \frac{C^{42}_{22,00}}{32\sqrt{15}} + \tfrac{1}{96}\sqrt{5}C^{42}_{22,20} + \frac{C^{40}_{22,22}}{192\sqrt{5}} + \frac{C^{42}_{22,22}}{96\sqrt{35}} + \tfrac{1}{560}C^{44}_{22,22} - \frac{C^{31}_{31,00}}{64\sqrt{3}} + \tfrac{1}{64}C^{31}_{31,20} + \frac{C^{31}_{31,22}}{64\sqrt{5}} + \tfrac{3}{320}\sqrt{\tfrac{3}{7}}C^{33}_{31,22} - \frac{3C^{33}_{33,00}}{160\sqrt{7}} + \tfrac{3}{160}\sqrt{\tfrac{3}{7}}C^{33}_{33,20} + \frac{3C^{33}_{33,22}}{80\sqrt{70}},$$

$$C^{3314,1}_{00,3314} = \tfrac{1}{64}C^{60}_{00,00} + \frac{C^{60}_{00,20}}{64\sqrt{3}} - \frac{C^{62}_{00,22}}{64\sqrt{15}} - \tfrac{1}{64}C^{51}_{11,00} - \frac{C^{51}_{11,20}}{64\sqrt{3}} + \frac{C^{51}_{11,22}}{64\sqrt{15}} + \frac{3C^{53}_{11,22}}{320\sqrt{7}} + \tfrac{1}{64}C^{40}_{20,00} + \frac{C^{40}_{20,20}}{64\sqrt{3}} - \frac{C^{42}_{20,22}}{64\sqrt{15}} + \frac{C^{42}_{22,00}}{32\sqrt{5}} + \frac{C^{42}_{22,20}}{32\sqrt{15}} - \frac{C^{40}_{22,22}}{64\sqrt{15}} - \frac{C^{42}_{22,22}}{32\sqrt{105}} - \tfrac{1}{560}\sqrt{3}C^{44}_{22,22} - \tfrac{1}{64}C^{31}_{31,00} - \frac{C^{31}_{31,20}}{64\sqrt{3}} + \frac{C^{31}_{31,22}}{64\sqrt{15}} + \frac{3C^{33}_{31,22}}{320\sqrt{7}} - \tfrac{3}{160}\sqrt{\tfrac{3}{7}}C^{33}_{33,00} - \frac{3C^{33}_{33,20}}{160\sqrt{7}} + \tfrac{1}{80}\sqrt{\tfrac{3}{70}}C^{33}_{33,22},$$

$$C^{2000,0}_{00,4000} = \tfrac{21}{256}C^{60}_{00,00} + \tfrac{7}{256}\sqrt{3}C^{60}_{00,20} + \tfrac{35}{256}C^{51}_{11,00} - \tfrac{7}{256}\sqrt{3}C^{51}_{11,20} + \tfrac{21}{256}C^{40}_{20,00} + \tfrac{7}{256}\sqrt{3}C^{40}_{20,20} + \frac{21C^{42}_{22,00}}{128\sqrt{5}} + \tfrac{7}{128}\sqrt{\tfrac{3}{5}}C^{42}_{22,20} + \tfrac{35}{256}C^{31}_{31,00} - \tfrac{7}{256}\sqrt{3}C^{31}_{31,20} + \tfrac{3}{128}\sqrt{21}C^{33}_{33,00} - \tfrac{9}{640}\sqrt{7}C^{33}_{33,20},$$

$$C^{2000,1}_{00,4000} = -\tfrac{7}{256}\sqrt{3}C^{60}_{00,00} + \tfrac{21}{256}C^{60}_{00,20} + \tfrac{7}{256}\sqrt{3}C^{51}_{11,00} - \tfrac{21}{256}C^{51}_{11,20} - \tfrac{7}{256}\sqrt{3}C^{40}_{20,00} + \tfrac{21}{256}C^{40}_{20,20} - \tfrac{7}{128}\sqrt{\tfrac{3}{5}}C^{42}_{22,00} + \frac{21C^{42}_{22,20}}{128\sqrt{5}} + \tfrac{7}{256}\sqrt{3}C^{31}_{31,00} - \tfrac{21}{256}C^{31}_{31,20} + \tfrac{9}{640}\sqrt{7}C^{33}_{33,00} - \tfrac{9}{640}\sqrt{21}C^{33}_{33,20},$$

$$C^{2011,0}_{00,4011} = -\tfrac{7}{256}\sqrt{3}C^{60}_{00,00} - \tfrac{35}{256}C^{60}_{00,20} + \tfrac{7}{256}\sqrt{3}C^{51}_{11,00} - \tfrac{21}{256}C^{51}_{11,20} - \tfrac{7}{256}\sqrt{3}C^{40}_{20,00} - \tfrac{35}{256}C^{40}_{20,20} - \tfrac{7}{128}\sqrt{\tfrac{3}{5}}C^{42}_{22,00} - \tfrac{7}{128}\sqrt{5}C^{42}_{22,20} + \tfrac{7}{256}\sqrt{3}C^{31}_{31,00} - \tfrac{21}{256}C^{31}_{31,20} + \tfrac{9}{640}\sqrt{7}C^{33}_{33,00} - \tfrac{9}{640}\sqrt{21}C^{33}_{33,20},$$

$$C^{2011,1}_{00,4011} = -\tfrac{21}{256}C^{60}_{00,00} - \tfrac{7}{256}\sqrt{3}C^{60}_{00,20} + \tfrac{21}{256}C^{51}_{11,00} + \tfrac{7}{256}\sqrt{3}C^{51}_{11,20} - \tfrac{21}{256}C^{40}_{20,00} - \tfrac{7}{256}\sqrt{3}C^{40}_{20,20} - \frac{21C^{42}_{22,00}}{128\sqrt{5}} - \tfrac{7}{128}\sqrt{\tfrac{3}{5}}C^{42}_{22,20} + \tfrac{21}{256}C^{31}_{31,00} + \tfrac{7}{256}\sqrt{3}C^{31}_{31,20} + \tfrac{9}{640}\sqrt{21}C^{33}_{33,00} + \tfrac{9}{640}\sqrt{7}C^{33}_{33,20},$$

$$C^{2211,0}_{00,4011} = -\tfrac{21}{640}C^{62}_{00,22} - \tfrac{63}{640}C^{51}_{11,22} - \tfrac{27}{640}\sqrt{\tfrac{21}{5}}C^{53}_{11,22} - \tfrac{21}{640}C^{42}_{20,22} - \tfrac{21}{640}C^{40}_{22,22} - \tfrac{3}{320}\sqrt{7}C^{42}_{22,22} - \frac{9C^{44}_{22,22}}{160\sqrt{5}} - \tfrac{63}{640}C^{31}_{31,22} - \tfrac{27}{640}\sqrt{\tfrac{21}{5}}C^{33}_{31,22} - \tfrac{27}{800}\sqrt{\tfrac{7}{2}}C^{33}_{33,22},$$

$$C^{2211,1}_{00,4011} = \tfrac{21}{640}\sqrt{3}C^{62}_{00,22} - \tfrac{21}{640}\sqrt{3}C^{51}_{11,22} - \tfrac{27}{640}\sqrt{\tfrac{7}{5}}C^{53}_{11,22} + \tfrac{21}{640}\sqrt{3}C^{42}_{20,22} + \tfrac{21}{640}\sqrt{3}C^{40}_{22,22} + \tfrac{3}{320}\sqrt{21}C^{42}_{22,22} + \tfrac{9}{160}\sqrt{\tfrac{3}{5}}C^{44}_{22,22} - \tfrac{21}{640}\sqrt{3}C^{31}_{31,22} - \tfrac{27}{640}\sqrt{\tfrac{7}{5}}C^{33}_{31,22} - \tfrac{9}{800}\sqrt{\tfrac{21}{2}}C^{33}_{33,22},$$

$$C^{2202,0}_{00,4202} = \tfrac{3}{64}\sqrt{5}C^{60}_{00,00} + \tfrac{1}{64}\sqrt{15}C^{60}_{00,20} + \tfrac{5}{64}\sqrt{5}C^{51}_{11,00} - \tfrac{1}{64}\sqrt{15}C^{51}_{11,20} + \tfrac{3}{64}\sqrt{5}C^{40}_{20,00} + \tfrac{1}{64}\sqrt{15}C^{40}_{20,20} + \tfrac{3}{32}C^{42}_{22,00} + \tfrac{1}{32}\sqrt{3}C^{42}_{22,20} + \tfrac{5}{64}\sqrt{5}C^{31}_{31,00} - \tfrac{1}{64}\sqrt{15}C^{31}_{31,20} + \tfrac{3}{32}\sqrt{\tfrac{15}{7}}C^{33}_{33,00} - \frac{9C^{33}_{33,20}}{32\sqrt{35}},$$

$$C^{2202,1}_{00,4202} = -\frac{1}{64}\sqrt{15}C^{60}_{00,00}+\frac{3}{64}\sqrt{5}C^{60}_{00,20}+\frac{1}{64}\sqrt{15}C^{51}_{11,00}-\frac{3}{64}\sqrt{5}C^{51}_{11,20}-\frac{1}{64}\sqrt{15}C^{40}_{20,00}+\frac{3}{64}\sqrt{5}C^{40}_{20,20}-\frac{1}{32}\sqrt{3}C^{42}_{22,00}+\frac{3}{32}C^{42}_{22,20}+\frac{1}{64}\sqrt{15}C^{31}_{31,00}-\frac{3}{64}\sqrt{5}C^{31}_{31,20}+\frac{9C^{33}_{33,00}}{32\sqrt{35}}-\frac{9}{32}\sqrt{\frac{3}{35}}C^{33}_{33,20},$$

$$C^{2011,0}_{00,4211} = -\frac{3}{64}C^{62}_{00,22}-\frac{9}{64}C^{51}_{11,22}-\frac{27}{64}\sqrt{\frac{3}{35}}C^{53}_{11,22}-\frac{3}{64}C^{42}_{20,22}-\frac{3}{64}C^{40}_{22,22}-\frac{3C^{42}_{22,22}}{32\sqrt{7}}-\frac{9C^{44}_{22,22}}{112\sqrt{5}}-\frac{9}{64}C^{31}_{31,22}-\frac{27}{64}\sqrt{\frac{3}{35}}C^{33}_{31,22}-\frac{27C^{33}_{33,22}}{80\sqrt{14}},$$

$$C^{2011,1}_{00,4211} = \frac{3}{64}\sqrt{3}C^{62}_{00,22}-\frac{3}{64}\sqrt{3}C^{51}_{11,22}-\frac{27C^{53}_{11,22}}{64\sqrt{35}}+\frac{3}{64}\sqrt{3}C^{42}_{20,22}+\frac{3}{64}\sqrt{3}C^{40}_{22,22}+\frac{3}{32}\sqrt{\frac{3}{7}}C^{42}_{22,22}+\frac{9}{112}\sqrt{\frac{3}{5}}C^{44}_{22,22}-\frac{3}{64}\sqrt{3}C^{31}_{31,22}-\frac{27C^{33}_{31,22}}{64\sqrt{35}}-\frac{9}{80}\sqrt{\frac{3}{14}}C^{33}_{33,22},$$

$$C^{2211,0}_{00,4211} = -\frac{1}{64}\sqrt{3}C^{60}_{00,00}-\frac{5}{64}C^{60}_{00,20}-\frac{3C^{62}_{00,22}}{64\sqrt{5}}+\frac{1}{64}\sqrt{3}C^{51}_{11,00}-\frac{3}{64}C^{51}_{11,20}-\frac{9C^{51}_{11,22}}{64\sqrt{5}}-\frac{27}{320}\sqrt{\frac{3}{7}}C^{53}_{11,22}-\frac{1}{64}\sqrt{3}C^{40}_{20,00}-\frac{5}{64}C^{40}_{20,20}-\frac{3C^{42}_{20,22}}{64\sqrt{5}}-\frac{1}{32}\sqrt{\frac{3}{5}}C^{42}_{22,00}-\frac{1}{32}\sqrt{5}C^{42}_{22,20}-\frac{3C^{40}_{22,22}}{64\sqrt{5}}-\frac{3C^{42}_{22,22}}{32\sqrt{35}}-\frac{9}{560}C^{44}_{22,22}+\frac{1}{64}\sqrt{3}C^{31}_{31,00}-\frac{3}{64}C^{31}_{31,20}-\frac{9C^{31}_{31,22}}{64\sqrt{5}}-\frac{27}{320}\sqrt{\frac{3}{7}}C^{33}_{31,22}+\frac{9C^{33}_{33,00}}{160\sqrt{7}}-\frac{9}{160}\sqrt{\frac{3}{7}}C^{33}_{33,20}-\frac{27C^{33}_{33,22}}{80\sqrt{70}},$$

$$C^{2211,1}_{00,4211} = -\frac{3}{64}C^{60}_{00,00}-\frac{1}{64}\sqrt{3}C^{60}_{00,20}+\frac{3}{64}\sqrt{\frac{3}{5}}C^{62}_{00,22}+\frac{3}{64}C^{51}_{11,00}+\frac{1}{64}\sqrt{3}C^{51}_{11,20}-\frac{3}{64}\sqrt{\frac{3}{5}}C^{51}_{11,22}-\frac{27C^{53}_{11,22}}{320\sqrt{7}}-\frac{3}{64}C^{40}_{20,00}-\frac{1}{64}\sqrt{3}C^{40}_{20,20}+\frac{3}{64}\sqrt{\frac{3}{5}}C^{42}_{20,22}-\frac{3C^{42}_{22,00}}{32\sqrt{5}}-\frac{1}{32}\sqrt{\frac{3}{5}}C^{42}_{22,20}+\frac{3}{64}\sqrt{\frac{3}{5}}C^{40}_{22,22}+\frac{3}{32}\sqrt{\frac{3}{35}}C^{42}_{22,22}+\frac{9}{560}\sqrt{3}C^{44}_{22,22}+\frac{3}{64}C^{31}_{31,00}+\frac{1}{64}\sqrt{3}C^{31}_{31,20}-\frac{3}{64}\sqrt{\frac{3}{5}}C^{31}_{31,22}-\frac{27C^{33}_{31,22}}{320\sqrt{7}}+\frac{9}{160}\sqrt{\frac{3}{7}}C^{33}_{33,00}+\frac{9C^{33}_{33,20}}{160\sqrt{7}}-\frac{9}{80}\sqrt{\frac{3}{70}}C^{33}_{33,22},$$

$$C^{2212,0}_{00,4212} = -\frac{1}{64}\sqrt{5}C^{60}_{00,00}-\frac{5}{64}\sqrt{\frac{5}{3}}C^{60}_{00,20}+\frac{1}{64}\sqrt{3}C^{62}_{00,22}+\frac{1}{64}\sqrt{5}C^{51}_{11,00}-\frac{1}{64}\sqrt{15}C^{51}_{11,20}+\frac{3}{64}\sqrt{3}C^{51}_{11,22}+\frac{27C^{53}_{11,22}}{64\sqrt{35}}-\frac{1}{64}\sqrt{5}C^{40}_{20,00}-\frac{5}{64}\sqrt{\frac{5}{3}}C^{40}_{20,20}+\frac{1}{64}\sqrt{3}C^{42}_{20,22}-\frac{1}{32}C^{42}_{22,00}-\frac{5C^{42}_{22,20}}{32\sqrt{3}}+\frac{1}{64}\sqrt{3}C^{40}_{22,22}+\frac{1}{32}\sqrt{\frac{3}{7}}C^{42}_{22,22}+\frac{3}{112}\sqrt{\frac{3}{5}}C^{44}_{22,22}+\frac{1}{64}\sqrt{5}C^{31}_{31,00}-\frac{1}{64}\sqrt{15}C^{31}_{31,20}+\frac{3}{64}\sqrt{3}C^{31}_{31,22}+\frac{27C^{33}_{31,22}}{64\sqrt{35}}+\frac{3}{32}\sqrt{\frac{3}{35}}C^{33}_{33,00}-\frac{9C^{33}_{33,20}}{32\sqrt{35}}+\frac{9}{80}\sqrt{\frac{3}{14}}C^{33}_{33,22},$$

$$C^{2212,1}_{00,4212} = -\frac{1}{64}\sqrt{15}C^{60}_{00,00}-\frac{1}{64}\sqrt{5}C^{60}_{00,20}-\frac{3}{64}C^{62}_{00,22}+\frac{1}{64}\sqrt{15}C^{51}_{11,00}+\frac{1}{64}\sqrt{5}C^{51}_{11,20}+\frac{3}{64}C^{51}_{11,22}+\frac{9}{64}\sqrt{\frac{3}{35}}C^{53}_{11,22}-\frac{1}{64}\sqrt{15}C^{40}_{20,00}-\frac{1}{64}\sqrt{5}C^{40}_{20,20}-\frac{3}{64}C^{42}_{20,22}-\frac{1}{32}\sqrt{3}C^{42}_{22,00}-\frac{1}{32}C^{42}_{22,20}-\frac{3}{64}C^{40}_{22,22}-\frac{3C^{42}_{22,22}}{32\sqrt{7}}-\frac{9C^{44}_{22,22}}{112\sqrt{5}}+\frac{1}{64}\sqrt{15}C^{31}_{31,00}+\frac{1}{64}\sqrt{5}C^{31}_{31,20}+\frac{3}{64}C^{31}_{31,22}+\frac{9}{64}\sqrt{\frac{3}{35}}C^{33}_{31,22}+\frac{9C^{33}_{33,00}}{32\sqrt{35}}+\frac{3}{32}\sqrt{\frac{3}{35}}C^{33}_{33,20}+\frac{9C^{33}_{33,22}}{80\sqrt{14}},$$

$$C^{2213,0}_{00,4213} = -\frac{1}{64}\sqrt{7}C^{60}_{00,00}-\frac{5}{64}\sqrt{\frac{7}{3}}C^{60}_{00,20}-\frac{1}{32}\sqrt{\frac{3}{35}}C^{62}_{00,22}+\frac{1}{64}\sqrt{7}C^{51}_{11,00}-\frac{1}{64}\sqrt{21}C^{51}_{11,20}-\frac{3}{32}\sqrt{\frac{3}{35}}C^{51}_{11,22}-\frac{27C^{53}_{11,22}}{1120}-\frac{1}{64}\sqrt{7}C^{40}_{20,00}-\frac{5}{64}\sqrt{\frac{7}{3}}C^{40}_{20,20}-\frac{1}{32}\sqrt{\frac{3}{35}}C^{42}_{20,22}-\frac{1}{32}\sqrt{\frac{7}{5}}C^{42}_{22,00}-\frac{1}{32}\sqrt{\frac{35}{3}}C^{42}_{22,20}-\frac{1}{32}\sqrt{\frac{3}{35}}C^{40}_{22,22}-\frac{1}{112}\sqrt{\frac{3}{5}}C^{42}_{22,22}-\frac{3}{280}\sqrt{\frac{3}{7}}C^{44}_{22,22}+\frac{1}{64}\sqrt{7}C^{31}_{31,00}-\frac{1}{64}\sqrt{21}C^{31}_{31,20}-\frac{3}{32}\sqrt{\frac{3}{35}}C^{31}_{31,22}-\frac{27C^{33}_{31,22}}{1120}+\frac{3}{160}\sqrt{3}C^{33}_{33,00}-\frac{9}{160}C^{33}_{33,20}-\frac{9}{280}\sqrt{\frac{3}{10}}C^{33}_{33,22},$$

$$C^{2213,1}_{00,4213} = -\frac{1}{64}\sqrt{21}C^{60}_{00,00}-\frac{1}{64}\sqrt{7}C^{60}_{00,20}+\frac{3C^{62}_{00,22}}{32\sqrt{35}}+\frac{1}{64}\sqrt{21}C^{51}_{11,00}+\frac{1}{64}\sqrt{7}C^{51}_{11,20}-\frac{3C^{51}_{11,22}}{32\sqrt{35}}-\frac{9\sqrt{3}C^{53}_{11,22}}{1120}-\frac{1}{64}\sqrt{21}C^{40}_{20,00}-\frac{1}{64}\sqrt{7}C^{40}_{20,20}+\frac{3C^{42}_{20,22}}{32\sqrt{35}}-\frac{1}{32}\sqrt{\frac{21}{5}}C^{42}_{22,00}-\frac{1}{32}\sqrt{\frac{7}{5}}C^{42}_{22,20}+$$

$\frac{3C^{40}_{22,22}}{32\sqrt{35}} + \frac{3C^{42}_{22,22}}{112\sqrt{5}} + \frac{9C^{44}_{22,22}}{280\sqrt{7}} + \frac{1}{64}\sqrt{21}C^{31}_{31,00} + \frac{1}{64}\sqrt{7}C^{31}_{31,20} - \frac{3C^{31}_{31,22}}{32\sqrt{35}} - \frac{9\sqrt{3}C^{33}_{31,22}}{1120} +$
$\frac{9}{160}C^{33}_{33,00} + \frac{3}{160}\sqrt{3}C^{33}_{33,20} - \frac{9C^{33}_{33,22}}{280\sqrt{10}},$

$C^{2213,0}_{00,4413} = -\frac{C^{62}_{00,22}}{32\sqrt{5}} - \frac{3C^{51}_{11,22}}{32\sqrt{5}} - \frac{9}{160}\sqrt{\frac{3}{7}}C^{53}_{11,22} - \frac{C^{42}_{20,22}}{32\sqrt{5}} - \frac{C^{40}_{22,22}}{32\sqrt{5}} - \frac{C^{42}_{22,22}}{16\sqrt{35}} - \frac{3}{280}C^{44}_{22,22} -$
$\frac{3C^{31}_{31,22}}{32\sqrt{5}} - \frac{9}{160}\sqrt{\frac{3}{7}}C^{33}_{31,22} - \frac{9C^{33}_{33,22}}{40\sqrt{70}},$

$C^{2213,1}_{00,4413} = \frac{1}{32}\sqrt{\frac{3}{5}}C^{62}_{00,22} - \frac{1}{32}\sqrt{\frac{3}{5}}C^{51}_{11,22} - \frac{9C^{53}_{11,22}}{160\sqrt{7}} + \frac{1}{32}\sqrt{\frac{3}{5}}C^{42}_{20,22} + \frac{1}{32}\sqrt{\frac{3}{5}}C^{40}_{22,22} +$
$\frac{1}{16}\sqrt{\frac{3}{35}}C^{42}_{22,22} + \frac{3}{280}\sqrt{3}C^{44}_{22,22} - \frac{1}{32}\sqrt{\frac{3}{5}}C^{31}_{31,22} - \frac{9C^{33}_{31,22}}{160\sqrt{7}} - \frac{3}{40}\sqrt{\frac{3}{70}}C^{33}_{33,22},$

$C^{1101,0}_{00,5101} = -\frac{9}{128}C^{60}_{00,00} - \frac{3}{128}\sqrt{3}C^{60}_{00,20} - \frac{15}{128}C^{51}_{11,00} + \frac{3}{128}\sqrt{3}C^{51}_{11,20} - \frac{9}{128}C^{40}_{20,00} -$
$\frac{3}{128}\sqrt{3}C^{40}_{20,20} - \frac{9C^{42}_{22,00}}{64\sqrt{5}} - \frac{3}{64}\sqrt{\frac{3}{5}}C^{42}_{22,20} - \frac{15}{128}C^{31}_{31,00} + \frac{3}{128}\sqrt{3}C^{31}_{31,20} - \frac{9}{64}\sqrt{\frac{3}{7}}C^{33}_{33,00} +$
$\frac{27C^{33}_{33,20}}{320\sqrt{7}},$

$C^{1101,1}_{00,5101} = \frac{3}{128}\sqrt{3}C^{60}_{00,00} - \frac{9}{128}C^{60}_{00,20} - \frac{3}{128}\sqrt{3}C^{51}_{11,00} + \frac{9}{128}C^{51}_{11,20} + \frac{3}{128}\sqrt{3}C^{40}_{20,00} -$
$\frac{9}{128}C^{40}_{20,20} + \frac{3}{64}\sqrt{\frac{3}{5}}C^{42}_{22,00} - \frac{9C^{42}_{22,20}}{64\sqrt{5}} - \frac{3}{128}\sqrt{3}C^{31}_{31,00} + \frac{9}{128}C^{31}_{31,20} - \frac{27C^{33}_{33,00}}{320\sqrt{7}} + \frac{27}{320}\sqrt{\frac{3}{7}}C^{33}_{33,20},$

$C^{1110,0}_{00,5110} = \frac{1}{128}\sqrt{3}C^{60}_{00,00} + \frac{5}{128}C^{60}_{00,20} + \frac{3C^{62}_{00,22}}{64\sqrt{5}} - \frac{1}{128}\sqrt{3}C^{51}_{11,00} + \frac{3}{128}C^{51}_{11,20} + \frac{9C^{51}_{11,22}}{64\sqrt{5}} +$
$\frac{27}{320}\sqrt{\frac{3}{7}}C^{53}_{11,22} + \frac{1}{128}\sqrt{3}C^{40}_{20,00} + \frac{5}{128}C^{40}_{20,20} + \frac{3C^{42}_{20,22}}{64\sqrt{5}} + \frac{1}{64}\sqrt{\frac{3}{5}}C^{42}_{22,00} + \frac{1}{64}\sqrt{5}C^{42}_{22,20} +$
$\frac{3C^{40}_{22,22}}{64\sqrt{5}} + \frac{3C^{42}_{22,22}}{32\sqrt{35}} + \frac{9}{560}C^{44}_{22,22} - \frac{1}{128}\sqrt{3}C^{31}_{31,00} + \frac{3}{128}C^{31}_{31,20} + \frac{9C^{31}_{31,22}}{64\sqrt{5}} + \frac{27}{320}\sqrt{\frac{3}{7}}C^{33}_{31,22} -$
$\frac{9C^{33}_{33,00}}{320\sqrt{7}} + \frac{9}{320}\sqrt{\frac{3}{7}}C^{33}_{33,20} + \frac{27C^{33}_{33,22}}{80\sqrt{70}},$

$C^{1110,1}_{00,5110} = \frac{3}{128}C^{60}_{00,00} + \frac{1}{128}\sqrt{3}C^{60}_{00,20} - \frac{3}{64}\sqrt{\frac{3}{5}}C^{62}_{00,22} - \frac{3}{128}C^{51}_{11,00} - \frac{1}{128}\sqrt{3}C^{51}_{11,20} +$
$\frac{3}{64}\sqrt{\frac{3}{5}}C^{51}_{11,22} + \frac{27C^{53}_{11,22}}{320\sqrt{7}} + \frac{3}{128}C^{40}_{20,00} + \frac{1}{128}\sqrt{3}C^{40}_{20,20} - \frac{3}{64}\sqrt{\frac{3}{5}}C^{42}_{20,22} + \frac{3C^{42}_{22,00}}{64\sqrt{5}} +$
$\frac{1}{64}\sqrt{\frac{3}{5}}C^{42}_{22,20} - \frac{3}{64}\sqrt{\frac{3}{5}}C^{40}_{22,22} - \frac{3}{32}\sqrt{\frac{3}{35}}C^{42}_{22,22} - \frac{9}{560}\sqrt{3}C^{44}_{22,22} - \frac{3}{128}C^{31}_{31,00} - \frac{1}{128}\sqrt{3}C^{31}_{31,20} +$
$\frac{3}{64}\sqrt{\frac{3}{5}}C^{31}_{31,22} + \frac{27C^{33}_{31,22}}{320\sqrt{7}} - \frac{9}{320}\sqrt{\frac{3}{7}}C^{33}_{33,00} - \frac{9C^{33}_{33,20}}{320\sqrt{7}} + \frac{9}{80}\sqrt{\frac{3}{70}}C^{33}_{33,22},$

$C^{1111,0}_{00,5111} = \frac{3}{128}C^{60}_{00,00} + \frac{5}{128}\sqrt{3}C^{60}_{00,20} - \frac{3}{128}\sqrt{\frac{3}{5}}C^{62}_{00,22} - \frac{3}{128}C^{51}_{11,00} + \frac{3}{128}\sqrt{3}C^{51}_{11,20} -$
$\frac{9}{128}\sqrt{\frac{3}{5}}C^{51}_{11,22} - \frac{81C^{53}_{11,22}}{640\sqrt{7}} + \frac{3}{128}C^{40}_{20,00} + \frac{5}{128}\sqrt{3}C^{40}_{20,20} - \frac{3}{128}\sqrt{\frac{3}{5}}C^{42}_{20,22} + \frac{3C^{42}_{22,00}}{64\sqrt{5}} +$
$\frac{1}{64}\sqrt{15}C^{42}_{22,20} - \frac{3}{128}\sqrt{\frac{3}{5}}C^{40}_{22,22} - \frac{3}{64}\sqrt{\frac{3}{35}}C^{42}_{22,22} - \frac{9\sqrt{3}C^{44}_{22,22}}{1120} - \frac{3}{128}C^{31}_{31,00} + \frac{3}{128}\sqrt{3}C^{31}_{31,20} -$
$\frac{9}{128}\sqrt{\frac{3}{5}}C^{31}_{31,22} - \frac{81C^{33}_{31,22}}{640\sqrt{7}} - \frac{9}{320}\sqrt{\frac{3}{7}}C^{33}_{33,00} + \frac{27C^{33}_{33,20}}{320\sqrt{7}} - \frac{27}{160}\sqrt{\frac{3}{70}}C^{33}_{33,22},$

$C^{1111,1}_{00,5111} = \frac{3}{128}\sqrt{3}C^{60}_{00,00} + \frac{3}{128}C^{60}_{00,20} + \frac{9C^{62}_{00,22}}{128\sqrt{5}} - \frac{3}{128}\sqrt{3}C^{51}_{11,00} - \frac{3}{128}C^{51}_{11,20} - \frac{9C^{51}_{11,22}}{128\sqrt{5}} -$
$\frac{27}{640}\sqrt{\frac{3}{7}}C^{53}_{11,22} + \frac{3}{128}\sqrt{3}C^{40}_{20,00} + \frac{3}{128}C^{40}_{20,20} + \frac{9C^{42}_{20,22}}{128\sqrt{5}} + \frac{3}{64}\sqrt{\frac{3}{5}}C^{42}_{22,00} + \frac{3C^{42}_{22,20}}{64\sqrt{5}} + \frac{9C^{40}_{22,22}}{128\sqrt{5}} +$
$\frac{9C^{42}_{22,22}}{64\sqrt{35}} + \frac{27C^{44}_{22,22}}{1120} - \frac{3}{128}\sqrt{3}C^{31}_{31,00} - \frac{3}{128}C^{31}_{31,20} - \frac{9C^{31}_{31,22}}{128\sqrt{5}} - \frac{27}{640}\sqrt{\frac{3}{7}}C^{33}_{31,22} - \frac{27C^{33}_{33,00}}{320\sqrt{7}} -$
$\frac{9}{320}\sqrt{\frac{3}{7}}C^{33}_{33,20} - \frac{27C^{33}_{33,22}}{160\sqrt{70}},$

$C^{1112,0}_{00,5112} = \frac{1}{128}\sqrt{15}C^{60}_{00,00} + \frac{5}{128}\sqrt{5}C^{60}_{00,20} + \frac{3}{640}C^{62}_{00,22} - \frac{1}{128}\sqrt{15}C^{51}_{11,00} + \frac{3}{128}\sqrt{5}C^{51}_{11,20} +$
$\frac{9}{640}C^{51}_{11,22} + \frac{27}{640}\sqrt{\frac{3}{35}}C^{53}_{11,22} + \frac{1}{128}\sqrt{15}C^{40}_{20,00} + \frac{5}{128}\sqrt{5}C^{40}_{20,20} + \frac{3}{640}C^{42}_{20,22} + \frac{1}{64}\sqrt{3}C^{42}_{22,00} +$

$\frac{5}{64}C^{42}_{22,20}+\frac{3}{640}C^{40}_{22,22}+\frac{3C^{42}_{22,22}}{320\sqrt{7}}+\frac{9C^{44}_{22,22}}{1120\sqrt{5}}-\frac{1}{128}\sqrt{15}C^{31}_{31,00}+\frac{3}{128}\sqrt{5}C^{31}_{31,20}+\frac{9}{640}C^{31}_{31,22}+\frac{27}{640}\sqrt{\frac{3}{35}}C^{33}_{31,22}-\frac{9C^{33}_{33,00}}{64\sqrt{35}}+\frac{9}{64}\sqrt{\frac{3}{35}}C^{33}_{33,20}+\frac{27C^{33}_{33,22}}{800\sqrt{14}}$,

$C^{1112,1}_{00,5112}=\frac{3}{128}\sqrt{5}C^{60}_{00,00}+\frac{1}{128}\sqrt{15}C^{60}_{00,20}-\frac{3}{640}\sqrt{3}C^{62}_{00,22}-\frac{3}{128}\sqrt{5}C^{51}_{11,00}-\frac{1}{128}\sqrt{15}C^{51}_{11,20}+\frac{3}{640}\sqrt{3}C^{51}_{11,22}+\frac{27C^{53}_{11,22}}{640\sqrt{35}}+\frac{3}{128}\sqrt{5}C^{40}_{20,00}+\frac{1}{128}\sqrt{15}C^{40}_{20,20}-\frac{3}{640}\sqrt{3}C^{42}_{20,22}+\frac{3}{64}C^{42}_{22,00}+\frac{1}{64}\sqrt{3}C^{42}_{22,20}-\frac{3}{640}\sqrt{3}C^{40}_{22,22}-\frac{3}{320}\sqrt{\frac{3}{7}}C^{42}_{22,22}-\frac{9\sqrt{\frac{3}{5}}C^{44}_{22,22}}{1120}-\frac{3}{128}\sqrt{5}C^{31}_{31,00}-\frac{1}{128}\sqrt{15}C^{31}_{31,20}+\frac{3}{640}\sqrt{3}C^{31}_{31,22}+\frac{27C^{33}_{31,22}}{640\sqrt{35}}-\frac{9}{64}\sqrt{\frac{3}{35}}C^{33}_{33,00}-\frac{9C^{33}_{33,20}}{64\sqrt{35}}+\frac{9}{800}\sqrt{\frac{3}{14}}C^{33}_{33,22}$,

$C^{1112,0}_{00,5312}=\frac{1}{32}\sqrt{\frac{7}{15}}C^{62}_{00,22}+\frac{1}{32}\sqrt{\frac{21}{5}}C^{51}_{11,22}+\frac{9}{160}C^{53}_{11,22}+\frac{1}{32}\sqrt{\frac{7}{15}}C^{42}_{20,22}+\frac{1}{32}\sqrt{\frac{7}{15}}C^{40}_{22,22}+\frac{C^{42}_{22,22}}{16\sqrt{15}}+\frac{1}{40}\sqrt{\frac{3}{7}}C^{44}_{22,22}+\frac{1}{32}\sqrt{\frac{21}{5}}C^{31}_{31,22}+\frac{9}{160}C^{33}_{31,22}+\frac{3}{40}\sqrt{\frac{3}{10}}C^{33}_{33,22}$,

$C^{1112,1}_{00,5312}=-\frac{1}{32}\sqrt{\frac{7}{5}}C^{62}_{00,22}+\frac{1}{32}\sqrt{\frac{7}{5}}C^{51}_{11,22}+\frac{3}{160}\sqrt{3}C^{53}_{11,22}-\frac{1}{32}\sqrt{\frac{7}{5}}C^{42}_{20,22}-\frac{1}{32}\sqrt{\frac{7}{5}}C^{40}_{22,22}-\frac{C^{42}_{22,22}}{16\sqrt{5}}-\frac{3C^{44}_{22,22}}{40\sqrt{7}}+\frac{1}{32}\sqrt{\frac{7}{5}}C^{31}_{31,22}+\frac{3}{160}\sqrt{3}C^{33}_{31,22}+\frac{3C^{33}_{33,22}}{40\sqrt{10}}$,

$C^{0000,0}_{00,6000}=\frac{3}{256}C^{60}_{00,00}+\frac{1}{256}\sqrt{3}C^{60}_{00,20}+\frac{5}{256}C^{51}_{11,00}-\frac{1}{256}\sqrt{3}C^{51}_{11,20}+\frac{3}{256}C^{40}_{20,00}+\frac{1}{256}\sqrt{3}C^{40}_{20,20}+\frac{3C^{42}_{22,00}}{128\sqrt{5}}+\frac{1}{128}\sqrt{\frac{3}{5}}C^{42}_{22,20}+\frac{5}{256}C^{31}_{31,00}-\frac{1}{256}\sqrt{3}C^{31}_{31,20}+\frac{3}{128}\sqrt{\frac{3}{7}}C^{33}_{33,00}-\frac{9C^{33}_{33,20}}{640\sqrt{7}}$,

$C^{0000,1}_{00,6000}=-\frac{1}{256}\sqrt{3}C^{60}_{00,00}+\frac{3}{256}C^{60}_{00,20}+\frac{1}{256}\sqrt{3}C^{51}_{11,00}-\frac{3}{256}C^{51}_{11,20}-\frac{1}{256}\sqrt{3}C^{40}_{20,00}+\frac{3}{256}C^{40}_{20,20}-\frac{1}{128}\sqrt{\frac{3}{5}}C^{42}_{22,00}+\frac{3C^{42}_{22,20}}{128\sqrt{5}}+\frac{1}{256}\sqrt{3}C^{31}_{31,00}-\frac{3}{256}C^{31}_{31,20}+\frac{9C^{33}_{33,00}}{640\sqrt{7}}-\frac{9}{640}\sqrt{\frac{3}{7}}C^{33}_{33,20}$,

$C^{0011,0}_{00,6011}=-\frac{1}{256}\sqrt{3}C^{60}_{00,00}-\frac{5}{256}C^{60}_{00,20}+\frac{1}{256}\sqrt{3}C^{51}_{11,00}-\frac{3}{256}C^{51}_{11,20}-\frac{1}{256}\sqrt{3}C^{40}_{20,00}-\frac{5}{256}C^{40}_{20,20}-\frac{1}{128}\sqrt{\frac{3}{5}}C^{42}_{22,00}-\frac{1}{128}\sqrt{5}C^{42}_{22,20}+\frac{1}{256}\sqrt{3}C^{31}_{31,00}-\frac{3}{256}C^{31}_{31,20}+\frac{9C^{33}_{33,00}}{640\sqrt{7}}-\frac{9}{640}\sqrt{\frac{3}{7}}C^{33}_{33,20}$,

$C^{0011,1}_{00,6011}=-\frac{3}{256}C^{60}_{00,00}-\frac{1}{256}\sqrt{3}C^{60}_{00,20}+\frac{3}{256}C^{51}_{11,00}+\frac{1}{256}\sqrt{3}C^{51}_{11,20}-\frac{3}{256}C^{40}_{20,00}-\frac{1}{256}\sqrt{3}C^{40}_{20,20}-\frac{3C^{42}_{22,00}}{128\sqrt{5}}-\frac{1}{128}\sqrt{\frac{3}{5}}C^{42}_{22,20}+\frac{3}{256}C^{31}_{31,00}+\frac{1}{256}\sqrt{3}C^{31}_{31,20}+\frac{9}{640}\sqrt{\frac{3}{7}}C^{33}_{33,00}+\frac{9C^{33}_{33,20}}{640\sqrt{7}}$,

$C^{0011,0}_{00,6211}=-\frac{1}{128}C^{62}_{00,22}-\frac{3}{128}C^{51}_{11,22}-\frac{9}{128}\sqrt{\frac{3}{35}}C^{53}_{11,22}-\frac{1}{128}C^{42}_{20,22}-\frac{1}{128}C^{40}_{22,22}-\frac{C^{42}_{22,22}}{64\sqrt{7}}-\frac{3C^{44}_{22,22}}{224\sqrt{5}}-\frac{3}{128}C^{31}_{31,22}-\frac{9}{128}\sqrt{\frac{3}{35}}C^{33}_{31,22}-\frac{9C^{33}_{33,22}}{160\sqrt{14}}$,

$C^{0011,1}_{00,6211}=\frac{1}{128}\sqrt{3}C^{62}_{00,22}-\frac{1}{128}\sqrt{3}C^{51}_{11,22}-\frac{9C^{53}_{11,22}}{128\sqrt{35}}+\frac{1}{128}\sqrt{3}C^{42}_{20,22}+\frac{1}{128}\sqrt{3}C^{40}_{22,22}+\frac{1}{64}\sqrt{\frac{3}{7}}C^{42}_{22,22}+\frac{3}{224}\sqrt{\frac{3}{5}}C^{44}_{22,22}-\frac{1}{128}\sqrt{3}C^{31}_{31,22}-\frac{9C^{33}_{31,22}}{128\sqrt{35}}-\frac{3}{160}\sqrt{\frac{3}{14}}C^{33}_{33,22}$,

$C^{5101,0}_{11,0011}=-\frac{3}{64}C^{51}_{11,11}-\frac{1}{32}\sqrt{\frac{3}{5}}C^{42}_{22,11}-\frac{3}{64}C^{31}_{31,11}-\frac{27C^{33}_{33,11}}{80\sqrt{14}}$,

$C^{5101,1}_{11,0011}=-\frac{1}{64}\sqrt{3}C^{51}_{11,11}+\frac{3C^{42}_{22,11}}{32\sqrt{5}}-\frac{1}{64}\sqrt{3}C^{31}_{31,11}-\frac{9}{80}\sqrt{\frac{3}{14}}C^{33}_{33,11}$,

$C^{4000,0}_{11,1111}=-\frac{7}{64}C^{51}_{11,11}-\frac{7C^{42}_{22,11}}{32\sqrt{15}}-\frac{7}{64}C^{31}_{31,11}-\frac{9}{80}\sqrt{\frac{7}{2}}C^{33}_{33,11}$,

$C^{4000,1}_{11,1111}=-\frac{7C^{51}_{11,11}}{64\sqrt{3}}+\frac{7C^{42}_{22,11}}{32\sqrt{5}}-\frac{7C^{31}_{31,11}}{64\sqrt{3}}-\frac{3}{80}\sqrt{\frac{21}{2}}C^{33}_{33,11}$,

$C^{4202,0}_{11,1111}=\frac{1}{32}\sqrt{5}C^{51}_{11,11}+\frac{C^{42}_{22,11}}{16\sqrt{3}}+\frac{1}{32}\sqrt{5}C^{31}_{31,11}+\frac{9C^{33}_{33,11}}{8\sqrt{70}}$,

$$C^{4202,1}_{11,1111} = \frac{1}{32}\sqrt{\frac{5}{3}}C^{51}_{11,11} - \frac{1}{16}C^{42}_{22,11} + \frac{1}{32}\sqrt{\frac{5}{3}}C^{31}_{31,11} + \frac{3}{8}\sqrt{\frac{3}{70}}C^{33}_{33,11},$$
$$C^{4202,0}_{11,1112} = \frac{1}{32}\sqrt{15}C^{51}_{11,11} + \frac{1}{16}C^{42}_{22,11} + \frac{1}{32}\sqrt{15}C^{31}_{31,11} + \frac{9}{8}\sqrt{\frac{3}{70}}C^{33}_{33,11},$$
$$C^{4202,1}_{11,1112} = \frac{1}{32}\sqrt{5}C^{51}_{11,11} - \frac{1}{16}\sqrt{3}C^{42}_{22,11} + \frac{1}{32}\sqrt{5}C^{31}_{31,11} + \frac{9C^{33}_{33,11}}{8\sqrt{70}},$$
$$C^{3101,0}_{11,2011} = -\frac{7}{32}C^{51}_{11,11} - \frac{7C^{42}_{22,11}}{16\sqrt{15}} - \frac{7}{32}C^{31}_{31,11} - \frac{9}{40}\sqrt{\frac{7}{2}}C^{33}_{33,11},$$
$$C^{3101,1}_{11,2011} = -\frac{7C^{51}_{11,11}}{32\sqrt{3}} + \frac{7C^{42}_{22,11}}{16\sqrt{5}} - \frac{7C^{31}_{31,11}}{32\sqrt{3}} - \frac{3}{40}\sqrt{\frac{21}{2}}C^{33}_{33,11},$$
$$C^{3101,0}_{11,2211} = \frac{7C^{51}_{11,11}}{32\sqrt{5}} + \frac{7C^{42}_{22,11}}{80\sqrt{3}} + \frac{7C^{31}_{31,11}}{32\sqrt{5}} + \frac{9}{40}\sqrt{\frac{7}{10}}C^{33}_{33,11},$$
$$C^{3101,1}_{11,2211} = \frac{7C^{51}_{11,11}}{32\sqrt{15}} - \frac{7}{80}C^{42}_{22,11} + \frac{7C^{31}_{31,11}}{32\sqrt{15}} + \frac{3}{40}\sqrt{\frac{21}{10}}C^{33}_{33,11},$$
$$C^{3101,0}_{11,2212} = \frac{7}{32}\sqrt{\frac{3}{5}}C^{51}_{11,11} + \frac{7}{80}C^{42}_{22,11} + \frac{7}{32}\sqrt{\frac{3}{5}}C^{31}_{31,11} + \frac{9}{40}\sqrt{\frac{21}{10}}C^{33}_{33,11},$$
$$C^{3101,1}_{11,2212} = \frac{7C^{51}_{11,11}}{32\sqrt{5}} - \frac{7}{80}\sqrt{3}C^{42}_{22,11} + \frac{7C^{31}_{31,11}}{32\sqrt{5}} + \frac{9}{40}\sqrt{\frac{7}{10}}C^{33}_{33,11},$$
$$C^{3303,0}_{11,2212} = -\frac{1}{48}\sqrt{7}C^{51}_{11,11} - \frac{1}{24}\sqrt{\frac{7}{15}}C^{42}_{22,11} - \frac{1}{48}\sqrt{7}C^{31}_{31,11} - \frac{3C^{33}_{33,11}}{20\sqrt{2}},$$
$$C^{3303,1}_{11,2212} = -\frac{1}{48}\sqrt{\frac{7}{3}}C^{51}_{11,11} + \frac{1}{24}\sqrt{\frac{7}{5}}C^{42}_{22,11} - \frac{1}{48}\sqrt{\frac{7}{3}}C^{31}_{31,11} - \frac{1}{20}\sqrt{\frac{3}{2}}C^{33}_{33,11},$$
$$C^{3303,0}_{11,2213} = -\frac{1}{24}\sqrt{\frac{7}{2}}C^{51}_{11,11} - \frac{1}{12}\sqrt{\frac{7}{30}}C^{42}_{22,11} - \frac{1}{24}\sqrt{\frac{7}{2}}C^{31}_{31,11} - \frac{3}{20}C^{33}_{33,11},$$
$$C^{3303,1}_{11,2213} = -\frac{1}{24}\sqrt{\frac{7}{6}}C^{51}_{11,11} + \frac{1}{12}\sqrt{\frac{7}{10}}C^{42}_{22,11} - \frac{1}{24}\sqrt{\frac{7}{6}}C^{31}_{31,11} - \frac{1}{20}\sqrt{3}C^{33}_{33,11},$$
$$C^{2000,0}_{11,3111} = -\frac{7}{32}C^{51}_{11,11} - \frac{7C^{42}_{22,11}}{16\sqrt{15}} - \frac{7}{32}C^{31}_{31,11} - \frac{9}{40}\sqrt{\frac{7}{2}}C^{33}_{33,11},$$
$$C^{2000,1}_{11,3111} = -\frac{7C^{51}_{11,11}}{32\sqrt{3}} + \frac{7C^{42}_{22,11}}{16\sqrt{5}} - \frac{7C^{31}_{31,11}}{32\sqrt{3}} - \frac{3}{40}\sqrt{\frac{21}{2}}C^{33}_{33,11},$$
$$C^{2202,0}_{11,3111} = \frac{7C^{51}_{11,11}}{32\sqrt{5}} + \frac{7C^{42}_{22,11}}{80\sqrt{3}} + \frac{7C^{31}_{31,11}}{32\sqrt{5}} + \frac{9}{40}\sqrt{\frac{7}{10}}C^{33}_{33,11},$$
$$C^{2202,1}_{11,3111} = \frac{7C^{51}_{11,11}}{32\sqrt{15}} - \frac{7}{80}C^{42}_{22,11} + \frac{7C^{31}_{31,11}}{32\sqrt{15}} + \frac{3}{40}\sqrt{\frac{21}{10}}C^{33}_{33,11},$$
$$C^{2202,0}_{11,3112} = \frac{7}{32}\sqrt{\frac{3}{5}}C^{51}_{11,11} + \frac{7}{80}C^{42}_{22,11} + \frac{7}{32}\sqrt{\frac{3}{5}}C^{31}_{31,11} + \frac{9}{40}\sqrt{\frac{21}{10}}C^{33}_{33,11},$$
$$C^{2202,1}_{11,3112} = \frac{7C^{51}_{11,11}}{32\sqrt{5}} - \frac{7}{80}\sqrt{3}C^{42}_{22,11} + \frac{7C^{31}_{31,11}}{32\sqrt{5}} + \frac{9}{40}\sqrt{\frac{7}{10}}C^{33}_{33,11},$$
$$C^{2202,0}_{11,3312} = -\frac{1}{48}\sqrt{7}C^{51}_{11,11} - \frac{1}{24}\sqrt{\frac{7}{15}}C^{42}_{22,11} - \frac{1}{48}\sqrt{7}C^{31}_{31,11} - \frac{3C^{33}_{33,11}}{20\sqrt{2}},$$
$$C^{2202,1}_{11,3312} = -\frac{1}{48}\sqrt{\frac{7}{3}}C^{51}_{11,11} + \frac{1}{24}\sqrt{\frac{7}{5}}C^{42}_{22,11} - \frac{1}{48}\sqrt{\frac{7}{3}}C^{31}_{31,11} - \frac{1}{20}\sqrt{\frac{3}{2}}C^{33}_{33,11},$$
$$C^{2202,0}_{11,3313} = -\frac{1}{24}\sqrt{\frac{7}{2}}C^{51}_{11,11} - \frac{1}{12}\sqrt{\frac{7}{30}}C^{42}_{22,11} - \frac{1}{24}\sqrt{\frac{7}{2}}C^{31}_{31,11} - \frac{3}{20}C^{33}_{33,11},$$
$$C^{2202,1}_{11,3313} = -\frac{1}{24}\sqrt{\frac{7}{6}}C^{51}_{11,11} + \frac{1}{12}\sqrt{\frac{7}{10}}C^{42}_{22,11} - \frac{1}{24}\sqrt{\frac{7}{6}}C^{31}_{31,11} - \frac{1}{20}\sqrt{3}C^{33}_{33,11},$$
$$C^{1101,0}_{11,4011} = -\frac{7}{64}C^{51}_{11,11} - \frac{7C^{42}_{22,11}}{32\sqrt{15}} - \frac{7}{64}C^{31}_{31,11} - \frac{9}{80}\sqrt{\frac{7}{2}}C^{33}_{33,11},$$
$$C^{1101,1}_{11,4011} = -\frac{7C^{51}_{11,11}}{64\sqrt{3}} + \frac{7C^{42}_{22,11}}{32\sqrt{5}} - \frac{7C^{31}_{31,11}}{64\sqrt{3}} - \frac{3}{80}\sqrt{\frac{21}{2}}C^{33}_{33,11},$$
$$C^{1101,0}_{11,4211} = \frac{1}{32}\sqrt{5}C^{51}_{11,11} + \frac{C^{42}_{22,11}}{16\sqrt{3}} + \frac{1}{32}\sqrt{5}C^{31}_{31,11} + \frac{9C^{33}_{33,11}}{8\sqrt{70}},$$
$$C^{1101,1}_{11,4211} = \frac{1}{32}\sqrt{\frac{5}{3}}C^{51}_{11,11} - \frac{1}{16}C^{42}_{22,11} + \frac{1}{32}\sqrt{\frac{5}{3}}C^{31}_{31,11} + \frac{3}{8}\sqrt{\frac{3}{70}}C^{33}_{33,11},$$
$$C^{1101,0}_{11,4212} = \frac{1}{32}\sqrt{15}C^{51}_{11,11} + \frac{1}{16}C^{42}_{22,11} + \frac{1}{32}\sqrt{15}C^{31}_{31,11} + \frac{9}{8}\sqrt{\frac{3}{70}}C^{33}_{33,11},$$

$$C^{1101,1}_{11,4212} = \frac{1}{32}\sqrt{5}C^{51}_{11,11} - \frac{1}{16}\sqrt{3}C^{42}_{22,11} + \frac{1}{32}\sqrt{5}C^{31}_{31,11} + \frac{9C^{33}_{33,11}}{8\sqrt{70}},$$

$$C^{0000,0}_{11,5111} = -\frac{3}{64}C^{51}_{11,11} - \frac{1}{32}\sqrt{\frac{3}{5}}C^{42}_{22,11} - \frac{3}{64}C^{31}_{31,11} - \frac{27C^{33}_{33,11}}{80\sqrt{14}},$$

$$C^{0000,1}_{11,5111} = -\frac{1}{64}\sqrt{3}C^{51}_{11,11} + \frac{3C^{42}_{22,11}}{32\sqrt{5}} - \frac{1}{64}\sqrt{3}C^{31}_{31,11} - \frac{9}{80}\sqrt{\frac{3}{14}}C^{33}_{33,11},$$

$$C^{2000,0}_{20,2000} = -\frac{35}{256}C^{60}_{00,00} - \frac{35C^{60}_{00,20}}{256\sqrt{3}} - \frac{175C^{51}_{11,00}}{2304} + \frac{35C^{51}_{11,20}}{768\sqrt{3}} - \frac{25}{768}C^{40}_{20,00} - \frac{25C^{40}_{20,20}}{768\sqrt{3}} + \frac{7}{384}\sqrt{5}C^{42}_{22,00} + \frac{7}{384}\sqrt{\frac{5}{3}}C^{42}_{22,20} + \frac{25C^{31}_{31,00}}{2304} - \frac{5C^{31}_{31,20}}{768\sqrt{3}} + \frac{5}{128}\sqrt{21}C^{33}_{33,00} - \frac{3}{128}\sqrt{7}C^{33}_{33,20},$$

$$C^{2000,1}_{20,2000} = \frac{35C^{60}_{00,00}}{256\sqrt{3}} - \frac{35}{256}C^{60}_{00,20} - \frac{35C^{51}_{11,00}}{768\sqrt{3}} + \frac{35}{768}C^{51}_{11,20} + \frac{25C^{40}_{20,00}}{768\sqrt{3}} - \frac{25}{768}C^{40}_{20,20} - \frac{7}{384}\sqrt{\frac{5}{3}}C^{42}_{22,00} + \frac{7}{384}\sqrt{5}C^{42}_{22,20} + \frac{5C^{31}_{31,00}}{768\sqrt{3}} - \frac{5}{768}C^{31}_{31,20} + \frac{3}{128}\sqrt{7}C^{33}_{33,00} - \frac{3}{128}\sqrt{21}C^{33}_{33,20},$$

$$C^{2011,0}_{20,2011} = \frac{35C^{60}_{00,00}}{256\sqrt{3}} + \frac{175}{768}C^{60}_{00,20} - \frac{35C^{51}_{11,00}}{768\sqrt{3}} + \frac{35}{768}C^{51}_{11,20} + \frac{25C^{40}_{20,00}}{768\sqrt{3}} + \frac{125C^{40}_{20,20}}{2304} - \frac{7}{384}\sqrt{\frac{5}{3}}C^{42}_{22,00} - \frac{35\sqrt{5}C^{42}_{22,20}}{1152} + \frac{5C^{31}_{31,00}}{768\sqrt{3}} - \frac{5}{768}C^{31}_{31,20} + \frac{3}{128}\sqrt{7}C^{33}_{33,00} - \frac{3}{128}\sqrt{21}C^{33}_{33,20},$$

$$C^{2011,1}_{20,2011} = \frac{35}{256}C^{60}_{00,00} + \frac{35C^{60}_{00,20}}{256\sqrt{3}} - \frac{35}{768}C^{51}_{11,00} - \frac{35C^{51}_{11,20}}{768\sqrt{3}} + \frac{25}{768}C^{40}_{20,00} + \frac{25C^{40}_{20,20}}{768\sqrt{3}} - \frac{7}{384}\sqrt{5}C^{42}_{22,00} - \frac{7}{384}\sqrt{\frac{5}{3}}C^{42}_{22,20} + \frac{5}{768}C^{31}_{31,00} + \frac{5C^{31}_{31,20}}{768\sqrt{3}} + \frac{3}{128}\sqrt{21}C^{33}_{33,00} + \frac{3}{128}\sqrt{7}C^{33}_{33,20},$$

$$C^{2202,0}_{20,2202} = -\frac{7}{128}\sqrt{5}C^{60}_{00,00} - \frac{7}{128}\sqrt{\frac{5}{3}}C^{60}_{00,20} - \frac{35\sqrt{5}C^{51}_{11,00}}{1152} + \frac{7}{384}\sqrt{\frac{5}{3}}C^{51}_{11,20} - \frac{5}{384}\sqrt{5}C^{40}_{20,00} - \frac{5}{384}\sqrt{\frac{5}{3}}C^{40}_{20,20} + \frac{7}{192}C^{42}_{22,00} + \frac{7C^{42}_{22,20}}{192\sqrt{3}} + \frac{5\sqrt{5}C^{31}_{31,00}}{1152} - \frac{1}{384}\sqrt{\frac{5}{3}}C^{31}_{31,20} + \frac{1}{64}\sqrt{105}C^{33}_{33,00} - \frac{3}{64}\sqrt{\frac{7}{5}}C^{33}_{33,20},$$

$$C^{2202,1}_{20,2202} = \frac{7}{128}\sqrt{\frac{5}{3}}C^{60}_{00,00} - \frac{7}{128}\sqrt{5}C^{60}_{00,20} - \frac{7}{384}\sqrt{\frac{5}{3}}C^{51}_{11,00} + \frac{7}{384}\sqrt{5}C^{51}_{11,20} + \frac{5}{384}\sqrt{\frac{5}{3}}C^{40}_{20,00} - \frac{5}{384}\sqrt{5}C^{40}_{20,20} - \frac{7C^{42}_{22,00}}{192\sqrt{3}} + \frac{7}{192}C^{42}_{22,20} + \frac{1}{384}\sqrt{\frac{5}{3}}C^{31}_{31,00} - \frac{1}{384}\sqrt{5}C^{31}_{31,20} + \frac{3}{64}\sqrt{\frac{7}{5}}C^{33}_{33,00} - \frac{3}{64}\sqrt{\frac{21}{5}}C^{33}_{33,20},$$

$$C^{2011,0}_{20,2211} = \frac{7}{64}C^{62}_{00,22} + \frac{35}{192}C^{51}_{11,22} + \frac{7}{576}C^{42}_{20,22} + \frac{7}{576}C^{40}_{22,22} - \frac{1}{144}\sqrt{7}C^{42}_{22,22} - \frac{3C^{44}_{22,22}}{16\sqrt{5}} + \frac{7}{192}C^{31}_{31,22} - \frac{1}{16}\sqrt{\frac{21}{5}}C^{33}_{31,22} - \frac{9}{80}\sqrt{\frac{7}{2}}C^{33}_{33,22},$$

$$C^{2011,1}_{20,2211} = -\frac{7}{64}\sqrt{3}C^{62}_{00,22} + \frac{35C^{51}_{11,22}}{192\sqrt{3}} - \frac{7C^{42}_{20,22}}{192\sqrt{3}} - \frac{7C^{40}_{22,22}}{192\sqrt{3}} + \frac{1}{48}\sqrt{\frac{7}{3}}C^{42}_{22,22} + \frac{3}{16}\sqrt{\frac{3}{5}}C^{44}_{22,22} + \frac{7C^{31}_{31,22}}{192\sqrt{3}} - \frac{1}{16}\sqrt{\frac{7}{5}}C^{33}_{31,22} - \frac{3}{80}\sqrt{\frac{21}{2}}C^{33}_{33,22},$$

$$C^{2211,0}_{20,2211} = \frac{7C^{60}_{00,00}}{128\sqrt{3}} + \frac{35}{384}C^{60}_{00,20} + \frac{7C^{62}_{00,22}}{128\sqrt{5}} - \frac{7C^{51}_{11,00}}{384\sqrt{3}} + \frac{7}{384}C^{51}_{11,20} + \frac{7}{384}\sqrt{5}C^{51}_{11,22} + \frac{5C^{40}_{20,00}}{384\sqrt{3}} + \frac{25C^{40}_{20,20}}{1152} + \frac{7C^{42}_{20,22}}{1152\sqrt{5}} - \frac{7C^{42}_{22,00}}{192\sqrt{15}} - \frac{7}{576}\sqrt{5}C^{42}_{22,20} + \frac{7C^{40}_{22,22}}{1152\sqrt{5}} - \frac{1}{288}\sqrt{\frac{7}{5}}C^{42}_{22,22} - \frac{3}{160}C^{44}_{22,22} + \frac{C^{31}_{31,00}}{384\sqrt{3}} - \frac{1}{384}C^{31}_{31,20} + \frac{7C^{31}_{31,22}}{384\sqrt{5}} - \frac{1}{160}\sqrt{21}C^{33}_{31,22} + \frac{3}{320}\sqrt{7}C^{33}_{33,00} - \frac{3}{320}\sqrt{21}C^{33}_{33,20} - \frac{9}{160}\sqrt{\frac{7}{10}}C^{33}_{33,22},$$

$$C^{2211,1}_{20,2211} = \frac{7}{128}C^{60}_{00,00} + \frac{7C^{60}_{00,20}}{128\sqrt{3}} - \frac{7}{128}\sqrt{\frac{3}{5}}C^{62}_{00,22} - \frac{7}{384}C^{51}_{11,00} - \frac{7C^{51}_{11,20}}{384\sqrt{3}} + \frac{7}{384}\sqrt{\frac{5}{3}}C^{51}_{11,22} + \frac{5}{384}C^{40}_{20,00} + \frac{5C^{40}_{20,20}}{384\sqrt{3}} - \frac{7C^{42}_{20,22}}{384\sqrt{15}} - \frac{7C^{42}_{22,00}}{192\sqrt{5}} - \frac{7C^{42}_{22,20}}{192\sqrt{15}} - \frac{7C^{40}_{22,22}}{384\sqrt{15}} + \frac{1}{96}\sqrt{\frac{7}{15}}C^{42}_{22,22} + \frac{3}{160}\sqrt{3}C^{44}_{22,22} + \frac{1}{384}C^{31}_{31,00} + \frac{C^{31}_{31,20}}{384\sqrt{3}} + \frac{7C^{31}_{31,22}}{384\sqrt{15}} - \frac{1}{160}\sqrt{7}C^{33}_{31,22} + \frac{3}{320}\sqrt{21}C^{33}_{33,00} + \frac{3}{320}\sqrt{7}C^{33}_{33,20} -$$

$\frac{3}{160}\sqrt{\frac{21}{10}}C^{33}_{33,22},$

$$C^{2212,0}_{20,2212} = \frac{7}{384}\sqrt{5}C^{60}_{00,00} + \frac{35}{384}\sqrt{\frac{5}{3}}C^{60}_{00,20} - \frac{7C^{62}_{00,22}}{128\sqrt{3}} - \frac{7\sqrt{5}C^{51}_{11,00}}{1152} + \frac{7}{384}\sqrt{\frac{5}{3}}C^{51}_{11,20} - \frac{35C^{51}_{11,22}}{384\sqrt{3}} + \frac{5\sqrt{5}C^{40}_{20,00}}{1152} + \frac{25\sqrt{\frac{5}{3}}C^{40}_{20,20}}{1152} - \frac{7C^{42}_{20,22}}{1152\sqrt{3}} - \frac{7}{576}C^{42}_{22,00} - \frac{35C^{42}_{22,20}}{576\sqrt{3}} - \frac{7C^{40}_{22,22}}{1152\sqrt{3}} + \frac{1}{288}\sqrt{\frac{7}{3}}C^{42}_{22,22} + \frac{1}{32}\sqrt{\frac{3}{5}}C^{44}_{22,22} + \frac{\sqrt{5}C^{31}_{31,00}}{1152} - \frac{1}{384}\sqrt{\frac{5}{3}}C^{31}_{31,20} - \frac{7C^{31}_{31,22}}{384\sqrt{3}} + \frac{1}{32}\sqrt{\frac{7}{5}}C^{33}_{31,22} + \frac{1}{64}\sqrt{\frac{21}{5}}C^{33}_{33,00} - \frac{3}{64}\sqrt{\frac{7}{5}}C^{33}_{33,20} + \frac{3}{160}\sqrt{\frac{21}{2}}C^{33}_{33,22},$$

$$C^{2212,1}_{20,2212} = \frac{7}{128}\sqrt{\frac{5}{3}}C^{60}_{00,00} + \frac{7}{384}\sqrt{5}C^{60}_{00,20} + \frac{7}{128}C^{62}_{00,22} - \frac{7}{384}\sqrt{\frac{5}{3}}C^{51}_{11,00} - \frac{7\sqrt{5}C^{51}_{11,20}}{1152} - \frac{35C^{51}_{11,22}}{1152} + \frac{5}{384}\sqrt{\frac{5}{3}}C^{40}_{20,00} + \frac{5\sqrt{5}C^{40}_{20,20}}{1152} + \frac{7C^{42}_{20,22}}{1152} - \frac{7C^{42}_{22,00}}{192\sqrt{3}} - \frac{7}{576}C^{42}_{22,20} + \frac{7C^{40}_{22,22}}{1152} - \frac{1}{288}\sqrt{7}C^{42}_{22,22} - \frac{3C^{44}_{22,22}}{32\sqrt{5}} + \frac{1}{384}\sqrt{\frac{5}{3}}C^{31}_{31,00} + \frac{\sqrt{5}C^{31}_{31,20}}{1152} - \frac{7C^{31}_{31,22}}{1152} + \frac{1}{32}\sqrt{\frac{7}{15}}C^{33}_{31,22} + \frac{3}{64}\sqrt{\frac{7}{5}}C^{33}_{33,00} + \frac{1}{64}\sqrt{\frac{21}{5}}C^{33}_{33,20} + \frac{3}{160}\sqrt{\frac{7}{2}}C^{33}_{33,22},$$

$$C^{2213,0}_{20,2213} = \frac{7}{384}\sqrt{7}C^{60}_{00,00} + \frac{35}{384}\sqrt{\frac{7}{3}}C^{60}_{00,20} + \frac{1}{64}\sqrt{\frac{7}{15}}C^{62}_{00,22} - \frac{7\sqrt{7}C^{51}_{11,00}}{1152} + \frac{7}{384}\sqrt{\frac{7}{3}}C^{51}_{11,20} + \frac{1}{192}\sqrt{\frac{35}{3}}C^{51}_{11,22} + \frac{5\sqrt{7}C^{40}_{20,00}}{1152} + \frac{25\sqrt{\frac{7}{3}}C^{40}_{20,20}}{1152} + \frac{1}{576}\sqrt{\frac{7}{15}}C^{42}_{20,22} - \frac{7}{576}\sqrt{\frac{7}{5}}C^{42}_{22,00} - \frac{7}{576}\sqrt{\frac{35}{3}}C^{42}_{22,20} + \frac{1}{576}\sqrt{\frac{7}{15}}C^{40}_{22,22} - \frac{C^{42}_{22,22}}{144\sqrt{15}} - \frac{1}{80}\sqrt{\frac{3}{7}}C^{44}_{22,22} + \frac{\sqrt{7}C^{31}_{31,00}}{1152} - \frac{1}{384}\sqrt{\frac{7}{3}}C^{31}_{31,20} + \frac{1}{192}\sqrt{\frac{7}{15}}C^{31}_{31,22} - \frac{1}{80}C^{33}_{31,22} + \frac{7}{320}\sqrt{3}C^{33}_{33,00} - \frac{21}{320}C^{33}_{33,20} - \frac{3}{80}\sqrt{\frac{3}{10}}C^{33}_{33,22},$$

$$C^{2213,1}_{20,2213} = \frac{7}{128}\sqrt{\frac{7}{3}}C^{60}_{00,00} + \frac{7}{384}\sqrt{7}C^{60}_{00,20} - \frac{1}{64}\sqrt{\frac{7}{5}}C^{62}_{00,22} - \frac{7}{384}\sqrt{\frac{7}{3}}C^{51}_{11,00} - \frac{7\sqrt{7}C^{51}_{11,20}}{1152} + \frac{1}{576}\sqrt{35}C^{51}_{11,22} + \frac{5}{384}\sqrt{\frac{7}{3}}C^{40}_{20,00} + \frac{5\sqrt{7}C^{40}_{20,20}}{1152} - \frac{1}{576}\sqrt{\frac{7}{5}}C^{42}_{20,22} - \frac{7}{192}\sqrt{\frac{7}{15}}C^{42}_{22,00} - \frac{7}{576}\sqrt{\frac{7}{5}}C^{42}_{22,20} - \frac{1}{576}\sqrt{\frac{7}{5}}C^{40}_{22,22} + \frac{C^{42}_{22,22}}{144\sqrt{5}} + \frac{3C^{44}_{22,22}}{80\sqrt{7}} + \frac{1}{384}\sqrt{\frac{7}{3}}C^{31}_{31,00} + \frac{\sqrt{7}C^{31}_{31,20}}{1152} + \frac{1}{576}\sqrt{\frac{7}{5}}C^{31}_{31,22} - \frac{C^{33}_{31,22}}{80\sqrt{3}} + \frac{21}{320}C^{33}_{33,00} + \frac{7}{320}\sqrt{3}C^{33}_{33,20} - \frac{3C^{33}_{33,22}}{80\sqrt{10}},$$

$$C^{1101,0}_{20,3101} = \frac{21}{64}C^{60}_{00,00} + \frac{7}{64}\sqrt{3}C^{60}_{00,20} + \frac{35}{192}C^{51}_{11,00} - \frac{7C^{51}_{11,20}}{64\sqrt{3}} + \frac{5}{64}C^{40}_{20,00} + \frac{5C^{40}_{20,20}}{64\sqrt{3}} - \frac{7C^{42}_{22,00}}{32\sqrt{5}} - \frac{7C^{42}_{22,20}}{32\sqrt{15}} - \frac{5}{192}C^{31}_{31,00} + \frac{C^{31}_{31,20}}{64\sqrt{3}} - \frac{3}{32}\sqrt{21}C^{33}_{33,00} + \frac{9}{160}\sqrt{7}C^{33}_{33,20},$$

$$C^{1101,1}_{20,3101} = -\frac{7}{64}\sqrt{3}C^{60}_{00,00} + \frac{21}{64}C^{60}_{00,20} + \frac{7C^{51}_{11,00}}{64\sqrt{3}} - \frac{7}{64}C^{51}_{11,20} - \frac{5C^{40}_{20,00}}{64\sqrt{3}} + \frac{5}{64}C^{40}_{20,20} + \frac{7C^{42}_{22,00}}{32\sqrt{15}} - \frac{7C^{42}_{22,20}}{32\sqrt{5}} - \frac{C^{31}_{31,00}}{64\sqrt{3}} + \frac{1}{64}C^{31}_{31,20} - \frac{9}{160}\sqrt{7}C^{33}_{33,00} + \frac{9}{160}\sqrt{21}C^{33}_{33,20},$$

$$C^{1110,0}_{20,3110} = -\frac{7C^{60}_{00,00}}{64\sqrt{3}} - \frac{35}{192}C^{60}_{00,20} - \frac{7C^{62}_{00,22}}{32\sqrt{5}} + \frac{7C^{51}_{11,00}}{192\sqrt{3}} - \frac{7}{192}C^{51}_{11,20} - \frac{7}{96}\sqrt{5}C^{51}_{11,22} - \frac{5C^{40}_{20,00}}{192\sqrt{3}} - \frac{25}{576}C^{40}_{20,20} - \frac{7C^{42}_{20,22}}{288\sqrt{5}} + \frac{7C^{42}_{22,00}}{96\sqrt{15}} + \frac{7}{288}\sqrt{5}C^{42}_{22,20} - \frac{7C^{40}_{22,22}}{288\sqrt{5}} + \frac{1}{72}\sqrt{\frac{7}{5}}C^{42}_{22,22} + \frac{3}{40}C^{44}_{22,22} - \frac{C^{31}_{31,00}}{192\sqrt{3}} + \frac{1}{192}C^{31}_{31,20} - \frac{7C^{31}_{31,22}}{96\sqrt{5}} + \frac{1}{40}\sqrt{21}C^{33}_{31,22} - \frac{3}{160}\sqrt{7}C^{33}_{33,00} + \frac{3}{160}\sqrt{21}C^{33}_{33,20} + \frac{9}{40}\sqrt{\frac{7}{10}}C^{33}_{33,22},$$

$$C^{1110,1}_{20,3110} = -\frac{7}{64}C^{60}_{00,00} - \frac{7C^{60}_{00,20}}{64\sqrt{3}} + \frac{7}{32}\sqrt{\frac{3}{5}}C^{62}_{00,22} + \frac{7}{192}C^{51}_{11,00} + \frac{7C^{51}_{11,20}}{192\sqrt{3}} - \frac{7}{96}\sqrt{\frac{5}{3}}C^{51}_{11,22} - \frac{5}{192}C^{40}_{20,00} - \frac{5C^{40}_{20,20}}{192\sqrt{3}} + \frac{7C^{42}_{20,22}}{96\sqrt{15}} + \frac{7C^{42}_{22,00}}{96\sqrt{5}} + \frac{7C^{42}_{22,20}}{96\sqrt{15}} + \frac{7C^{40}_{22,22}}{96\sqrt{15}} - \frac{1}{24}\sqrt{\frac{7}{15}}C^{42}_{22,22} - \frac{3}{40}\sqrt{3}C^{44}_{22,22} - \frac{1}{192}C^{31}_{31,00} - \frac{C^{31}_{31,20}}{192\sqrt{3}} - \frac{7C^{31}_{31,22}}{96\sqrt{15}} + \frac{1}{40}\sqrt{7}C^{33}_{31,22} - \frac{3}{160}\sqrt{21}C^{33}_{33,00} - \frac{3}{160}\sqrt{7}C^{33}_{33,20} + \frac{3}{40}\sqrt{\frac{21}{10}}C^{33}_{33,22},$$

$$C^{1111,0}_{20,3111} = -\frac{7}{64}C^{60}_{00,00} - \frac{35C^{60}_{00,20}}{64\sqrt{3}} + \frac{7}{64}\sqrt{\frac{3}{5}}C^{62}_{00,22} + \frac{7}{192}C^{51}_{11,00} - \frac{7C^{51}_{11,20}}{64\sqrt{3}} + \frac{7}{64}\sqrt{\frac{5}{3}}C^{51}_{11,22} - \frac{5}{192}C^{40}_{20,00} - \frac{25C^{40}_{20,20}}{192\sqrt{3}} + \frac{7C^{42}_{20,22}}{192\sqrt{15}} + \frac{7C^{42}_{22,00}}{96\sqrt{5}} + \frac{7}{96}\sqrt{\frac{5}{3}}C^{42}_{22,20} + \frac{7C^{40}_{22,22}}{192\sqrt{15}} - \frac{1}{48}\sqrt{\frac{7}{15}}C^{42}_{22,22} - \frac{3}{80}\sqrt{3}C^{44}_{22,22} - \frac{1}{192}C^{31}_{31,00} + \frac{C^{31}_{31,20}}{64\sqrt{3}} + \frac{7C^{31}_{31,22}}{64\sqrt{15}} - \frac{3}{80}\sqrt{7}C^{33}_{31,22} - \frac{3}{160}\sqrt{21}C^{33}_{33,00} + \frac{9}{160}\sqrt{7}C^{33}_{33,20} - \frac{9}{80}\sqrt{\frac{21}{10}}C^{33}_{33,22},$$

$$C^{1111,1}_{20,3111} = -\frac{7}{64}\sqrt{3}C^{60}_{00,00} - \frac{7}{64}C^{60}_{00,20} - \frac{21C^{62}_{00,22}}{64\sqrt{5}} + \frac{7C^{51}_{11,00}}{64\sqrt{3}} + \frac{7}{192}C^{51}_{11,20} + \frac{7}{192}\sqrt{5}C^{51}_{11,22} - \frac{5C^{40}_{20,00}}{64\sqrt{3}} - \frac{5}{192}C^{40}_{20,20} - \frac{7C^{42}_{20,22}}{192\sqrt{5}} + \frac{7C^{42}_{22,00}}{32\sqrt{15}} + \frac{7C^{42}_{22,20}}{96\sqrt{5}} - \frac{7C^{40}_{22,22}}{192\sqrt{5}} + \frac{1}{48}\sqrt{\frac{7}{5}}C^{42}_{22,22} + \frac{9}{80}C^{44}_{22,22} - \frac{C^{31}_{31,00}}{64\sqrt{3}} - \frac{1}{192}C^{31}_{31,20} + \frac{7C^{31}_{31,22}}{192\sqrt{5}} - \frac{1}{80}\sqrt{21}C^{33}_{31,22} - \frac{9}{160}\sqrt{7}C^{33}_{33,00} - \frac{3}{160}\sqrt{21}C^{33}_{33,20} - \frac{9}{80}\sqrt{\frac{7}{10}}C^{33}_{33,22},$$

$$C^{1112,0}_{20,3112} = -\frac{7}{64}\sqrt{\frac{5}{3}}C^{60}_{00,00} - \frac{35}{192}\sqrt{5}C^{60}_{00,20} - \frac{7}{320}C^{62}_{00,22} + \frac{7}{192}\sqrt{\frac{5}{3}}C^{51}_{11,00} - \frac{7}{192}\sqrt{5}C^{51}_{11,20} - \frac{7}{192}C^{51}_{11,22} - \frac{5}{192}\sqrt{\frac{5}{3}}C^{40}_{20,00} - \frac{25}{576}\sqrt{5}C^{40}_{20,20} - \frac{7C^{42}_{20,22}}{2880} + \frac{7C^{42}_{22,00}}{96\sqrt{3}} + \frac{35}{288}C^{42}_{22,20} - \frac{7C^{40}_{22,22}}{2880} + \frac{1}{720}\sqrt{7}C^{42}_{22,22} + \frac{3C^{44}_{22,22}}{80\sqrt{5}} - \frac{1}{192}\sqrt{\frac{5}{3}}C^{31}_{31,00} + \frac{1}{192}\sqrt{5}C^{31}_{31,20} - \frac{7}{960}C^{31}_{31,22} + \frac{1}{80}\sqrt{\frac{21}{5}}C^{33}_{31,22} - \frac{3}{32}\sqrt{\frac{7}{5}}C^{33}_{33,00} + \frac{3}{32}\sqrt{\frac{21}{5}}C^{33}_{33,20} + \frac{9}{400}\sqrt{\frac{7}{2}}C^{33}_{33,22},$$

$$C^{1112,1}_{20,3112} = -\frac{7}{64}\sqrt{5}C^{60}_{00,00} - \frac{7}{64}\sqrt{\frac{5}{3}}C^{60}_{00,20} + \frac{7}{320}\sqrt{3}C^{62}_{00,22} + \frac{7}{192}\sqrt{5}C^{51}_{11,00} + \frac{7}{192}\sqrt{\frac{5}{3}}C^{51}_{11,20} - \frac{7C^{51}_{11,22}}{192\sqrt{3}} - \frac{5}{192}\sqrt{5}C^{40}_{20,00} - \frac{5}{192}\sqrt{\frac{5}{3}}C^{40}_{20,20} + \frac{7C^{42}_{20,22}}{960\sqrt{3}} + \frac{7}{96}C^{42}_{22,00} + \frac{7C^{42}_{22,20}}{96\sqrt{3}} + \frac{7C^{40}_{22,22}}{960\sqrt{3}} - \frac{1}{240}\sqrt{\frac{7}{3}}C^{42}_{22,22} - \frac{3}{80}\sqrt{\frac{3}{5}}C^{44}_{22,22} - \frac{1}{192}\sqrt{5}C^{31}_{31,00} - \frac{1}{192}\sqrt{\frac{5}{3}}C^{31}_{31,20} - \frac{7C^{31}_{31,22}}{960\sqrt{3}} + \frac{1}{80}\sqrt{\frac{7}{5}}C^{33}_{31,22} - \frac{3}{32}\sqrt{\frac{21}{5}}C^{33}_{33,00} - \frac{3}{32}\sqrt{\frac{7}{5}}C^{33}_{33,20} + \frac{3}{400}\sqrt{\frac{21}{2}}C^{33}_{33,22},$$

$$C^{1112,0}_{20,3312} = -\frac{1}{32}\sqrt{\frac{21}{5}}C^{62}_{00,22} - \frac{1}{32}\sqrt{\frac{35}{3}}C^{51}_{11,22} - \frac{1}{96}\sqrt{\frac{7}{15}}C^{42}_{20,22} - \frac{1}{96}\sqrt{\frac{7}{15}}C^{40}_{22,22} + \frac{C^{42}_{22,22}}{24\sqrt{15}} + \frac{3}{40}\sqrt{\frac{3}{7}}C^{44}_{22,22} - \frac{1}{32}\sqrt{\frac{7}{15}}C^{31}_{31,22} + \frac{3}{40}C^{33}_{31,22} + \frac{9}{40}\sqrt{\frac{3}{10}}C^{33}_{33,22},$$

$$C^{1112,1}_{20,3312} = \frac{3}{32}\sqrt{\frac{7}{5}}C^{62}_{00,22} - \frac{1}{96}\sqrt{35}C^{51}_{11,22} + \frac{1}{96}\sqrt{\frac{7}{5}}C^{42}_{20,22} + \frac{1}{96}\sqrt{\frac{7}{5}}C^{40}_{22,22} - \frac{C^{42}_{22,22}}{24\sqrt{5}} - \frac{9C^{44}_{22,22}}{40\sqrt{7}} - \frac{1}{96}\sqrt{\frac{7}{5}}C^{31}_{31,22} + \frac{1}{40}\sqrt{3}C^{33}_{31,22} + \frac{9C^{33}_{33,22}}{40\sqrt{10}},$$

$$C^{0000,0}_{20,4000} = -\frac{21}{256}C^{60}_{00,00} - \frac{7}{256}\sqrt{3}C^{60}_{00,20} - \frac{35}{768}C^{51}_{11,00} + \frac{7C^{51}_{11,20}}{256\sqrt{3}} - \frac{5}{256}C^{40}_{20,00} - \frac{5C^{40}_{20,20}}{256\sqrt{3}} + \frac{7C^{42}_{22,00}}{128\sqrt{5}} + \frac{7C^{42}_{22,20}}{128\sqrt{15}} + \frac{5}{768}C^{31}_{31,00} - \frac{C^{31}_{31,20}}{256\sqrt{3}} + \frac{3}{128}\sqrt{21}C^{33}_{33,00} - \frac{9}{640}\sqrt{7}C^{33}_{33,20},$$

$$C^{0000,1}_{20,4000} = \frac{7}{256}\sqrt{3}C^{60}_{00,00} - \frac{21}{256}C^{60}_{00,20} - \frac{7C^{51}_{11,00}}{256\sqrt{3}} + \frac{7}{256}C^{51}_{11,20} + \frac{5C^{40}_{20,00}}{256\sqrt{3}} - \frac{5}{256}C^{40}_{20,20} - \frac{7C^{42}_{22,00}}{128\sqrt{15}} + \frac{7C^{42}_{22,20}}{128\sqrt{5}} + \frac{C^{31}_{31,00}}{256\sqrt{3}} - \frac{1}{256}C^{31}_{31,20} + \frac{9}{640}\sqrt{7}C^{33}_{33,00} - \frac{9}{640}\sqrt{21}C^{33}_{33,20},$$

$$C^{0011,0}_{20,4011} = \frac{7}{256}\sqrt{3}C^{60}_{00,00} + \frac{35}{256}C^{60}_{00,20} - \frac{7C^{51}_{11,00}}{256\sqrt{3}} + \frac{7}{256}C^{51}_{11,20} + \frac{5C^{40}_{20,00}}{256\sqrt{3}} + \frac{25}{768}C^{40}_{20,20} - \frac{7C^{42}_{22,00}}{128\sqrt{15}} - \frac{7}{384}\sqrt{5}C^{42}_{22,20} + \frac{C^{31}_{31,00}}{256\sqrt{3}} - \frac{1}{256}C^{31}_{31,20} + \frac{9}{640}\sqrt{7}C^{33}_{33,00} - \frac{9}{640}\sqrt{21}C^{33}_{33,20},$$

$$C^{0011,1}_{20,4011} = \frac{21}{256}C^{60}_{00,00} + \frac{7}{256}\sqrt{3}C^{60}_{00,20} - \frac{7}{256}C^{51}_{11,00} - \frac{7C^{51}_{11,20}}{256\sqrt{3}} + \frac{5}{256}C^{40}_{20,00} + \frac{5C^{40}_{20,20}}{256\sqrt{3}} - \frac{7C^{42}_{22,00}}{128\sqrt{5}} - \frac{7C^{42}_{22,20}}{128\sqrt{15}} + \frac{1}{256}C^{31}_{31,00} + \frac{C^{31}_{31,20}}{256\sqrt{3}} + \frac{9}{640}\sqrt{21}C^{33}_{33,00} + \frac{9}{640}\sqrt{7}C^{33}_{33,20},$$

$$C^{0011,0}_{20,4211} = \frac{3}{64}C^{62}_{00,22} + \frac{5}{64}C^{51}_{11,22} + \frac{1}{192}C^{42}_{20,22} + \frac{1}{192}C^{40}_{22,22} - \frac{C^{42}_{22,22}}{48\sqrt{7}} - \frac{9C^{44}_{22,22}}{112\sqrt{5}} + \frac{1}{64}C^{31}_{31,22} -$$

$$\frac{3}{16}\sqrt{\frac{3}{35}}C^{33}_{31,22} - \frac{27C^{33}_{33,22}}{80\sqrt{14}},$$

$$C^{0011,1}_{20,4211} = -\frac{3}{64}\sqrt{3}C^{62}_{00,22} + \frac{5C^{51}_{11,22}}{64\sqrt{3}} - \frac{C^{42}_{20,22}}{64\sqrt{3}} - \frac{C^{40}_{22,22}}{64\sqrt{3}} + \frac{C^{42}_{22,22}}{16\sqrt{21}} + \frac{9}{112}\sqrt{\frac{3}{5}}C^{44}_{22,22} + \frac{C^{31}_{31,22}}{64\sqrt{3}} - \frac{3C^{33}_{31,22}}{16\sqrt{35}} - \frac{9}{80}\sqrt{\frac{3}{14}}C^{33}_{33,22},$$

$$C^{2011,0}_{22,2011} = \frac{7}{128}C^{62}_{00,22} - \frac{7}{384}C^{51}_{11,22} + \frac{9}{128}\sqrt{\frac{21}{5}}C^{53}_{11,22} + \frac{7C^{42}_{20,22}}{1152} - \frac{17C^{40}_{22,22}}{1152} - \frac{5}{576}\sqrt{7}C^{42}_{22,22} + \frac{3C^{44}_{22,22}}{32\sqrt{5}} - \frac{23}{384}C^{31}_{31,22} + \frac{1}{128}\sqrt{\frac{21}{5}}C^{33}_{31,22} - \frac{9}{160}\sqrt{\frac{7}{2}}C^{33}_{33,22},$$

$$C^{2011,1}_{22,2011} = -\frac{7}{128}\sqrt{3}C^{62}_{00,22} - \frac{7C^{51}_{11,22}}{384\sqrt{3}} + \frac{9}{128}\sqrt{\frac{7}{5}}C^{53}_{11,22} - \frac{7C^{42}_{20,22}}{384\sqrt{3}} + \frac{17C^{40}_{22,22}}{384\sqrt{3}} + \frac{5}{192}\sqrt{\frac{7}{3}}C^{42}_{22,22} - \frac{3}{32}\sqrt{\frac{3}{5}}C^{44}_{22,22} - \frac{23C^{31}_{31,22}}{384\sqrt{3}} + \frac{1}{128}\sqrt{\frac{7}{5}}C^{33}_{31,22} - \frac{3}{160}\sqrt{\frac{21}{2}}C^{33}_{33,22},$$

$$C^{2000,0}_{22,2202} = -\frac{7}{64}\sqrt{5}C^{60}_{00,00} - \frac{7}{64}\sqrt{\frac{5}{3}}C^{60}_{00,20} - \frac{35}{576}\sqrt{5}C^{51}_{11,00} + \frac{7}{192}\sqrt{\frac{5}{3}}C^{51}_{11,20} + \frac{7}{192}\sqrt{5}C^{40}_{20,00} + \frac{7}{192}\sqrt{\frac{5}{3}}C^{40}_{20,20} - \frac{7}{192}C^{42}_{22,00} - \frac{7C^{42}_{22,20}}{192\sqrt{3}} + \frac{35}{576}\sqrt{5}C^{31}_{31,00} - \frac{7}{192}\sqrt{\frac{5}{3}}C^{31}_{31,20} - \frac{1}{64}\sqrt{105}C^{33}_{33,00} + \frac{3}{64}\sqrt{\frac{7}{5}}C^{33}_{33,20},$$

$$C^{2000,1}_{22,2202} = \frac{7}{64}\sqrt{\frac{5}{3}}C^{60}_{00,00} - \frac{7}{64}\sqrt{5}C^{60}_{00,20} - \frac{7}{192}\sqrt{\frac{5}{3}}C^{51}_{11,00} + \frac{7}{192}\sqrt{5}C^{51}_{11,20} - \frac{7}{192}\sqrt{\frac{5}{3}}C^{40}_{20,00} + \frac{7}{192}\sqrt{5}C^{40}_{20,20} + \frac{7C^{42}_{22,00}}{192\sqrt{3}} - \frac{7}{192}C^{42}_{22,20} + \frac{7}{192}\sqrt{\frac{5}{3}}C^{31}_{31,00} - \frac{7}{192}\sqrt{5}C^{31}_{31,20} - \frac{3}{64}\sqrt{\frac{7}{5}}C^{33}_{33,00} + \frac{3}{64}\sqrt{\frac{21}{5}}C^{33}_{33,20},$$

$$C^{2202,0}_{22,2202} = -\frac{1}{64}\sqrt{35}C^{60}_{00,00} - \frac{1}{64}\sqrt{\frac{35}{3}}C^{60}_{00,20} - \frac{5}{576}\sqrt{35}C^{51}_{11,00} + \frac{1}{192}\sqrt{\frac{35}{3}}C^{51}_{11,20} + \frac{1}{192}\sqrt{35}C^{40}_{20,00} + \frac{1}{192}\sqrt{\frac{35}{3}}C^{40}_{20,20} - \frac{1}{192}\sqrt{7}C^{42}_{22,00} - \frac{1}{192}\sqrt{\frac{7}{3}}C^{42}_{22,20} + \frac{5}{576}\sqrt{35}C^{31}_{31,00} - \frac{1}{192}\sqrt{\frac{35}{3}}C^{31}_{31,20} - \frac{1}{64}\sqrt{15}C^{33}_{33,00} + \frac{3C^{33}_{33,20}}{64\sqrt{5}},$$

$$C^{2202,1}_{22,2202} = \frac{1}{64}\sqrt{\frac{35}{3}}C^{60}_{00,00} - \frac{1}{64}\sqrt{35}C^{60}_{00,20} - \frac{1}{192}\sqrt{\frac{35}{3}}C^{51}_{11,00} + \frac{1}{192}\sqrt{35}C^{51}_{11,20} - \frac{1}{192}\sqrt{\frac{35}{3}}C^{40}_{20,00} + \frac{1}{192}\sqrt{35}C^{40}_{20,20} + \frac{1}{192}\sqrt{\frac{7}{3}}C^{42}_{22,00} - \frac{1}{192}\sqrt{7}C^{42}_{22,20} + \frac{1}{192}\sqrt{\frac{35}{3}}C^{31}_{31,00} - \frac{1}{192}\sqrt{35}C^{31}_{31,20} - \frac{3C^{33}_{33,00}}{64\sqrt{5}} + \frac{3}{64}\sqrt{\frac{3}{5}}C^{33}_{33,20},$$

$$C^{2011,0}_{22,2211} = \frac{7C^{60}_{00,00}}{64\sqrt{3}} + \frac{35}{192}C^{60}_{00,20} + \frac{7C^{62}_{00,22}}{64\sqrt{5}} - \frac{7C^{51}_{11,00}}{192\sqrt{3}} + \frac{7}{192}C^{51}_{11,20} + \frac{7C^{51}_{11,22}}{96\sqrt{5}} + \frac{9}{640}\sqrt{21}C^{53}_{11,22} - \frac{7C^{40}_{20,00}}{192\sqrt{3}} - \frac{35}{576}C^{40}_{20,20} - \frac{7C^{42}_{20,22}}{288\sqrt{5}} + \frac{7C^{42}_{22,00}}{192\sqrt{15}} + \frac{7}{576}\sqrt{5}C^{42}_{22,20} - \frac{7}{576}\sqrt{5}C^{40}_{22,22} + \frac{7}{288}\sqrt{\frac{7}{5}}C^{42}_{22,22} + \frac{7C^{31}_{31,00}}{192\sqrt{3}} - \frac{7}{192}C^{31}_{31,20} - \frac{7C^{31}_{31,22}}{96\sqrt{5}} - \frac{9}{640}\sqrt{21}C^{33}_{31,22} - \frac{3}{320}\sqrt{7}C^{33}_{33,00} + \frac{3}{320}\sqrt{21}C^{33}_{33,20} + \frac{9}{40}\sqrt{\frac{7}{10}}C^{33}_{33,22},$$

$$C^{2011,1}_{22,2211} = \frac{7}{64}C^{60}_{00,00} + \frac{7C^{60}_{00,20}}{64\sqrt{3}} - \frac{7}{64}\sqrt{\frac{3}{5}}C^{62}_{00,22} - \frac{7}{192}C^{51}_{11,00} - \frac{7C^{51}_{11,20}}{192\sqrt{3}} + \frac{7C^{51}_{11,22}}{96\sqrt{15}} + \frac{9}{640}\sqrt{7}C^{53}_{11,22} - \frac{7}{192}C^{40}_{20,00} - \frac{7C^{40}_{20,20}}{192\sqrt{3}} + \frac{7C^{42}_{20,22}}{96\sqrt{15}} + \frac{7C^{42}_{22,00}}{192\sqrt{5}} + \frac{7C^{42}_{22,20}}{192\sqrt{15}} + \frac{7}{192}\sqrt{\frac{5}{3}}C^{40}_{22,22} - \frac{7}{96}\sqrt{\frac{7}{15}}C^{42}_{22,22} + \frac{7}{192}C^{31}_{31,00} + \frac{7C^{31}_{31,20}}{192\sqrt{3}} - \frac{7C^{31}_{31,22}}{96\sqrt{15}} - \frac{9}{640}\sqrt{7}C^{33}_{31,22} - \frac{3}{320}\sqrt{21}C^{33}_{33,00} - \frac{3}{320}\sqrt{7}C^{33}_{33,20} + \frac{3}{40}\sqrt{\frac{21}{10}}C^{33}_{33,22},$$

$$C^{2211,0}_{22,2211} = \frac{7C^{60}_{00,00}}{128\sqrt{15}} + \frac{7}{384}\sqrt{5}C^{60}_{00,20} + \frac{21}{640}C^{62}_{00,22} - \frac{7C^{51}_{11,00}}{384\sqrt{15}} + \frac{7C^{51}_{11,20}}{384\sqrt{5}} + \frac{63}{640}C^{51}_{11,22} -$$

$\frac{9}{320}\sqrt{\frac{21}{5}}C^{53}_{11,22} - \frac{7C^{40}_{20,00}}{384\sqrt{15}} - \frac{7\sqrt{5}C^{40}_{20,20}}{1152} - \frac{21}{640}C^{42}_{20,22} + \frac{7C^{42}_{22,00}}{1920\sqrt{3}} + \frac{7C^{42}_{22,20}}{1152} + \frac{67C^{40}_{22,22}}{1920} - \frac{1}{960}\sqrt{7}C^{42}_{22,22} + \frac{3C^{44}_{22,22}}{80\sqrt{5}} + \frac{7C^{31}_{31,00}}{384\sqrt{15}} - \frac{7C^{31}_{31,20}}{384\sqrt{5}} - \frac{13}{128}C^{31}_{31,22} + \frac{1}{32}\sqrt{\frac{21}{5}}C^{33}_{31,22} - \frac{3}{640}\sqrt{\frac{7}{5}}C^{33}_{33,00} + \frac{3}{640}\sqrt{\frac{21}{5}}C^{33}_{33,20}$,

$C^{2211,1}_{22,2211} = \frac{7C^{60}_{00,00}}{128\sqrt{5}} + \frac{7C^{60}_{00,20}}{128\sqrt{15}} - \frac{21}{640}\sqrt{3}C^{62}_{00,22} - \frac{7C^{51}_{11,00}}{384\sqrt{5}} - \frac{7C^{51}_{11,20}}{384\sqrt{15}} + \frac{21}{640}\sqrt{3}C^{51}_{11,22} - \frac{9}{320}\sqrt{\frac{7}{5}}C^{53}_{11,22} - \frac{7C^{40}_{20,00}}{384\sqrt{5}} - \frac{7C^{40}_{20,20}}{384\sqrt{15}} + \frac{21}{640}\sqrt{3}C^{42}_{20,22} + \frac{7C^{42}_{22,00}}{1920} + \frac{7C^{42}_{22,20}}{1920\sqrt{3}} - \frac{67C^{40}_{22,22}}{640\sqrt{3}} + \frac{1}{320}\sqrt{\frac{7}{3}}C^{42}_{22,22} - \frac{3}{80}\sqrt{\frac{3}{5}}C^{44}_{22,22} + \frac{7C^{31}_{31,00}}{384\sqrt{5}} + \frac{7C^{31}_{31,20}}{384\sqrt{15}} - \frac{13C^{31}_{31,22}}{128\sqrt{3}} + \frac{1}{32}\sqrt{\frac{7}{5}}C^{33}_{31,22} - \frac{3}{640}\sqrt{\frac{21}{5}}C^{33}_{33,00} - \frac{3}{640}\sqrt{\frac{7}{5}}C^{33}_{33,20}$,

$C^{2011,0}_{22,2212} = -\frac{7}{192}\sqrt{5}C^{60}_{00,00} - \frac{35}{192}\sqrt{\frac{5}{3}}C^{60}_{00,20} + \frac{7C^{62}_{00,22}}{64\sqrt{3}} + \frac{7}{576}\sqrt{5}C^{51}_{11,00} - \frac{7}{192}\sqrt{\frac{5}{3}}C^{51}_{11,20} + \frac{7C^{51}_{11,22}}{96\sqrt{3}} + \frac{9}{128}\sqrt{\frac{7}{5}}C^{53}_{11,22} + \frac{7}{576}\sqrt{5}C^{40}_{20,00} + \frac{35}{576}\sqrt{\frac{5}{3}}C^{40}_{20,20} - \frac{7C^{42}_{20,22}}{288\sqrt{3}} - \frac{7}{576}C^{42}_{22,00} - \frac{35C^{42}_{22,20}}{576\sqrt{3}} - \frac{35C^{40}_{22,22}}{576\sqrt{3}} + \frac{7}{288}\sqrt{\frac{7}{3}}C^{42}_{22,22} - \frac{7}{576}\sqrt{5}C^{31}_{31,00} + \frac{7}{192}\sqrt{\frac{5}{3}}C^{31}_{31,20} - \frac{7C^{31}_{31,22}}{96\sqrt{3}} - \frac{9}{128}\sqrt{\frac{7}{5}}C^{33}_{31,22} + \frac{1}{64}\sqrt{\frac{21}{5}}C^{33}_{33,00} - \frac{3}{64}\sqrt{\frac{7}{5}}C^{33}_{33,20} + \frac{3}{40}\sqrt{\frac{21}{2}}C^{33}_{33,22}$,

$C^{2011,1}_{22,2212} = -\frac{7}{64}\sqrt{\frac{5}{3}}C^{60}_{00,00} - \frac{7}{192}\sqrt{5}C^{60}_{00,20} - \frac{7}{64}C^{62}_{00,22} + \frac{7}{192}\sqrt{\frac{5}{3}}C^{51}_{11,00} + \frac{7}{576}\sqrt{5}C^{51}_{11,20} + \frac{7}{288}C^{51}_{11,22} + \frac{3}{128}\sqrt{\frac{21}{5}}C^{53}_{11,22} + \frac{7}{192}\sqrt{\frac{5}{3}}C^{40}_{20,00} + \frac{7}{576}\sqrt{5}C^{40}_{20,20} + \frac{7}{288}C^{42}_{20,22} - \frac{7C^{42}_{22,00}}{192\sqrt{3}} - \frac{7}{576}C^{42}_{22,20} + \frac{35}{576}C^{40}_{22,22} - \frac{7}{288}\sqrt{7}C^{42}_{22,22} - \frac{7}{192}\sqrt{\frac{5}{3}}C^{31}_{31,00} - \frac{7}{576}\sqrt{5}C^{31}_{31,20} - \frac{7}{288}C^{31}_{31,22} - \frac{3}{128}\sqrt{\frac{21}{5}}C^{33}_{31,22} + \frac{3}{64}\sqrt{\frac{7}{5}}C^{33}_{33,00} + \frac{1}{64}\sqrt{\frac{21}{5}}C^{33}_{33,20} + \frac{3}{40}\sqrt{\frac{7}{2}}C^{33}_{33,22}$,

$C^{2211,0}_{22,2212} = \frac{7}{192}C^{60}_{00,00} + \frac{35C^{60}_{00,20}}{192\sqrt{3}} - \frac{7C^{62}_{00,22}}{64\sqrt{15}} - \frac{7}{576}C^{51}_{11,00} + \frac{7C^{51}_{11,20}}{192\sqrt{3}} - \frac{77C^{51}_{11,22}}{192\sqrt{15}} + \frac{9}{320}\sqrt{7}C^{53}_{11,22} - \frac{7}{576}C^{40}_{20,00} - \frac{35C^{40}_{20,20}}{576\sqrt{3}} + \frac{77C^{42}_{20,22}}{576\sqrt{15}} + \frac{7C^{42}_{22,00}}{576\sqrt{5}} + \frac{7}{576}\sqrt{\frac{5}{3}}C^{42}_{22,20} - \frac{11}{576}\sqrt{\frac{5}{3}}C^{40}_{22,22} - \frac{7}{288}\sqrt{\frac{7}{15}}C^{42}_{22,22} + \frac{7}{576}C^{31}_{31,00} - \frac{7C^{31}_{31,20}}{192\sqrt{3}} + \frac{59C^{31}_{31,22}}{192\sqrt{15}} - \frac{3}{320}\sqrt{7}C^{33}_{31,22} - \frac{1}{320}\sqrt{21}C^{33}_{33,00} + \frac{3}{320}\sqrt{7}C^{33}_{33,20} - \frac{3}{40}\sqrt{\frac{21}{10}}C^{33}_{33,22}$,

$C^{2211,1}_{22,2212} = \frac{7C^{60}_{00,00}}{64\sqrt{3}} + \frac{7}{192}C^{60}_{00,20} + \frac{7C^{62}_{00,22}}{64\sqrt{5}} - \frac{7C^{51}_{11,00}}{192\sqrt{3}} - \frac{7}{576}C^{51}_{11,20} - \frac{77C^{51}_{11,22}}{576\sqrt{5}} + \frac{3}{320}\sqrt{21}C^{53}_{11,22} - \frac{7C^{40}_{20,00}}{192\sqrt{3}} - \frac{7}{576}C^{40}_{20,20} - \frac{77C^{42}_{20,22}}{576\sqrt{5}} + \frac{7C^{42}_{22,00}}{192\sqrt{15}} + \frac{7C^{42}_{22,20}}{576\sqrt{5}} + \frac{11}{576}\sqrt{5}C^{40}_{22,22} + \frac{7}{288}\sqrt{\frac{7}{5}}C^{42}_{22,22} + \frac{7C^{31}_{31,00}}{192\sqrt{3}} + \frac{7}{576}C^{31}_{31,20} + \frac{59C^{31}_{31,22}}{576\sqrt{5}} - \frac{1}{320}\sqrt{21}C^{33}_{31,22} - \frac{3}{320}\sqrt{7}C^{33}_{33,00} - \frac{1}{320}\sqrt{21}C^{33}_{33,20} - \frac{3}{40}\sqrt{\frac{7}{10}}C^{33}_{33,22}$,

$C^{2212,0}_{22,2212} = \frac{1}{384}\sqrt{35}C^{60}_{00,00} + \frac{5}{384}\sqrt{\frac{35}{3}}C^{60}_{00,20} - \frac{1}{128}\sqrt{\frac{7}{3}}C^{62}_{00,22} - \frac{\sqrt{35}C^{51}_{11,00}}{1152} + \frac{1}{384}\sqrt{\frac{35}{3}}C^{51}_{11,20} - \frac{5}{384}\sqrt{\frac{7}{3}}C^{51}_{11,22} - \frac{\sqrt{35}C^{40}_{20,00}}{1152} - \frac{5\sqrt{\frac{35}{3}}C^{40}_{20,20}}{1152} + \frac{5\sqrt{\frac{7}{3}}C^{42}_{20,22}}{1152} + \frac{\sqrt{7}C^{42}_{22,00}}{1152} + \frac{5\sqrt{\frac{7}{3}}C^{42}_{22,20}}{1152} - \frac{13\sqrt{\frac{7}{3}}C^{40}_{22,22}}{1152} + \frac{17C^{42}_{22,22}}{576\sqrt{3}} - \frac{1}{16}\sqrt{\frac{3}{35}}C^{44}_{22,22} + \frac{\sqrt{35}C^{31}_{31,00}}{1152} - \frac{1}{384}\sqrt{\frac{35}{3}}C^{31}_{31,20} + \frac{11}{384}\sqrt{\frac{7}{3}}C^{31}_{31,22} - \frac{7C^{33}_{31,22}}{64\sqrt{5}} - \frac{1}{128}\sqrt{\frac{3}{5}}C^{33}_{33,00} + \frac{3C^{33}_{33,20}}{128\sqrt{5}} + \frac{3}{40}\sqrt{\frac{3}{2}}C^{33}_{33,22}$,

$C^{2212,1}_{22,2212} = \frac{1}{128}\sqrt{\frac{35}{3}}C^{60}_{00,00} + \frac{1}{384}\sqrt{35}C^{60}_{00,20} + \frac{1}{128}\sqrt{7}C^{62}_{00,22} - \frac{1}{384}\sqrt{\frac{35}{3}}C^{51}_{11,00} - \frac{\sqrt{35}C^{51}_{11,20}}{1152} -$

$$\frac{5\sqrt{7}C^{51}_{11,22}}{1152} - \frac{1}{384}\sqrt{\frac{35}{3}}C^{40}_{20,00} - \frac{\sqrt{35}C^{40}_{20,20}}{1152} - \frac{5\sqrt{7}C^{42}_{20,22}}{1152} + \frac{1}{384}\sqrt{\frac{7}{3}}C^{42}_{22,00} + \frac{\sqrt{7}C^{42}_{22,20}}{1152} + \frac{13\sqrt{7}C^{40}_{22,22}}{1152} - \frac{17}{576}C^{42}_{22,22} + \frac{3C^{44}_{22,22}}{16\sqrt{35}} + \frac{1}{384}\sqrt{\frac{35}{3}}C^{31}_{31,00} + \frac{\sqrt{35}C^{31}_{31,20}}{1152} + \frac{11\sqrt{7}C^{31}_{31,22}}{1152} - \frac{7C^{33}_{31,22}}{64\sqrt{15}} - \frac{3C^{33}_{33,00}}{128\sqrt{5}} - \frac{1}{128}\sqrt{\frac{3}{5}}C^{33}_{33,20} + \frac{3C^{33}_{33,22}}{40\sqrt{2}},$$

$$C^{2011,0}_{22,2213} = \frac{7}{192}\sqrt{7}C^{60}_{00,00} + \frac{35}{192}\sqrt{\frac{7}{3}}C^{60}_{00,20} + \frac{1}{32}\sqrt{\frac{7}{15}}C^{62}_{00,22} - \frac{7}{576}\sqrt{7}C^{51}_{11,00} + \frac{7}{192}\sqrt{\frac{7}{3}}C^{51}_{11,20} + \frac{1}{48}\sqrt{\frac{7}{15}}C^{51}_{11,22} + \frac{9}{320}C^{53}_{11,22} - \frac{7}{576}\sqrt{7}C^{40}_{20,00} - \frac{35}{576}\sqrt{\frac{7}{3}}C^{40}_{20,20} - \frac{1}{144}\sqrt{\frac{7}{15}}C^{42}_{20,22} + \frac{7}{576}\sqrt{\frac{7}{5}}C^{42}_{22,00} + \frac{7}{576}\sqrt{\frac{35}{3}}C^{42}_{22,20} - \frac{1}{288}\sqrt{\frac{35}{3}}C^{40}_{22,22} + \frac{7C^{42}_{22,22}}{144\sqrt{15}} + \frac{7}{576}\sqrt{7}C^{31}_{31,00} - \frac{7}{192}\sqrt{\frac{7}{3}}C^{31}_{31,20} - \frac{1}{48}\sqrt{\frac{7}{15}}C^{31}_{31,22} - \frac{9}{320}C^{33}_{31,22} - \frac{7}{320}\sqrt{3}C^{33}_{33,00} + \frac{21}{320}C^{33}_{33,20} + \frac{3}{20}\sqrt{\frac{3}{10}}C^{33}_{33,22},$$

$$C^{2011,1}_{22,2213} = \frac{7}{64}\sqrt{\frac{7}{3}}C^{60}_{00,00} + \frac{7}{192}\sqrt{7}C^{60}_{00,20} - \frac{1}{32}\sqrt{\frac{7}{5}}C^{62}_{00,22} - \frac{7}{192}\sqrt{\frac{7}{3}}C^{51}_{11,00} - \frac{7}{576}\sqrt{7}C^{51}_{11,20} + \frac{1}{144}\sqrt{\frac{7}{5}}C^{51}_{11,22} + \frac{3}{320}\sqrt{3}C^{53}_{11,22} - \frac{7}{192}\sqrt{\frac{7}{3}}C^{40}_{20,00} - \frac{7}{576}\sqrt{7}C^{40}_{20,20} + \frac{1}{144}\sqrt{\frac{7}{5}}C^{42}_{20,22} + \frac{7}{192}\sqrt{\frac{7}{15}}C^{42}_{22,00} + \frac{7}{576}\sqrt{\frac{7}{5}}C^{42}_{22,20} + \frac{1}{288}\sqrt{35}C^{40}_{22,22} - \frac{7C^{42}_{22,22}}{144\sqrt{5}} + \frac{7}{192}\sqrt{\frac{7}{3}}C^{31}_{31,00} + \frac{7}{576}\sqrt{7}C^{31}_{31,20} - \frac{1}{144}\sqrt{\frac{7}{5}}C^{31}_{31,22} - \frac{3}{320}\sqrt{3}C^{33}_{31,22} - \frac{21}{320}C^{33}_{33,00} - \frac{7}{320}\sqrt{3}C^{33}_{33,20} + \frac{3C^{33}_{33,22}}{20\sqrt{10}},$$

$$C^{2211,0}_{22,2213} = \frac{1}{96}\sqrt{\frac{7}{5}}C^{60}_{00,00} + \frac{1}{96}\sqrt{\frac{35}{3}}C^{60}_{00,20} + \frac{1}{20}\sqrt{\frac{7}{3}}C^{62}_{00,22} - \frac{1}{288}\sqrt{\frac{7}{5}}C^{51}_{11,00} + \frac{1}{96}\sqrt{\frac{7}{15}}C^{51}_{11,20} + \frac{7}{480}\sqrt{\frac{7}{3}}C^{51}_{11,22} + \frac{99C^{53}_{11,22}}{320\sqrt{5}} - \frac{1}{288}\sqrt{\frac{7}{5}}C^{40}_{20,00} - \frac{1}{288}\sqrt{\frac{35}{3}}C^{40}_{20,20} - \frac{7\sqrt{\frac{7}{3}}C^{42}_{20,22}}{1440} + \frac{\sqrt{7}C^{42}_{22,00}}{1440} + \frac{1}{288}\sqrt{\frac{7}{3}}C^{42}_{22,20} - \frac{11}{720}\sqrt{\frac{7}{3}}C^{40}_{22,22} + \frac{C^{42}_{22,22}}{360\sqrt{3}} + \frac{9}{80}\sqrt{\frac{3}{35}}C^{44}_{22,22} + \frac{1}{288}\sqrt{\frac{7}{5}}C^{31}_{31,00} - \frac{1}{96}\sqrt{\frac{7}{15}}C^{31}_{31,20} - \frac{5}{96}\sqrt{\frac{7}{3}}C^{31}_{31,22} - \frac{3C^{33}_{31,22}}{64\sqrt{5}} - \frac{1}{160}\sqrt{\frac{3}{5}}C^{33}_{33,00} + \frac{3C^{33}_{33,20}}{160\sqrt{5}} + \frac{3}{80}\sqrt{\frac{3}{2}}C^{33}_{33,22},$$

$$C^{2211,1}_{22,2213} = \frac{1}{32}\sqrt{\frac{7}{15}}C^{60}_{00,00} + \frac{1}{96}\sqrt{\frac{7}{5}}C^{60}_{00,20} - \frac{1}{20}\sqrt{7}C^{62}_{00,22} - \frac{1}{96}\sqrt{\frac{7}{15}}C^{51}_{11,00} - \frac{1}{288}\sqrt{\frac{7}{5}}C^{51}_{11,20} + \frac{7\sqrt{7}C^{51}_{11,22}}{1440} + \frac{33}{320}\sqrt{\frac{3}{5}}C^{53}_{11,22} - \frac{1}{96}\sqrt{\frac{7}{15}}C^{40}_{20,00} - \frac{1}{288}\sqrt{\frac{7}{5}}C^{40}_{20,20} + \frac{7\sqrt{7}C^{42}_{20,22}}{1440} + \frac{1}{480}\sqrt{\frac{7}{3}}C^{42}_{22,00} + \frac{\sqrt{7}C^{42}_{22,20}}{1440} + \frac{11}{720}\sqrt{7}C^{40}_{22,22} - \frac{1}{360}C^{42}_{22,22} - \frac{27C^{44}_{22,22}}{80\sqrt{35}} + \frac{1}{96}\sqrt{\frac{7}{15}}C^{31}_{31,00} + \frac{1}{288}\sqrt{\frac{7}{5}}C^{31}_{31,20} - \frac{5}{288}\sqrt{7}C^{31}_{31,22} - \frac{1}{64}\sqrt{\frac{3}{5}}C^{33}_{31,22} - \frac{3C^{33}_{33,00}}{160\sqrt{5}} - \frac{1}{160}\sqrt{\frac{3}{5}}C^{33}_{33,20} + \frac{3C^{33}_{33,22}}{80\sqrt{2}},$$

$$C^{2212,0}_{22,2213} = \frac{1}{48}\sqrt{\frac{7}{2}}C^{60}_{00,00} + \frac{5}{48}\sqrt{\frac{7}{6}}C^{60}_{00,20} - \frac{1}{16}\sqrt{\frac{7}{30}}C^{62}_{00,22} - \frac{1}{144}\sqrt{\frac{7}{2}}C^{51}_{11,00} + \frac{1}{48}\sqrt{\frac{7}{6}}C^{51}_{11,20} + \frac{1}{12}\sqrt{\frac{7}{30}}C^{51}_{11,22} - \frac{27C^{53}_{11,22}}{160\sqrt{2}} - \frac{1}{144}\sqrt{\frac{7}{2}}C^{40}_{20,00} - \frac{5}{144}\sqrt{\frac{7}{6}}C^{40}_{20,20} - \frac{1}{36}\sqrt{\frac{7}{30}}C^{42}_{20,22} + \frac{1}{144}\sqrt{\frac{7}{10}}C^{42}_{22,00} + \frac{1}{144}\sqrt{\frac{35}{6}}C^{42}_{22,20} + \frac{1}{144}\sqrt{\frac{35}{6}}C^{40}_{22,22} + \frac{C^{42}_{22,22}}{9\sqrt{30}} - \frac{1}{16}\sqrt{\frac{3}{14}}C^{44}_{22,22} + \frac{1}{144}\sqrt{\frac{7}{2}}C^{31}_{31,00} - \frac{1}{48}\sqrt{\frac{7}{6}}C^{31}_{31,20} + \frac{1}{24}\sqrt{\frac{7}{30}}C^{31}_{31,22} - \frac{C^{33}_{31,22}}{160\sqrt{2}} - \frac{1}{80}\sqrt{\frac{3}{2}}C^{33}_{33,00} + \frac{3C^{33}_{33,20}}{80\sqrt{2}} + \frac{21}{160}\sqrt{\frac{3}{5}}C^{33}_{33,22},$$

$$C^{2212,1}_{22,2213} = \frac{1}{16}\sqrt{\frac{7}{6}}C^{60}_{00,00} + \frac{1}{48}\sqrt{\frac{7}{2}}C^{60}_{00,20} + \frac{1}{16}\sqrt{\frac{7}{10}}C^{62}_{00,22} - \frac{1}{48}\sqrt{\frac{7}{6}}C^{51}_{11,00} - \frac{1}{144}\sqrt{\frac{7}{2}}C^{51}_{11,20} + \frac{1}{36}\sqrt{\frac{7}{10}}C^{51}_{11,22} - \frac{9}{160}\sqrt{\frac{3}{2}}C^{53}_{11,22} - \frac{1}{48}\sqrt{\frac{7}{6}}C^{40}_{20,00} - \frac{1}{144}\sqrt{\frac{7}{2}}C^{40}_{20,20} + \frac{1}{36}\sqrt{\frac{7}{10}}C^{42}_{20,22} + \frac{1}{48}\sqrt{\frac{7}{30}}C^{42}_{22,00} + \frac{1}{144}\sqrt{\frac{7}{10}}C^{42}_{22,20} - \frac{1}{144}\sqrt{\frac{35}{2}}C^{40}_{22,22} - \frac{C^{42}_{22,22}}{9\sqrt{10}} + \frac{3C^{44}_{22,22}}{16\sqrt{14}} + \frac{1}{48}\sqrt{\frac{7}{6}}C^{31}_{31,00} + \frac{1}{144}\sqrt{\frac{7}{2}}C^{31}_{31,20} + \frac{1}{72}\sqrt{\frac{7}{10}}C^{31}_{31,22} - \frac{C^{33}_{31,22}}{160\sqrt{6}} - \frac{3C^{33}_{33,00}}{80\sqrt{2}} - \frac{1}{80}\sqrt{\frac{3}{2}}C^{33}_{33,20} + \frac{21C^{33}_{33,22}}{160\sqrt{5}},$$

$$C^{2213,0}_{22,2213} = \frac{1}{16}\sqrt{\frac{7}{30}}C^{60}_{00,00} + \frac{1}{48}\sqrt{\frac{35}{2}}C^{60}_{00,20} + \frac{1}{160}\sqrt{\frac{7}{2}}C^{62}_{00,22} - \frac{1}{48}\sqrt{\frac{7}{30}}C^{51}_{11,00} + \frac{1}{48}\sqrt{\frac{7}{10}}C^{51}_{11,20} -$$

$$\frac{1}{480}\sqrt{\frac{7}{2}}C^{51}_{11,22} + \frac{9}{160}\sqrt{\frac{3}{10}}C^{53}_{11,22} - \frac{1}{48}\sqrt{\frac{7}{30}}C^{40}_{20,00} - \frac{1}{144}\sqrt{\frac{35}{2}}C^{40}_{20,20} + \frac{\sqrt{\frac{7}{2}}C^{42}_{20,22}}{1440} + \frac{1}{240}\sqrt{\frac{7}{6}}C^{42}_{22,00} + \frac{1}{144}\sqrt{\frac{7}{2}}C^{42}_{22,20} + \frac{\sqrt{\frac{7}{2}}C^{40}_{22,22}}{1440} - \frac{11C^{42}_{22,22}}{720\sqrt{2}} + \frac{9C^{44}_{22,22}}{80\sqrt{70}} + \frac{1}{48}\sqrt{\frac{7}{30}}C^{31}_{31,00} - \frac{1}{48}\sqrt{\frac{7}{10}}C^{31}_{31,20} - \frac{1}{96}\sqrt{\frac{7}{2}}C^{31}_{31,22} + \frac{1}{32}\sqrt{\frac{3}{10}}C^{33}_{31,22} - \frac{3C^{33}_{33,00}}{80\sqrt{10}} + \frac{3}{80}\sqrt{\frac{3}{10}}C^{33}_{33,20} - \frac{9}{160}C^{33}_{33,22},$$

$$C^{2213,1}_{22,2213} = \frac{1}{16}\sqrt{\frac{7}{10}}C^{60}_{00,00} + \frac{1}{16}\sqrt{\frac{7}{30}}C^{60}_{00,20} - \frac{1}{160}\sqrt{\frac{21}{2}}C^{62}_{00,22} - \frac{1}{48}\sqrt{\frac{7}{10}}C^{51}_{11,00} - \frac{1}{48}\sqrt{\frac{7}{30}}C^{51}_{11,20} - \frac{1}{480}\sqrt{\frac{7}{6}}C^{51}_{11,22} + \frac{9C^{53}_{11,22}}{160\sqrt{10}} - \frac{1}{48}\sqrt{\frac{7}{10}}C^{40}_{20,00} - \frac{1}{48}\sqrt{\frac{7}{30}}C^{40}_{20,20} - \frac{1}{480}\sqrt{\frac{7}{6}}C^{42}_{20,22} + \frac{1}{240}\sqrt{\frac{7}{2}}C^{42}_{22,00} + \frac{1}{240}\sqrt{\frac{7}{6}}C^{42}_{22,20} - \frac{1}{480}\sqrt{\frac{7}{6}}C^{40}_{22,22} + \frac{11C^{42}_{22,22}}{240\sqrt{6}} - \frac{9}{80}\sqrt{\frac{3}{70}}C^{44}_{22,22} + \frac{1}{48}\sqrt{\frac{7}{10}}C^{31}_{31,00} + \frac{1}{48}\sqrt{\frac{7}{30}}C^{31}_{31,20} - \frac{1}{96}\sqrt{\frac{7}{6}}C^{31}_{31,22} + \frac{C^{33}_{31,22}}{32\sqrt{10}} - \frac{3}{80}\sqrt{\frac{3}{10}}C^{33}_{33,00} - \frac{3C^{33}_{33,20}}{80\sqrt{10}} - \frac{3}{160}\sqrt{3}C^{33}_{33,22},$$

$$C^{1101,0}_{22,3101} = \frac{21C^{60}_{00,00}}{32\sqrt{5}} + \frac{7}{32}\sqrt{\frac{3}{5}}C^{60}_{00,20} + \frac{7}{96}\sqrt{5}C^{51}_{11,00} - \frac{7C^{51}_{11,20}}{32\sqrt{15}} - \frac{7C^{40}_{20,00}}{32\sqrt{5}} - \frac{7C^{40}_{20,20}}{32\sqrt{15}} + \frac{7}{160}C^{42}_{22,00} + \frac{7C^{42}_{22,20}}{160\sqrt{3}} - \frac{7}{96}\sqrt{5}C^{31}_{31,00} + \frac{7C^{31}_{31,20}}{32\sqrt{15}} + \frac{3}{32}\sqrt{\frac{21}{5}}C^{33}_{33,00} - \frac{9}{160}\sqrt{\frac{7}{5}}C^{33}_{33,20},$$

$$C^{1101,1}_{22,3101} = -\frac{7}{32}\sqrt{\frac{3}{5}}C^{60}_{00,00} + \frac{21C^{60}_{00,20}}{32\sqrt{5}} + \frac{7C^{51}_{11,00}}{32\sqrt{15}} - \frac{7C^{51}_{11,20}}{32\sqrt{5}} + \frac{7C^{40}_{20,00}}{32\sqrt{15}} - \frac{7C^{40}_{20,20}}{32\sqrt{5}} - \frac{7C^{42}_{22,00}}{160\sqrt{3}} + \frac{7}{160}C^{42}_{22,20} - \frac{7C^{31}_{31,00}}{32\sqrt{15}} + \frac{7C^{31}_{31,20}}{32\sqrt{5}} + \frac{9}{160}\sqrt{\frac{7}{5}}C^{33}_{33,00} - \frac{9}{160}\sqrt{\frac{21}{5}}C^{33}_{33,20},$$

$$C^{1112,0}_{22,3110} = -\frac{7C^{60}_{00,00}}{32\sqrt{15}} - \frac{7}{96}\sqrt{5}C^{60}_{00,20} - \frac{7}{80}C^{62}_{00,22} + \frac{7C^{51}_{11,00}}{96\sqrt{15}} - \frac{7C^{51}_{11,20}}{96\sqrt{5}} - \frac{7}{480}C^{51}_{11,22} - \frac{27}{320}\sqrt{\frac{21}{5}}C^{53}_{11,22} + \frac{7C^{40}_{20,00}}{96\sqrt{15}} + \frac{7}{288}\sqrt{5}C^{40}_{20,20} + \frac{7C^{42}_{20,22}}{1440} - \frac{7C^{42}_{22,00}}{480\sqrt{3}} - \frac{7}{288}C^{42}_{22,20} + \frac{13}{360}C^{40}_{22,22} - \frac{1}{360}\sqrt{7}C^{42}_{22,22} - \frac{3C^{44}_{22,22}}{40\sqrt{5}} - \frac{7C^{31}_{31,00}}{96\sqrt{15}} + \frac{7C^{31}_{31,20}}{96\sqrt{5}} + \frac{37}{480}C^{31}_{31,22} + \frac{7}{320}\sqrt{\frac{21}{5}}C^{33}_{31,22} + \frac{3}{160}\sqrt{\frac{7}{5}}C^{33}_{33,00} - \frac{3}{160}\sqrt{\frac{21}{5}}C^{33}_{33,20} - \frac{9}{200}\sqrt{\frac{7}{2}}C^{33}_{33,22},$$

$$C^{1112,1}_{22,3110} = -\frac{7C^{60}_{00,00}}{32\sqrt{5}} - \frac{7C^{60}_{00,20}}{32\sqrt{15}} + \frac{7}{80}\sqrt{3}C^{62}_{00,22} + \frac{7C^{51}_{11,00}}{96\sqrt{5}} + \frac{7C^{51}_{11,20}}{96\sqrt{15}} - \frac{7C^{51}_{11,22}}{480\sqrt{3}} - \frac{27}{320}\sqrt{\frac{7}{5}}C^{53}_{11,22} + \frac{7C^{40}_{20,00}}{96\sqrt{5}} + \frac{7C^{40}_{20,20}}{96\sqrt{15}} - \frac{7C^{42}_{20,22}}{480\sqrt{3}} - \frac{7}{480}C^{42}_{22,00} - \frac{7C^{42}_{22,20}}{480\sqrt{3}} - \frac{13C^{40}_{22,22}}{120\sqrt{3}} + \frac{1}{120}\sqrt{\frac{7}{3}}C^{42}_{22,22} + \frac{3}{40}\sqrt{\frac{3}{5}}C^{44}_{22,22} - \frac{7C^{31}_{31,00}}{96\sqrt{5}} - \frac{7C^{31}_{31,20}}{96\sqrt{15}} + \frac{37C^{31}_{31,22}}{480\sqrt{3}} + \frac{7}{320}\sqrt{\frac{7}{5}}C^{33}_{31,22} + \frac{3}{160}\sqrt{\frac{21}{5}}C^{33}_{33,00} + \frac{3}{160}\sqrt{\frac{7}{5}}C^{33}_{33,20} - \frac{3}{200}\sqrt{\frac{21}{2}}C^{33}_{33,22},$$

$$C^{1111,0}_{22,3111} = \frac{7C^{60}_{00,00}}{64\sqrt{5}} + \frac{7}{64}\sqrt{\frac{5}{3}}C^{60}_{00,20} - \frac{7}{320}\sqrt{3}C^{62}_{00,22} - \frac{7C^{51}_{11,00}}{192\sqrt{5}} + \frac{7C^{51}_{11,20}}{64\sqrt{15}} - \frac{7C^{51}_{11,22}}{64\sqrt{3}} - \frac{7C^{40}_{20,00}}{192\sqrt{5}} - \frac{7}{192}\sqrt{\frac{5}{3}}C^{40}_{20,20} + \frac{7C^{42}_{20,22}}{192\sqrt{3}} + \frac{7}{960}C^{42}_{22,00} + \frac{7C^{42}_{22,20}}{192\sqrt{3}} + \frac{53C^{40}_{22,22}}{960\sqrt{3}} - \frac{19}{480}\sqrt{\frac{7}{3}}C^{42}_{22,22} + \frac{3}{80}\sqrt{\frac{3}{5}}C^{44}_{22,22} + \frac{7C^{31}_{31,00}}{192\sqrt{5}} - \frac{7C^{31}_{31,20}}{64\sqrt{15}} + \frac{C^{31}_{31,22}}{64\sqrt{3}} + \frac{3}{32}\sqrt{\frac{7}{5}}C^{33}_{31,22} - \frac{3}{320}\sqrt{\frac{21}{5}}C^{33}_{33,00} + \frac{9}{320}\sqrt{\frac{7}{5}}C^{33}_{33,20} - \frac{9}{80}\sqrt{\frac{21}{2}}C^{33}_{33,22},$$

$$C^{1111,1}_{22,3111} = \frac{7}{64}\sqrt{\frac{3}{5}}C^{60}_{00,00} + \frac{7C^{60}_{00,20}}{64\sqrt{5}} + \frac{21}{320}C^{62}_{00,22} - \frac{7C^{51}_{11,00}}{64\sqrt{15}} - \frac{7C^{51}_{11,20}}{192\sqrt{5}} - \frac{7}{192}C^{51}_{11,22} - \frac{7C^{40}_{20,00}}{64\sqrt{15}} - \frac{7C^{40}_{20,20}}{192\sqrt{5}} - \frac{7}{192}C^{42}_{20,22} + \frac{7C^{42}_{22,00}}{320\sqrt{3}} + \frac{7}{960}C^{42}_{22,20} - \frac{53}{960}C^{40}_{22,22} + \frac{19}{480}\sqrt{7}C^{42}_{22,22} - \frac{9C^{44}_{22,22}}{80\sqrt{5}} + \frac{7C^{31}_{31,00}}{64\sqrt{15}} + \frac{7C^{31}_{31,20}}{192\sqrt{5}} + \frac{1}{192}C^{31}_{31,22} + \frac{1}{32}\sqrt{\frac{21}{5}}C^{33}_{31,22} - \frac{9}{320}\sqrt{\frac{7}{5}}C^{33}_{33,00} - \frac{3}{320}\sqrt{\frac{21}{5}}C^{33}_{33,20} - \frac{9}{80}\sqrt{\frac{7}{2}}C^{33}_{33,22},$$

$$C^{1112,0}_{22,3111} = \frac{7}{64}\sqrt{\frac{3}{5}}C^{60}_{00,00} + \frac{7}{64}\sqrt{5}C^{60}_{00,20} - \frac{21}{320}C^{62}_{00,22} - \frac{7C^{51}_{11,00}}{64\sqrt{15}} + \frac{7C^{51}_{11,20}}{64\sqrt{5}} + \frac{7}{320}C^{51}_{11,22} -$$

$$\frac{27}{320}\sqrt{\frac{21}{5}}C^{53}_{11,22}-\frac{7C^{40}_{20,00}}{64\sqrt{15}}-\frac{7}{192}\sqrt{5}C^{40}_{20,20}-\frac{7}{960}C^{42}_{20,22}+\frac{7C^{42}_{22,00}}{320\sqrt{3}}+\frac{7}{192}C^{42}_{22,20}+\frac{17}{960}C^{40}_{22,22}+ \frac{1}{96}\sqrt{7}C^{42}_{22,22}-\frac{9C^{44}_{22,22}}{80\sqrt{5}}+\frac{7C^{31}_{31,00}}{64\sqrt{15}}-\frac{7C^{31}_{31,20}}{64\sqrt{5}}+\frac{23}{320}C^{31}_{31,22}-\frac{3}{320}\sqrt{\frac{21}{5}}C^{33}_{31,22}-\frac{9}{320}\sqrt{\frac{7}{5}}C^{33}_{33,00}+ \frac{9}{320}\sqrt{\frac{21}{5}}C^{33}_{33,20}+\frac{27}{400}\sqrt{\frac{7}{2}}C^{33}_{33,22},$$

$$C^{1112,1}_{22,3111}=\frac{21C^{60}_{00,00}}{64\sqrt{5}}+\frac{7}{64}\sqrt{\frac{3}{5}}C^{60}_{00,20}+\frac{21}{320}\sqrt{3}C^{62}_{00,22}-\frac{7C^{51}_{11,00}}{64\sqrt{5}}-\frac{7C^{51}_{11,20}}{64\sqrt{15}}+\frac{7C^{51}_{11,22}}{320\sqrt{3}}- \frac{27}{320}\sqrt{\frac{7}{5}}C^{53}_{11,22}-\frac{7C^{40}_{20,00}}{64\sqrt{5}}-\frac{7C^{40}_{20,20}}{64\sqrt{15}}+\frac{7C^{42}_{20,22}}{320\sqrt{3}}+\frac{7}{320}C^{42}_{22,00}+\frac{7C^{42}_{22,20}}{320\sqrt{3}}-\frac{17C^{40}_{22,22}}{320\sqrt{3}}- \frac{1}{32}\sqrt{\frac{7}{3}}C^{42}_{22,22}+\frac{9}{80}\sqrt{\frac{3}{5}}C^{44}_{22,22}+\frac{7C^{31}_{31,00}}{64\sqrt{5}}+\frac{7C^{31}_{31,20}}{64\sqrt{15}}+\frac{23C^{31}_{31,22}}{320\sqrt{3}}-\frac{3}{320}\sqrt{\frac{7}{5}}C^{33}_{31,22}-\frac{9}{320}\sqrt{\frac{21}{5}}C^{33}_{33,00}- \frac{9}{320}\sqrt{\frac{7}{5}}C^{33}_{33,20}+\frac{9}{400}\sqrt{\frac{21}{2}}C^{33}_{33,22},$$

$$C^{1110,0}_{22,3112}=-\frac{7C^{60}_{00,00}}{32\sqrt{15}}-\frac{7}{96}\sqrt{5}C^{60}_{00,20}-\frac{7}{80}C^{62}_{00,22}+\frac{7C^{51}_{11,00}}{96\sqrt{15}}-\frac{7C^{51}_{11,20}}{96\sqrt{5}}-\frac{7}{480}C^{51}_{11,22}- \frac{27}{320}\sqrt{\frac{21}{5}}C^{53}_{11,22}+\frac{7C^{40}_{20,00}}{96\sqrt{15}}+\frac{7}{288}\sqrt{5}C^{40}_{20,20}+\frac{7C^{42}_{20,22}}{1440}-\frac{7C^{42}_{22,00}}{480\sqrt{3}}-\frac{7}{288}C^{42}_{22,20}+\frac{13}{360}C^{40}_{22,22}- \frac{1}{360}\sqrt{7}C^{42}_{22,22}-\frac{3C^{44}_{22,22}}{40\sqrt{5}}-\frac{7C^{31}_{31,00}}{96\sqrt{15}}+\frac{7C^{31}_{31,20}}{96\sqrt{5}}+\frac{37}{480}C^{31}_{31,22}+\frac{7}{320}\sqrt{\frac{21}{5}}C^{33}_{31,22}+\frac{3}{160}\sqrt{\frac{7}{5}}C^{33}_{33,00}- \frac{3}{160}\sqrt{\frac{21}{5}}C^{33}_{33,20}-\frac{9}{200}\sqrt{\frac{7}{2}}C^{33}_{33,22},$$

$$C^{1110,1}_{22,3112}=-\frac{7C^{60}_{00,00}}{32\sqrt{5}}-\frac{7C^{60}_{00,20}}{32\sqrt{15}}+\frac{7}{80}\sqrt{3}C^{62}_{00,22}+\frac{7C^{51}_{11,00}}{96\sqrt{5}}+\frac{7C^{51}_{11,20}}{96\sqrt{15}}-\frac{7C^{51}_{11,22}}{480\sqrt{3}}-\frac{27}{320}\sqrt{\frac{7}{5}}C^{53}_{11,22}+ \frac{7C^{40}_{20,00}}{96\sqrt{5}}+\frac{7C^{40}_{20,20}}{96\sqrt{15}}-\frac{7C^{42}_{20,22}}{480\sqrt{3}}-\frac{7}{480}C^{42}_{22,00}-\frac{7C^{42}_{22,20}}{480\sqrt{3}}-\frac{13C^{40}_{22,22}}{120\sqrt{3}}+\frac{1}{120}\sqrt{\frac{7}{3}}C^{42}_{22,22}+ \frac{3}{40}\sqrt{\frac{3}{5}}C^{44}_{22,22}-\frac{7C^{31}_{31,00}}{96\sqrt{5}}-\frac{7C^{31}_{31,20}}{96\sqrt{15}}+\frac{37C^{31}_{31,22}}{480\sqrt{3}}+\frac{7}{320}\sqrt{\frac{7}{5}}C^{33}_{31,22}+\frac{3}{160}\sqrt{\frac{21}{5}}C^{33}_{33,00}+ \frac{3}{160}\sqrt{\frac{7}{5}}C^{33}_{33,20}-\frac{3}{200}\sqrt{\frac{21}{2}}C^{33}_{33,22},$$

$$C^{1111,0}_{22,3112}=-\frac{7}{64}\sqrt{\frac{3}{5}}C^{60}_{00,00}-\frac{7}{64}\sqrt{5}C^{60}_{00,20}+\frac{21}{320}C^{62}_{00,22}+\frac{7C^{51}_{11,00}}{64\sqrt{15}}-\frac{7C^{51}_{11,20}}{64\sqrt{5}}-\frac{7}{320}C^{51}_{11,22}+ \frac{27}{320}\sqrt{\frac{21}{5}}C^{53}_{11,22}+\frac{7C^{40}_{20,00}}{64\sqrt{15}}+\frac{7}{192}\sqrt{5}C^{40}_{20,20}+\frac{7}{960}C^{42}_{20,22}-\frac{7C^{42}_{22,00}}{320\sqrt{3}}-\frac{7}{192}C^{42}_{22,20}-\frac{17}{960}C^{40}_{22,22}- \frac{1}{96}\sqrt{7}C^{42}_{22,22}+\frac{9C^{44}_{22,22}}{80\sqrt{5}}-\frac{7C^{31}_{31,00}}{64\sqrt{15}}+\frac{7C^{31}_{31,20}}{64\sqrt{5}}-\frac{23}{320}C^{31}_{31,22}+\frac{3}{320}\sqrt{\frac{21}{5}}C^{33}_{31,22}+\frac{9}{320}\sqrt{\frac{7}{5}}C^{33}_{33,00}- \frac{9}{320}\sqrt{\frac{21}{5}}C^{33}_{33,20}-\frac{27}{400}\sqrt{\frac{7}{2}}C^{33}_{33,22},$$

$$C^{1111,1}_{22,3112}=-\frac{21C^{60}_{00,00}}{64\sqrt{5}}-\frac{7}{64}\sqrt{\frac{3}{5}}C^{60}_{00,20}-\frac{21}{320}\sqrt{3}C^{62}_{00,22}+\frac{7C^{51}_{11,00}}{64\sqrt{5}}+\frac{7C^{51}_{11,20}}{64\sqrt{15}}-\frac{7C^{51}_{11,22}}{320\sqrt{3}}+ \frac{27}{320}\sqrt{\frac{7}{5}}C^{53}_{11,22}+\frac{7C^{40}_{20,00}}{64\sqrt{5}}+\frac{7C^{40}_{20,20}}{64\sqrt{15}}-\frac{7C^{42}_{20,22}}{320\sqrt{3}}-\frac{7}{320}C^{42}_{22,00}-\frac{7C^{42}_{22,20}}{320\sqrt{3}}+\frac{17C^{40}_{22,22}}{320\sqrt{3}}+ \frac{1}{32}\sqrt{\frac{7}{3}}C^{42}_{22,22}-\frac{9}{80}\sqrt{\frac{3}{5}}C^{44}_{22,22}-\frac{7C^{31}_{31,00}}{64\sqrt{5}}-\frac{7C^{31}_{31,20}}{64\sqrt{15}}-\frac{23C^{31}_{31,22}}{320\sqrt{3}}+\frac{3}{320}\sqrt{\frac{7}{5}}C^{33}_{31,22}+\frac{9}{320}\sqrt{\frac{21}{5}}C^{33}_{33,00}+ \frac{9}{320}\sqrt{\frac{7}{5}}C^{33}_{33,20}-\frac{9}{400}\sqrt{\frac{21}{2}}C^{33}_{33,22},$$

$$C^{1112,0}_{22,3112}=-\frac{7}{64}\sqrt{\frac{7}{15}}C^{60}_{00,00}-\frac{7}{192}\sqrt{35}C^{60}_{00,20}-\frac{1}{64}\sqrt{7}C^{62}_{00,22}+\frac{7}{192}\sqrt{\frac{7}{15}}C^{51}_{11,00}-\frac{7}{192}\sqrt{\frac{7}{5}}C^{51}_{11,20}+ \frac{11}{960}\sqrt{7}C^{51}_{11,22}-\frac{27}{160}\sqrt{\frac{3}{5}}C^{53}_{11,22}+\frac{7}{192}\sqrt{\frac{7}{15}}C^{40}_{20,00}+\frac{7}{576}\sqrt{35}C^{40}_{20,20}-\frac{11\sqrt{7}C^{42}_{20,22}}{2880}-\frac{7}{960}\sqrt{\frac{7}{3}}C^{42}_{22,00}- \frac{7}{576}\sqrt{7}C^{42}_{22,20}+\frac{7\sqrt{7}C^{40}_{22,22}}{2880}+\frac{49C^{42}_{22,22}}{1440}-\frac{3}{80}\sqrt{\frac{7}{5}}C^{44}_{22,22}-\frac{7}{192}\sqrt{\frac{7}{15}}C^{31}_{31,00}+\frac{7}{192}\sqrt{\frac{7}{5}}C^{31}_{31,20}+ \frac{19}{960}\sqrt{7}C^{31}_{31,22}-\frac{1}{20}\sqrt{\frac{3}{5}}C^{33}_{31,22}+\frac{21C^{33}_{33,00}}{320\sqrt{5}}-\frac{21}{320}\sqrt{\frac{3}{5}}C^{33}_{33,20}+\frac{99C^{33}_{33,22}}{400\sqrt{2}},$$

$$C^{1112,1}_{22,3112}=-\frac{7}{64}\sqrt{\frac{7}{5}}C^{60}_{00,00}-\frac{7}{64}\sqrt{\frac{7}{15}}C^{60}_{00,20}+\frac{1}{64}\sqrt{21}C^{62}_{00,22}+\frac{7}{192}\sqrt{\frac{7}{5}}C^{51}_{11,00}+\frac{7}{192}\sqrt{\frac{7}{15}}C^{51}_{11,20}+$$

$$\frac{11}{960}\sqrt{\frac{7}{3}}C^{51}_{11,22}-\frac{27C^{53}_{11,22}}{160\sqrt{5}}+\frac{7}{192}\sqrt{\frac{7}{5}}C^{40}_{20,00}+\frac{7}{192}\sqrt{\frac{7}{15}}C^{40}_{20,20}+\frac{11}{960}\sqrt{\frac{7}{3}}C^{42}_{20,22}-\frac{7}{960}\sqrt{7}C^{42}_{22,00}-$$
$$\frac{7}{960}\sqrt{\frac{7}{3}}C^{42}_{22,20}-\frac{7}{960}\sqrt{\frac{7}{3}}C^{40}_{22,22}-\frac{49C^{42}_{22,22}}{480\sqrt{3}}+\frac{3}{80}\sqrt{\frac{21}{5}}C^{44}_{22,22}-\frac{7}{192}\sqrt{\frac{7}{5}}C^{31}_{31,00}-\frac{7}{192}\sqrt{\frac{7}{15}}C^{31}_{31,20}+$$
$$\frac{19}{960}\sqrt{\frac{7}{3}}C^{31}_{31,22}-\frac{C^{33}_{31,22}}{20\sqrt{5}}+\frac{21}{320}\sqrt{\frac{3}{5}}C^{33}_{33,00}+\frac{21C^{33}_{33,20}}{320\sqrt{5}}+\frac{33}{400}\sqrt{\frac{3}{2}}C^{33}_{33,22},$$

$$C^{1101,0}_{22,3303}=\frac{1}{32}\sqrt{21}C^{60}_{00,00}+\frac{1}{32}\sqrt{7}C^{60}_{00,20}+\frac{5}{96}\sqrt{\frac{7}{3}}C^{51}_{11,00}-\frac{1}{96}\sqrt{7}C^{51}_{11,20}-\frac{1}{32}\sqrt{\frac{7}{3}}C^{40}_{20,00}-$$
$$\frac{1}{96}\sqrt{7}C^{40}_{20,20}+\frac{1}{32}\sqrt{\frac{7}{15}}C^{42}_{22,00}+\frac{1}{96}\sqrt{\frac{7}{5}}C^{42}_{22,20}-\frac{5}{96}\sqrt{\frac{7}{3}}C^{31}_{31,00}+\frac{1}{96}\sqrt{7}C^{31}_{31,20}+\frac{3}{32}C^{33}_{33,00}-$$
$$\frac{3}{160}\sqrt{3}C^{33}_{33,20},$$

$$C^{1101,1}_{22,3303}=-\frac{1}{32}\sqrt{7}C^{60}_{00,00}+\frac{1}{32}\sqrt{21}C^{60}_{00,20}+\frac{1}{96}\sqrt{7}C^{51}_{11,00}-\frac{1}{32}\sqrt{\frac{7}{3}}C^{51}_{11,20}+\frac{1}{96}\sqrt{7}C^{40}_{20,00}-$$
$$\frac{1}{32}\sqrt{\frac{7}{3}}C^{40}_{20,20}-\frac{1}{96}\sqrt{\frac{7}{5}}C^{42}_{22,00}+\frac{1}{32}\sqrt{\frac{7}{15}}C^{42}_{22,20}-\frac{1}{96}\sqrt{7}C^{31}_{31,00}+\frac{1}{32}\sqrt{\frac{7}{3}}C^{31}_{31,20}+\frac{3}{160}\sqrt{3}C^{33}_{33,00}-$$
$$\frac{9}{160}C^{33}_{33,20},$$

$$C^{1110,0}_{22,3312}=-\frac{1}{96}\sqrt{7}C^{60}_{00,00}-\frac{5}{96}\sqrt{\frac{7}{3}}C^{60}_{00,20}-\frac{1}{16}\sqrt{\frac{7}{15}}C^{62}_{00,22}+\frac{1}{288}\sqrt{7}C^{51}_{11,00}-\frac{1}{96}\sqrt{\frac{7}{3}}C^{51}_{11,20}-$$
$$\frac{1}{6}\sqrt{\frac{7}{15}}C^{51}_{11,22}+\frac{9}{160}C^{53}_{11,22}+\frac{1}{288}\sqrt{7}C^{40}_{20,00}+\frac{5}{288}\sqrt{\frac{7}{3}}C^{40}_{20,20}+\frac{1}{18}\sqrt{\frac{7}{15}}C^{42}_{20,22}-\frac{1}{288}\sqrt{\frac{7}{5}}C^{42}_{22,00}-$$
$$\frac{1}{288}\sqrt{\frac{35}{3}}C^{42}_{22,20}-\frac{7}{144}\sqrt{\frac{7}{15}}C^{40}_{22,22}-\frac{C^{42}_{22,22}}{72\sqrt{15}}-\frac{1}{40}\sqrt{\frac{3}{7}}C^{44}_{22,22}-\frac{1}{288}\sqrt{7}C^{31}_{31,00}+\frac{1}{96}\sqrt{\frac{7}{3}}C^{31}_{31,20}+$$
$$\frac{1}{6}\sqrt{\frac{7}{15}}C^{31}_{31,22}-\frac{9}{160}C^{33}_{31,22}+\frac{1}{160}\sqrt{3}C^{33}_{33,00}-\frac{3}{160}C^{33}_{33,20}-\frac{3}{40}\sqrt{\frac{3}{10}}C^{33}_{33,22},$$

$$C^{1110,1}_{22,3312}=-\frac{1}{32}\sqrt{\frac{7}{3}}C^{60}_{00,00}-\frac{1}{96}\sqrt{7}C^{60}_{00,20}+\frac{1}{16}\sqrt{\frac{7}{5}}C^{62}_{00,22}+\frac{1}{96}\sqrt{\frac{7}{3}}C^{51}_{11,00}+\frac{1}{288}\sqrt{7}C^{51}_{11,20}-$$
$$\frac{1}{18}\sqrt{\frac{7}{5}}C^{51}_{11,22}+\frac{3}{160}\sqrt{3}C^{53}_{11,22}+\frac{1}{96}\sqrt{\frac{7}{3}}C^{40}_{20,00}+\frac{1}{288}\sqrt{7}C^{40}_{20,20}-\frac{1}{18}\sqrt{\frac{7}{5}}C^{42}_{20,22}-\frac{1}{96}\sqrt{\frac{7}{15}}C^{42}_{22,00}-$$
$$\frac{1}{288}\sqrt{\frac{7}{5}}C^{42}_{22,20}+\frac{7}{144}\sqrt{\frac{7}{5}}C^{40}_{22,22}+\frac{C^{42}_{22,22}}{72\sqrt{5}}+\frac{3C^{44}_{22,22}}{40\sqrt{7}}-\frac{1}{96}\sqrt{\frac{7}{3}}C^{31}_{31,00}-\frac{1}{288}\sqrt{7}C^{31}_{31,20}+$$
$$\frac{1}{18}\sqrt{\frac{7}{5}}C^{31}_{31,22}-\frac{3}{160}\sqrt{3}C^{33}_{31,22}+\frac{3}{160}C^{33}_{33,00}+\frac{1}{160}\sqrt{3}C^{33}_{33,20}-\frac{3C^{33}_{33,22}}{40\sqrt{10}},$$

$$C^{1111,0}_{22,3312}=\frac{1}{96}\sqrt{7}C^{60}_{00,00}+\frac{5}{96}\sqrt{\frac{7}{3}}C^{60}_{00,20}-\frac{1}{32}\sqrt{\frac{7}{15}}C^{62}_{00,22}-\frac{1}{288}\sqrt{7}C^{51}_{11,00}+\frac{1}{96}\sqrt{\frac{7}{3}}C^{51}_{11,20}-$$
$$\frac{7}{48}\sqrt{\frac{7}{15}}C^{51}_{11,22}+\frac{27}{320}C^{53}_{11,22}-\frac{1}{288}\sqrt{7}C^{40}_{20,00}-\frac{5}{288}\sqrt{\frac{7}{3}}C^{40}_{20,20}+\frac{7}{144}\sqrt{\frac{7}{15}}C^{42}_{20,22}+\frac{1}{288}\sqrt{\frac{7}{5}}C^{42}_{22,00}+$$
$$\frac{1}{288}\sqrt{\frac{35}{3}}C^{42}_{22,20}-\frac{19}{288}\sqrt{\frac{7}{15}}C^{40}_{22,22}+\frac{1}{144}\sqrt{\frac{5}{3}}C^{42}_{22,22}-\frac{1}{40}\sqrt{\frac{3}{7}}C^{44}_{22,22}+\frac{1}{288}\sqrt{7}C^{31}_{31,00}-$$
$$\frac{1}{96}\sqrt{\frac{7}{3}}C^{31}_{31,20}+\frac{7}{48}\sqrt{\frac{7}{15}}C^{31}_{31,22}-\frac{27}{320}C^{33}_{31,22}-\frac{1}{160}\sqrt{3}C^{33}_{33,00}+\frac{3}{160}C^{33}_{33,20}+\frac{3}{40}\sqrt{\frac{3}{10}}C^{33}_{33,22},$$

$$C^{1111,1}_{22,3312}=\frac{1}{32}\sqrt{\frac{7}{3}}C^{60}_{00,00}+\frac{1}{96}\sqrt{7}C^{60}_{00,20}+\frac{1}{32}\sqrt{\frac{7}{5}}C^{62}_{00,22}-\frac{1}{96}\sqrt{\frac{7}{3}}C^{51}_{11,00}-\frac{1}{288}\sqrt{7}C^{51}_{11,20}-$$
$$\frac{7}{144}\sqrt{\frac{7}{5}}C^{51}_{11,22}+\frac{9}{320}\sqrt{3}C^{53}_{11,22}-\frac{1}{96}\sqrt{\frac{7}{3}}C^{40}_{20,00}-\frac{1}{288}\sqrt{7}C^{40}_{20,20}-\frac{7}{144}\sqrt{\frac{7}{5}}C^{42}_{20,22}+\frac{1}{96}\sqrt{\frac{7}{15}}C^{42}_{22,00}+$$
$$\frac{1}{288}\sqrt{\frac{7}{5}}C^{42}_{22,20}+\frac{19}{288}\sqrt{\frac{7}{5}}C^{40}_{22,22}-\frac{1}{144}\sqrt{5}C^{42}_{22,22}+\frac{3C^{44}_{22,22}}{40\sqrt{7}}+\frac{1}{96}\sqrt{\frac{7}{3}}C^{31}_{31,00}+\frac{1}{288}\sqrt{7}C^{31}_{31,20}+$$
$$\frac{7}{144}\sqrt{\frac{7}{5}}C^{31}_{31,22}-\frac{9}{320}\sqrt{3}C^{33}_{31,22}-\frac{3}{160}C^{33}_{33,00}-\frac{1}{160}\sqrt{3}C^{33}_{33,20}+\frac{3C^{33}_{33,22}}{40\sqrt{10}},$$

$$C^{1112,0}_{22,3312}=-\frac{1}{96}C^{60}_{00,00}-\frac{5C^{60}_{00,20}}{96\sqrt{3}}-\frac{1}{32}\sqrt{\frac{5}{3}}C^{62}_{00,22}+\frac{1}{288}C^{51}_{11,00}-\frac{C^{51}_{11,20}}{96\sqrt{3}}-\frac{11C^{51}_{11,22}}{48\sqrt{15}}-$$
$$\frac{9C^{53}_{11,22}}{320\sqrt{7}}+\frac{1}{288}C^{40}_{20,00}+\frac{5C^{40}_{20,20}}{288\sqrt{3}}+\frac{11C^{42}_{20,22}}{144\sqrt{15}}-\frac{C^{42}_{22,00}}{288\sqrt{5}}-\frac{1}{288}\sqrt{\frac{5}{3}}C^{42}_{22,20}+\frac{C^{40}_{22,22}}{288\sqrt{15}}-\frac{23C^{42}_{22,22}}{144\sqrt{105}}-$$
$$\frac{1}{280}\sqrt{3}C^{44}_{22,22}-\frac{1}{288}C^{31}_{31,00}+\frac{C^{31}_{31,20}}{96\sqrt{3}}+\frac{11C^{31}_{31,22}}{48\sqrt{15}}+\frac{9C^{33}_{31,22}}{320\sqrt{7}}+\frac{1}{160}\sqrt{\frac{3}{7}}C^{33}_{33,00}-\frac{3C^{33}_{33,20}}{160\sqrt{7}}-$$
$$\frac{3}{40}\sqrt{\frac{21}{10}}C^{33}_{33,22},$$

$$C^{1112,1}_{22,3312} = -\frac{C^{60}_{00,00}}{32\sqrt{3}} - \frac{1}{96}C^{60}_{00,20} + \frac{1}{32}\sqrt{5}C^{62}_{00,22} + \frac{C^{51}_{11,00}}{96\sqrt{3}} + \frac{1}{288}C^{51}_{11,20} - \frac{11C^{51}_{11,22}}{144\sqrt{5}} - \frac{3}{320}\sqrt{\frac{3}{7}}C^{53}_{11,22} + \frac{C^{40}_{20,00}}{96\sqrt{3}} + \frac{1}{288}C^{40}_{20,20} - \frac{11C^{42}_{20,22}}{144\sqrt{5}} - \frac{C^{42}_{22,00}}{96\sqrt{15}} - \frac{C^{42}_{22,20}}{288\sqrt{5}} - \frac{C^{40}_{22,22}}{288\sqrt{5}} + \frac{23C^{42}_{22,22}}{144\sqrt{35}} + \frac{3}{280}C^{44}_{22,22} - \frac{C^{31}_{31,00}}{96\sqrt{3}} - \frac{1}{288}C^{31}_{31,20} + \frac{11C^{31}_{31,22}}{144\sqrt{5}} + \frac{3}{320}\sqrt{\frac{3}{7}}C^{33}_{31,22} + \frac{3C^{33}_{33,00}}{160\sqrt{7}} + \frac{1}{160}\sqrt{\frac{3}{7}}C^{33}_{33,20} - \frac{3}{40}\sqrt{\frac{7}{10}}C^{33}_{33,22},$$

$$C^{1111,0}_{22,3313} = -\frac{1}{48}\sqrt{\frac{7}{2}}C^{60}_{00,00} - \frac{5}{48}\sqrt{\frac{7}{6}}C^{60}_{00,20} + \frac{1}{16}\sqrt{\frac{7}{30}}C^{62}_{00,22} + \frac{1}{144}\sqrt{\frac{7}{2}}C^{51}_{11,00} - \frac{1}{48}\sqrt{\frac{7}{6}}C^{51}_{11,20} + \frac{1}{48}\sqrt{\frac{35}{6}}C^{51}_{11,22} + \frac{1}{144}\sqrt{\frac{7}{2}}C^{40}_{20,00} + \frac{5}{144}\sqrt{\frac{7}{6}}C^{40}_{20,20} - \frac{1}{144}\sqrt{\frac{35}{6}}C^{42}_{20,22} - \frac{1}{144}\sqrt{\frac{7}{10}}C^{42}_{22,00} - \frac{1}{144}\sqrt{\frac{35}{6}}C^{42}_{22,20} + \frac{1}{144}\sqrt{\frac{7}{30}}C^{40}_{22,22} + \frac{C^{42}_{22,22}}{18\sqrt{30}} + \frac{1}{80}\sqrt{\frac{3}{14}}C^{44}_{22,22} - \frac{1}{144}\sqrt{\frac{7}{2}}C^{31}_{31,00} + \frac{1}{48}\sqrt{\frac{7}{6}}C^{31}_{31,20} - \frac{1}{48}\sqrt{\frac{35}{6}}C^{31}_{31,22} + \frac{1}{80}\sqrt{\frac{3}{2}}C^{33}_{33,00} - \frac{3C^{33}_{33,20}}{80\sqrt{2}} + \frac{3}{32}\sqrt{\frac{3}{5}}C^{33}_{33,22},$$

$$C^{1111,1}_{22,3313} = -\frac{1}{16}\sqrt{\frac{7}{6}}C^{60}_{00,00} - \frac{1}{48}\sqrt{\frac{7}{2}}C^{60}_{00,20} - \frac{1}{16}\sqrt{\frac{7}{10}}C^{62}_{00,22} + \frac{1}{48}\sqrt{\frac{7}{6}}C^{51}_{11,00} + \frac{1}{144}\sqrt{\frac{7}{2}}C^{51}_{11,20} + \frac{1}{144}\sqrt{\frac{35}{2}}C^{51}_{11,22} + \frac{1}{48}\sqrt{\frac{7}{6}}C^{40}_{20,00} + \frac{1}{144}\sqrt{\frac{7}{2}}C^{40}_{20,20} + \frac{1}{144}\sqrt{\frac{35}{2}}C^{42}_{20,22} - \frac{1}{48}\sqrt{\frac{7}{30}}C^{42}_{22,00} - \frac{1}{144}\sqrt{\frac{7}{10}}C^{42}_{22,20} - \frac{1}{144}\sqrt{\frac{7}{10}}C^{40}_{22,22} - \frac{C^{42}_{22,22}}{18\sqrt{10}} - \frac{3C^{44}_{22,22}}{80\sqrt{14}} - \frac{1}{48}\sqrt{\frac{7}{6}}C^{31}_{31,00} - \frac{1}{144}\sqrt{\frac{7}{2}}C^{31}_{31,20} - \frac{1}{144}\sqrt{\frac{35}{2}}C^{31}_{31,22} + \frac{3C^{33}_{33,00}}{80\sqrt{2}} + \frac{1}{80}\sqrt{\frac{3}{2}}C^{33}_{33,20} + \frac{3C^{33}_{33,22}}{32\sqrt{5}},$$

$$C^{1112,0}_{22,3313} = \frac{1}{96}\sqrt{7}C^{60}_{00,00} + \frac{5}{96}\sqrt{\frac{7}{3}}C^{60}_{00,20} - \frac{1}{32}\sqrt{\frac{7}{15}}C^{62}_{00,22} - \frac{1}{288}\sqrt{7}C^{51}_{11,00} + \frac{1}{96}\sqrt{\frac{7}{3}}C^{51}_{11,20} + \frac{1}{96}\sqrt{\frac{7}{15}}C^{51}_{11,22} - \frac{9}{160}C^{53}_{11,22} - \frac{1}{288}\sqrt{7}C^{40}_{20,00} - \frac{5}{288}\sqrt{\frac{7}{3}}C^{40}_{20,20} - \frac{1}{288}\sqrt{\frac{7}{15}}C^{42}_{20,22} + \frac{1}{288}\sqrt{\frac{7}{5}}C^{42}_{22,00} + \frac{1}{288}\sqrt{\frac{35}{3}}C^{42}_{22,20} + \frac{11}{288}\sqrt{\frac{7}{15}}C^{40}_{22,22} - \frac{1}{72}\sqrt{\frac{5}{3}}C^{42}_{22,22} + \frac{1}{160}\sqrt{\frac{3}{7}}C^{44}_{22,22} + \frac{1}{288}\sqrt{7}C^{31}_{31,00} - \frac{1}{96}\sqrt{\frac{7}{3}}C^{31}_{31,20} - \frac{1}{96}\sqrt{\frac{7}{15}}C^{31}_{31,22} + \frac{9}{160}C^{33}_{31,22} - \frac{1}{160}\sqrt{3}C^{33}_{33,00} + \frac{3}{160}C^{33}_{33,20} - \frac{33}{160}\sqrt{\frac{3}{10}}C^{33}_{33,22},$$

$$C^{1112,1}_{22,3313} = \frac{1}{32}\sqrt{\frac{7}{3}}C^{60}_{00,00} + \frac{1}{96}\sqrt{7}C^{60}_{00,20} + \frac{1}{32}\sqrt{\frac{7}{5}}C^{62}_{00,22} - \frac{1}{96}\sqrt{\frac{7}{3}}C^{51}_{11,00} - \frac{1}{288}\sqrt{7}C^{51}_{11,20} + \frac{1}{288}\sqrt{\frac{7}{5}}C^{51}_{11,22} - \frac{3}{160}\sqrt{3}C^{53}_{11,22} - \frac{1}{96}\sqrt{\frac{7}{3}}C^{40}_{20,00} - \frac{1}{288}\sqrt{7}C^{40}_{20,20} + \frac{1}{288}\sqrt{\frac{7}{5}}C^{42}_{20,22} + \frac{1}{96}\sqrt{\frac{7}{15}}C^{42}_{22,00} + \frac{1}{288}\sqrt{\frac{7}{5}}C^{42}_{22,20} - \frac{11}{288}\sqrt{\frac{7}{5}}C^{40}_{22,22} + \frac{1}{72}\sqrt{5}C^{42}_{22,22} - \frac{3C^{44}_{22,22}}{160\sqrt{7}} + \frac{1}{96}\sqrt{\frac{7}{3}}C^{31}_{31,00} + \frac{1}{288}\sqrt{7}C^{31}_{31,20} - \frac{1}{288}\sqrt{\frac{7}{5}}C^{31}_{31,22} + \frac{3}{160}\sqrt{3}C^{33}_{31,22} - \frac{3}{160}C^{33}_{33,00} - \frac{1}{160}\sqrt{3}C^{33}_{33,20} - \frac{33C^{33}_{33,22}}{160\sqrt{10}},$$

$$C^{1112,0}_{22,3314} = -\frac{1}{32}\sqrt{3}C^{60}_{00,00} - \frac{5}{32}C^{60}_{00,20} - \frac{C^{62}_{00,22}}{32\sqrt{5}} + \frac{C^{51}_{11,00}}{32\sqrt{3}} - \frac{1}{32}C^{51}_{11,20} - \frac{C^{51}_{11,22}}{32\sqrt{5}} - \frac{3}{160}\sqrt{\frac{3}{7}}C^{53}_{11,22} + \frac{C^{40}_{20,00}}{32\sqrt{3}} + \frac{5}{96}C^{40}_{20,20} + \frac{C^{42}_{20,22}}{96\sqrt{5}} - \frac{C^{42}_{22,00}}{32\sqrt{15}} - \frac{1}{96}\sqrt{5}C^{42}_{22,20} + \frac{C^{40}_{22,22}}{96\sqrt{5}} - \frac{C^{42}_{22,22}}{24\sqrt{35}} - \frac{C^{44}_{22,22}}{1120} - \frac{C^{31}_{31,00}}{32\sqrt{3}} + \frac{1}{32}C^{31}_{31,20} + \frac{C^{31}_{31,22}}{32\sqrt{5}} + \frac{3}{160}\sqrt{\frac{3}{7}}C^{33}_{31,22} + \frac{9C^{33}_{33,00}}{160\sqrt{7}} - \frac{9}{160}\sqrt{\frac{3}{7}}C^{33}_{33,20} - \frac{9}{160}\sqrt{\frac{7}{10}}C^{33}_{33,22},$$

$$C^{1112,1}_{22,3314} = -\frac{3}{32}C^{60}_{00,00} - \frac{1}{32}\sqrt{3}C^{60}_{00,20} + \frac{1}{32}\sqrt{\frac{3}{5}}C^{62}_{00,22} + \frac{1}{32}C^{51}_{11,00} + \frac{C^{51}_{11,20}}{32\sqrt{3}} - \frac{C^{51}_{11,22}}{32\sqrt{15}} - \frac{3C^{53}_{11,22}}{160\sqrt{7}} + \frac{1}{32}C^{40}_{20,00} + \frac{C^{40}_{20,20}}{32\sqrt{3}} - \frac{C^{42}_{20,22}}{32\sqrt{15}} - \frac{C^{42}_{22,00}}{32\sqrt{5}} - \frac{C^{42}_{22,20}}{32\sqrt{15}} - \frac{C^{40}_{22,22}}{32\sqrt{15}} + \frac{C^{42}_{22,22}}{8\sqrt{105}} + \frac{\sqrt{3}C^{44}_{22,22}}{1120} - \frac{1}{32}C^{31}_{31,00} - \frac{C^{31}_{31,20}}{32\sqrt{3}} + \frac{C^{31}_{31,22}}{32\sqrt{15}} + \frac{3C^{33}_{31,22}}{160\sqrt{7}} + \frac{9}{160}\sqrt{\frac{3}{7}}C^{33}_{33,00} + \frac{9C^{33}_{33,20}}{160\sqrt{7}} - \frac{3}{160}\sqrt{\frac{21}{10}}C^{33}_{33,22},$$

$$C^{0011,0}_{22,4011} = \frac{21}{640}C^{62}_{00,22} - \frac{7}{640}C^{51}_{11,22} + \frac{27}{640}\sqrt{\frac{21}{5}}C^{53}_{11,22} + \frac{7C^{42}_{20,22}}{1920} - \frac{17C^{40}_{22,22}}{1920} - \frac{1}{192}\sqrt{7}C^{42}_{22,22} + \frac{9C^{44}_{22,22}}{160\sqrt{5}} - \frac{23}{640}C^{31}_{31,22} + \frac{3}{640}\sqrt{\frac{21}{5}}C^{33}_{31,22} - \frac{27}{800}\sqrt{\frac{7}{2}}C^{33}_{33,22},$$

$C^{0011,1}_{22,4011} = -\frac{21}{640}\sqrt{3}C^{62}_{00,22} - \frac{7C^{51}_{11,22}}{640\sqrt{3}} + \frac{27}{640}\sqrt{\frac{7}{5}}C^{53}_{11,22} - \frac{7C^{42}_{20,22}}{640\sqrt{3}} + \frac{17C^{40}_{22,22}}{640\sqrt{3}} + \frac{1}{64}\sqrt{\frac{7}{3}}C^{42}_{22,22} - \frac{9}{160}\sqrt{\frac{3}{5}}C^{44}_{22,22} - \frac{23C^{31}_{31,22}}{640\sqrt{3}} + \frac{3}{640}\sqrt{\frac{7}{5}}C^{33}_{31,22} - \frac{9}{800}\sqrt{\frac{21}{2}}C^{33}_{33,22}$,

$C^{0000,0}_{22,4202} = -\frac{3}{64}\sqrt{5}C^{60}_{00,00} - \frac{1}{64}\sqrt{15}C^{60}_{00,20} - \frac{5}{192}\sqrt{5}C^{51}_{11,00} + \frac{1}{64}\sqrt{\frac{5}{3}}C^{51}_{11,20} + \frac{1}{64}\sqrt{5}C^{40}_{20,00} + \frac{1}{64}\sqrt{\frac{5}{3}}C^{40}_{20,20} - \frac{1}{64}C^{42}_{22,00} - \frac{C^{42}_{22,20}}{64\sqrt{3}} + \frac{5}{192}\sqrt{5}C^{31}_{31,00} - \frac{1}{64}\sqrt{\frac{5}{3}}C^{31}_{31,20} - \frac{3}{64}\sqrt{\frac{15}{7}}C^{33}_{33,00} + \frac{9C^{33}_{33,20}}{64\sqrt{35}}$,

$C^{0000,1}_{22,4202} = \frac{1}{64}\sqrt{15}C^{60}_{00,00} - \frac{3}{64}\sqrt{5}C^{60}_{00,20} - \frac{1}{64}\sqrt{\frac{5}{3}}C^{51}_{11,00} + \frac{1}{64}\sqrt{5}C^{51}_{11,20} - \frac{1}{64}\sqrt{\frac{5}{3}}C^{40}_{20,00} + \frac{1}{64}\sqrt{5}C^{40}_{20,20} + \frac{C^{42}_{22,00}}{64\sqrt{3}} - \frac{1}{64}C^{42}_{22,20} + \frac{1}{64}\sqrt{\frac{5}{3}}C^{31}_{31,00} - \frac{1}{64}\sqrt{5}C^{31}_{31,20} - \frac{9C^{33}_{33,00}}{64\sqrt{35}} + \frac{9}{64}\sqrt{\frac{3}{35}}C^{33}_{33,20}$,

$C^{0011,0}_{22,4211} = \frac{1}{64}\sqrt{3}C^{60}_{00,00} + \frac{5}{64}C^{60}_{00,20} + \frac{3C^{62}_{00,22}}{64\sqrt{5}} - \frac{C^{51}_{11,00}}{64\sqrt{3}} + \frac{1}{64}C^{51}_{11,20} + \frac{C^{51}_{11,22}}{32\sqrt{5}} + \frac{27}{640}\sqrt{\frac{3}{7}}C^{53}_{11,22} - \frac{C^{40}_{20,00}}{64\sqrt{3}} - \frac{5}{192}C^{40}_{20,20} - \frac{C^{42}_{20,22}}{96\sqrt{5}} + \frac{C^{42}_{22,00}}{64\sqrt{15}} + \frac{1}{192}\sqrt{5}C^{42}_{22,20} - \frac{1}{192}\sqrt{5}C^{40}_{22,22} + \frac{1}{96}\sqrt{\frac{7}{5}}C^{42}_{22,22} + \frac{C^{31}_{31,00}}{64\sqrt{3}} - \frac{1}{64}C^{31}_{31,20} - \frac{C^{31}_{31,22}}{32\sqrt{5}} - \frac{27}{640}\sqrt{\frac{3}{7}}C^{33}_{31,22} - \frac{9C^{33}_{33,00}}{320\sqrt{7}} + \frac{9}{320}\sqrt{\frac{3}{7}}C^{33}_{33,20} + \frac{27C^{33}_{33,22}}{40\sqrt{70}}$,

$C^{0011,1}_{22,4211} = \frac{3}{64}C^{60}_{00,00} + \frac{1}{64}\sqrt{3}C^{60}_{00,20} - \frac{3}{64}\sqrt{\frac{3}{5}}C^{62}_{00,22} - \frac{1}{64}C^{51}_{11,00} - \frac{C^{51}_{11,20}}{64\sqrt{3}} + \frac{C^{51}_{11,22}}{32\sqrt{15}} + \frac{27C^{53}_{11,22}}{640\sqrt{7}} - \frac{1}{64}C^{40}_{20,00} - \frac{C^{40}_{20,20}}{64\sqrt{3}} + \frac{C^{42}_{20,22}}{32\sqrt{15}} + \frac{C^{42}_{22,00}}{64\sqrt{5}} + \frac{C^{42}_{22,20}}{64\sqrt{15}} + \frac{1}{64}\sqrt{\frac{5}{3}}C^{40}_{22,22} - \frac{1}{32}\sqrt{\frac{7}{15}}C^{42}_{22,22} + \frac{1}{64}C^{31}_{31,00} + \frac{C^{31}_{31,20}}{64\sqrt{3}} - \frac{C^{31}_{31,22}}{32\sqrt{15}} - \frac{27C^{33}_{31,22}}{640\sqrt{7}} - \frac{9}{320}\sqrt{\frac{3}{7}}C^{33}_{33,00} - \frac{9C^{33}_{33,20}}{320\sqrt{7}} + \frac{9}{40}\sqrt{\frac{3}{70}}C^{33}_{33,22}$,

$C^{0011,0}_{22,4212} = -\frac{1}{64}\sqrt{5}C^{60}_{00,00} - \frac{5}{64}\sqrt{\frac{5}{3}}C^{60}_{00,20} + \frac{1}{64}\sqrt{3}C^{62}_{00,22} + \frac{1}{192}\sqrt{5}C^{51}_{11,00} - \frac{1}{64}\sqrt{\frac{5}{3}}C^{51}_{11,20} + \frac{C^{51}_{11,22}}{32\sqrt{3}} + \frac{27C^{53}_{11,22}}{128\sqrt{35}} + \frac{1}{192}\sqrt{5}C^{40}_{20,00} + \frac{5}{192}\sqrt{\frac{5}{3}}C^{40}_{20,20} - \frac{C^{42}_{20,22}}{96\sqrt{3}} - \frac{1}{192}C^{42}_{22,00} - \frac{5C^{42}_{22,20}}{192\sqrt{3}} - \frac{5C^{40}_{22,22}}{192\sqrt{3}} + \frac{1}{96}\sqrt{\frac{7}{3}}C^{42}_{22,22} - \frac{1}{192}\sqrt{5}C^{31}_{31,00} + \frac{1}{64}\sqrt{\frac{5}{3}}C^{31}_{31,20} - \frac{C^{31}_{31,22}}{32\sqrt{3}} - \frac{27C^{33}_{31,22}}{128\sqrt{35}} + \frac{3}{64}\sqrt{\frac{3}{35}}C^{33}_{33,00} - \frac{9C^{33}_{33,20}}{64\sqrt{35}} + \frac{9}{40}\sqrt{\frac{3}{14}}C^{33}_{33,22}$,

$C^{0011,1}_{22,4212} = -\frac{1}{64}\sqrt{15}C^{60}_{00,00} - \frac{1}{64}\sqrt{5}C^{60}_{00,20} - \frac{3}{64}C^{62}_{00,22} + \frac{1}{64}\sqrt{\frac{5}{3}}C^{51}_{11,00} + \frac{1}{192}\sqrt{5}C^{51}_{11,20} + \frac{1}{96}C^{51}_{11,22} + \frac{9}{128}\sqrt{\frac{3}{35}}C^{53}_{11,22} + \frac{1}{64}\sqrt{\frac{5}{3}}C^{40}_{20,00} + \frac{1}{192}\sqrt{5}C^{40}_{20,20} + \frac{1}{96}C^{42}_{20,22} - \frac{C^{42}_{22,00}}{64\sqrt{3}} - \frac{1}{192}C^{42}_{22,20} + \frac{5}{192}C^{40}_{22,22} - \frac{1}{96}\sqrt{7}C^{42}_{22,22} - \frac{1}{64}\sqrt{\frac{5}{3}}C^{31}_{31,00} - \frac{1}{192}\sqrt{5}C^{31}_{31,20} - \frac{1}{96}C^{31}_{31,22} - \frac{9}{128}\sqrt{\frac{3}{35}}C^{33}_{31,22} + \frac{9C^{33}_{33,00}}{64\sqrt{35}} + \frac{3}{64}\sqrt{\frac{3}{35}}C^{33}_{33,20} + \frac{9C^{33}_{33,22}}{40\sqrt{14}}$,

$C^{0011,0}_{22,4213} = \frac{1}{64}\sqrt{7}C^{60}_{00,00} + \frac{5}{64}\sqrt{\frac{7}{3}}C^{60}_{00,20} + \frac{1}{32}\sqrt{\frac{3}{35}}C^{62}_{00,22} - \frac{1}{192}\sqrt{7}C^{51}_{11,00} + \frac{1}{64}\sqrt{\frac{7}{3}}C^{51}_{11,20} + \frac{C^{51}_{11,22}}{16\sqrt{105}} + \frac{27C^{53}_{11,22}}{2240} - \frac{1}{192}\sqrt{7}C^{40}_{20,00} - \frac{5}{192}\sqrt{\frac{7}{3}}C^{40}_{20,20} - \frac{C^{42}_{20,22}}{48\sqrt{105}} + \frac{1}{192}\sqrt{\frac{7}{5}}C^{42}_{22,00} + \frac{1}{192}\sqrt{\frac{35}{3}}C^{42}_{22,20} - \frac{1}{96}\sqrt{\frac{5}{21}}C^{40}_{22,22} + \frac{C^{42}_{22,22}}{48\sqrt{15}} + \frac{1}{192}\sqrt{7}C^{31}_{31,00} - \frac{1}{64}\sqrt{\frac{7}{3}}C^{31}_{31,20} - \frac{C^{31}_{31,22}}{16\sqrt{105}} - \frac{27C^{33}_{31,22}}{2240} - \frac{3}{320}\sqrt{3}C^{33}_{33,00} + \frac{9}{320}C^{33}_{33,20} + \frac{9}{140}\sqrt{\frac{3}{10}}C^{33}_{33,22}$,

$C^{0011,1}_{22,4213} = \frac{1}{64}\sqrt{21}C^{60}_{00,00} + \frac{1}{64}\sqrt{7}C^{60}_{00,20} - \frac{3C^{62}_{00,22}}{32\sqrt{35}} - \frac{1}{64}\sqrt{\frac{7}{3}}C^{51}_{11,00} - \frac{1}{192}\sqrt{7}C^{51}_{11,20} + \frac{C^{51}_{11,22}}{48\sqrt{35}} + \frac{9\sqrt{3}C^{53}_{11,22}}{2240} - \frac{1}{64}\sqrt{\frac{7}{3}}C^{40}_{20,00} - \frac{1}{192}\sqrt{7}C^{40}_{20,20} + \frac{C^{42}_{20,22}}{48\sqrt{35}} + \frac{1}{64}\sqrt{\frac{7}{15}}C^{42}_{22,00} + \frac{1}{192}\sqrt{\frac{7}{5}}C^{42}_{22,20} + \frac{1}{96}\sqrt{\frac{5}{7}}C^{40}_{22,22} - \frac{C^{42}_{22,22}}{48\sqrt{5}} + \frac{1}{64}\sqrt{\frac{7}{3}}C^{31}_{31,00} + \frac{1}{192}\sqrt{7}C^{31}_{31,20} - \frac{C^{31}_{31,22}}{48\sqrt{35}} - \frac{9\sqrt{3}C^{33}_{31,22}}{2240} - \frac{9}{320}C^{33}_{33,00} -$

$\frac{3}{320}\sqrt{3}C^{33}_{33,20} + \frac{9C^{33}_{33,22}}{140\sqrt{10}}$,

$C^{0011,0}_{22,4413} = \frac{C^{62}_{00,22}}{32\sqrt{5}} + \frac{3C^{51}_{11,22}}{32\sqrt{5}} - \frac{3}{80}\sqrt{\frac{3}{7}}C^{53}_{11,22} - \frac{C^{42}_{20,22}}{32\sqrt{5}} + \frac{C^{40}_{22,22}}{32\sqrt{5}} + \frac{1}{160}C^{44}_{22,22} - \frac{3C^{31}_{31,22}}{32\sqrt{5}} +$
$\frac{3}{80}\sqrt{\frac{3}{7}}C^{33}_{31,22} + \frac{9C^{33}_{33,22}}{160\sqrt{70}}$,

$C^{0011,1}_{22,4413} = -\frac{1}{32}\sqrt{\frac{3}{5}}C^{62}_{00,22} + \frac{1}{32}\sqrt{\frac{3}{5}}C^{51}_{11,22} - \frac{3C^{53}_{11,22}}{80\sqrt{7}} + \frac{1}{32}\sqrt{\frac{3}{5}}C^{42}_{20,22} - \frac{1}{32}\sqrt{\frac{3}{5}}C^{40}_{22,22} -$
$\frac{1}{160}\sqrt{3}C^{44}_{22,22} - \frac{1}{32}\sqrt{\frac{3}{5}}C^{31}_{31,22} + \frac{3C^{33}_{31,22}}{80\sqrt{7}} + \frac{3}{160}\sqrt{\frac{3}{70}}C^{33}_{33,22}$,

$C^{3101,0}_{31,0011} = \frac{21}{160}C^{51}_{11,11} + \frac{9}{160}C^{31}_{31,11} - \frac{27}{200}\sqrt{\frac{7}{2}}C^{33}_{33,11}$,

$C^{3101,1}_{31,0011} = \frac{7}{160}\sqrt{3}C^{51}_{11,11} + \frac{3}{160}\sqrt{3}C^{31}_{31,11} - \frac{9}{200}\sqrt{\frac{21}{2}}C^{33}_{33,11}$,

$C^{2000,0}_{31,1111} = \frac{7}{32}C^{51}_{11,11} + \frac{3}{32}C^{31}_{31,11} - \frac{9}{40}\sqrt{\frac{7}{2}}C^{33}_{33,11}$,

$C^{2000,1}_{31,1111} = \frac{7C^{51}_{11,11}}{32\sqrt{3}} + \frac{1}{32}\sqrt{3}C^{31}_{31,11} - \frac{3}{40}\sqrt{\frac{21}{2}}C^{33}_{33,11}$,

$C^{2202,0}_{31,1111} = -\frac{7C^{51}_{11,11}}{32\sqrt{5}} - \frac{3C^{31}_{31,11}}{32\sqrt{5}} + \frac{9}{40}\sqrt{\frac{7}{10}}C^{33}_{33,11}$,

$C^{2202,1}_{31,1111} = -\frac{7C^{51}_{11,11}}{32\sqrt{15}} - \frac{1}{32}\sqrt{\frac{3}{5}}C^{31}_{31,11} + \frac{3}{40}\sqrt{\frac{21}{10}}C^{33}_{33,11}$,

$C^{2202,0}_{31,1112} = -\frac{7}{32}\sqrt{\frac{3}{5}}C^{51}_{11,11} - \frac{3}{32}\sqrt{\frac{3}{5}}C^{31}_{31,11} + \frac{9}{40}\sqrt{\frac{21}{10}}C^{33}_{33,11}$,

$C^{2202,1}_{31,1112} = -\frac{7C^{51}_{11,11}}{32\sqrt{5}} - \frac{3C^{31}_{31,11}}{32\sqrt{5}} + \frac{9}{40}\sqrt{\frac{7}{10}}C^{33}_{33,11}$,

$C^{1101,0}_{31,2011} = \frac{7}{32}C^{51}_{11,11} + \frac{3}{32}C^{31}_{31,11} - \frac{9}{40}\sqrt{\frac{7}{2}}C^{33}_{33,11}$,

$C^{1101,1}_{31,2011} = \frac{7C^{51}_{11,11}}{32\sqrt{3}} + \frac{1}{32}\sqrt{3}C^{31}_{31,11} - \frac{3}{40}\sqrt{\frac{21}{2}}C^{33}_{33,11}$,

$C^{1101,0}_{31,2211} = -\frac{7C^{51}_{11,11}}{32\sqrt{5}} - \frac{3C^{31}_{31,11}}{32\sqrt{5}} + \frac{9}{40}\sqrt{\frac{7}{10}}C^{33}_{33,11}$,

$C^{1101,1}_{31,2211} = -\frac{7C^{51}_{11,11}}{32\sqrt{15}} - \frac{1}{32}\sqrt{\frac{3}{5}}C^{31}_{31,11} + \frac{3}{40}\sqrt{\frac{21}{10}}C^{33}_{33,11}$,

$C^{1101,0}_{31,2212} = -\frac{7}{32}\sqrt{\frac{3}{5}}C^{51}_{11,11} - \frac{3}{32}\sqrt{\frac{3}{5}}C^{31}_{31,11} + \frac{9}{40}\sqrt{\frac{21}{10}}C^{33}_{33,11}$,

$C^{1101,1}_{31,2212} = -\frac{7C^{51}_{11,11}}{32\sqrt{5}} - \frac{3C^{31}_{31,11}}{32\sqrt{5}} + \frac{9}{40}\sqrt{\frac{7}{10}}C^{33}_{33,11}$,

$C^{0000,0}_{31,3111} = \frac{21}{160}C^{51}_{11,11} + \frac{9}{160}C^{31}_{31,11} - \frac{27}{200}\sqrt{\frac{7}{2}}C^{33}_{33,11}$,

$C^{0000,1}_{31,3111} = \frac{7}{160}\sqrt{3}C^{51}_{11,11} + \frac{3}{160}\sqrt{3}C^{31}_{31,11} - \frac{9}{200}\sqrt{\frac{21}{2}}C^{33}_{33,11}$,

$C^{3303,0}_{33,0011} = \frac{1}{24}\sqrt{\frac{7}{2}}C^{51}_{11,11} - \frac{1}{24}\sqrt{\frac{7}{2}}C^{31}_{31,11} + \frac{3}{80}C^{33}_{33,11}$,

$C^{3303,1}_{33,0011} = \frac{1}{24}\sqrt{\frac{7}{6}}C^{51}_{11,11} - \frac{1}{24}\sqrt{\frac{7}{6}}C^{31}_{31,11} + \frac{1}{80}\sqrt{3}C^{33}_{33,11}$,

$C^{2202,0}_{33,1111} = \frac{1}{8}\sqrt{\frac{7}{3}}C^{51}_{11,11} - \frac{1}{8}\sqrt{\frac{7}{3}}C^{31}_{31,11} + \frac{3}{40}\sqrt{\frac{3}{2}}C^{33}_{33,11}$,

$C^{2202,1}_{33,1111} = \frac{1}{24}\sqrt{7}C^{51}_{11,11} - \frac{1}{24}\sqrt{7}C^{31}_{31,11} + \frac{3C^{33}_{33,11}}{40\sqrt{2}}$,

$C^{2202,0}_{33,1112} = -\frac{1}{8}\sqrt{\frac{7}{6}}C^{51}_{11,11} + \frac{1}{8}\sqrt{\frac{7}{6}}C^{31}_{31,11} - \frac{3}{80}\sqrt{3}C^{33}_{33,11}$,

$C^{2202,1}_{33,1112} = -\frac{1}{24}\sqrt{\frac{7}{2}}C^{51}_{11,11} + \frac{1}{24}\sqrt{\frac{7}{2}}C^{31}_{31,11} - \frac{3}{80}C^{33}_{33,11}$,

$C^{1101,0}_{33,2212} = -\frac{1}{12}\sqrt{7}C^{51}_{11,11} + \frac{1}{12}\sqrt{7}C^{31}_{31,11} - \frac{3C^{33}_{33,11}}{20\sqrt{2}}$,

$C^{1101,1}_{33,2212} = -\frac{1}{12}\sqrt{\frac{7}{3}}C^{51}_{11,11} + \frac{1}{12}\sqrt{\frac{7}{3}}C^{31}_{31,11} - \frac{1}{20}\sqrt{\frac{3}{2}}C^{33}_{33,11}$,

$C^{1101,0}_{33,2213} = \frac{1}{24}\sqrt{\frac{7}{2}}C^{51}_{11,11} - \frac{1}{24}\sqrt{\frac{7}{2}}C^{31}_{31,11} + \frac{3}{80}C^{33}_{33,11}$,

$C^{1101,1}_{33,2213} = \frac{1}{24}\sqrt{\frac{7}{6}}C^{51}_{11,11} - \frac{1}{24}\sqrt{\frac{7}{6}}C^{31}_{31,11} + \frac{1}{80}\sqrt{3}C^{33}_{33,11}$,

$C^{0000,0}_{33,3313} = \frac{1}{24}\sqrt{\frac{7}{2}}C^{51}_{11,11} - \frac{1}{24}\sqrt{\frac{7}{2}}C^{31}_{31,11} + \frac{3}{80}C^{33}_{33,11}$,

$C^{0000,1}_{33,3313} = \frac{1}{24}\sqrt{\frac{7}{6}}C^{51}_{11,11} - \frac{1}{24}\sqrt{\frac{7}{6}}C^{31}_{31,11} + \frac{1}{80}\sqrt{3}C^{33}_{33,11}$,

$C^{1101,0}_{40,1101} = -\frac{21}{256}C^{60}_{00,00} - \frac{7}{256}\sqrt{3}C^{60}_{00,20} + \frac{35}{768}C^{51}_{11,00} - \frac{7C^{51}_{11,20}}{256\sqrt{3}} - \frac{5}{256}C^{40}_{20,00} - \frac{5C^{40}_{20,20}}{256\sqrt{3}} + \frac{7C^{42}_{22,00}}{128\sqrt{5}} + \frac{7C^{42}_{22,20}}{128\sqrt{15}} - \frac{5}{768}C^{31}_{31,00} + \frac{C^{31}_{31,20}}{256\sqrt{3}} - \frac{3}{128}\sqrt{21}C^{33}_{33,00} + \frac{9}{640}\sqrt{7}C^{33}_{33,20}$,

$C^{1101,1}_{40,1101} = \frac{7}{256}\sqrt{3}C^{60}_{00,00} - \frac{21}{256}C^{60}_{00,20} + \frac{7C^{51}_{11,00}}{256\sqrt{3}} - \frac{7}{256}C^{51}_{11,20} + \frac{5C^{40}_{20,00}}{256\sqrt{3}} - \frac{5}{256}C^{40}_{20,20} - \frac{7C^{42}_{22,00}}{128\sqrt{15}} + \frac{7C^{42}_{22,20}}{128\sqrt{5}} - \frac{C^{31}_{31,00}}{256\sqrt{3}} + \frac{1}{256}C^{31}_{31,20} - \frac{9}{640}\sqrt{7}C^{33}_{33,00} + \frac{9}{640}\sqrt{21}C^{33}_{33,20}$,

$C^{1110,0}_{40,1110} = \frac{7C^{60}_{00,00}}{256\sqrt{3}} + \frac{35}{768}C^{60}_{00,20} + \frac{7C^{62}_{00,22}}{128\sqrt{5}} + \frac{7C^{51}_{11,00}}{768\sqrt{3}} - \frac{7}{768}C^{51}_{11,20} + \frac{7C^{51}_{11,22}}{384\sqrt{5}} - \frac{9}{640}\sqrt{21}C^{53}_{11,22} + \frac{5C^{40}_{20,00}}{768\sqrt{3}} + \frac{25C^{40}_{20,20}}{2304} + \frac{7C^{42}_{20,22}}{1152\sqrt{5}} - \frac{7C^{42}_{22,00}}{384\sqrt{15}} - \frac{7\sqrt{5}C^{42}_{22,20}}{1152} - \frac{17C^{40}_{22,22}}{1152\sqrt{5}} - \frac{1}{576}\sqrt{35}C^{42}_{22,22} + \frac{3}{160}C^{44}_{22,22} - \frac{C^{31}_{31,00}}{768\sqrt{3}} + \frac{1}{768}C^{31}_{31,20} + \frac{23C^{31}_{31,22}}{384\sqrt{5}} - \frac{1}{640}\sqrt{21}C^{33}_{31,22} - \frac{3}{640}\sqrt{7}C^{33}_{33,00} + \frac{3}{640}\sqrt{21}C^{33}_{33,20} + \frac{9}{160}\sqrt{\frac{7}{10}}C^{33}_{33,22}$,

$C^{1110,1}_{40,1110} = \frac{7}{256}C^{60}_{00,00} + \frac{7C^{60}_{00,20}}{256\sqrt{3}} - \frac{7}{128}\sqrt{\frac{3}{5}}C^{62}_{00,22} + \frac{7}{768}C^{51}_{11,00} + \frac{7C^{51}_{11,20}}{768\sqrt{3}} + \frac{7C^{51}_{11,22}}{384\sqrt{15}} - \frac{9}{640}\sqrt{7}C^{53}_{11,22} + \frac{5}{768}C^{40}_{20,00} + \frac{5C^{40}_{20,20}}{768\sqrt{3}} - \frac{7C^{42}_{20,22}}{384\sqrt{15}} - \frac{7C^{42}_{22,00}}{384\sqrt{5}} - \frac{7C^{42}_{22,20}}{384\sqrt{15}} + \frac{17C^{40}_{22,22}}{384\sqrt{15}} + \frac{1}{192}\sqrt{\frac{35}{3}}C^{42}_{22,22} - \frac{3}{160}\sqrt{3}C^{44}_{22,22} - \frac{1}{768}C^{31}_{31,00} - \frac{C^{31}_{31,20}}{768\sqrt{3}} + \frac{23C^{31}_{31,22}}{384\sqrt{15}} - \frac{1}{640}\sqrt{7}C^{33}_{31,22} - \frac{3}{640}\sqrt{21}C^{33}_{33,00} - \frac{3}{640}\sqrt{7}C^{33}_{33,20} + \frac{3}{160}\sqrt{\frac{21}{10}}C^{33}_{33,22}$,

$C^{1111,0}_{40,1111} = \frac{7}{256}C^{60}_{00,00} + \frac{35C^{60}_{00,20}}{256\sqrt{3}} - \frac{7}{256}\sqrt{\frac{3}{5}}C^{62}_{00,22} + \frac{7}{768}C^{51}_{11,00} - \frac{7C^{51}_{11,20}}{256\sqrt{3}} - \frac{7C^{51}_{11,22}}{256\sqrt{15}} + \frac{27\sqrt{7}C^{53}_{11,22}}{1280} + \frac{5}{768}C^{40}_{20,00} + \frac{25C^{40}_{20,20}}{768\sqrt{3}} - \frac{7C^{42}_{20,22}}{768\sqrt{15}} - \frac{7C^{42}_{22,00}}{384\sqrt{5}} - \frac{7}{384}\sqrt{\frac{5}{3}}C^{42}_{22,20} + \frac{17C^{40}_{22,22}}{768\sqrt{15}} + \frac{1}{384}\sqrt{\frac{35}{3}}C^{42}_{22,22} - \frac{3}{320}\sqrt{3}C^{44}_{22,22} - \frac{1}{768}C^{31}_{31,00} + \frac{C^{31}_{31,20}}{256\sqrt{3}} - \frac{23C^{31}_{31,22}}{256\sqrt{15}} + \frac{3\sqrt{7}C^{33}_{31,22}}{1280} - \frac{3}{640}\sqrt{21}C^{33}_{33,00} + \frac{9}{640}\sqrt{7}C^{33}_{33,20} - \frac{9}{320}\sqrt{\frac{21}{10}}C^{33}_{33,22}$,

$C^{1111,1}_{40,1111} = \frac{7}{256}\sqrt{3}C^{60}_{00,00} + \frac{7}{256}C^{60}_{00,20} + \frac{21C^{62}_{00,22}}{256\sqrt{5}} + \frac{7C^{51}_{11,00}}{256\sqrt{3}} + \frac{7}{768}C^{51}_{11,20} - \frac{7C^{51}_{11,22}}{768\sqrt{5}} + \frac{9\sqrt{21}C^{53}_{11,22}}{1280} + \frac{5C^{40}_{20,00}}{256\sqrt{3}} + \frac{5}{768}C^{40}_{20,20} + \frac{7C^{42}_{20,22}}{768\sqrt{5}} - \frac{7C^{42}_{22,00}}{128\sqrt{15}} - \frac{7C^{42}_{22,20}}{384\sqrt{5}} - \frac{17C^{40}_{22,22}}{768\sqrt{5}} - \frac{1}{384}\sqrt{35}C^{42}_{22,22} + \frac{9}{320}C^{44}_{22,22} - \frac{C^{31}_{31,00}}{256\sqrt{3}} - \frac{1}{768}C^{31}_{31,20} - \frac{23C^{31}_{31,22}}{768\sqrt{5}} + \frac{\sqrt{21}C^{33}_{31,22}}{1280} - \frac{9}{640}\sqrt{7}C^{33}_{33,00} - \frac{3}{640}\sqrt{21}C^{33}_{33,20} - \frac{9}{320}\sqrt{\frac{7}{10}}C^{33}_{33,22}$,

$C^{1112,0}_{40,1112} = \frac{7}{256}\sqrt{\frac{5}{3}}C^{60}_{00,00} + \frac{35}{768}\sqrt{5}C^{60}_{00,20} + \frac{7C^{62}_{00,22}}{1280} + \frac{7}{768}\sqrt{\frac{5}{3}}C^{51}_{11,00} - \frac{7}{768}\sqrt{5}C^{51}_{11,20} + \frac{7C^{51}_{11,22}}{3840} - \frac{9\sqrt{\frac{21}{5}}C^{53}_{11,22}}{1280} + \frac{5}{768}\sqrt{\frac{5}{3}}C^{40}_{20,00} + \frac{25\sqrt{5}C^{40}_{20,20}}{2304} + \frac{7C^{42}_{20,22}}{11520} - \frac{7C^{42}_{22,00}}{384\sqrt{3}} - \frac{35C^{42}_{22,20}}{1152} - \frac{17C^{40}_{22,22}}{11520} - \frac{\sqrt{7}C^{42}_{22,22}}{1152} + \frac{3C^{44}_{22,22}}{320\sqrt{5}} - \frac{1}{768}\sqrt{\frac{5}{3}}C^{31}_{31,00} + \frac{1}{768}\sqrt{5}C^{31}_{31,20} + \frac{23C^{31}_{31,22}}{3840} - \frac{\sqrt{\frac{21}{5}}C^{33}_{31,22}}{1280} -$

$\frac{3}{128}\sqrt{\frac{7}{5}}C^{33}_{33,00}+\frac{3}{128}\sqrt{\frac{21}{5}}C^{33}_{33,20}+\frac{9\sqrt{\frac{7}{2}}C^{33}_{33,22}}{1600}$,

$C^{1112,1}_{40,1112}=\frac{7}{256}\sqrt{5}C^{60}_{00,00}+\frac{7}{256}\sqrt{\frac{5}{3}}C^{60}_{00,20}-\frac{7\sqrt{3}C^{62}_{00,22}}{1280}+\frac{7}{768}\sqrt{5}C^{51}_{11,00}+\frac{7}{768}\sqrt{\frac{5}{3}}C^{51}_{11,20}+\frac{7C^{51}_{11,22}}{3840\sqrt{3}}-\frac{9\sqrt{\frac{7}{5}}C^{53}_{11,22}}{1280}+\frac{5}{768}\sqrt{5}C^{40}_{20,00}+\frac{5}{768}\sqrt{\frac{5}{3}}C^{40}_{20,20}-\frac{7C^{42}_{20,22}}{3840\sqrt{3}}-\frac{7}{384}C^{42}_{22,00}-\frac{7C^{42}_{22,20}}{384\sqrt{3}}+\frac{17C^{40}_{22,22}}{3840\sqrt{3}}+\frac{1}{384}\sqrt{\frac{7}{3}}C^{42}_{22,22}-\frac{3}{320}\sqrt{\frac{3}{5}}C^{44}_{22,22}-\frac{1}{768}\sqrt{5}C^{31}_{31,00}-\frac{1}{768}\sqrt{\frac{5}{3}}C^{31}_{31,20}+\frac{23C^{31}_{31,22}}{3840\sqrt{3}}-\frac{\sqrt{\frac{7}{5}}C^{33}_{31,22}}{1280}-\frac{3}{128}\sqrt{\frac{21}{5}}C^{33}_{33,00}-\frac{3}{128}\sqrt{\frac{7}{5}}C^{33}_{33,20}+\frac{3\sqrt{\frac{21}{2}}C^{33}_{33,22}}{1600}$,

$C^{0000,0}_{40,2000}=\frac{21}{256}C^{60}_{00,00}+\frac{7}{256}\sqrt{3}C^{60}_{00,20}-\frac{35}{768}C^{51}_{11,00}+\frac{7C^{51}_{11,20}}{256\sqrt{3}}+\frac{5}{256}C^{40}_{20,00}+\frac{5C^{40}_{20,20}}{256\sqrt{3}}-\frac{7C^{42}_{22,00}}{128\sqrt{5}}-\frac{7C^{42}_{22,20}}{128\sqrt{15}}+\frac{5}{768}C^{31}_{31,00}-\frac{C^{31}_{31,20}}{256\sqrt{3}}+\frac{3}{128}\sqrt{21}C^{33}_{33,00}-\frac{9}{640}\sqrt{7}C^{33}_{33,20}$,

$C^{0000,1}_{40,2000}=-\frac{7}{256}\sqrt{3}C^{60}_{00,00}+\frac{21}{256}C^{60}_{00,20}-\frac{7C^{51}_{11,00}}{256\sqrt{3}}+\frac{7}{256}C^{51}_{11,20}-\frac{5C^{40}_{20,00}}{256\sqrt{3}}+\frac{5}{256}C^{40}_{20,20}+\frac{7C^{42}_{22,00}}{128\sqrt{15}}-\frac{7C^{42}_{22,20}}{128\sqrt{5}}+\frac{C^{31}_{31,00}}{256\sqrt{3}}-\frac{1}{256}C^{31}_{31,20}+\frac{9}{640}\sqrt{7}C^{33}_{33,00}-\frac{9}{640}\sqrt{21}C^{33}_{33,20}$,

$C^{0011,0}_{40,2011}=-\frac{7}{256}\sqrt{3}C^{60}_{00,00}-\frac{35}{256}C^{60}_{00,20}-\frac{7C^{51}_{11,00}}{256\sqrt{3}}+\frac{7}{256}C^{51}_{11,20}-\frac{5C^{40}_{20,00}}{256\sqrt{3}}-\frac{25}{768}C^{40}_{20,20}+\frac{7C^{42}_{22,00}}{128\sqrt{15}}+\frac{7}{384}\sqrt{5}C^{42}_{22,20}+\frac{C^{31}_{31,00}}{256\sqrt{3}}-\frac{1}{256}C^{31}_{31,20}+\frac{9}{640}\sqrt{7}C^{33}_{33,00}-\frac{9}{640}\sqrt{21}C^{33}_{33,20}$,

$C^{0011,1}_{40,2011}=-\frac{21}{256}C^{60}_{00,00}-\frac{7}{256}\sqrt{3}C^{60}_{00,20}-\frac{7}{256}C^{51}_{11,00}-\frac{7C^{51}_{11,20}}{256\sqrt{3}}-\frac{5}{256}C^{40}_{20,00}-\frac{5C^{40}_{20,20}}{256\sqrt{3}}+\frac{7C^{42}_{22,00}}{128\sqrt{5}}+\frac{7C^{42}_{22,20}}{128\sqrt{15}}+\frac{1}{256}C^{31}_{31,00}+\frac{C^{31}_{31,20}}{256\sqrt{3}}+\frac{9}{640}\sqrt{21}C^{33}_{33,00}+\frac{9}{640}\sqrt{7}C^{33}_{33,20}$,

$C^{0011,0}_{40,2211}=-\frac{21}{640}C^{62}_{00,22}-\frac{7}{640}C^{51}_{11,22}+\frac{27}{640}\sqrt{\frac{21}{5}}C^{53}_{11,22}-\frac{7C^{42}_{20,22}}{1920}+\frac{17C^{40}_{22,22}}{1920}+\frac{1}{192}\sqrt{7}C^{42}_{22,22}-\frac{9C^{44}_{22,22}}{160\sqrt{5}}-\frac{23}{640}C^{31}_{31,22}+\frac{3}{640}\sqrt{\frac{21}{5}}C^{33}_{31,22}-\frac{27}{800}\sqrt{\frac{7}{2}}C^{33}_{33,22}$,

$C^{0011,1}_{40,2211}=\frac{21}{640}\sqrt{3}C^{62}_{00,22}-\frac{7C^{51}_{11,22}}{640\sqrt{3}}+\frac{27}{640}\sqrt{\frac{7}{5}}C^{53}_{11,22}+\frac{7C^{42}_{20,22}}{640\sqrt{3}}-\frac{17C^{40}_{22,22}}{640\sqrt{3}}-\frac{1}{64}\sqrt{\frac{7}{3}}C^{42}_{22,22}+\frac{9}{160}\sqrt{\frac{3}{5}}C^{44}_{22,22}-\frac{23C^{31}_{31,22}}{640\sqrt{3}}+\frac{3}{640}\sqrt{\frac{7}{5}}C^{33}_{31,22}-\frac{9}{800}\sqrt{\frac{21}{2}}C^{33}_{33,22}$,

$C^{1101,0}_{42,1101}=-\frac{3}{64}\sqrt{5}C^{60}_{00,00}-\frac{1}{64}\sqrt{15}C^{60}_{00,20}+\frac{5}{192}\sqrt{5}C^{51}_{11,00}-\frac{1}{64}\sqrt{\frac{5}{3}}C^{51}_{11,20}+\frac{1}{64}\sqrt{5}C^{40}_{20,00}+\frac{1}{64}\sqrt{\frac{5}{3}}C^{40}_{20,20}-\frac{1}{64}C^{42}_{22,00}-\frac{C^{42}_{22,20}}{64\sqrt{3}}-\frac{5}{192}\sqrt{5}C^{31}_{31,00}+\frac{1}{64}\sqrt{\frac{5}{3}}C^{31}_{31,20}+\frac{3}{64}\sqrt{\frac{15}{7}}C^{33}_{33,00}-\frac{9C^{33}_{33,20}}{64\sqrt{35}}$,

$C^{1101,1}_{42,1101}=\frac{1}{64}\sqrt{15}C^{60}_{00,00}-\frac{3}{64}\sqrt{5}C^{60}_{00,20}+\frac{1}{64}\sqrt{\frac{5}{3}}C^{51}_{11,00}-\frac{1}{64}\sqrt{5}C^{51}_{11,20}-\frac{1}{64}\sqrt{\frac{5}{3}}C^{40}_{20,00}+\frac{1}{64}\sqrt{5}C^{40}_{20,20}+\frac{C^{42}_{22,00}}{64\sqrt{3}}-\frac{1}{64}C^{42}_{22,20}-\frac{1}{64}\sqrt{\frac{5}{3}}C^{31}_{31,00}+\frac{1}{64}\sqrt{5}C^{31}_{31,20}+\frac{9C^{33}_{33,00}}{64\sqrt{35}}-\frac{9}{64}\sqrt{\frac{3}{35}}C^{33}_{33,20}$,

$C^{1111,0}_{42,1111}=-\frac{1}{128}\sqrt{5}C^{60}_{00,00}-\frac{5}{128}\sqrt{\frac{5}{3}}C^{60}_{00,20}+\frac{1}{128}\sqrt{3}C^{62}_{00,22}-\frac{1}{384}\sqrt{5}C^{51}_{11,00}+\frac{1}{128}\sqrt{\frac{5}{3}}C^{51}_{11,20}+\frac{C^{51}_{11,22}}{128\sqrt{3}}-\frac{27C^{53}_{11,22}}{128\sqrt{35}}+\frac{1}{384}\sqrt{5}C^{40}_{20,00}+\frac{5}{384}\sqrt{\frac{5}{3}}C^{40}_{20,20}-\frac{5C^{42}_{20,22}}{384\sqrt{3}}-\frac{1}{384}C^{42}_{22,00}-\frac{5C^{42}_{22,20}}{384\sqrt{3}}-\frac{11C^{40}_{22,22}}{384\sqrt{3}}+\frac{C^{42}_{22,22}}{12\sqrt{21}}+\frac{3}{224}\sqrt{\frac{3}{5}}C^{44}_{22,22}+\frac{1}{384}\sqrt{5}C^{31}_{31,00}-\frac{1}{128}\sqrt{\frac{5}{3}}C^{31}_{31,20}+\frac{5C^{31}_{31,22}}{128\sqrt{3}}+\frac{3}{128}\sqrt{\frac{5}{7}}C^{33}_{31,22}-\frac{3}{128}\sqrt{\frac{3}{35}}C^{33}_{33,00}+\frac{9C^{33}_{33,20}}{128\sqrt{35}}-\frac{9}{32}\sqrt{\frac{3}{14}}C^{33}_{33,22}$,

$C^{1111,1}_{42,1111}=-\frac{1}{128}\sqrt{15}C^{60}_{00,00}-\frac{1}{128}\sqrt{5}C^{60}_{00,20}-\frac{3}{128}C^{62}_{00,22}-\frac{1}{128}\sqrt{\frac{5}{3}}C^{51}_{11,00}-\frac{1}{384}\sqrt{5}C^{51}_{11,20}+\frac{1}{384}C^{51}_{11,22}-\frac{9}{128}\sqrt{\frac{3}{35}}C^{53}_{11,22}+\frac{1}{128}\sqrt{\frac{5}{3}}C^{40}_{20,00}+\frac{1}{384}\sqrt{5}C^{40}_{20,20}+\frac{5}{384}C^{42}_{20,22}-\frac{C^{42}_{22,00}}{128\sqrt{3}}-$

$$\frac{1}{384}C^{42}_{22,20}+\frac{11}{384}C^{40}_{22,22}-\frac{C^{42}_{22,22}}{12\sqrt{7}}-\frac{9C^{44}_{22,22}}{224\sqrt{5}}+\frac{1}{128}\sqrt{\frac{5}{3}}C^{31}_{31,00}+\frac{1}{384}\sqrt{5}C^{31}_{31,20}+\frac{5}{384}C^{31}_{31,22}+\frac{1}{128}\sqrt{\frac{15}{7}}C^{33}_{31,22}-\frac{9C^{33}_{33,00}}{128\sqrt{35}}-\frac{3}{128}\sqrt{\frac{3}{35}}C^{33}_{33,20}-\frac{9C^{33}_{33,22}}{32\sqrt{14}},$$

$$C^{1110,0}_{42,1112}=\frac{1}{32}\sqrt{\frac{5}{3}}C^{60}_{00,00}+\frac{5}{96}\sqrt{5}C^{60}_{00,20}+\frac{1}{16}C^{62}_{00,22}+\frac{1}{96}\sqrt{\frac{5}{3}}C^{51}_{11,00}-\frac{1}{96}\sqrt{5}C^{51}_{11,20}-\frac{7}{96}C^{51}_{11,22}-\frac{9}{64}\sqrt{\frac{3}{35}}C^{53}_{11,22}-\frac{1}{96}\sqrt{\frac{5}{3}}C^{40}_{20,00}-\frac{5}{288}\sqrt{5}C^{40}_{20,20}-\frac{1}{288}C^{42}_{20,22}+\frac{C^{42}_{22,00}}{96\sqrt{3}}+\frac{5}{288}C^{42}_{22,20}-\frac{1}{72}C^{40}_{22,22}+\frac{5C^{42}_{22,22}}{144\sqrt{7}}-\frac{3C^{44}_{22,22}}{56\sqrt{5}}-\frac{1}{96}\sqrt{\frac{5}{3}}C^{31}_{31,00}+\frac{1}{96}\sqrt{5}C^{31}_{31,20}+\frac{1}{96}C^{31}_{31,22}+\frac{17}{64}\sqrt{\frac{3}{35}}C^{33}_{31,22}+\frac{3C^{33}_{33,00}}{32\sqrt{35}}-\frac{3}{32}\sqrt{\frac{3}{35}}C^{33}_{33,20}-\frac{9C^{33}_{33,22}}{40\sqrt{14}},$$

$$C^{1110,1}_{42,1112}=\frac{1}{32}\sqrt{5}C^{60}_{00,00}+\frac{1}{32}\sqrt{\frac{5}{3}}C^{60}_{00,20}-\frac{1}{16}\sqrt{3}C^{62}_{00,22}+\frac{1}{96}\sqrt{5}C^{51}_{11,00}+\frac{1}{96}\sqrt{\frac{5}{3}}C^{51}_{11,20}-\frac{7C^{51}_{11,22}}{96\sqrt{3}}-\frac{9C^{53}_{11,22}}{64\sqrt{35}}-\frac{1}{96}\sqrt{5}C^{40}_{20,00}-\frac{1}{96}\sqrt{\frac{5}{3}}C^{40}_{20,20}+\frac{C^{42}_{20,22}}{96\sqrt{3}}+\frac{1}{96}C^{42}_{22,00}+\frac{C^{42}_{22,20}}{96\sqrt{3}}+\frac{C^{40}_{22,22}}{24\sqrt{3}}-\frac{5C^{42}_{22,22}}{48\sqrt{21}}+\frac{3}{56}\sqrt{\frac{3}{5}}C^{44}_{22,22}-\frac{1}{96}\sqrt{5}C^{31}_{31,00}-\frac{1}{96}\sqrt{\frac{5}{3}}C^{31}_{31,20}+\frac{C^{31}_{31,22}}{96\sqrt{3}}+\frac{17C^{33}_{31,22}}{64\sqrt{35}}+\frac{3}{32}\sqrt{\frac{3}{35}}C^{33}_{33,00}+\frac{3C^{33}_{33,20}}{32\sqrt{35}}-\frac{3}{40}\sqrt{\frac{3}{14}}C^{33}_{33,22},$$

$$C^{1111,0}_{42,1112}=\frac{1}{64}\sqrt{15}C^{60}_{00,00}+\frac{5}{64}\sqrt{5}C^{60}_{00,20}-\frac{3}{64}C^{62}_{00,22}+\frac{1}{64}\sqrt{\frac{5}{3}}C^{51}_{11,00}-\frac{1}{64}\sqrt{5}C^{51}_{11,20}+\frac{5}{64}C^{51}_{11,22}-\frac{1}{64}\sqrt{\frac{5}{3}}C^{40}_{20,00}-\frac{5}{192}\sqrt{5}C^{40}_{20,20}-\frac{1}{192}C^{42}_{20,22}+\frac{C^{42}_{22,00}}{64\sqrt{3}}+\frac{5}{192}C^{42}_{22,20}-\frac{1}{192}C^{40}_{22,22}+\frac{C^{42}_{22,22}}{48\sqrt{7}}+\frac{9C^{44}_{22,22}}{112\sqrt{5}}-\frac{1}{64}\sqrt{\frac{5}{3}}C^{31}_{31,00}+\frac{1}{64}\sqrt{5}C^{31}_{31,20}+\frac{1}{64}C^{31}_{31,22}-\frac{3}{16}\sqrt{\frac{3}{35}}C^{33}_{31,22}+\frac{9C^{33}_{33,00}}{64\sqrt{35}}-\frac{9}{64}\sqrt{\frac{3}{35}}C^{33}_{33,20}-\frac{27C^{33}_{33,22}}{80\sqrt{14}},$$

$$C^{1111,1}_{42,1112}=\frac{3}{64}\sqrt{5}C^{60}_{00,00}+\frac{1}{64}\sqrt{15}C^{60}_{00,20}+\frac{3}{64}\sqrt{3}C^{62}_{00,22}+\frac{1}{64}\sqrt{5}C^{51}_{11,00}+\frac{1}{64}\sqrt{\frac{5}{3}}C^{51}_{11,20}+\frac{5C^{51}_{11,22}}{64\sqrt{3}}-\frac{1}{64}\sqrt{5}C^{40}_{20,00}-\frac{1}{64}\sqrt{\frac{5}{3}}C^{40}_{20,20}+\frac{C^{42}_{20,22}}{64\sqrt{3}}+\frac{1}{64}C^{42}_{22,00}+\frac{C^{42}_{22,20}}{64\sqrt{3}}+\frac{C^{40}_{22,22}}{64\sqrt{3}}-\frac{C^{42}_{22,22}}{16\sqrt{21}}-\frac{9}{112}\sqrt{\frac{3}{5}}C^{44}_{22,22}-\frac{1}{64}\sqrt{5}C^{31}_{31,00}-\frac{1}{64}\sqrt{\frac{5}{3}}C^{31}_{31,20}+\frac{C^{31}_{31,22}}{64\sqrt{3}}-\frac{3C^{33}_{31,22}}{16\sqrt{35}}+\frac{9}{64}\sqrt{\frac{3}{35}}C^{33}_{33,00}+\frac{9C^{33}_{33,20}}{64\sqrt{35}}-\frac{9}{80}\sqrt{\frac{3}{14}}C^{33}_{33,22},$$

$$C^{1112,0}_{42,1112}=\frac{1}{128}\sqrt{\frac{35}{3}}C^{60}_{00,00}+\frac{5}{384}\sqrt{35}C^{60}_{00,20}+\frac{5C^{62}_{00,22}}{128\sqrt{7}}+\frac{1}{384}\sqrt{\frac{35}{3}}C^{51}_{11,00}-\frac{1}{384}\sqrt{35}C^{51}_{11,20}-\frac{31C^{51}_{11,22}}{384\sqrt{7}}+\frac{9}{896}\sqrt{\frac{3}{5}}C^{53}_{11,22}-\frac{1}{384}\sqrt{\frac{35}{3}}C^{40}_{20,00}-\frac{5\sqrt{35}C^{40}_{20,20}}{1152}+\frac{11C^{42}_{20,22}}{1152\sqrt{7}}+\frac{1}{384}\sqrt{\frac{7}{3}}C^{42}_{22,00}+\frac{5\sqrt{7}C^{42}_{22,20}}{1152}+\frac{17C^{40}_{22,22}}{1152\sqrt{7}}-\frac{1}{144}C^{42}_{22,22}-\frac{3C^{44}_{22,22}}{32\sqrt{35}}-\frac{1}{384}\sqrt{\frac{35}{3}}C^{31}_{31,00}+\frac{1}{384}\sqrt{35}C^{31}_{31,20}-\frac{11C^{31}_{31,22}}{384\sqrt{7}}+\frac{19}{896}\sqrt{\frac{3}{5}}C^{33}_{31,22}+\frac{3C^{33}_{33,00}}{128\sqrt{5}}-\frac{3}{128}\sqrt{\frac{3}{5}}C^{33}_{33,20}+\frac{99C^{33}_{33,22}}{1120\sqrt{2}},$$

$$C^{1112,1}_{42,1112}=\frac{1}{128}\sqrt{35}C^{60}_{00,00}+\frac{1}{128}\sqrt{\frac{35}{3}}C^{60}_{00,20}-\frac{5}{128}\sqrt{\frac{3}{7}}C^{62}_{00,22}+\frac{1}{384}\sqrt{35}C^{51}_{11,00}+\frac{1}{384}\sqrt{\frac{35}{3}}C^{51}_{11,20}-\frac{31C^{51}_{11,22}}{384\sqrt{21}}+\frac{9C^{53}_{11,22}}{896\sqrt{5}}-\frac{1}{384}\sqrt{35}C^{40}_{20,00}-\frac{1}{384}\sqrt{\frac{35}{3}}C^{40}_{20,20}-\frac{11C^{42}_{20,22}}{384\sqrt{21}}+\frac{1}{384}\sqrt{7}C^{42}_{22,00}+\frac{1}{384}\sqrt{\frac{7}{3}}C^{42}_{22,20}-\frac{17C^{40}_{22,22}}{384\sqrt{21}}+\frac{C^{42}_{22,22}}{48\sqrt{3}}+\frac{3}{32}\sqrt{\frac{3}{35}}C^{44}_{22,22}-\frac{1}{384}\sqrt{35}C^{31}_{31,00}-\frac{1}{384}\sqrt{\frac{35}{3}}C^{31}_{31,20}-\frac{11C^{31}_{31,22}}{384\sqrt{21}}+\frac{19C^{33}_{31,22}}{896\sqrt{5}}+\frac{3}{128}\sqrt{\frac{3}{5}}C^{33}_{33,00}+\frac{3C^{33}_{33,20}}{128\sqrt{5}}+\frac{33\sqrt{\frac{3}{2}}C^{33}_{33,22}}{1120},$$

$$C^{0011,0}_{42,2011}=-\frac{3}{64}C^{62}_{00,22}+\frac{5}{64}C^{51}_{11,22}-\frac{1}{192}C^{42}_{20,22}-\frac{1}{192}C^{40}_{22,22}+\frac{C^{42}_{22,22}}{48\sqrt{7}}+\frac{9C^{44}_{22,22}}{112\sqrt{5}}+\frac{1}{64}C^{31}_{31,22}-\frac{3}{16}\sqrt{\frac{3}{35}}C^{33}_{31,22}-\frac{27C^{33}_{33,22}}{80\sqrt{14}},$$

$C^{0011,1}_{42,2011} = \frac{3}{64}\sqrt{3}C^{62}_{00,22} + \frac{5C^{51}_{11,22}}{64\sqrt{3}} + \frac{C^{42}_{20,22}}{64\sqrt{3}} + \frac{C^{40}_{22,22}}{64\sqrt{3}} - \frac{C^{42}_{22,22}}{16\sqrt{21}} - \frac{9}{112}\sqrt{\frac{3}{5}}C^{44}_{22,22} + \frac{C^{31}_{31,22}}{64\sqrt{3}} - \frac{3C^{33}_{31,22}}{16\sqrt{35}} - \frac{9}{80}\sqrt{\frac{3}{14}}C^{33}_{33,22},$

$C^{0000,0}_{42,2202} = \frac{3}{64}\sqrt{5}C^{60}_{00,00} + \frac{1}{64}\sqrt{15}C^{60}_{00,20} - \frac{5}{192}\sqrt{5}C^{51}_{11,00} + \frac{1}{64}\sqrt{\frac{5}{3}}C^{51}_{11,20} - \frac{1}{64}\sqrt{5}C^{40}_{20,00} - \frac{1}{64}\sqrt{\frac{5}{3}}C^{40}_{20,20} + \frac{1}{64}C^{42}_{22,00} + \frac{C^{42}_{22,20}}{64\sqrt{3}} + \frac{5}{192}\sqrt{5}C^{31}_{31,00} - \frac{1}{64}\sqrt{\frac{5}{3}}C^{31}_{31,20} - \frac{3}{64}\sqrt{\frac{15}{7}}C^{33}_{33,00} + \frac{9C^{33}_{33,20}}{64\sqrt{35}},$

$C^{0000,1}_{42,2202} = -\frac{1}{64}\sqrt{15}C^{60}_{00,00} + \frac{3}{64}\sqrt{5}C^{60}_{00,20} - \frac{1}{64}\sqrt{\frac{5}{3}}C^{51}_{11,00} + \frac{1}{64}\sqrt{5}C^{51}_{11,20} + \frac{1}{64}\sqrt{\frac{5}{3}}C^{40}_{20,00} - \frac{1}{64}\sqrt{5}C^{40}_{20,20} - \frac{C^{42}_{22,00}}{64\sqrt{3}} + \frac{1}{64}C^{42}_{22,20} + \frac{1}{64}\sqrt{\frac{5}{3}}C^{31}_{31,00} - \frac{1}{64}\sqrt{5}C^{31}_{31,20} - \frac{9C^{33}_{33,00}}{64\sqrt{35}} + \frac{9}{64}\sqrt{\frac{3}{35}}C^{33}_{33,20},$

$C^{0011,0}_{42,2211} = -\frac{1}{64}\sqrt{3}C^{60}_{00,00} - \frac{5}{64}C^{60}_{00,20} - \frac{3C^{62}_{00,22}}{64\sqrt{5}} - \frac{C^{51}_{11,00}}{64\sqrt{3}} + \frac{1}{64}C^{51}_{11,20} + \frac{C^{51}_{11,22}}{32\sqrt{5}} + \frac{27}{640}\sqrt{\frac{3}{7}}C^{53}_{11,22} + \frac{C^{40}_{20,00}}{64\sqrt{3}} + \frac{5}{192}C^{40}_{20,20} + \frac{C^{42}_{20,22}}{96\sqrt{5}} - \frac{C^{42}_{22,00}}{64\sqrt{15}} - \frac{1}{192}\sqrt{5}C^{42}_{22,20} + \frac{1}{192}\sqrt{5}C^{40}_{22,22} - \frac{1}{96}\sqrt{\frac{7}{5}}C^{42}_{22,22} + \frac{C^{31}_{31,00}}{64\sqrt{3}} - \frac{1}{64}C^{31}_{31,20} - \frac{C^{31}_{31,22}}{32\sqrt{5}} - \frac{27}{640}\sqrt{\frac{3}{7}}C^{33}_{31,22} - \frac{9C^{33}_{33,00}}{320\sqrt{7}} + \frac{9}{320}\sqrt{\frac{3}{7}}C^{33}_{33,20} + \frac{27C^{33}_{33,22}}{40\sqrt{70}},$

$C^{0011,1}_{42,2211} = -\frac{3}{64}C^{60}_{00,00} - \frac{1}{64}\sqrt{3}C^{60}_{00,20} + \frac{3}{64}\sqrt{\frac{3}{5}}C^{62}_{00,22} - \frac{1}{64}C^{51}_{11,00} - \frac{C^{51}_{11,20}}{64\sqrt{3}} + \frac{C^{51}_{11,22}}{32\sqrt{15}} + \frac{27C^{53}_{11,22}}{640\sqrt{7}} + \frac{1}{64}C^{40}_{20,00} + \frac{C^{40}_{20,20}}{64\sqrt{3}} - \frac{C^{42}_{20,22}}{32\sqrt{15}} - \frac{C^{42}_{22,00}}{64\sqrt{5}} - \frac{C^{42}_{22,20}}{64\sqrt{15}} - \frac{1}{64}\sqrt{\frac{5}{3}}C^{40}_{22,22} + \frac{1}{32}\sqrt{\frac{7}{15}}C^{42}_{22,22} + \frac{1}{64}C^{31}_{31,00} + \frac{C^{31}_{31,20}}{64\sqrt{3}} - \frac{C^{31}_{31,22}}{32\sqrt{15}} - \frac{27C^{33}_{31,22}}{640\sqrt{7}} - \frac{9}{320}\sqrt{\frac{3}{7}}C^{33}_{33,00} - \frac{9C^{33}_{33,20}}{320\sqrt{7}} + \frac{9}{40}\sqrt{\frac{3}{70}}C^{33}_{33,22},$

$C^{0011,0}_{42,2212} = \frac{1}{64}\sqrt{5}C^{60}_{00,00} + \frac{5}{64}\sqrt{\frac{5}{3}}C^{60}_{00,20} - \frac{1}{64}\sqrt{3}C^{62}_{00,22} + \frac{1}{192}\sqrt{5}C^{51}_{11,00} - \frac{1}{64}\sqrt{\frac{5}{3}}C^{51}_{11,20} + \frac{C^{51}_{11,22}}{32\sqrt{3}} + \frac{27C^{53}_{11,22}}{128\sqrt{35}} - \frac{1}{192}\sqrt{5}C^{40}_{20,00} - \frac{5}{192}\sqrt{\frac{5}{3}}C^{40}_{20,20} + \frac{C^{42}_{20,22}}{96\sqrt{3}} + \frac{1}{192}C^{42}_{22,00} + \frac{5C^{42}_{22,20}}{192\sqrt{3}} + \frac{5C^{40}_{22,22}}{192\sqrt{3}} - \frac{1}{96}\sqrt{\frac{7}{3}}C^{42}_{22,22} - \frac{1}{192}\sqrt{5}C^{31}_{31,00} + \frac{1}{64}\sqrt{\frac{5}{3}}C^{31}_{31,20} - \frac{C^{31}_{31,22}}{32\sqrt{3}} - \frac{27C^{33}_{31,22}}{128\sqrt{35}} + \frac{3}{64}\sqrt{\frac{3}{35}}C^{33}_{33,00} - \frac{9C^{33}_{33,20}}{64\sqrt{35}} + \frac{9}{40}\sqrt{\frac{3}{14}}C^{33}_{33,22},$

$C^{0011,1}_{42,2212} = \frac{1}{64}\sqrt{15}C^{60}_{00,00} + \frac{1}{64}\sqrt{5}C^{60}_{00,20} + \frac{3}{64}C^{62}_{00,22} + \frac{1}{64}\sqrt{\frac{5}{3}}C^{51}_{11,00} + \frac{1}{192}\sqrt{5}C^{51}_{11,20} + \frac{1}{96}C^{51}_{11,22} + \frac{9}{128}\sqrt{\frac{3}{35}}C^{53}_{11,22} - \frac{1}{64}\sqrt{\frac{5}{3}}C^{40}_{20,00} - \frac{1}{192}\sqrt{5}C^{40}_{20,20} - \frac{1}{96}C^{42}_{20,22} + \frac{C^{42}_{22,00}}{64\sqrt{3}} + \frac{1}{192}C^{42}_{22,20} - \frac{5}{192}C^{40}_{22,22} + \frac{1}{96}\sqrt{7}C^{42}_{22,22} - \frac{1}{64}\sqrt{\frac{5}{3}}C^{31}_{31,00} - \frac{1}{192}\sqrt{5}C^{31}_{31,20} - \frac{1}{96}C^{31}_{31,22} - \frac{9}{128}\sqrt{\frac{3}{35}}C^{33}_{31,22} + \frac{9C^{33}_{33,00}}{64\sqrt{35}} + \frac{3}{64}\sqrt{\frac{3}{35}}C^{33}_{33,20} + \frac{9C^{33}_{33,22}}{40\sqrt{14}},$

$C^{0011,0}_{42,2213} = -\frac{1}{64}\sqrt{7}C^{60}_{00,00} - \frac{5}{64}\sqrt{\frac{7}{3}}C^{60}_{00,20} - \frac{1}{32}\sqrt{\frac{3}{35}}C^{62}_{00,22} - \frac{1}{192}\sqrt{7}C^{51}_{11,00} + \frac{1}{64}\sqrt{\frac{7}{3}}C^{51}_{11,20} + \frac{C^{51}_{11,22}}{16\sqrt{105}} + \frac{27C^{53}_{11,22}}{2240} + \frac{1}{192}\sqrt{7}C^{40}_{20,00} + \frac{5}{192}\sqrt{\frac{7}{3}}C^{40}_{20,20} + \frac{C^{42}_{20,22}}{48\sqrt{105}} - \frac{1}{192}\sqrt{\frac{7}{5}}C^{42}_{22,00} - \frac{1}{192}\sqrt{\frac{35}{3}}C^{42}_{22,20} + \frac{1}{96}\sqrt{\frac{5}{21}}C^{40}_{22,22} - \frac{C^{42}_{22,22}}{48\sqrt{15}} + \frac{1}{192}\sqrt{7}C^{31}_{31,00} - \frac{1}{64}\sqrt{\frac{7}{3}}C^{31}_{31,20} - \frac{C^{31}_{31,22}}{16\sqrt{105}} - \frac{27C^{33}_{31,22}}{2240} - \frac{3}{320}\sqrt{3}C^{33}_{33,00} + \frac{9}{320}C^{33}_{33,20} + \frac{9}{140}\sqrt{\frac{3}{10}}C^{33}_{33,22},$

$C^{0011,1}_{42,2213} = -\frac{1}{64}\sqrt{21}C^{60}_{00,00} - \frac{1}{64}\sqrt{7}C^{60}_{00,20} + \frac{3C^{62}_{00,22}}{32\sqrt{35}} - \frac{1}{64}\sqrt{\frac{7}{3}}C^{51}_{11,00} - \frac{1}{192}\sqrt{7}C^{51}_{11,20} + \frac{C^{51}_{11,22}}{48\sqrt{35}} + \frac{9\sqrt{3}C^{53}_{11,22}}{2240} + \frac{1}{64}\sqrt{\frac{7}{3}}C^{40}_{20,00} + \frac{1}{192}\sqrt{7}C^{40}_{20,20} - \frac{C^{42}_{20,22}}{48\sqrt{35}} - \frac{1}{64}\sqrt{\frac{7}{15}}C^{42}_{22,00} - \frac{1}{192}\sqrt{\frac{7}{5}}C^{42}_{22,20} -$

$\frac{1}{96}\sqrt{\frac{5}{7}}C^{40}_{22,22}+\frac{C^{42}_{22,22}}{48\sqrt{5}}+\frac{1}{64}\sqrt{\frac{7}{3}}C^{31}_{31,00}+\frac{1}{192}\sqrt{7}C^{31}_{31,20}-\frac{C^{31}_{31,22}}{48\sqrt{35}}-\frac{9\sqrt{3}C^{33}_{31,22}}{2240}-\frac{9}{320}C^{33}_{33,00}-\frac{3}{320}\sqrt{3}C^{33}_{33,20}+\frac{9C^{33}_{33,22}}{140\sqrt{10}}$,

$C^{1112,0}_{44,1112}=\frac{C^{62}_{00,22}}{32\sqrt{5}}-\frac{3C^{51}_{11,22}}{32\sqrt{5}}+\frac{3}{80}\sqrt{\frac{3}{7}}C^{53}_{11,22}-\frac{C^{42}_{20,22}}{32\sqrt{5}}+\frac{C^{40}_{22,22}}{32\sqrt{5}}+\frac{1}{160}C^{44}_{22,22}+\frac{3C^{31}_{31,22}}{32\sqrt{5}}-\frac{3}{80}\sqrt{\frac{3}{7}}C^{33}_{31,22}-\frac{9C^{33}_{33,22}}{160\sqrt{70}}$,

$C^{1112,1}_{44,1112}=-\frac{1}{32}\sqrt{\frac{3}{5}}C^{62}_{00,22}-\frac{1}{32}\sqrt{\frac{3}{5}}C^{51}_{11,22}+\frac{3C^{53}_{11,22}}{80\sqrt{7}}+\frac{1}{32}\sqrt{\frac{3}{5}}C^{42}_{20,22}-\frac{1}{32}\sqrt{\frac{3}{5}}C^{40}_{22,22}-\frac{1}{160}\sqrt{3}C^{44}_{22,22}+\frac{1}{32}\sqrt{\frac{3}{5}}C^{31}_{31,22}-\frac{3C^{33}_{31,22}}{80\sqrt{7}}-\frac{3}{160}\sqrt{\frac{3}{70}}C^{33}_{33,22}$,

$C^{0011,0}_{44,2213}=-\frac{C^{62}_{00,22}}{32\sqrt{5}}+\frac{3C^{51}_{11,22}}{32\sqrt{5}}-\frac{3}{80}\sqrt{\frac{3}{7}}C^{53}_{11,22}+\frac{C^{42}_{20,22}}{32\sqrt{5}}-\frac{C^{40}_{22,22}}{32\sqrt{5}}-\frac{1}{160}C^{44}_{22,22}-\frac{3C^{31}_{31,22}}{32\sqrt{5}}+\frac{3}{80}\sqrt{\frac{3}{7}}C^{33}_{31,22}+\frac{9C^{33}_{33,22}}{160\sqrt{70}}$,

$C^{0011,1}_{44,2213}=\frac{1}{32}\sqrt{\frac{3}{5}}C^{62}_{00,22}+\frac{1}{32}\sqrt{\frac{3}{5}}C^{51}_{11,22}-\frac{3C^{53}_{11,22}}{80\sqrt{7}}-\frac{1}{32}\sqrt{\frac{3}{5}}C^{42}_{20,22}+\frac{1}{32}\sqrt{\frac{3}{5}}C^{40}_{22,22}+\frac{1}{160}\sqrt{3}C^{44}_{22,22}-\frac{1}{32}\sqrt{\frac{3}{5}}C^{31}_{31,22}+\frac{3C^{33}_{31,22}}{80\sqrt{7}}+\frac{3}{160}\sqrt{\frac{3}{70}}C^{33}_{33,22}$,

$C^{1101,0}_{51,0011}=-\frac{3}{64}C^{51}_{11,11}+\frac{1}{32}\sqrt{\frac{3}{5}}C^{42}_{22,11}-\frac{3}{64}C^{31}_{31,11}-\frac{27C^{33}_{33,11}}{80\sqrt{14}}$,

$C^{1101,1}_{51,0011}=-\frac{1}{64}\sqrt{3}C^{51}_{11,11}-\frac{3C^{42}_{22,11}}{32\sqrt{5}}-\frac{1}{64}\sqrt{3}C^{31}_{31,11}-\frac{9}{80}\sqrt{\frac{3}{14}}C^{33}_{33,11}$,

$C^{0000,0}_{51,1111}=-\frac{3}{64}C^{51}_{11,11}+\frac{1}{32}\sqrt{\frac{3}{5}}C^{42}_{22,11}-\frac{3}{64}C^{31}_{31,11}-\frac{27C^{33}_{33,11}}{80\sqrt{14}}$,

$C^{0000,1}_{51,1111}=-\frac{1}{64}\sqrt{3}C^{51}_{11,11}-\frac{3C^{42}_{22,11}}{32\sqrt{5}}-\frac{1}{64}\sqrt{3}C^{31}_{31,11}-\frac{9}{80}\sqrt{\frac{3}{14}}C^{33}_{33,11}$,

$C^{0000,0}_{60,0000}=-\frac{3}{512}C^{60}_{00,00}-\frac{1}{512}\sqrt{3}C^{60}_{00,20}+\frac{5}{512}C^{51}_{11,00}-\frac{1}{512}\sqrt{3}C^{51}_{11,20}-\frac{3}{512}C^{40}_{20,00}-\frac{1}{512}\sqrt{3}C^{40}_{20,20}-\frac{3C^{42}_{22,00}}{256\sqrt{5}}-\frac{1}{256}\sqrt{\frac{3}{5}}C^{42}_{22,20}+\frac{5}{512}C^{31}_{31,00}-\frac{1}{512}\sqrt{3}C^{31}_{31,20}+\frac{3}{256}\sqrt{\frac{3}{7}}C^{33}_{33,00}-\frac{9C^{33}_{33,20}}{1280\sqrt{7}}$,

$C^{0000,1}_{60,0000}=\frac{1}{512}\sqrt{3}C^{60}_{00,00}-\frac{3}{512}C^{60}_{00,20}+\frac{1}{512}\sqrt{3}C^{51}_{11,00}-\frac{3}{512}C^{51}_{11,20}+\frac{1}{512}\sqrt{3}C^{40}_{20,00}-\frac{3}{512}C^{40}_{20,20}+\frac{1}{256}\sqrt{\frac{3}{5}}C^{42}_{22,00}-\frac{3C^{42}_{22,20}}{256\sqrt{5}}+\frac{1}{512}\sqrt{3}C^{31}_{31,00}-\frac{3}{512}C^{31}_{31,20}+\frac{9C^{33}_{33,00}}{1280\sqrt{7}}-\frac{9\sqrt{\frac{3}{7}}C^{33}_{33,20}}{1280}$,

$C^{0011,0}_{60,0011}=\frac{1}{512}\sqrt{3}C^{60}_{00,00}+\frac{5}{512}C^{60}_{00,20}+\frac{1}{512}\sqrt{3}C^{51}_{11,00}-\frac{3}{512}C^{51}_{11,20}+\frac{1}{512}\sqrt{3}C^{40}_{20,00}+\frac{5}{512}C^{40}_{20,20}+\frac{1}{256}\sqrt{\frac{3}{5}}C^{42}_{22,00}+\frac{1}{256}\sqrt{5}C^{42}_{22,20}+\frac{1}{512}\sqrt{3}C^{31}_{31,00}-\frac{3}{512}C^{31}_{31,20}+\frac{9C^{33}_{33,00}}{1280\sqrt{7}}-\frac{9\sqrt{\frac{3}{7}}C^{33}_{33,20}}{1280}$,

$C^{0011,1}_{60,0011}=\frac{3}{512}C^{60}_{00,00}+\frac{1}{512}\sqrt{3}C^{60}_{00,20}+\frac{3}{512}C^{51}_{11,00}+\frac{1}{512}\sqrt{3}C^{51}_{11,20}+\frac{3}{512}C^{40}_{20,00}+\frac{1}{512}\sqrt{3}C^{40}_{20,20}+\frac{3C^{42}_{22,00}}{256\sqrt{5}}+\frac{1}{256}\sqrt{\frac{3}{5}}C^{42}_{22,20}+\frac{3}{512}C^{31}_{31,00}+\frac{1}{512}\sqrt{3}C^{31}_{31,20}+\frac{9\sqrt{\frac{3}{7}}C^{33}_{33,00}}{1280}+\frac{9C^{33}_{33,20}}{1280\sqrt{7}}$,

$C^{0011,0}_{62,0011}=\frac{1}{256}C^{62}_{00,22}-\frac{3}{256}C^{51}_{11,22}-\frac{9}{256}\sqrt{\frac{3}{35}}C^{53}_{11,22}+\frac{1}{256}C^{42}_{20,22}+\frac{1}{256}C^{40}_{22,22}+\frac{C^{42}_{22,22}}{128\sqrt{7}}+\frac{3C^{44}_{22,22}}{448\sqrt{5}}-\frac{3}{256}C^{31}_{31,22}-\frac{9}{256}\sqrt{\frac{3}{35}}C^{33}_{31,22}-\frac{9C^{33}_{33,22}}{320\sqrt{14}}$,

$C^{0011,1}_{62,0011}=-\frac{1}{256}\sqrt{3}C^{62}_{00,22}-\frac{1}{256}\sqrt{3}C^{51}_{11,22}-\frac{9C^{53}_{11,22}}{256\sqrt{35}}-\frac{1}{256}\sqrt{3}C^{42}_{20,22}-\frac{1}{256}\sqrt{3}C^{40}_{22,22}-\frac{1}{128}\sqrt{\frac{3}{7}}C^{42}_{22,22}-\frac{3}{448}\sqrt{\frac{3}{5}}C^{44}_{22,22}-\frac{1}{256}\sqrt{3}C^{31}_{31,22}-\frac{9C^{33}_{31,22}}{256\sqrt{35}}-\frac{3}{320}\sqrt{\frac{3}{14}}C^{33}_{33,22}$.
