# Supplementary material for: Effective pseudopotential for energy density functionals with higher order derivatives
Source: arXiv:1103.0682 ancillary file (2011-04-17)
Supplement: Supplementary file 2 [file Suppl_T_Section_IIIA.tex.pdf]

**Fourth-order parameters of the pseudopotential as functions of the coupling constants of the isoscalar ($t = 0$) EDF for the case of Galilean invariance. As the set of independent coupling constants of the Galilean-invariant EDF we selected the ones used in Appendix C of Ref. Phys. Rev. C 78, 044326 (2008).**

$$C^{40}_{00,00} = \frac{7C^{0011,0}_{00,4211}}{2\sqrt{15}} + \frac{10}{3}C^{1101,0}_{20,1101} + \frac{4}{3}\sqrt{5}C^{1101,0}_{22,1101} + \frac{4C^{1111,0}_{22,1112}}{3\sqrt{15}} + \frac{8C^{1112,0}_{22,1112}}{\sqrt{105}} - \frac{4C^{0011,0}_{22,2213}}{3\sqrt{7}} + \frac{20}{3}C^{0000,0}_{40,0000} + \frac{4C^{0011,0}_{40,0011}}{\sqrt{3}} + \sqrt{5}C^{2202,0}_{00,2202} + \frac{3C^{2212,0}_{00,2212}}{\sqrt{5}} - \frac{2C^{0011,0}_{20,2011}}{\sqrt{3}},$$

$$C^{40}_{00,20} = -\frac{7C^{0011,0}_{00,4211}}{2\sqrt{5}} - \frac{2C^{1101,0}_{20,1101}}{\sqrt{3}} - \frac{4C^{1101,0}_{22,1101}}{\sqrt{15}} - \frac{4C^{1111,0}_{22,1112}}{3\sqrt{5}} - \frac{8C^{1112,0}_{22,1112}}{\sqrt{35}} + \frac{4C^{0011,0}_{22,2213}}{\sqrt{21}} - \frac{4C^{0000,0}_{40,0000}}{\sqrt{3}} - 4C^{0011,0}_{40,0011} - \sqrt{\frac{3}{5}}C^{2202,0}_{00,2202} - 3\sqrt{\frac{3}{5}}C^{2212,0}_{00,2212} + 2C^{0011,0}_{20,2011},$$

$$C^{42}_{00,22} = -4C^{0011,0}_{00,4211} + 4C^{0011,0}_{20,2211} + \frac{16}{3}C^{1111,0}_{22,1112} + \frac{8C^{1112,0}_{22,1112}}{\sqrt{7}} + 20\sqrt{\frac{5}{21}}C^{0011,0}_{22,2213} - 8C^{0011,0}_{42,0011},$$

$$C^{31}_{11,00} = -\frac{14C^{0011,0}_{00,4211}}{\sqrt{15}} - 16C^{0000,0}_{40,0000} + \frac{16C^{0011,0}_{40,0011}}{\sqrt{3}} + \frac{12C^{2202,0}_{00,2202}}{\sqrt{5}} - \frac{12C^{2212,0}_{00,2212}}{\sqrt{5}},$$

$$C^{31}_{11,11} = \frac{8C^{1101,0}_{11,2212}}{\sqrt{15}} + \frac{8}{3}C^{1101,0}_{31,0011},$$

$$C^{31}_{11,20} = -\frac{14}{3}\sqrt{5}C^{0011,0}_{00,4211} - \frac{16C^{0000,0}_{40,0000}}{\sqrt{3}} + \frac{80}{3}C^{0011,0}_{40,0011} + 4\sqrt{\frac{3}{5}}C^{2202,0}_{00,2202} - 4\sqrt{15}C^{2212,0}_{00,2212},$$

$$C^{31}_{11,22} = -\frac{56}{15}C^{0011,0}_{00,4211} + \frac{8}{5}C^{0011,0}_{20,2211} - \frac{16}{15}C^{1111,0}_{22,1112} + \frac{16C^{1112,0}_{22,1112}}{5\sqrt{7}} - \frac{8C^{0011,0}_{22,2213}}{\sqrt{105}} + \frac{112}{15}C^{0011,0}_{42,0011},$$

$$C^{33}_{11,22} = -\frac{8}{3}\sqrt{\frac{7}{15}}C^{0011,0}_{00,4211} - \frac{8}{3}\sqrt{\frac{7}{15}}C^{0011,0}_{20,2211} + \frac{16}{9}\sqrt{\frac{7}{15}}C^{1111,0}_{22,1112} - \frac{16C^{1112,0}_{22,1112}}{3\sqrt{15}} + \frac{8}{9}C^{0011,0}_{22,2213} + \frac{16}{3}\sqrt{\frac{7}{15}}C^{0011,0}_{42,0011},$$

$$C^{20}_{20,00} = \frac{7}{6}\sqrt{\frac{5}{3}}C^{0011,0}_{00,4211} + \frac{10}{9}C^{1101,0}_{20,1101} - \frac{20}{9}\sqrt{5}C^{1101,0}_{22,1101} - \frac{4}{9}\sqrt{\frac{5}{3}}C^{1111,0}_{22,1112} - \frac{8}{3}\sqrt{\frac{5}{21}}C^{1112,0}_{22,1112} + \frac{20C^{0011,0}_{22,2213}}{9\sqrt{7}} + \frac{100}{9}C^{0000,0}_{40,0000} + \frac{20C^{0011,0}_{40,0011}}{3\sqrt{3}} + \frac{5}{3}\sqrt{5}C^{2202,0}_{00,2202} + \sqrt{5}C^{2212,0}_{00,2212} - \frac{2C^{0011,0}_{20,2011}}{3\sqrt{3}},$$

$$C^{20}_{20,20} = -\frac{7}{6}\sqrt{5}C^{0011,0}_{00,4211} - \frac{2C^{1101,0}_{20,1101}}{3\sqrt{3}} + \frac{4}{3}\sqrt{\frac{5}{3}}C^{1101,0}_{22,1101} + \frac{4}{9}\sqrt{5}C^{1111,0}_{22,1112} + \frac{8}{3}\sqrt{\frac{5}{7}}C^{1112,0}_{22,1112} - \frac{20C^{0011,0}_{22,2213}}{3\sqrt{21}} - \frac{20C^{0000,0}_{40,0000}}{3\sqrt{3}} - \frac{20}{3}C^{0011,0}_{40,0011} - \sqrt{\frac{5}{3}}C^{2202,0}_{00,2202} - \sqrt{15}C^{2212,0}_{00,2212} + \frac{2}{3}C^{0011,0}_{20,2011},$$

$$C^{22}_{20,22} = -\frac{28}{3}C^{0011,0}_{00,4211} - \frac{4}{3}C^{0011,0}_{20,2211} - \frac{64}{9}C^{1111,0}_{22,1112} - \frac{104C^{1112,0}_{22,1112}}{3\sqrt{7}} - \frac{116}{3}\sqrt{\frac{5}{21}}C^{0011,0}_{22,2213} - \frac{56}{3}C^{0011,0}_{42,0011},$$

$$C^{22}_{22,00} = \frac{7C^{0011,0}_{00,4211}}{3\sqrt{3}} - \frac{20}{9}\sqrt{5}C^{1101,0}_{20,1101} + \frac{20}{9}C^{1101,0}_{22,1101} + \frac{4C^{1111,0}_{22,1112}}{9\sqrt{3}} + \frac{8C^{1112,0}_{22,1112}}{3\sqrt{21}} - \frac{4}{9}\sqrt{\frac{5}{7}}C^{0011,0}_{22,2213} + \frac{40}{9}\sqrt{5}C^{0000,0}_{40,0000} + \frac{8}{3}\sqrt{\frac{5}{3}}C^{0011,0}_{40,0011} + \frac{10}{3}C^{2202,0}_{00,2202} + 2C^{2212,0}_{00,2212} + \frac{4}{3}\sqrt{\frac{5}{3}}C^{0011,0}_{20,2011},$$

$$C^{22}_{22,11} = 4C^{1101,0}_{11,2212} - 4\sqrt{\frac{5}{3}}C^{1101,0}_{31,0011},$$

$$C^{22}_{22,20} = -\frac{7}{3}C^{0011,0}_{00,4211} + \frac{4}{3}\sqrt{\frac{5}{3}}C^{1101,0}_{20,1101} - \frac{4C^{1101,0}_{22,1101}}{3\sqrt{3}} - \frac{4}{9}C^{1111,0}_{22,1112} - \frac{8C^{1112,0}_{22,1112}}{3\sqrt{7}} + \frac{4}{3}\sqrt{\frac{5}{21}}C^{0011,0}_{22,2213} - \frac{8}{3}\sqrt{\frac{5}{3}}C^{0000,0}_{40,0000} - \frac{8}{3}\sqrt{5}C^{0011,0}_{40,0011} - \frac{2C^{2202,0}_{00,2202}}{\sqrt{3}} - 2\sqrt{3}C^{2212,0}_{00,2212} - \frac{4}{3}\sqrt{5}C^{0011,0}_{20,2011},$$

$$C^{22}_{22,22} = -\frac{4}{3}\sqrt{7}C^{0011,0}_{00,4211} - \frac{4}{3}\sqrt{7}C^{0011,0}_{20,2211} + \frac{8}{9}\sqrt{7}C^{1111,0}_{22,1112} + \frac{40}{3}C^{1112,0}_{22,1112} + \frac{28}{3}\sqrt{\frac{5}{3}}C^{0011,0}_{22,2213} - \frac{8}{3}\sqrt{7}C^{0011,0}_{42,0011},$$

**Fourth-order parameters of the pseudopotential as functions of the coupling constants of the isovector ($t = 1$) EDF for the case of Galilean invariance. As the set of independent coupling constants of the Galilean-invariant EDF we selected the ones used in Appendix C of Ref. Phys. Rev. C 78, 044326 (2008).**

$$C^{40}_{00,00} = -3\sqrt{\tfrac{3}{5}}C^{2212,1}_{00,2212} - \frac{7C^{0011,1}_{00,4211}}{2\sqrt{5}} - \frac{2C^{1101,1}_{20,1101}}{\sqrt{3}} + 2C^{0011,1}_{20,2011} - \frac{8C^{1112,1}_{22,1112}}{\sqrt{35}} + \frac{4C^{0011,1}_{22,2213}}{\sqrt{21}} - \frac{4C^{0000,1}_{40,0000}}{\sqrt{3}} - 4C^{0011,1}_{40,0011} - \sqrt{\tfrac{3}{5}}C^{2202,1}_{00,2202} - \frac{4C^{1101,1}_{22,1101}}{\sqrt{15}} - \frac{4C^{1111,1}_{22,1112}}{3\sqrt{5}},$$

$$C^{40}_{00,20} = -\frac{3C^{2212,1}_{00,2212}}{\sqrt{5}} - \frac{7C^{0011,1}_{00,4211}}{2\sqrt{15}} + 2C^{1101,1}_{20,1101} + \frac{2C^{0011,1}_{20,2011}}{\sqrt{3}} - \frac{8C^{1112,1}_{22,1112}}{\sqrt{105}} + \frac{4C^{0011,1}_{22,2213}}{3\sqrt{7}} + 4C^{0000,1}_{40,0000} - \frac{4C^{0011,1}_{40,0011}}{\sqrt{3}} + \frac{3C^{2202,1}_{00,2202}}{\sqrt{5}} + \frac{4C^{1101,1}_{22,1101}}{\sqrt{5}} - \frac{4C^{1111,1}_{22,1112}}{3\sqrt{15}},$$

$$C^{42}_{00,22} = \frac{4C^{0011,1}_{00,4211}}{\sqrt{3}} - \frac{4C^{0011,1}_{20,2211}}{\sqrt{3}} - \frac{8C^{1112,1}_{22,1112}}{\sqrt{21}} - \frac{20}{3}\sqrt{\tfrac{5}{7}}C^{0011,1}_{22,2213} + \frac{8C^{0011,1}_{42,0011}}{\sqrt{3}} - \frac{16C^{1111,1}_{22,1112}}{3\sqrt{3}},$$

$$C^{31}_{11,00} = 12\sqrt{\tfrac{3}{5}}C^{2212,1}_{00,2212} + \frac{14C^{0011,1}_{00,4211}}{\sqrt{5}} - \frac{16C^{0000,1}_{40,0000}}{\sqrt{3}} - 16C^{0011,1}_{40,0011} + 4\sqrt{\tfrac{3}{5}}C^{2202,1}_{00,2202},$$

$$C^{31}_{11,11} = \frac{8C^{1101,1}_{11,2212}}{\sqrt{5}} + \frac{8C^{1101,1}_{31,0011}}{\sqrt{3}},$$

$$C^{31}_{11,20} = \frac{12C^{2212,1}_{00,2212}}{\sqrt{5}} + \frac{14C^{0011,1}_{00,4211}}{\sqrt{15}} + 16C^{0000,1}_{40,0000} - \frac{16C^{0011,1}_{40,0011}}{\sqrt{3}} - \frac{12C^{2202,1}_{00,2202}}{\sqrt{5}},$$

$$C^{31}_{11,22} = -\frac{56C^{0011,1}_{00,4211}}{5\sqrt{3}} + \frac{8}{5}\sqrt{3}C^{0011,1}_{20,2211} + \frac{16}{5}\sqrt{\tfrac{3}{7}}C^{1112,1}_{22,1112} - \frac{8C^{0011,1}_{22,2213}}{\sqrt{35}} + \frac{112C^{0011,1}_{42,0011}}{5\sqrt{3}} - \frac{16C^{1111,1}_{22,1112}}{5\sqrt{3}},$$

$$C^{33}_{11,22} = -\frac{8}{3}\sqrt{\tfrac{7}{5}}C^{0011,1}_{00,4211} - \frac{8}{3}\sqrt{\tfrac{7}{5}}C^{0011,1}_{20,2211} - \frac{16C^{1112,1}_{22,1112}}{3\sqrt{5}} + \frac{8C^{0011,1}_{22,2213}}{3\sqrt{3}} + \frac{16}{3}\sqrt{\tfrac{7}{5}}C^{0011,1}_{42,0011} + \frac{16}{9}\sqrt{\tfrac{7}{5}}C^{1111,1}_{22,1112},$$

$$C^{20}_{20,00} = -\sqrt{15}C^{2212,1}_{00,2212} - \frac{7}{6}\sqrt{5}C^{0011,1}_{00,4211} - \frac{2C^{1101,1}_{20,1101}}{3\sqrt{3}} + \frac{2}{3}C^{0011,1}_{20,2011} + \frac{8}{3}\sqrt{\tfrac{5}{7}}C^{1112,1}_{22,1112} - \frac{20C^{0011,1}_{22,2213}}{3\sqrt{21}} - \frac{20C^{0000,1}_{40,0000}}{3\sqrt{3}} - \frac{20}{3}C^{0011,1}_{40,0011} - \sqrt{\tfrac{5}{3}}C^{2202,1}_{00,2202} + \frac{4}{3}\sqrt{\tfrac{5}{3}}C^{1101,1}_{22,1101} + \frac{4}{9}\sqrt{5}C^{1111,1}_{22,1112},$$

$$C^{20}_{20,20} = -\sqrt{5}C^{2212,1}_{00,2212} - \frac{7}{6}\sqrt{\tfrac{5}{3}}C^{0011,1}_{00,4211} + \frac{2}{3}C^{1101,1}_{20,1101} + \frac{2C^{0011,1}_{20,2011}}{3\sqrt{3}} + \frac{8}{3}\sqrt{\tfrac{5}{21}}C^{1112,1}_{22,1112} - \frac{20C^{0011,1}_{22,2213}}{9\sqrt{7}} + \frac{20}{3}C^{0000,1}_{40,0000} - \frac{20C^{0011,1}_{40,0011}}{3\sqrt{3}} + \sqrt{5}C^{2202,1}_{00,2202} - \frac{4}{3}\sqrt{5}C^{1101,1}_{22,1101} + \frac{4}{9}\sqrt{\tfrac{5}{3}}C^{1111,1}_{22,1112},$$

$$C^{22}_{20,22} = \frac{28C^{0011,1}_{00,4211}}{3\sqrt{3}} + \frac{4C^{0011,1}_{20,2211}}{3\sqrt{3}} + \frac{104C^{1112,1}_{22,1112}}{3\sqrt{21}} + \frac{116}{9}\sqrt{\tfrac{5}{7}}C^{0011,1}_{22,2213} + \frac{56C^{0011,1}_{42,0011}}{3\sqrt{3}} + \frac{64C^{1111,1}_{22,1112}}{9\sqrt{3}},$$

$$C^{22}_{22,00} = -2\sqrt{3}C^{2212,1}_{00,2212} - \frac{7}{3}C^{0011,1}_{00,4211} + \frac{4}{3}\sqrt{\tfrac{5}{3}}C^{1101,1}_{20,1101} - \frac{4}{3}\sqrt{5}C^{0011,1}_{20,2011} - \frac{8C^{1112,1}_{22,1112}}{3\sqrt{7}} + \frac{4}{3}\sqrt{\tfrac{5}{21}}C^{0011,1}_{22,2213} - \frac{8}{3}\sqrt{\tfrac{5}{3}}C^{0000,1}_{40,0000} - \frac{8}{3}\sqrt{5}C^{0011,1}_{40,0011} - \frac{2C^{2202,1}_{00,2202}}{\sqrt{3}} - \frac{4C^{1101,1}_{22,1101}}{3\sqrt{3}} - \frac{4}{9}C^{1111,1}_{22,1112},$$

$$C^{22}_{22,11} = -\frac{4C^{1101,1}_{11,2212}}{\sqrt{3}} + \frac{4}{3}\sqrt{5}C^{1101,1}_{31,0011},$$

$$C^{22}_{22,20} = -2C^{2212,1}_{00,2212} - \frac{7C^{0011,1}_{00,4211}}{3\sqrt{3}} - \frac{4}{3}\sqrt{5}C^{1101,1}_{20,1101} - \frac{4}{3}\sqrt{\tfrac{5}{3}}C^{0011,1}_{20,2011} - \frac{8C^{1112,1}_{22,1112}}{3\sqrt{21}} + \frac{4}{9}\sqrt{\tfrac{5}{7}}C^{0011,1}_{22,2213} + \frac{8}{3}\sqrt{5}C^{0000,1}_{40,0000} - \frac{8}{3}\sqrt{\tfrac{5}{3}}C^{0011,1}_{40,0011} + 2C^{2202,1}_{00,2202} + \frac{4}{3}C^{1101,1}_{22,1101} - \frac{4C^{1111,1}_{22,1112}}{9\sqrt{3}},$$

$$C^{22}_{22,22} = \frac{4}{3}\sqrt{\tfrac{7}{3}}C^{0011,1}_{00,4211} + \frac{4}{3}\sqrt{\tfrac{7}{3}}C^{0011,1}_{20,2211} - \frac{40C^{1112,1}_{22,1112}}{3\sqrt{3}} - \frac{28}{9}\sqrt{5}C^{0011,1}_{22,2213} + \frac{8}{3}\sqrt{\tfrac{7}{3}}C^{0011,1}_{42,0011} - \frac{8}{9}\sqrt{\tfrac{7}{3}}C^{1111,1}_{22,1112},$$

**Sixth-order parameters of the pseudopotential as functions of the coupling constants of the isoscalar ($t = 0$) EDF for the case of Galilean invariance. In this case, as the set of independent coupling constants of the Galilean-invariant EDF we made a different choice as compared to the one in Appendix C of Ref. Phys. Rev. C 78, 044326 (2008). The reason for this was that the matrix to invert for that particular choice was found to be singular.**

$$C^{60}_{00,00} = -\frac{5}{2}\sqrt{\frac{3}{7}}C^{3303,0}_{00,3303} - \frac{3}{2}\sqrt{\frac{3}{7}}C^{3313,0}_{00,3313} + \sqrt{\frac{3}{5}}C^{0011,0}_{00,6211} - \frac{2}{5}\sqrt{3}C^{2011,0}_{20,2011} - \sqrt{5}C^{2202,0}_{20,2202} + \frac{2}{7}\sqrt{\frac{5}{3}}C^{1110,0}_{22,3112} + \frac{4}{21}\sqrt{\frac{5}{3}}C^{1111,0}_{22,3112} + \frac{10C^{1101,0}_{22,3303}}{\sqrt{21}} + \frac{4C^{0011,0}_{22,4212}}{3\sqrt{5}} - \frac{10}{3}C^{1101,0}_{40,1101} - 2\sqrt{\frac{3}{5}}C^{1112,0}_{40,1112} - \frac{C^{0011,0}_{40,2211}}{\sqrt{15}} - \frac{4}{3}\sqrt{5}C^{1101,0}_{42,1101} - \frac{8C^{1111,0}_{42,1111}}{3\sqrt{5}} - \frac{2C^{1110,0}_{42,1112}}{\sqrt{15}} - \frac{4C^{0011,0}_{42,2212}}{\sqrt{5}} - \frac{20}{3}C^{0000,0}_{60,0000} - \frac{4C^{0011,0}_{60,0011}}{\sqrt{3}},$$

$$C^{60}_{00,20} = \frac{3C^{3303,0}_{00,3303}}{2\sqrt{7}} + \frac{9C^{3313,0}_{00,3313}}{2\sqrt{7}} - \frac{3C^{0011,0}_{00,6211}}{\sqrt{5}} + \frac{6}{5}C^{2011,0}_{20,2011} + \sqrt{\frac{3}{5}}C^{2202,0}_{20,2202} - \frac{2}{7}\sqrt{5}C^{1110,0}_{22,3112} - \frac{4}{21}\sqrt{5}C^{1111,0}_{22,3112} - \frac{2C^{1101,0}_{22,3303}}{\sqrt{7}} - \frac{4C^{0011,0}_{22,4212}}{\sqrt{15}} + \frac{2C^{1101,0}_{40,1101}}{\sqrt{3}} + \frac{6C^{1112,0}_{40,1112}}{\sqrt{5}} + \frac{C^{0011,0}_{40,2211}}{\sqrt{5}} + \frac{4C^{1101,0}_{42,1101}}{\sqrt{15}} + \frac{8C^{1111,0}_{42,1111}}{\sqrt{15}} + \frac{2C^{1110,0}_{42,1112}}{\sqrt{5}} + 4\sqrt{\frac{3}{5}}C^{0011,0}_{42,2212} + \frac{4C^{0000,0}_{60,0000}}{\sqrt{3}} + 4C^{0011,0}_{60,0011},$$

$$C^{62}_{00,22} = -4C^{0011,0}_{00,6211} + \frac{12}{7}C^{2011,0}_{20,2211} - \frac{15}{7}C^{1110,0}_{22,3112} + \frac{4}{7}C^{1111,0}_{22,3112} + 8\sqrt{\frac{6}{35}}C^{1111,0}_{22,3313} - \frac{14C^{0011,0}_{22,4212}}{5\sqrt{3}} - 4C^{0011,0}_{40,2211} - \frac{80C^{1111,0}_{42,1111}}{7\sqrt{3}} + \frac{22}{7}C^{1110,0}_{42,1112} - 4\sqrt{3}C^{0011,0}_{42,2212} - \frac{48C^{0011,0}_{44,2213}}{7\sqrt{5}} + 8C^{0011,0}_{62,0011},$$

$$C^{51}_{11,00} = -9\sqrt{\frac{3}{7}}C^{3303,0}_{00,3303} + 9\sqrt{\frac{3}{7}}C^{3313,0}_{00,3313} - 6\sqrt{\frac{3}{5}}C^{0011,0}_{00,6211} + \frac{4}{5}\sqrt{3}C^{2011,0}_{20,2011} - \frac{6C^{2202,0}_{20,2202}}{\sqrt{5}} - \frac{4}{7}\sqrt{\frac{5}{3}}C^{1110,0}_{22,3112} - \frac{8}{21}\sqrt{\frac{5}{3}}C^{1111,0}_{22,3112} + 4\sqrt{\frac{3}{7}}C^{1101,0}_{22,3303} - \frac{8C^{0011,0}_{22,4212}}{3\sqrt{5}} + 4C^{1101,0}_{40,1101} - 4\sqrt{\frac{3}{5}}C^{1112,0}_{40,1112} - \frac{2C^{0011,0}_{40,2211}}{\sqrt{15}} + \frac{8C^{1101,0}_{42,1101}}{\sqrt{5}} - \frac{16C^{1111,0}_{42,1111}}{3\sqrt{5}} - \frac{4C^{1110,0}_{42,1112}}{\sqrt{15}} - \frac{8C^{0011,0}_{42,2212}}{\sqrt{5}} + 24C^{0000,0}_{60,0000} - 8\sqrt{3}C^{0011,0}_{60,0011},$$

$$C^{51}_{11,11} = \frac{4}{7}\sqrt{\frac{5}{3}}C^{3101,0}_{11,2212} - \frac{8C^{2202,0}_{31,1112}}{\sqrt{15}} + \frac{48}{5}\sqrt{\frac{2}{7}}C^{1101,0}_{33,2213} - \frac{8}{3}C^{1101,0}_{51,0011},$$

$$C^{51}_{11,20} = -\frac{9C^{3303,0}_{00,3303}}{\sqrt{7}} + \frac{45C^{3313,0}_{00,3313}}{\sqrt{7}} - 6\sqrt{5}C^{0011,0}_{00,6211} + 4C^{2011,0}_{20,2011} - 2\sqrt{\frac{3}{5}}C^{2202,0}_{20,2202} - \frac{20}{21}\sqrt{5}C^{1110,0}_{22,3112} - \frac{40}{63}\sqrt{5}C^{1111,0}_{22,3112} + \frac{4C^{1101,0}_{22,3303}}{\sqrt{7}} - \frac{8}{3}\sqrt{\frac{5}{3}}C^{0011,0}_{22,4212} + \frac{4C^{1101,0}_{40,1101}}{\sqrt{3}} - 4\sqrt{5}C^{1112,0}_{40,1112} - \frac{2}{3}\sqrt{5}C^{0011,0}_{40,2211} + \frac{8C^{1101,0}_{42,1101}}{\sqrt{15}} - \frac{16}{3}\sqrt{\frac{5}{3}}C^{1111,0}_{42,1111} - \frac{4}{3}\sqrt{5}C^{1110,0}_{42,1112} - 8\sqrt{\frac{5}{3}}C^{0011,0}_{42,2212} + 8\sqrt{3}C^{0000,0}_{60,0000} - 40C^{0011,0}_{60,0011},$$

$$C^{51}_{11,22} = -\frac{24}{5}C^{0011,0}_{00,6211} + \frac{8}{7}C^{2011,0}_{20,2211} - \frac{10}{21}C^{1110,0}_{22,3112} - \frac{184}{315}C^{1111,0}_{22,3112} + \frac{48}{5}\sqrt{\frac{6}{35}}C^{1111,0}_{22,3313} - \frac{292C^{0011,0}_{22,4212}}{75\sqrt{3}} - \frac{8}{15}C^{0011,0}_{40,2211} + \frac{992C^{1111,0}_{42,1111}}{105\sqrt{3}} - \frac{172}{105}C^{1110,0}_{42,1112} + \frac{8C^{0011,0}_{42,2212}}{\sqrt{3}} + \frac{288C^{0011,0}_{44,2213}}{35\sqrt{5}} - \frac{48}{5}C^{0011,0}_{62,0011},$$

$$C^{53}_{11,22} = -\frac{16}{3}\sqrt{\frac{7}{15}}C^{0011,0}_{00,6211} - \frac{20}{9}\sqrt{\frac{5}{21}}C^{1110,0}_{22,3112} + \frac{304C^{1111,0}_{22,3112}}{27\sqrt{105}} - \frac{64}{45}\sqrt{2}C^{1111,0}_{22,3313} + \frac{152}{135}\sqrt{\frac{7}{5}}C^{0011,0}_{22,4212} + \frac{16}{3}\sqrt{\frac{7}{15}}C^{0011,0}_{40,2211} - \frac{64C^{1111,0}_{42,1111}}{9\sqrt{35}} - \frac{16C^{1110,0}_{42,1112}}{3\sqrt{105}} - \frac{128C^{0011,0}_{44,2213}}{15\sqrt{21}} - \frac{32}{3}\sqrt{\frac{7}{15}}C^{0011,0}_{62,0011},$$

$$C^{40}_{20,00} = -\frac{5}{2}\sqrt{21}C^{3303,0}_{00,3303} - \frac{3}{2}\sqrt{21}C^{3313,0}_{00,3313} + 7\sqrt{\frac{3}{5}}C^{0011,0}_{00,6211} - \frac{2C^{2011,0}_{20,2011}}{\sqrt{3}} - \frac{5}{3}\sqrt{5}C^{2202,0}_{20,2202} - \frac{2}{3}\sqrt{\frac{5}{3}}C^{1110,0}_{22,3112} - \frac{4}{9}\sqrt{\frac{5}{3}}C^{1111,0}_{22,3112} - \frac{10}{3}\sqrt{\frac{7}{3}}C^{1101,0}_{22,3303} - \frac{28C^{0011,0}_{22,4212}}{9\sqrt{5}} - \frac{50}{9}C^{1101,0}_{40,1101} - 2\sqrt{\frac{5}{3}}C^{1112,0}_{40,1112} - \frac{1}{3}\sqrt{\frac{5}{3}}C^{0011,0}_{40,2211} + \frac{28}{9}\sqrt{5}C^{1101,0}_{42,1101} + \frac{56C^{1111,0}_{42,1111}}{9\sqrt{5}} + \frac{14C^{1110,0}_{42,1112}}{3\sqrt{15}} + \frac{28C^{0011,0}_{42,2212}}{3\sqrt{5}} - \frac{140}{3}C^{0000,0}_{60,0000} -$$

$\frac{28C^{0011,0}_{60,0011}}{\sqrt{3}}$,

$C^{40}_{20,20} = \frac{3}{2}\sqrt{7}C^{3303,0}_{00,3303} + \frac{9}{2}\sqrt{7}C^{3313,0}_{00,3313} - \frac{21C^{0011,0}_{00,6211}}{\sqrt{5}} + 2C^{2011,0}_{20,2011} + \sqrt{\frac{5}{3}}C^{2202,0}_{20,2202} + \frac{2}{3}\sqrt{5}C^{1110,0}_{22,3112} + \frac{4}{9}\sqrt{5}C^{1111,0}_{22,3112} + \frac{2}{3}\sqrt{7}C^{1101,0}_{22,3303} + \frac{28C^{0011,0}_{22,4212}}{3\sqrt{15}} + \frac{10C^{1101,0}_{40,1101}}{3\sqrt{3}} + 2\sqrt{5}C^{1112,0}_{40,1112} + \frac{1}{3}\sqrt{5}C^{0011,0}_{40,2211} - \frac{28C^{1101,0}_{42,1101}}{3\sqrt{15}} - \frac{56C^{1111,0}_{42,1111}}{3\sqrt{15}} - \frac{14C^{1110,0}_{42,1112}}{3\sqrt{5}} - \frac{28C^{0011,0}_{42,2212}}{\sqrt{15}} + \frac{28C^{0000,0}_{60,0000}}{\sqrt{3}} + 28C^{0011,0}_{60,0011}$,

$C^{42}_{20,22} = -24C^{0011,0}_{00,6211} + \frac{8}{7}C^{2011,0}_{20,2211} + \frac{50}{21}C^{1110,0}_{22,3112} + \frac{184}{63}C^{1111,0}_{22,3112} - 48\sqrt{\frac{6}{35}}C^{1111,0}_{22,3313} + \frac{292C^{0011,0}_{22,4212}}{15\sqrt{3}} - \frac{8}{3}C^{0011,0}_{40,2211} - \frac{352C^{1111,0}_{42,1111}}{21\sqrt{3}} - \frac{4}{21}C^{1110,0}_{42,1112} - \frac{8C^{0011,0}_{42,2212}}{\sqrt{3}} + \frac{288C^{0011,0}_{44,2213}}{7\sqrt{5}} + 48C^{0011,0}_{62,0011}$,

$C^{42}_{22,00} = -10\sqrt{\frac{15}{7}}C^{3303,0}_{00,3303} - 6\sqrt{\frac{15}{7}}C^{3313,0}_{00,3313} + 4\sqrt{3}C^{0011,0}_{00,6211} + \frac{8C^{2011,0}_{20,2011}}{\sqrt{15}} + \frac{20}{3}C^{2202,0}_{20,2202} + \frac{20C^{1110,0}_{22,3112}}{21\sqrt{3}} + \frac{40C^{1111,0}_{22,3112}}{63\sqrt{3}} + \frac{20}{3}\sqrt{\frac{5}{21}}C^{1101,0}_{22,3303} + \frac{8}{9}C^{0011,0}_{22,4212} + \frac{40}{9}\sqrt{5}C^{1101,0}_{40,1101} + \frac{8C^{1112,0}_{40,1112}}{\sqrt{3}} + \frac{4C^{0011,0}_{40,2211}}{3\sqrt{3}} - \frac{40}{9}C^{1101,0}_{42,1101} - \frac{16}{9}C^{1111,0}_{42,1111} - \frac{4C^{1110,0}_{42,1112}}{3\sqrt{3}} - \frac{8}{3}C^{0011,0}_{42,2212} - \frac{80}{3}\sqrt{5}C^{0000,0}_{60,0000} - 16\sqrt{\frac{5}{3}}C^{0011,0}_{60,0011}$,

$C^{42}_{22,11} = \frac{40}{7}C^{3101,0}_{11,2212} + 16\sqrt{\frac{5}{3}}C^{1101,0}_{51,0011}$,

$C^{42}_{22,20} = 6\sqrt{\frac{5}{7}}C^{3303,0}_{00,3303} + 18\sqrt{\frac{5}{7}}C^{3313,0}_{00,3313} - 12C^{0011,0}_{00,6211} - \frac{8C^{2011,0}_{20,2011}}{\sqrt{5}} - \frac{4C^{2202,0}_{20,2202}}{\sqrt{3}} - \frac{20}{21}C^{1110,0}_{22,3112} - \frac{40}{63}C^{1111,0}_{22,3112} - \frac{4}{3}\sqrt{\frac{5}{7}}C^{1101,0}_{22,3303} - \frac{8C^{0011,0}_{22,4212}}{3\sqrt{3}} - \frac{8}{3}\sqrt{\frac{5}{3}}C^{1101,0}_{40,1101} - 8C^{1112,0}_{40,1112} - \frac{4}{3}C^{0011,0}_{40,2211} + \frac{8C^{1101,0}_{42,1101}}{3\sqrt{3}} + \frac{16C^{1111,0}_{42,1111}}{3\sqrt{3}} + \frac{4}{3}C^{1110,0}_{42,1112} + \frac{8C^{0011,0}_{42,2212}}{\sqrt{3}} + 16\sqrt{\frac{5}{3}}C^{0000,0}_{60,0000} + 16\sqrt{5}C^{0011,0}_{60,0011}$,

$C^{40}_{22,22} = -\frac{84}{5}C^{0011,0}_{00,6211} + \frac{4}{5}C^{2011,0}_{20,2211} + \frac{5}{3}C^{1110,0}_{22,3112} - \frac{52}{45}C^{1111,0}_{22,3112} + \frac{24}{5}\sqrt{\frac{42}{5}}C^{1111,0}_{22,3313} - \frac{2002C^{0011,0}_{22,4212}}{75\sqrt{3}} + \frac{68}{15}C^{0011,0}_{40,2211} - \frac{272C^{1111,0}_{42,1111}}{15\sqrt{3}} - \frac{26}{15}C^{1110,0}_{42,1112} - \frac{28C^{0011,0}_{42,2212}}{5\sqrt{3}} - \frac{144C^{0011,0}_{44,2213}}{5\sqrt{5}} + \frac{168}{5}C^{0011,0}_{62,0011}$,

$C^{42}_{22,22} = -\frac{48C^{0011,0}_{00,6211}}{\sqrt{7}} - \frac{32C^{2011,0}_{20,2211}}{7\sqrt{7}} - \frac{20C^{1110,0}_{22,3112}}{21\sqrt{7}} - \frac{880C^{1111,0}_{22,3112}}{63\sqrt{7}} + \frac{184C^{0011,0}_{22,4212}}{3\sqrt{21}} + \frac{80C^{0011,0}_{40,2211}}{3\sqrt{7}} + \frac{256C^{1111,0}_{42,1111}}{3\sqrt{21}} + \frac{16C^{1110,0}_{42,1112}}{3\sqrt{7}} + \frac{32C^{0011,0}_{42,2212}}{\sqrt{21}} + \frac{96C^{0011,0}_{62,0011}}{\sqrt{7}}$,

$C^{44}_{22,22} = -\frac{16C^{0011,0}_{00,6211}}{\sqrt{5}} - \frac{48C^{2011,0}_{20,2211}}{7\sqrt{5}} - \frac{20}{21}\sqrt{5}C^{1110,0}_{22,3112} + \frac{304C^{1111,0}_{22,3112}}{63\sqrt{5}} + \frac{8}{5}\sqrt{\frac{14}{3}}C^{1111,0}_{22,3313} - \frac{328C^{0011,0}_{22,4212}}{15\sqrt{15}} - \frac{16C^{0011,0}_{40,2211}}{\sqrt{5}} + \frac{64C^{1111,0}_{42,1111}}{\sqrt{15}} - \frac{8C^{1110,0}_{42,1112}}{\sqrt{5}} + 16\sqrt{\frac{3}{5}}C^{0011,0}_{42,2212} - \frac{16}{5}C^{0011,0}_{44,2213} + \frac{32C^{0011,0}_{62,0011}}{\sqrt{5}}$,

$C^{31}_{31,00} = -\frac{9}{5}\sqrt{21}C^{3303,0}_{00,3303} + \frac{9}{5}\sqrt{21}C^{3313,0}_{00,3313} - \frac{42}{5}\sqrt{\frac{3}{5}}C^{0011,0}_{00,6211} - \frac{4}{25}\sqrt{3}C^{2011,0}_{20,2011} + \frac{6C^{2202,0}_{20,2202}}{5\sqrt{5}} + \frac{4C^{1110,0}_{22,3112}}{\sqrt{15}} + \frac{8C^{1111,0}_{22,3112}}{3\sqrt{15}} - \frac{4}{5}\sqrt{21}C^{1101,0}_{22,3303} + \frac{56C^{0011,0}_{22,4212}}{15\sqrt{5}} - \frac{4}{5}C^{1101,0}_{40,1101} + \frac{4}{5}\sqrt{\frac{3}{5}}C^{1112,0}_{40,1112} + \frac{2C^{0011,0}_{40,2211}}{5\sqrt{15}} - \frac{56C^{1101,0}_{42,1101}}{5\sqrt{5}} + \frac{112C^{1111,0}_{42,1111}}{15\sqrt{5}} + \frac{28C^{1110,0}_{42,1112}}{5\sqrt{15}} + \frac{56C^{0011,0}_{42,2212}}{5\sqrt{5}} + \frac{168}{5}C^{0000,0}_{60,0000} - \frac{56}{5}\sqrt{3}C^{0011,0}_{60,0011}$,

$C^{31}_{31,11} = \frac{4C^{3101,0}_{11,2212}}{\sqrt{15}} - \frac{8}{5}\sqrt{\frac{3}{5}}C^{2202,0}_{31,1112} - \frac{48}{25}\sqrt{14}C^{1101,0}_{33,2213} - \frac{56}{15}C^{1101,0}_{51,0011}$,

$C^{31}_{31,20} = -\frac{9}{5}\sqrt{7}C^{3303,0}_{00,3303} + 9\sqrt{7}C^{3313,0}_{00,3313} - \frac{42C^{0011,0}_{00,6211}}{\sqrt{5}} - \frac{4}{5}C^{2011,0}_{20,2011} + \frac{2}{5}\sqrt{\frac{3}{5}}C^{2202,0}_{20,2202} + \frac{4}{3}\sqrt{5}C^{1110,0}_{22,3112} + \frac{8}{9}\sqrt{5}C^{1111,0}_{22,3112} - \frac{4}{5}\sqrt{7}C^{1101,0}_{22,3303} + \frac{56C^{0011,0}_{22,4212}}{3\sqrt{15}} - \frac{4C^{1101,0}_{40,1101}}{5\sqrt{3}} + \frac{4C^{1112,0}_{40,1112}}{\sqrt{5}} + \frac{2C^{0011,0}_{40,2211}}{3\sqrt{5}} - \frac{56C^{1101,0}_{42,1101}}{5\sqrt{15}} + \frac{112C^{1111,0}_{42,1111}}{3\sqrt{15}} + \frac{28C^{1110,0}_{42,1112}}{3\sqrt{5}} + \frac{56C^{0011,0}_{42,2212}}{\sqrt{15}} + \frac{56}{5}\sqrt{3}C^{0000,0}_{60,0000} - 56C^{0011,0}_{60,0011}$,

$$C^{31}_{31,22} = -\frac{168}{25}C^{0011,0}_{00,6211} + \frac{8}{25}C^{2011,0}_{20,2211} + \frac{22}{15}C^{1110,0}_{22,3112} - \frac{56}{225}C^{1111,0}_{22,3112} - \frac{48}{25}\sqrt{\frac{42}{5}}C^{1111,0}_{22,3313} + \frac{2884C^{0011,0}_{22,4212}}{375\sqrt{3}} - \frac{184}{75}C^{0011,0}_{40,2211} + \frac{352C^{1111,0}_{42,1111}}{75\sqrt{3}} + \frac{4}{75}C^{1110,0}_{42,1112} + \frac{56C^{0011,0}_{42,2212}}{25\sqrt{3}} - \frac{288C^{0011,0}_{44,2213}}{25\sqrt{5}} - \frac{336}{25}C^{0011,0}_{62,0011},$$

$$C^{33}_{31,22} = -\frac{16}{5}\sqrt{\frac{21}{5}}C^{0011,0}_{00,6211} - \frac{64C^{2011,0}_{20,2211}}{5\sqrt{105}} + \frac{4C^{1110,0}_{22,3112}}{3\sqrt{105}} + \frac{208C^{1111,0}_{22,3112}}{45\sqrt{105}} + \frac{64}{25}\sqrt{2}C^{1111,0}_{22,3313} - \frac{1016}{225}\sqrt{\frac{7}{5}}C^{0011,0}_{22,4212} + \frac{16}{15}\sqrt{\frac{7}{15}}C^{0011,0}_{40,2211} - \frac{1216C^{1111,0}_{42,1111}}{45\sqrt{35}} + \frac{368C^{1110,0}_{42,1112}}{15\sqrt{105}} - \frac{64}{15}\sqrt{\frac{7}{5}}C^{0011,0}_{42,2212} + \frac{128}{25}\sqrt{\frac{3}{7}}C^{0011,0}_{44,2213} - \frac{32}{5}\sqrt{\frac{21}{5}}C^{0011,0}_{62,0011},$$

$$C^{33}_{33,00} = -2C^{3303,0}_{00,3303} + 2C^{3313,0}_{00,3313} - \frac{4}{3}\sqrt{\frac{7}{5}}C^{0011,0}_{00,6211} - \frac{8}{15}\sqrt{7}C^{2011,0}_{20,2011} + 4\sqrt{\frac{7}{15}}C^{2202,0}_{20,2202} - \frac{4}{9}\sqrt{\frac{5}{7}}C^{1110,0}_{22,3112} - \frac{8}{27}\sqrt{\frac{5}{7}}C^{1111,0}_{22,3112} + \frac{4}{3}C^{1101,0}_{22,3303} - \frac{8}{9}\sqrt{\frac{7}{15}}C^{0011,0}_{22,4212} - \frac{8}{3}\sqrt{\frac{7}{3}}C^{1101,0}_{40,1101} + \frac{8}{3}\sqrt{\frac{7}{5}}C^{1112,0}_{40,1112} + \frac{4}{9}\sqrt{\frac{7}{5}}C^{0011,0}_{40,2211} + \frac{8}{3}\sqrt{\frac{7}{15}}C^{1101,0}_{42,1101} - \frac{16}{9}\sqrt{\frac{7}{15}}C^{1111,0}_{42,1111} - \frac{4}{9}\sqrt{\frac{7}{5}}C^{1110,0}_{42,1112} - \frac{8}{3}\sqrt{\frac{7}{15}}C^{0011,0}_{42,2212} + \frac{16}{3}\sqrt{\frac{7}{3}}C^{0000,0}_{60,0000} - \frac{16}{9}\sqrt{7}C^{0011,0}_{60,0011},$$

$$C^{33}_{33,11} = \frac{8}{9}\sqrt{\frac{10}{21}}C^{3101,0}_{11,2212} + \frac{16}{9}\sqrt{\frac{14}{15}}C^{2202,0}_{31,1112} + \frac{16}{15}C^{1101,0}_{33,2213} - \frac{16}{27}\sqrt{14}C^{1101,0}_{51,0011},$$

$$C^{33}_{33,20} = -\frac{2C^{3303,0}_{00,3303}}{\sqrt{3}} + \frac{10C^{3313,0}_{00,3313}}{\sqrt{3}} - \frac{4}{3}\sqrt{\frac{35}{3}}C^{0011,0}_{00,6211} - \frac{8}{3}\sqrt{\frac{7}{3}}C^{2011,0}_{20,2011} + \frac{4}{3}\sqrt{\frac{7}{5}}C^{2202,0}_{20,2202} - \frac{20}{9}\sqrt{\frac{5}{21}}C^{1110,0}_{22,3112} - \frac{40}{27}\sqrt{\frac{5}{21}}C^{1111,0}_{22,3112} + \frac{4C^{1101,0}_{22,3303}}{3\sqrt{3}} - \frac{8}{27}\sqrt{35}C^{0011,0}_{22,4212} - \frac{8}{9}\sqrt{7}C^{1101,0}_{40,1101} + \frac{8}{3}\sqrt{\frac{35}{3}}C^{1112,0}_{40,1112} + \frac{4}{9}\sqrt{\frac{35}{3}}C^{0011,0}_{40,2211} + \frac{8}{9}\sqrt{\frac{7}{5}}C^{1101,0}_{42,1101} - \frac{16}{27}\sqrt{35}C^{1111,0}_{42,1111} - \frac{4}{9}\sqrt{\frac{35}{3}}C^{1110,0}_{42,1112} - \frac{8}{9}\sqrt{35}C^{0011,0}_{42,2212} + \frac{16}{9}\sqrt{7}C^{0000,0}_{60,0000} - \frac{80}{9}\sqrt{\frac{7}{3}}C^{0011,0}_{60,0011},$$

$$C^{33}_{33,22} = -\frac{16}{45}\sqrt{14}C^{0011,0}_{00,6211} - \frac{16}{15}\sqrt{\frac{2}{7}}C^{2011,0}_{20,2211} - \frac{4}{9}\sqrt{\frac{2}{7}}C^{1110,0}_{22,3112} - \frac{208}{135}\sqrt{\frac{2}{7}}C^{1111,0}_{22,3112} + \frac{16C^{1111,0}_{22,3313}}{15\sqrt{15}} + \frac{8}{25}\sqrt{42}C^{0011,0}_{22,4212} - \frac{16}{45}\sqrt{14}C^{0011,0}_{40,2211} - \frac{704}{45}\sqrt{\frac{2}{21}}C^{1111,0}_{42,1111} - \frac{8}{45}\sqrt{\frac{2}{7}}C^{1110,0}_{42,1112} - \frac{16}{15}\sqrt{\frac{14}{3}}C^{0011,0}_{42,2212} + \frac{16}{15}\sqrt{\frac{2}{35}}C^{0011,0}_{44,2213} - \frac{32}{45}\sqrt{14}C^{0011,0}_{62,0011}.$$

**Sixth-order parameters of the pseudopotential as functions of the coupling constants of the isovector ($t = 1$) EDF for the case of Galilean invariance. In this case, as the set of independent coupling constants of the Galilean-invariant EDF we made a different choice as compared to the one in Appendix C of Ref. Phys. Rev. C 78, 044326 (2008). The reason for this was that the matrix to invert for that particular choice was found to be singular.**

$$C^{60}_{00,00} = \frac{3C^{3303,1}_{00,3303}}{2\sqrt{7}} + \frac{9C^{3313,1}_{00,3313}}{2\sqrt{7}} - \frac{3C^{0011,1}_{00,6211}}{\sqrt{5}} + \frac{6}{5}C^{2011,1}_{20,2011} + \sqrt{\frac{3}{5}}C^{2202,1}_{20,2202} - \frac{2}{7}\sqrt{5}C^{1110,1}_{22,3112} - \frac{4}{21}\sqrt{5}C^{1111,1}_{22,3112} - \frac{2C^{1101,1}_{22,3303}}{\sqrt{7}} - \frac{4C^{0011,1}_{22,4212}}{\sqrt{15}} + \frac{2C^{1101,1}_{40,1101}}{\sqrt{3}} + \frac{6C^{1112,1}_{40,1112}}{\sqrt{5}} + \frac{C^{0011,1}_{40,2211}}{\sqrt{5}} + \frac{4C^{1101,1}_{42,1101}}{\sqrt{15}} + \frac{8C^{1111,1}_{42,1111}}{\sqrt{15}} + \frac{2C^{1110,1}_{42,1112}}{\sqrt{5}} + 4\sqrt{\frac{3}{5}}C^{0011,1}_{42,2212} + \frac{4C^{0000,1}_{60,0000}}{\sqrt{3}} + 4C^{0011,1}_{60,0011},$$

$$C^{60}_{00,20} = -\frac{3}{2}\sqrt{\frac{3}{7}}C^{3303,1}_{00,3303} + \frac{3}{2}\sqrt{\frac{3}{7}}C^{3313,1}_{00,3313} - \sqrt{\frac{3}{5}}C^{0011,1}_{00,6211} + \frac{2}{5}\sqrt{3}C^{2011,1}_{20,2011} - \frac{3C^{2202,1}_{20,2202}}{\sqrt{5}} - \frac{2}{7}\sqrt{\frac{5}{3}}C^{1110,1}_{22,3112} - \frac{4}{21}\sqrt{\frac{5}{3}}C^{1111,1}_{22,3112} + 2\sqrt{\frac{3}{7}}C^{1101,1}_{22,3303} - \frac{4C^{0011,1}_{22,4212}}{3\sqrt{5}} - 2C^{1101,1}_{40,1101} + 2\sqrt{\frac{3}{5}}C^{1112,1}_{40,1112} +$$

$$\frac{C^{0011,1}_{40,2211}}{\sqrt{15}} - \frac{4C^{1101,1}_{42,1101}}{\sqrt{5}} + \frac{8C^{1111,1}_{42,1111}}{3\sqrt{5}} + \frac{2C^{1110,1}_{42,1112}}{\sqrt{15}} + \frac{4C^{0011,1}_{42,2212}}{\sqrt{5}} - 4C^{0000,1}_{60,0000} + \frac{4C^{0011,1}_{60,0011}}{\sqrt{3}},$$

$$C^{62}_{00,22} = -\frac{8C^{0011,1}_{62,0011}}{\sqrt3} + \frac{4C^{0011,1}_{00,6211}}{\sqrt3} - \frac47\sqrt3 C^{2011,1}_{20,2211} + \frac57\sqrt3 C^{1110,1}_{22,3112} - \frac{4C^{1111,1}_{22,3112}}{7\sqrt3} - 8\sqrt{\frac{2}{35}} C^{1111,1}_{22,3313} + \frac{14}{15}C^{0011,1}_{22,4212} + \frac{4C^{0011,1}_{40,2211}}{\sqrt3} + \frac{80}{21}C^{1111,1}_{42,1111} - \frac{22C^{1110,1}_{42,1112}}{7\sqrt3} + 4C^{0011,1}_{42,2212} + \frac{16}{7}\sqrt{\frac35}C^{0011,1}_{44,2213},$$

$$C^{51}_{11,00} = -\frac{9C^{3303,1}_{00,3303}}{\sqrt7} - \frac{27C^{3313,1}_{00,3313}}{\sqrt7} + \frac{18C^{0011,1}_{00,6211}}{\sqrt5} - \frac{12}{5}C^{2011,1}_{20,2011} - 2\sqrt{\frac35}C^{2202,1}_{20,2202} + \frac47\sqrt5 C^{1110,1}_{22,3112} + \frac{8}{21}\sqrt5 C^{1111,1}_{22,3112} + \frac{4C^{1101,1}_{22,3303}}{\sqrt7} + \frac{8C^{0011,1}_{22,4212}}{\sqrt{15}} + \frac{4C^{1101,1}_{40,1101}}{\sqrt3} + \frac{12C^{1112,1}_{40,1112}}{\sqrt5} + \frac{2C^{0011,1}_{40,2211}}{\sqrt5} + \frac{8C^{1101,1}_{42,1101}}{\sqrt{15}} + \frac{16C^{1111,1}_{42,1111}}{\sqrt{15}} + \frac{4C^{1110,1}_{42,1112}}{\sqrt5} + 8\sqrt{\frac35}C^{0011,1}_{42,2212} + 8\sqrt3 C^{0000,1}_{60,0000} + 24C^{0011,1}_{60,0011},$$

$$C^{51}_{11,11} = \frac47\sqrt5 C^{3101,1}_{11,2212} - \frac{8C^{2202,1}_{31,1112}}{\sqrt5} + \frac{48}{5}\sqrt{\frac67}C^{1101,1}_{33,2213} - \frac{8C^{1101,1}_{51,0011}}{\sqrt3},$$

$$C^{51}_{11,20} = 9\sqrt{\frac37}C^{3303,1}_{00,3303} - 9\sqrt{\frac37}C^{3313,1}_{00,3313} + 6\sqrt{\frac35}C^{0011,1}_{00,6211} - \frac45\sqrt3 C^{2011,1}_{20,2011} + \frac{6C^{2202,1}_{20,2202}}{\sqrt5} + \frac47\sqrt{\frac53}C^{1110,1}_{22,3112} + \frac{8}{21}\sqrt{\frac53}C^{1111,1}_{22,3112} - 4\sqrt{\frac37}C^{1101,1}_{22,3303} + \frac{8C^{0011,1}_{22,4212}}{3\sqrt5} - 4C^{1101,1}_{40,1101} + 4\sqrt{\frac35}C^{1112,1}_{40,1112} + \frac{2C^{0011,1}_{40,2211}}{\sqrt{15}} - \frac{8C^{1101,1}_{42,1101}}{\sqrt5} + \frac{16C^{1111,1}_{42,1111}}{3\sqrt5} + \frac{4C^{1110,1}_{42,1112}}{\sqrt{15}} + \frac{8C^{0011,1}_{42,2212}}{\sqrt5} - 24C^{0000,1}_{60,0000} + 8\sqrt3 C^{0011,1}_{60,0011},$$

$$C^{51}_{11,22} = -\frac{48}{5}\sqrt3 C^{0011,1}_{62,0011} - \frac{24}{5}\sqrt3 C^{0011,1}_{00,6211} + \frac87\sqrt3 C^{2011,1}_{20,2211} - \frac{10C^{1110,1}_{22,3112}}{7\sqrt3} - \frac{184C^{1111,1}_{22,3112}}{105\sqrt3} + \frac{144}{5}\sqrt{\frac{2}{35}}C^{1111,1}_{22,3313} - \frac{292}{75}C^{0011,1}_{22,4212} - \frac{8C^{0011,1}_{40,2211}}{5\sqrt3} + \frac{992}{105}C^{1111,1}_{42,1111} - \frac{172C^{1110,1}_{42,1112}}{35\sqrt3} + 8C^{0011,1}_{42,2212} + \frac{288}{35}\sqrt{\frac35}C^{0011,1}_{44,2213},$$

$$C^{53}_{11,22} = -\frac{32}{3}\sqrt{\frac75}C^{0011,1}_{62,0011} - \frac{16}{3}\sqrt{\frac75}C^{0011,1}_{00,6211} - \frac{20}{9}\sqrt{\frac57}C^{1110,1}_{22,3112} + \frac{304C^{1111,1}_{22,3112}}{27\sqrt{35}} - \frac{64}{15}\sqrt{\frac23}C^{1111,1}_{22,3313} + \frac{152}{45}\sqrt{\frac{7}{15}}C^{0011,1}_{22,4212} + \frac{16}{3}\sqrt{\frac75}C^{0011,1}_{40,2211} - \frac{64C^{1111,1}_{42,1111}}{3\sqrt{105}} - \frac{16C^{1110,1}_{42,1112}}{3\sqrt{35}} - \frac{128C^{0011,1}_{44,2213}}{15\sqrt7},$$

$$C^{40}_{20,00} = \frac32\sqrt7 C^{3303,1}_{00,3303} + \frac92\sqrt7 C^{3313,1}_{00,3313} - \frac{21C^{0011,1}_{00,6211}}{\sqrt5} + 2C^{2011,1}_{20,2011} + \sqrt{\frac53}C^{2202,1}_{20,2202} + \frac23\sqrt5 C^{1110,1}_{22,3112} + \frac49\sqrt5 C^{1111,1}_{22,3112} + \frac23\sqrt7 C^{1101,1}_{22,3303} + \frac{28C^{0011,1}_{22,4212}}{3\sqrt{15}} + \frac{10C^{1101,1}_{40,1101}}{3\sqrt3} + 2\sqrt5 C^{1112,1}_{40,1112} + \frac13\sqrt5 C^{0011,1}_{40,2211} - \frac{28C^{1101,1}_{42,1101}}{3\sqrt{15}} - \frac{56C^{1111,1}_{42,1111}}{3\sqrt{15}} - \frac{14C^{1110,1}_{42,1112}}{3\sqrt5} - \frac{28C^{0011,1}_{42,2212}}{\sqrt{15}} + \frac{28C^{0000,1}_{60,0000}}{\sqrt3} + 28C^{0011,1}_{60,0011},$$

$$C^{40}_{20,20} = -\frac32\sqrt{21}C^{3303,1}_{00,3303} + \frac32\sqrt{21}C^{3313,1}_{00,3313} - 7\sqrt{\frac35}C^{0011,1}_{00,6211} + \frac{2C^{2011,1}_{20,2011}}{\sqrt3} - \sqrt5 C^{2202,1}_{20,2202} + \frac23\sqrt{\frac53}C^{1110,1}_{22,3112} + \frac49\sqrt{\frac53}C^{1111,1}_{22,3112} - 2\sqrt{\frac73}C^{1101,1}_{22,3303} + \frac{28C^{0011,1}_{22,4212}}{9\sqrt5} - \frac{10}{3}C^{1101,1}_{40,1101} + 2\sqrt{\frac53}C^{1112,1}_{40,1112} + \frac13\sqrt{\frac53}C^{0011,1}_{40,2211} + \frac{28C^{1101,1}_{42,1101}}{3\sqrt5} - \frac{56C^{1111,1}_{42,1111}}{9\sqrt5} - \frac{14C^{1110,1}_{42,1112}}{3\sqrt{15}} - \frac{28C^{0011,1}_{42,2212}}{3\sqrt5} - 28C^{0000,1}_{60,0000} + \frac{28C^{0011,1}_{60,0011}}{\sqrt3},$$

$$C^{42}_{20,22} = -16\sqrt3 C^{0011,1}_{62,0011} + 8\sqrt3 C^{0011,1}_{00,6211} - \frac{8C^{2011,1}_{20,2211}}{7\sqrt3} - \frac{50C^{1110,1}_{22,3112}}{21\sqrt3} - \frac{184C^{1111,1}_{22,3112}}{63\sqrt3} + 48\sqrt{\frac{2}{35}}C^{1111,1}_{22,3313} - \frac{292}{45}C^{0011,1}_{22,4212} + \frac{8C^{0011,1}_{40,2211}}{3\sqrt3} + \frac{352}{63}C^{1111,1}_{42,1111} + \frac{4C^{1110,1}_{42,1112}}{21\sqrt3} + \frac83 C^{0011,1}_{42,2212} - \frac{96}{7}\sqrt{\frac35}C^{0011,1}_{44,2213},$$

$$C^{42}_{22,00} = 6\sqrt{\frac57}C^{3303,1}_{00,3303} + 18\sqrt{\frac57}C^{3313,1}_{00,3313} - 12C^{0011,1}_{00,6211} - \frac{8C^{2011,1}_{20,2011}}{\sqrt5} - \frac{4C^{2202,1}_{20,2202}}{\sqrt3} - \frac{20}{21}C^{1110,1}_{22,3112} - \frac{40}{63}C^{1111,1}_{22,3112} - \frac43\sqrt{\frac57}C^{1101,1}_{22,3303} - \frac{8C^{0011,1}_{22,4212}}{3\sqrt3} - \frac83\sqrt{\frac53}C^{1101,1}_{40,1101} - 8C^{1112,1}_{40,1112} - \frac43 C^{0011,1}_{40,2211} + \frac{8C^{1101,1}_{42,1101}}{3\sqrt3} + \frac{16C^{1111,1}_{42,1111}}{3\sqrt3} + \frac43 C^{1110,1}_{42,1112} + \frac{8C^{0011,1}_{42,2212}}{\sqrt3} + 16\sqrt{\frac53}C^{0000,1}_{60,0000} + 16\sqrt5 C^{0011,1}_{60,0011},$$

$$C^{42}_{22,11} = -\frac{40C^{3101,1}_{11,2212}}{7\sqrt3} - \frac{16}{3}\sqrt5 C^{1101,1}_{51,0011},$$

$$C^{42}_{22,20} = -6\sqrt{\tfrac{15}{7}}C^{3303,1}_{00,3303} + 6\sqrt{\tfrac{15}{7}}C^{3313,1}_{00,3313} - 4\sqrt{3}C^{0011,1}_{00,6211} - \frac{8C^{2011,1}_{20,2011}}{\sqrt{15}} + 4C^{2202,1}_{20,2202} - \frac{20C^{1110,1}_{22,3112}}{21\sqrt{3}} - \frac{40C^{1111,1}_{22,3112}}{63\sqrt{3}} + 4\sqrt{\tfrac{5}{21}}C^{1101,1}_{22,3303} - \tfrac{8}{9}C^{0011,1}_{22,4212} + \tfrac{8}{3}\sqrt{5}C^{1101,1}_{40,1101} - \frac{8C^{1112,1}_{40,1112}}{\sqrt{3}} - \frac{4C^{0011,1}_{40,2211}}{3\sqrt{3}} - \tfrac{8}{3}C^{1101,1}_{42,1101} + \tfrac{16}{9}C^{1111,1}_{42,1111} + \frac{4C^{1110,1}_{42,1112}}{3\sqrt{3}} + \tfrac{8}{3}C^{0011,1}_{42,2212} - 16\sqrt{5}C^{0000,1}_{60,0000} + 16\sqrt{\tfrac{5}{3}}C^{0011,1}_{60,0011},$$

$$C^{40}_{22,22} = -\tfrac{56}{5}\sqrt{3}C^{0011,1}_{62,0011} + \tfrac{28}{5}\sqrt{3}C^{0011,1}_{00,6211} - \frac{4C^{2011,1}_{20,2211}}{5\sqrt{3}} - \frac{5C^{1110,1}_{22,3112}}{3\sqrt{3}} + \frac{52C^{1111,1}_{22,3112}}{45\sqrt{3}} - \tfrac{24}{5}\sqrt{\tfrac{14}{5}}C^{1111,1}_{22,3313} + \tfrac{2002}{225}C^{0011,1}_{22,4212} - \frac{68C^{0011,1}_{40,2211}}{15\sqrt{3}} + \tfrac{272}{45}C^{1111,1}_{42,1111} + \frac{26C^{1110,1}_{42,1112}}{15\sqrt{3}} + \tfrac{28}{15}C^{0011,1}_{42,2212} + \tfrac{48}{5}\sqrt{\tfrac{3}{5}}C^{0011,1}_{44,2213},$$

$$C^{42}_{22,22} = -32\sqrt{\tfrac{3}{7}}C^{0011,1}_{62,0011} + 16\sqrt{\tfrac{3}{7}}C^{0011,1}_{00,6211} + \frac{32C^{2011,1}_{20,2211}}{7\sqrt{21}} + \frac{20C^{1110,1}_{22,3112}}{21\sqrt{21}} + \frac{880C^{1111,1}_{22,3112}}{63\sqrt{21}} - \frac{184C^{0011,1}_{22,4212}}{9\sqrt{7}} - \frac{80C^{0011,1}_{40,2211}}{3\sqrt{21}} - \frac{256C^{1111,1}_{42,1111}}{9\sqrt{7}} - \frac{16C^{1110,1}_{42,1112}}{3\sqrt{21}} - \frac{32C^{0011,1}_{42,2212}}{3\sqrt{7}},$$

$$C^{44}_{22,22} = -\frac{32C^{0011,1}_{62,0011}}{\sqrt{15}} + \frac{16C^{0011,1}_{00,6211}}{\sqrt{15}} + \tfrac{16}{7}\sqrt{\tfrac{3}{5}}C^{2011,1}_{20,2211} + \tfrac{20}{21}\sqrt{\tfrac{5}{3}}C^{1110,1}_{22,3112} - \frac{304C^{1111,1}_{22,3112}}{63\sqrt{15}} - \tfrac{8}{15}\sqrt{14}C^{1111,1}_{22,3313} + \frac{328C^{0011,1}_{22,4212}}{45\sqrt{5}} + \frac{16C^{0011,1}_{40,2211}}{\sqrt{15}} - \frac{64C^{1111,1}_{42,1111}}{3\sqrt{5}} + \frac{8C^{1110,1}_{42,1112}}{\sqrt{15}} - \frac{16C^{0011,1}_{42,2212}}{\sqrt{5}} + \frac{16C^{0011,1}_{44,2213}}{5\sqrt{3}},$$

$$C^{31}_{31,00} = -\tfrac{9}{5}\sqrt{7}C^{3303,1}_{00,3303} - \tfrac{27}{5}\sqrt{7}C^{3313,1}_{00,3313} + \frac{126C^{0011,1}_{00,6211}}{5\sqrt{5}} + \tfrac{12}{25}C^{2011,1}_{20,2011} + \tfrac{2}{5}\sqrt{\tfrac{3}{5}}C^{2202,1}_{20,2202} - \frac{4C^{1110,1}_{22,3112}}{\sqrt{5}} - \frac{8C^{1111,1}_{22,3112}}{3\sqrt{5}} - \tfrac{4}{5}\sqrt{7}C^{1101,1}_{22,3303} - \frac{56C^{0011,1}_{22,4212}}{5\sqrt{15}} - \frac{4C^{1101,1}_{40,1101}}{5\sqrt{3}} - \frac{12C^{1112,1}_{40,1112}}{5\sqrt{5}} - \frac{2C^{0011,1}_{40,2211}}{5\sqrt{5}} - \frac{56C^{1101,1}_{42,1101}}{5\sqrt{15}} - \frac{112C^{1111,1}_{42,1111}}{5\sqrt{15}} - \frac{28C^{1110,1}_{42,1112}}{5\sqrt{5}} - \tfrac{56}{5}\sqrt{\tfrac{3}{5}}C^{0011,1}_{42,2212} + \tfrac{56}{5}\sqrt{3}C^{0000,1}_{60,0000} + \tfrac{168}{5}C^{0011,1}_{60,0011},$$

$$C^{31}_{31,11} = \frac{4C^{3101,1}_{11,2212}}{\sqrt{5}} - \frac{24C^{2202,1}_{31,1112}}{5\sqrt{5}} - \tfrac{48}{25}\sqrt{42}C^{1101,1}_{33,2213} - \frac{56C^{1101,1}_{51,0011}}{5\sqrt{3}},$$

$$C^{31}_{31,20} = \tfrac{9}{5}\sqrt{21}C^{3303,1}_{00,3303} - \tfrac{9}{5}\sqrt{21}C^{3313,1}_{00,3313} + \tfrac{42}{5}\sqrt{\tfrac{3}{5}}C^{0011,1}_{00,6211} + \tfrac{4}{25}\sqrt{3}C^{2011,1}_{20,2011} - \frac{6C^{2202,1}_{20,2202}}{5\sqrt{5}} - \frac{4C^{1110,1}_{22,3112}}{\sqrt{15}} - \frac{8C^{1111,1}_{22,3112}}{3\sqrt{15}} + \tfrac{4}{5}\sqrt{21}C^{1101,1}_{22,3303} - \frac{56C^{0011,1}_{22,4212}}{15\sqrt{5}} + \tfrac{4}{5}C^{1101,1}_{40,1101} - \tfrac{4}{5}\sqrt{\tfrac{3}{5}}C^{1112,1}_{40,1112} - \frac{2C^{0011,1}_{40,2211}}{5\sqrt{15}} + \frac{56C^{1101,1}_{42,1101}}{5\sqrt{5}} - \frac{112C^{1111,1}_{42,1111}}{15\sqrt{5}} - \frac{28C^{1110,1}_{42,1112}}{5\sqrt{15}} - \frac{56C^{0011,1}_{42,2212}}{5\sqrt{5}} - \tfrac{168}{5}C^{0000,1}_{60,0000} + \tfrac{56}{5}\sqrt{3}C^{0011,1}_{60,0011},$$

$$C^{31}_{31,22} = -\tfrac{336}{25}\sqrt{3}C^{0011,1}_{62,0011} - \tfrac{168}{25}\sqrt{3}C^{0011,1}_{00,6211} + \tfrac{8}{25}\sqrt{3}C^{2011,1}_{20,2211} + \frac{22C^{1110,1}_{22,3112}}{5\sqrt{3}} - \frac{56C^{1111,1}_{22,3112}}{75\sqrt{3}} - \tfrac{144}{25}\sqrt{\tfrac{14}{5}}C^{1111,1}_{22,3313} + \tfrac{2884}{375}C^{0011,1}_{22,4212} - \frac{184C^{0011,1}_{40,2211}}{25\sqrt{3}} + \tfrac{352}{75}C^{1111,1}_{42,1111} + \frac{4C^{1110,1}_{42,1112}}{25\sqrt{3}} + \tfrac{56}{25}C^{0011,1}_{42,2212} - \tfrac{288}{25}\sqrt{\tfrac{3}{5}}C^{0011,1}_{44,2213},$$

$$C^{33}_{31,22} = -\tfrac{96}{5}\sqrt{\tfrac{7}{5}}C^{0011,1}_{62,0011} - \tfrac{48}{5}\sqrt{\tfrac{7}{5}}C^{0011,1}_{00,6211} - \frac{64C^{2011,1}_{20,2211}}{5\sqrt{35}} + \frac{4C^{1110,1}_{22,3112}}{3\sqrt{35}} + \frac{208C^{1111,1}_{22,3112}}{45\sqrt{35}} + \tfrac{64}{25}\sqrt{6}C^{1111,1}_{22,3313} - \tfrac{1016}{75}\sqrt{\tfrac{7}{15}}C^{0011,1}_{22,4212} + \tfrac{16}{15}\sqrt{\tfrac{7}{5}}C^{0011,1}_{40,2211} - \frac{1216C^{1111,1}_{42,1111}}{15\sqrt{105}} + \frac{368C^{1110,1}_{42,1112}}{15\sqrt{35}} - \tfrac{64}{5}\sqrt{\tfrac{7}{15}}C^{0011,1}_{42,2212} + \frac{384C^{0011,1}_{44,2213}}{25\sqrt{7}},$$

$$C^{33}_{33,00} = -\frac{2C^{3303,1}_{00,3303}}{\sqrt{3}} - 2\sqrt{3}C^{3313,1}_{00,3313} + 4\sqrt{\tfrac{7}{15}}C^{0011,1}_{00,6211} + \tfrac{8}{5}\sqrt{\tfrac{7}{3}}C^{2011,1}_{20,2011} + \tfrac{4}{3}\sqrt{\tfrac{7}{5}}C^{2202,1}_{20,2202} + \tfrac{4}{3}\sqrt{\tfrac{5}{21}}C^{1110,1}_{22,3112} + \tfrac{8}{9}\sqrt{\tfrac{5}{21}}C^{1111,1}_{22,3112} + \frac{4C^{1101,1}_{22,3303}}{3\sqrt{3}} + \tfrac{8}{9}\sqrt{\tfrac{7}{5}}C^{0011,1}_{22,4212} - \tfrac{8}{9}\sqrt{7}C^{1101,1}_{40,1101} - 8\sqrt{\tfrac{7}{15}}C^{1112,1}_{40,1112} - \tfrac{4}{3}\sqrt{\tfrac{7}{15}}C^{0011,1}_{40,2211} + \tfrac{8}{9}\sqrt{\tfrac{7}{5}}C^{1101,1}_{42,1101} + \tfrac{16}{9}\sqrt{\tfrac{7}{5}}C^{1111,1}_{42,1111} + \tfrac{4}{3}\sqrt{\tfrac{7}{15}}C^{1110,1}_{42,1112} + \tfrac{8}{3}\sqrt{\tfrac{7}{5}}C^{0011,1}_{42,2212} + \tfrac{16}{9}\sqrt{7}C^{0000,1}_{60,0000} + \tfrac{16}{3}\sqrt{\tfrac{7}{3}}C^{0011,1}_{60,0011},$$

$C^{33}_{33,11} = \frac{8}{9}\sqrt{\frac{10}{7}}C^{3101,1}_{11,2212} + \frac{16}{9}\sqrt{\frac{14}{5}}C^{2202,1}_{31,1112} + \frac{16C^{1101,1}_{33,2213}}{5\sqrt{3}} - \frac{16}{9}\sqrt{\frac{14}{3}}C^{1101,1}_{51,0011}$,
$C^{33}_{33,20} = 2C^{3303,1}_{00,3303} - 2C^{3313,1}_{00,3313} + \frac{4}{3}\sqrt{\frac{7}{5}}C^{0011,1}_{00,6211} + \frac{8}{15}\sqrt{7}C^{2011,1}_{20,2011} - 4\sqrt{\frac{7}{15}}C^{2202,1}_{20,2202} + \frac{4}{9}\sqrt{\frac{5}{7}}C^{1110,1}_{22,3112} + \frac{8}{27}\sqrt{\frac{5}{7}}C^{1111,1}_{22,3112} - \frac{4}{3}C^{1101,1}_{22,3303} + \frac{8}{9}\sqrt{\frac{7}{15}}C^{0011,1}_{22,4212} + \frac{8}{3}\sqrt{\frac{7}{3}}C^{1101,1}_{40,1101} - \frac{8}{3}\sqrt{\frac{7}{5}}C^{1112,1}_{40,1112} - \frac{4}{9}\sqrt{\frac{7}{5}}C^{0011,1}_{40,2211} - \frac{8}{3}\sqrt{\frac{7}{15}}C^{1101,1}_{42,1101} + \frac{16}{9}\sqrt{\frac{7}{15}}C^{1111,1}_{42,1111} + \frac{4}{9}\sqrt{\frac{7}{5}}C^{1110,1}_{42,1112} + \frac{8}{3}\sqrt{\frac{7}{15}}C^{0011,1}_{42,2212} - \frac{16}{3}\sqrt{\frac{7}{3}}C^{0000,1}_{60,0000} + \frac{16}{9}\sqrt{7}C^{0011,1}_{60,0011}$,
$C^{33}_{33,22} = -\frac{32}{15}\sqrt{\frac{14}{3}}C^{0011,1}_{62,0011} - \frac{16}{15}\sqrt{\frac{14}{3}}C^{0011,1}_{00,6211} - \frac{16}{5}\sqrt{\frac{2}{21}}C^{2011,1}_{20,2211} - \frac{4}{3}\sqrt{\frac{2}{21}}C^{1110,1}_{22,3112} - \frac{208}{45}\sqrt{\frac{2}{21}}C^{1111,1}_{22,3112} + \frac{16C^{1111,1}_{22,3313}}{15\sqrt{5}} + \frac{24}{25}\sqrt{14}C^{0011,1}_{22,4212} - \frac{16}{15}\sqrt{\frac{14}{3}}C^{0011,1}_{40,2211} - \frac{704}{45}\sqrt{\frac{2}{7}}C^{1111,1}_{42,1111} - \frac{8}{15}\sqrt{\frac{2}{21}}C^{1110,1}_{42,1112} - \frac{16}{15}\sqrt{14}C^{0011,1}_{42,2212} + \frac{16}{5}\sqrt{\frac{2}{105}}C^{0011,1}_{44,2213}$.
