# Supplementary material for: Effective pseudopotential for energy density functionals with higher order derivatives
Source: arXiv:1103.0682 ancillary file (2011-04-17)
Supplement: Supplementary file 3 [file Suppl_T_Section_IIIB.tex.pdf]

**Set of constraints on the Galilean-invariant EDF fourth-order coupling constants: 15 isovector fourth-order coupling constants are expressed through the 15 corresponding isoscalar fourth-order coupling costants.**

$$C^{2202,1}_{00,2202} = -\frac{4}{3}\sqrt{\frac{5}{3}}C^{0000,0}_{40,0000} - \frac{4}{3}\sqrt{5}C^{0011,0}_{40,0011} - \frac{C^{2202,0}_{00,2202}}{\sqrt{3}},$$
$$C^{2212,1}_{00,2212} = -\frac{4}{3}\sqrt{\frac{5}{3}}C^{0000,0}_{40,0000} + \frac{4}{9}\sqrt{5}C^{0011,0}_{40,0011} + \frac{14}{9}C^{0011,0}_{42,0011} - \frac{C^{2212,0}_{00,2212}}{\sqrt{3}},$$
$$C^{0011,1}_{00,4211} = -\frac{C^{0011,0}_{00,4211}}{\sqrt{3}} - \frac{4C^{0011,0}_{42,0011}}{\sqrt{3}},$$
$$C^{0000,1}_{40,0000} = -\frac{7C^{0011,0}_{00,4211}}{8\sqrt{5}} - \frac{C^{0000,0}_{40,0000}}{\sqrt{3}} - \frac{1}{4}\sqrt{\frac{3}{5}}C^{2202,0}_{00,2202} - \frac{3}{4}\sqrt{\frac{3}{5}}C^{2212,0}_{00,2212},$$
$$C^{0011,1}_{40,0011} = \frac{7C^{0011,0}_{00,4211}}{8\sqrt{15}} - \frac{C^{0011,0}_{40,0011}}{\sqrt{3}} - \frac{3C^{2202,0}_{00,2202}}{4\sqrt{5}} + \frac{3C^{2212,0}_{00,2212}}{4\sqrt{5}},$$
$$C^{0011,1}_{42,0011} = -\frac{C^{0011,0}_{00,4211}}{\sqrt{3}} - \frac{C^{0011,0}_{42,0011}}{\sqrt{3}},$$
$$C^{1101,1}_{20,1101} = -\frac{2C^{1101,0}_{20,1101}}{\sqrt{3}} + C^{0011,0}_{20,2011},$$
$$C^{1101,1}_{22,1101} = -\frac{2C^{1101,0}_{22,1101}}{\sqrt{3}} - \frac{1}{3}C^{1111,0}_{22,1112} - \frac{2C^{1112,0}_{22,1112}}{\sqrt{7}} + \sqrt{\frac{5}{21}}C^{0011,0}_{22,2213},$$
$$C^{0011,1}_{20,2011} = C^{1101,0}_{20,1101},$$
$$C^{0011,1}_{20,2211} = -\frac{C^{0011,0}_{20,2211}}{\sqrt{3}} - \frac{4C^{1111,0}_{22,1112}}{3\sqrt{3}} + \frac{4C^{1112,0}_{22,1112}}{\sqrt{21}} - \frac{2}{3}\sqrt{\frac{5}{7}}C^{0011,0}_{22,2213},$$
$$C^{1111,1}_{22,1112} = -\frac{2C^{0011,0}_{20,2211}}{\sqrt{3}} - C^{1101,0}_{22,1101} - \frac{2C^{1111,0}_{22,1112}}{3\sqrt{3}} + \frac{2C^{1112,0}_{22,1112}}{\sqrt{21}} - \frac{1}{3}\sqrt{\frac{5}{7}}C^{0011,0}_{22,2213},$$
$$C^{1112,1}_{22,1112} = \frac{1}{3}\sqrt{\frac{7}{3}}C^{0011,0}_{20,2211} - \frac{1}{6}\sqrt{7}C^{1101,0}_{22,1101} - \frac{1}{18}\sqrt{\frac{7}{3}}C^{1111,0}_{22,1112} - \frac{4C^{1112,0}_{22,1112}}{3\sqrt{3}} - \frac{5}{18}\sqrt{5}C^{0011,0}_{22,2213},$$
$$C^{0011,1}_{22,2213} = \sqrt{\frac{7}{15}}C^{1101,0}_{22,1101} - \frac{1}{3}\sqrt{\frac{7}{5}}C^{1111,0}_{22,1112} - \frac{2C^{1112,0}_{22,1112}}{\sqrt{5}} - \frac{2C^{0011,0}_{22,2213}}{\sqrt{3}},$$
$$C^{1101,1}_{31,0011} = \frac{2C^{1101,0}_{11,2212}}{\sqrt{5}} - \frac{C^{1101,0}_{31,0011}}{\sqrt{3}},$$
$$C^{1101,1}_{11,2212} = -\frac{C^{1101,0}_{11,2212}}{\sqrt{3}} + \frac{2}{3}\sqrt{5}C^{1101,0}_{31,0011},$$

**Set of constraints on the Galilean-invariant EDF sixth-order coupling constants: 26 isovector sixth-order coupling constants are expressed through the 26 corresponding isoscalar sixth-order coupling costants.**

$$C^{0000,1}_{60,0000} = -\frac{3C^{3303,0}_{00,3303}}{8\sqrt{7}} - \frac{9C^{3313,0}_{00,3313}}{8\sqrt{7}} + \frac{3C^{0011,0}_{00,6211}}{4\sqrt{5}} - \frac{C^{0000,0}_{60,0000}}{\sqrt{3}},$$
$$C^{0011,1}_{60,0011} = -\frac{3}{8}\sqrt{\frac{3}{7}}C^{3303,0}_{00,3303} + \frac{3}{8}\sqrt{\frac{3}{7}}C^{3313,0}_{00,3313} - \frac{1}{4}\sqrt{\frac{3}{5}}C^{0011,0}_{00,6211} - \frac{C^{0011,0}_{60,0011}}{\sqrt{3}},$$
$$C^{0011,1}_{62,0011} = \frac{C^{0011,0}_{00,6211}}{\sqrt{3}} - \frac{C^{0011,0}_{62,0011}}{\sqrt{3}},$$
$$C^{3303,1}_{00,3303} = -\frac{C^{3303,0}_{00,3303}}{\sqrt{3}} - \frac{8}{9}\sqrt{7}C^{0000,0}_{60,0000} - \frac{8}{3}\sqrt{\frac{7}{3}}C^{0011,0}_{60,0011},$$
$$C^{0011,1}_{00,6211} = -\frac{C^{0011,0}_{00,6211}}{\sqrt{3}} + \frac{4C^{0011,0}_{62,0011}}{\sqrt{3}},$$
$$C^{3313,1}_{00,3313} = -\frac{C^{3313,0}_{00,3313}}{\sqrt{3}} - \frac{8}{9}\sqrt{7}C^{0000,0}_{60,0000} + \frac{8}{9}\sqrt{\frac{7}{3}}C^{0011,0}_{60,0011} + \frac{8}{3}\sqrt{\frac{7}{15}}C^{0011,0}_{62,0011},$$
$$C^{2202,1}_{20,2202} = -\frac{C^{2202,0}_{20,2202}}{\sqrt{3}} - \frac{2}{3}\sqrt{\frac{5}{3}}C^{1101,0}_{40,1101} - 2C^{1112,0}_{40,1112} - \frac{1}{3}C^{0011,0}_{40,2211},$$

$$C^{1110,1}_{42,1112} = -\frac{4C^{2011,0}_{20,2211}}{7\sqrt{3}} + \frac{5C^{1110,0}_{22,3112}}{21\sqrt{3}} + \frac{10C^{1111,0}_{22,3112}}{63\sqrt{3}} + \sqrt{\frac{5}{21}}C^{1101,0}_{22,3303} - \frac{10}{9}C^{0011,0}_{22,4212} - \frac{C^{1110,0}_{42,1112}}{\sqrt{3}},$$

$$C^{1110,1}_{22,3112} = -\frac{C^{1110,0}_{22,3112}}{\sqrt{3}} - \frac{8C^{0011,0}_{40,2211}}{3\sqrt{3}} + \frac{14}{15}C^{1101,0}_{42,1101} + \frac{28}{45}C^{1111,0}_{42,1111} + \frac{7C^{1110,0}_{42,1112}}{15\sqrt{3}} - \frac{14}{15}C^{0011,0}_{42,2212},$$

$$C^{1111,1}_{42,1111} = \frac{1}{7}C^{2011,0}_{20,2211} + \frac{25}{84}C^{1110,0}_{22,3112} + \frac{25}{126}C^{1111,0}_{22,3112} - \frac{1}{4}\sqrt{\frac{5}{7}}C^{1101,0}_{22,3303} - \frac{7C^{0011,0}_{22,4212}}{6\sqrt{3}} - \frac{C^{1111,0}_{42,1111}}{\sqrt{3}},$$

$$C^{1111,1}_{22,3112} = -\frac{C^{1111,0}_{22,3112}}{\sqrt{3}} + \frac{4C^{0011,0}_{40,2211}}{\sqrt{3}} + \frac{7}{5}C^{1101,0}_{42,1101} - \frac{14}{15}C^{1111,0}_{42,1111} - \frac{7C^{1110,0}_{42,1112}}{10\sqrt{3}} - \frac{7}{5}C^{0011,0}_{42,2212},$$

$$C^{1111,1}_{22,3313} = -\frac{C^{1111,0}_{22,3313}}{\sqrt{3}} + \frac{2}{3}\sqrt{\frac{14}{15}}C^{1101,0}_{42,1101} - \frac{4}{3}\sqrt{\frac{10}{21}}C^{1111,0}_{42,1111} - \frac{1}{3}\sqrt{\frac{10}{7}}C^{1110,0}_{42,1112} - \frac{2}{3}\sqrt{\frac{14}{15}}C^{0011,0}_{42,2212} + 2\sqrt{\frac{2}{7}}C^{0011,0}_{44,2213},$$

$$C^{1112,1}_{40,1112} = \frac{C^{2011,0}_{20,2011}}{\sqrt{15}} - \frac{1}{2}C^{2202,0}_{20,2202} + \frac{C^{1110,0}_{22,3112}}{12\sqrt{3}} - \frac{C^{1111,0}_{22,3112}}{9\sqrt{3}} + \frac{7}{90}C^{0011,0}_{22,4212} - \frac{C^{1112,0}_{40,1112}}{\sqrt{3}},$$

$$C^{1101,1}_{40,1101} = -\frac{3}{5}C^{2011,0}_{20,2011} - \frac{1}{2}\sqrt{\frac{3}{5}}C^{2202,0}_{20,2202} - \frac{C^{1101,0}_{40,1101}}{\sqrt{3}},$$

$$C^{1101,1}_{42,1101} = \frac{5}{14}C^{1110,0}_{22,3112} + \frac{5}{21}C^{1111,0}_{22,3112} + \frac{1}{2}\sqrt{\frac{5}{7}}C^{1101,0}_{22,3303} + \frac{C^{0011,0}_{22,4212}}{\sqrt{3}} - \frac{C^{1101,0}_{42,1101}}{\sqrt{3}},$$

$$C^{1101,1}_{22,3303} = -\frac{C^{1101,0}_{22,3303}}{\sqrt{3}} + \frac{2}{3}\sqrt{\frac{7}{5}}C^{1101,0}_{42,1101} + \frac{4}{3}\sqrt{\frac{7}{5}}C^{1111,0}_{42,1111} + \sqrt{\frac{7}{15}}C^{1110,0}_{42,1112} + 2\sqrt{\frac{7}{5}}C^{0011,0}_{42,2212},$$

$$C^{1101,1}_{51,0011} = -\frac{1}{7}\sqrt{5}C^{3101,0}_{11,2212} - \frac{C^{1101,0}_{51,0011}}{\sqrt{3}},$$

$$C^{2202,1}_{31,1112} = \frac{C^{2202,0}_{31,1112}}{\sqrt{3}},$$

$$C^{1101,1}_{33,2213} = \frac{C^{1101,0}_{33,2213}}{\sqrt{3}},$$

$$C^{3101,1}_{11,2212} = -\frac{C^{3101,0}_{11,2212}}{\sqrt{3}} - \frac{28C^{1101,0}_{51,0011}}{3\sqrt{5}},$$

$$C^{0011,1}_{40,2211} = -\frac{C^{1110,0}_{22,3112}}{2\sqrt{3}} + \frac{2C^{1111,0}_{22,3112}}{3\sqrt{3}} - \frac{7}{15}C^{0011,0}_{22,4212} - \frac{C^{0011,0}_{40,2211}}{\sqrt{3}},$$

$$C^{0011,1}_{42,2212} = -\frac{5}{14}C^{1110,0}_{22,3112} - \frac{5}{21}C^{1111,0}_{22,3112} + \frac{1}{2}\sqrt{\frac{5}{7}}C^{1101,0}_{22,3303} + \frac{C^{0011,0}_{22,4212}}{\sqrt{3}} - \frac{C^{0011,0}_{42,2212}}{\sqrt{3}},$$

$$C^{0011,1}_{44,2213} = -\frac{2}{21}\sqrt{\frac{5}{3}}C^{1110,0}_{22,3112} - \frac{4}{63}\sqrt{\frac{5}{3}}C^{1111,0}_{22,3112} + \frac{1}{3}\sqrt{14}C^{1111,0}_{22,3313} - \frac{4}{9}\sqrt{5}C^{0011,0}_{22,4212} - \frac{C^{0011,0}_{44,2213}}{\sqrt{3}},$$

$$C^{2011,1}_{20,2011} = -\frac{C^{2011,0}_{20,2011}}{\sqrt{3}} - \frac{5}{3}C^{1101,0}_{40,1101} + \sqrt{\frac{5}{3}}C^{1112,0}_{40,1112} + \frac{1}{6}\sqrt{\frac{5}{3}}C^{0011,0}_{40,2211},$$

$$C^{2011,1}_{20,2211} = -\frac{C^{2011,0}_{20,2211}}{\sqrt{3}} + \frac{56}{9}C^{1111,0}_{42,1111} - \frac{7C^{1110,0}_{42,1112}}{3\sqrt{3}} + \frac{14}{3}C^{0011,0}_{42,2212},$$

$$C^{0011,1}_{22,4212} = -\frac{C^{0011,0}_{22,4212}}{\sqrt{3}} + \frac{C^{1101,0}_{42,1101}}{\sqrt{3}} - \frac{2C^{1111,0}_{42,1111}}{\sqrt{3}} - \frac{1}{2}C^{1110,0}_{42,1112} - \frac{C^{0011,0}_{42,2212}}{\sqrt{3}}.$$
