# Supplementary material for: Effective pseudopotential for energy density functionals with higher order derivatives
Source: arXiv:1103.0682 ancillary file (2011-04-17)
Supplement: Supplementary file 4 [file Suppl_T_Section_IV.tex.pdf]

**14 fourth-order coupling constants of the Galilean and spherical symmetric EDF expressed by 13 pseudopotential parameters (Spin - Orbit terms excluded).**

$$C^{0000,0}_{40,0000} = \frac{3}{128}C^{40}_{00,00} + \frac{1}{128}\sqrt{3}C^{40}_{00,20} - \frac{5}{128}C^{31}_{11,00} + \frac{1}{128}\sqrt{3}C^{31}_{11,20} + \frac{3}{128}C^{20}_{20,00} + \frac{1}{128}\sqrt{3}C^{20}_{20,20} + \frac{3C^{22}_{22,00}}{64\sqrt{5}} + \frac{1}{64}\sqrt{\frac{3}{5}}C^{22}_{22,20},$$

$$C^{0000,1}_{40,0000} = -\frac{1}{128}\sqrt{3}C^{40}_{00,00} + \frac{3}{128}C^{40}_{00,20} - \frac{1}{128}\sqrt{3}C^{31}_{11,00} + \frac{3}{128}C^{31}_{11,20} - \frac{1}{128}\sqrt{3}C^{20}_{20,00} + \frac{3}{128}C^{20}_{20,20} - \frac{1}{64}\sqrt{\frac{3}{5}}C^{22}_{22,00} + \frac{3C^{22}_{22,20}}{64\sqrt{5}},$$

$$C^{0000,0}_{20,2000} = -\frac{5}{32}C^{40}_{00,00} - \frac{5C^{40}_{00,20}}{32\sqrt{3}} - \frac{1}{32}C^{20}_{20,00} - \frac{C^{20}_{20,20}}{32\sqrt{3}} + \frac{1}{16}\sqrt{5}C^{22}_{22,00} + \frac{1}{16}\sqrt{\frac{5}{3}}C^{22}_{22,20},$$

$$C^{0000,1}_{20,2000} = \frac{5C^{40}_{00,00}}{32\sqrt{3}} - \frac{5}{32}C^{40}_{00,20} + \frac{C^{20}_{20,00}}{32\sqrt{3}} - \frac{1}{32}C^{20}_{20,20} - \frac{1}{16}\sqrt{\frac{5}{3}}C^{22}_{22,00} + \frac{1}{16}\sqrt{5}C^{22}_{22,20},$$

$$C^{0000,0}_{22,2202} = -\frac{1}{16}\sqrt{5}C^{40}_{00,00} - \frac{1}{16}\sqrt{\frac{5}{3}}C^{40}_{00,20} + \frac{1}{16}\sqrt{5}C^{20}_{20,00} + \frac{1}{16}\sqrt{\frac{5}{3}}C^{20}_{20,20} - \frac{1}{16}C^{22}_{22,00} - \frac{C^{22}_{22,20}}{16\sqrt{3}},$$

$$C^{0000,1}_{22,2202} = \frac{1}{16}\sqrt{\frac{5}{3}}C^{40}_{00,00} - \frac{1}{16}\sqrt{5}C^{40}_{00,20} - \frac{1}{16}\sqrt{\frac{5}{3}}C^{20}_{20,00} + \frac{1}{16}\sqrt{5}C^{20}_{20,20} + \frac{C^{22}_{22,00}}{16\sqrt{3}} - \frac{1}{16}C^{22}_{22,20},$$

$$C^{2202,0}_{00,2202} = \frac{1}{32}\sqrt{5}C^{40}_{00,00} + \frac{1}{32}\sqrt{\frac{5}{3}}C^{40}_{00,20} + \frac{5}{96}\sqrt{5}C^{31}_{11,00} - \frac{1}{32}\sqrt{\frac{5}{3}}C^{31}_{11,20} + \frac{1}{32}\sqrt{5}C^{20}_{20,00} + \frac{1}{32}\sqrt{\frac{5}{3}}C^{20}_{20,20} + \frac{1}{16}C^{22}_{22,00} + \frac{C^{22}_{22,20}}{16\sqrt{3}},$$

$$C^{2202,1}_{00,2202} = -\frac{1}{32}\sqrt{\frac{5}{3}}C^{40}_{00,00} + \frac{1}{32}\sqrt{5}C^{40}_{00,20} + \frac{1}{32}\sqrt{\frac{5}{3}}C^{31}_{11,00} - \frac{1}{32}\sqrt{5}C^{31}_{11,20} - \frac{1}{32}\sqrt{\frac{5}{3}}C^{20}_{20,00} + \frac{1}{32}\sqrt{5}C^{20}_{20,20} - \frac{C^{22}_{22,00}}{16\sqrt{3}} + \frac{1}{16}C^{22}_{22,20},$$

$$C^{1111,0}_{20,1111} = -\frac{5}{96}C^{40}_{00,00} - \frac{25C^{40}_{00,20}}{96\sqrt{3}} + \frac{7}{192}\sqrt{\frac{5}{3}}C^{42}_{00,22} + \frac{1}{64}\sqrt{15}C^{31}_{11,22} - \frac{3}{64}\sqrt{7}C^{33}_{11,22} - \frac{1}{96}C^{20}_{20,00} - \frac{5C^{20}_{20,20}}{96\sqrt{3}} - \frac{1}{192}\sqrt{\frac{5}{3}}C^{22}_{20,22} + \frac{1}{48}\sqrt{5}C^{22}_{22,00} + \frac{5}{48}\sqrt{\frac{5}{3}}C^{22}_{22,20} - \frac{1}{96}\sqrt{\frac{35}{3}}C^{22}_{22,22},$$

$$C^{1111,1}_{20,1111} = -\frac{5C^{40}_{00,00}}{32\sqrt{3}} - \frac{5}{96}C^{40}_{00,20} - \frac{7}{192}\sqrt{5}C^{42}_{00,22} + \frac{1}{64}\sqrt{5}C^{31}_{11,22} - \frac{1}{64}\sqrt{21}C^{33}_{11,22} - \frac{C^{20}_{20,00}}{32\sqrt{3}} - \frac{1}{96}C^{20}_{20,20} + \frac{1}{192}\sqrt{5}C^{22}_{20,22} + \frac{1}{16}\sqrt{\frac{5}{3}}C^{22}_{22,00} + \frac{1}{48}\sqrt{5}C^{22}_{22,20} + \frac{1}{96}\sqrt{35}C^{22}_{22,22},$$

$$C^{1111,0}_{22,1111} = \frac{1}{96}\sqrt{5}C^{40}_{00,00} + \frac{5}{96}\sqrt{\frac{5}{3}}C^{40}_{00,20} - \frac{7C^{42}_{00,22}}{192\sqrt{3}} - \frac{1}{64}\sqrt{3}C^{31}_{11,22} + \frac{3}{64}\sqrt{\frac{7}{5}}C^{33}_{11,22} - \frac{1}{96}\sqrt{5}C^{20}_{20,00} - \frac{5}{96}\sqrt{\frac{5}{3}}C^{20}_{20,20} + \frac{13C^{22}_{20,22}}{192\sqrt{3}} + \frac{1}{96}C^{22}_{22,00} + \frac{5C^{22}_{22,20}}{96\sqrt{3}} - \frac{5}{96}\sqrt{\frac{7}{3}}C^{22}_{22,22},$$

$$C^{1111,1}_{22,1111} = \frac{1}{32}\sqrt{\frac{5}{3}}C^{40}_{00,00} + \frac{1}{96}\sqrt{5}C^{40}_{00,20} + \frac{7}{192}C^{42}_{00,22} - \frac{1}{64}C^{31}_{11,22} + \frac{1}{64}\sqrt{\frac{21}{5}}C^{33}_{11,22} - \frac{1}{32}\sqrt{\frac{5}{3}}C^{20}_{20,00} - \frac{1}{96}\sqrt{5}C^{20}_{20,20} - \frac{13}{192}C^{22}_{20,22} + \frac{C^{22}_{22,00}}{32\sqrt{3}} + \frac{1}{96}C^{22}_{22,20} + \frac{5}{96}\sqrt{7}C^{22}_{22,22},$$

$$C^{1111,0}_{00,3111} = \frac{1}{16}C^{40}_{00,00} + \frac{5C^{40}_{00,20}}{16\sqrt{3}} - \frac{7C^{42}_{00,22}}{32\sqrt{15}} - \frac{1}{16}C^{31}_{11,00} + \frac{1}{16}\sqrt{3}C^{31}_{11,20} - \frac{7}{32}\sqrt{\frac{3}{5}}C^{31}_{11,22} - \frac{9}{160}\sqrt{7}C^{33}_{11,22} + \frac{1}{16}C^{20}_{20,00} + \frac{5C^{20}_{20,20}}{16\sqrt{3}} - \frac{7C^{22}_{20,22}}{32\sqrt{15}} + \frac{C^{22}_{22,00}}{8\sqrt{5}} + \frac{1}{8}\sqrt{\frac{5}{3}}C^{22}_{22,20} - \frac{1}{16}\sqrt{\frac{7}{15}}C^{22}_{22,22},$$

$$C^{1111,1}_{00,3111} = \frac{1}{16}\sqrt{3}C^{40}_{00,00} + \frac{1}{16}C^{40}_{00,20} + \frac{7C^{42}_{00,22}}{32\sqrt{5}} - \frac{1}{16}\sqrt{3}C^{31}_{11,00} - \frac{1}{16}C^{31}_{11,20} - \frac{7C^{31}_{11,22}}{32\sqrt{5}} - \frac{3}{160}\sqrt{21}C^{33}_{11,22} + \frac{1}{16}\sqrt{3}C^{20}_{20,00} + \frac{1}{16}C^{20}_{20,20} + \frac{7C^{22}_{20,22}}{32\sqrt{5}} + \frac{1}{8}\sqrt{\frac{3}{5}}C^{22}_{22,00} + \frac{C^{22}_{22,20}}{8\sqrt{5}} + \frac{1}{16}\sqrt{\frac{7}{5}}C^{22}_{22,22}.$$

One of the 14 fourth order coupling constants is dependent to the others and can be expressed as function of the independent ones. The choice of the set of independent coupling constants is not unique. We did the following choice,

$$C^{1111,1}_{22,1111} = -\sqrt{\tfrac{3}{5}}C^{1111,0}_{20,1111} - \frac{C^{1111,1}_{20,1111}}{\sqrt{5}} + \sqrt{\tfrac{3}{5}}C^{0000,0}_{20,2000} + \frac{C^{0000,1}_{20,2000}}{\sqrt{5}} - \sqrt{3}C^{1111,0}_{22,1111} - \frac{\sqrt{3}C^{0000,0}_{22,2202}}{2} - \frac{C^{0000,1}_{22,2202}}{2}.$$

**13 fourth order parameters of the pseudopotential as function of the 13 independent coupling constants of the Galilean and spherical symmetric fourth - order EDF.**

$$C^{40}_{00,00} = \frac{3C^{2202,0}_{00,2202}}{\sqrt{5}} - \sqrt{\tfrac{3}{5}}C^{2202,1}_{00,2202} - 2C^{0000,0}_{20,2000} + \frac{2C^{0000,1}_{20,2000}}{\sqrt{3}} - \frac{4C^{0000,0}_{22,2202}}{\sqrt{5}} + \frac{4C^{0000,1}_{22,2202}}{\sqrt{15}} + 4C^{0000,0}_{40,0000} - \frac{4C^{0000,1}_{40,0000}}{\sqrt{3}},$$

$$C^{40}_{00,20} = \sqrt{\tfrac{3}{5}}C^{2202,0}_{00,2202} + \frac{3C^{2202,1}_{00,2202}}{\sqrt{5}} - \frac{2C^{0000,0}_{20,2000}}{\sqrt{3}} - 2C^{0000,1}_{20,2000} - \frac{4C^{0000,0}_{22,2202}}{\sqrt{15}} - \frac{4C^{0000,1}_{22,2202}}{\sqrt{5}} + \frac{4C^{0000,0}_{40,0000}}{\sqrt{3}} + 4C^{0000,1}_{40,0000},$$

$$C^{42}_{00,22} = \tfrac{4}{7}\sqrt{3}C^{2202,0}_{00,2202} - \tfrac{12}{7}C^{2202,1}_{00,2202} - \tfrac{2}{7}\sqrt{15}C^{1111,0}_{00,3111} + \tfrac{6}{7}\sqrt{5}C^{1111,1}_{00,3111} + \tfrac{4}{7}\sqrt{15}C^{1111,0}_{20,1111} - \frac{108C^{1111,1}_{20,1111}}{7\sqrt{5}} + \frac{68C^{0000,0}_{20,2000}}{7\sqrt{15}} - \tfrac{4}{7}\sqrt{5}C^{0000,1}_{20,2000} - \tfrac{16}{7}\sqrt{3}C^{1111,0}_{22,1111} - \frac{16C^{0000,0}_{22,2202}}{7\sqrt{3}} - \tfrac{8}{7}C^{0000,1}_{22,2202} - \tfrac{32}{7}\sqrt{\tfrac{5}{3}}C^{0000,0}_{40,0000} + \tfrac{32}{7}\sqrt{5}C^{0000,1}_{40,0000},$$

$$C^{31}_{11,00} = \frac{12C^{2202,0}_{00,2202}}{\sqrt{5}} - 4\sqrt{\tfrac{3}{5}}C^{2202,1}_{00,2202} - 16C^{0000,0}_{40,0000} + \frac{16C^{0000,1}_{40,0000}}{\sqrt{3}},$$

$$C^{31}_{11,20} = 4\sqrt{\tfrac{3}{5}}C^{2202,0}_{00,2202} - 4\sqrt{5}C^{2202,1}_{00,2202} - \frac{16C^{0000,0}_{40,0000}}{\sqrt{3}} + \tfrac{80}{3}C^{0000,1}_{40,0000},$$

$$C^{31}_{11,22} = \tfrac{8}{5}\sqrt{3}C^{2202,0}_{00,2202} + \tfrac{8}{5}C^{2202,1}_{00,2202} - 4\sqrt{\tfrac{3}{5}}C^{1111,0}_{00,3111} - \frac{4C^{1111,1}_{00,3111}}{\sqrt{5}} + \tfrac{24}{5}\sqrt{\tfrac{3}{5}}C^{1111,0}_{20,1111} + \frac{24C^{1111,1}_{20,1111}}{5\sqrt{5}} - \tfrac{24}{5}\sqrt{\tfrac{3}{5}}C^{0000,0}_{20,2000} - \frac{24C^{0000,1}_{20,2000}}{5\sqrt{5}} + \frac{64C^{0000,0}_{40,0000}}{\sqrt{15}} + \frac{64C^{0000,1}_{40,0000}}{3\sqrt{5}},$$

$$C^{33}_{11,22} = \frac{8C^{2202,0}_{00,2202}}{\sqrt{35}} + \frac{8C^{2202,1}_{00,2202}}{\sqrt{105}} - \frac{4C^{1111,0}_{00,3111}}{\sqrt{7}} - \frac{4C^{1111,1}_{00,3111}}{\sqrt{21}} - \tfrac{8}{5}\sqrt{7}C^{1111,0}_{20,1111} - \tfrac{8}{5}\sqrt{\tfrac{7}{3}}C^{1111,1}_{20,1111} + \tfrac{8}{5}\sqrt{7}C^{0000,0}_{20,2000} + \tfrac{8}{5}\sqrt{\tfrac{7}{3}}C^{0000,1}_{20,2000} + \frac{64C^{0000,0}_{40,0000}}{3\sqrt{7}} + \frac{64C^{0000,1}_{40,0000}}{3\sqrt{21}},$$

$$C^{20}_{20,00} = \sqrt{5}C^{2202,0}_{00,2202} - \sqrt{\tfrac{5}{3}}C^{2202,1}_{00,2202} - \tfrac{2}{3}C^{0000,0}_{20,2000} + \frac{2C^{0000,1}_{20,2000}}{3\sqrt{3}} + \tfrac{4}{3}\sqrt{5}C^{0000,0}_{22,2202} - \tfrac{4}{3}\sqrt{\tfrac{5}{3}}C^{0000,1}_{22,2202} + \tfrac{20}{3}C^{0000,0}_{40,0000} - \frac{20C^{0000,1}_{40,0000}}{3\sqrt{3}},$$

$$C^{20}_{20,20} = \sqrt{\tfrac{5}{3}}C^{2202,0}_{00,2202} + \sqrt{5}C^{2202,1}_{00,2202} - \frac{2C^{0000,0}_{20,2000}}{3\sqrt{3}} - \tfrac{2}{3}C^{0000,1}_{20,2000} + \tfrac{4}{3}\sqrt{\tfrac{5}{3}}C^{0000,0}_{22,2202} + \tfrac{4}{3}\sqrt{5}C^{0000,1}_{22,2202} + \frac{20C^{0000,0}_{40,0000}}{3\sqrt{3}} + \tfrac{20}{3}C^{0000,1}_{40,0000},$$

$$C^{22}_{20,22} = \frac{4C^{2202,0}_{00,2202}}{\sqrt{3}} - 4C^{2202,1}_{00,2202} - 2\sqrt{\tfrac{5}{3}}C^{1111,0}_{00,3111} + 2\sqrt{5}C^{1111,1}_{00,3111} + \frac{4C^{1111,0}_{20,1111}}{\sqrt{15}} + \frac{12C^{1111,1}_{20,1111}}{\sqrt{5}} - \frac{44C^{0000,0}_{20,2000}}{3\sqrt{15}} - \frac{4C^{0000,1}_{20,2000}}{3\sqrt{5}} + \frac{16C^{1111,0}_{22,1111}}{\sqrt{3}} + \frac{16C^{0000,0}_{22,2202}}{3\sqrt{3}} + \tfrac{8}{3}C^{0000,1}_{22,2202} - \tfrac{32}{3}\sqrt{\tfrac{5}{3}}C^{0000,0}_{40,0000} + \tfrac{32}{3}\sqrt{5}C^{0000,1}_{40,0000},$$

$$C^{22}_{22,00} = 2C^{2202,0}_{00,2202} - \frac{2C^{2202,1}_{00,2202}}{\sqrt{3}} + \tfrac{4}{3}\sqrt{5}C^{0000,0}_{20,2000} - \tfrac{4}{3}\sqrt{\tfrac{5}{3}}C^{0000,1}_{20,2000} - \tfrac{4}{3}C^{0000,0}_{22,2202} + \frac{4C^{0000,1}_{22,2202}}{3\sqrt{3}} + \tfrac{8}{3}\sqrt{5}C^{0000,0}_{40,0000} - \tfrac{8}{3}\sqrt{\tfrac{5}{3}}C^{0000,1}_{40,0000},$$

$$C^{22}_{22,20} = \frac{2C^{2202,0}_{00,2202}}{\sqrt{3}} + 2C^{2202,1}_{00,2202} + \frac{4}{3}\sqrt{\frac{5}{3}}C^{0000,0}_{20,2000} + \frac{4}{3}\sqrt{5}C^{0000,1}_{20,2000} - \frac{4C^{0000,0}_{22,2202}}{3\sqrt{3}} - \frac{4}{3}C^{0000,1}_{22,2202} + \frac{8}{3}\sqrt{\frac{5}{3}}C^{0000,0}_{40,0000} + \frac{8}{3}\sqrt{5}C^{0000,1}_{40,0000},$$

$$C^{22}_{22,22} = \frac{4C^{2202,0}_{00,2202}}{\sqrt{21}} - \frac{4C^{2202,1}_{00,2202}}{\sqrt{7}} - 2\sqrt{\frac{5}{21}}C^{1111,0}_{00,3111} + 2\sqrt{\frac{5}{7}}C^{1111,1}_{00,3111} - \frac{44C^{1111,0}_{20,1111}}{\sqrt{105}} + \frac{12C^{1111,1}_{20,1111}}{\sqrt{35}} + \frac{52C^{0000,0}_{20,2000}}{3\sqrt{105}} + \frac{44C^{0000,1}_{20,2000}}{3\sqrt{35}} - \frac{32C^{1111,0}_{22,1111}}{\sqrt{21}} - \frac{32C^{0000,0}_{22,2202}}{3\sqrt{21}} - \frac{16C^{0000,1}_{22,2202}}{3\sqrt{7}} - \frac{32}{3}\sqrt{\frac{5}{21}}C^{0000,0}_{40,0000} + \frac{32}{3}\sqrt{\frac{5}{7}}C^{0000,1}_{40,0000}.$$

## 24 sixth - order coupling constants of the Galilean and spherical symmetric EDF expressed by 22 pseudopotential parameters (Spin-Orbit terms excluded).

$$C^{0000,0}_{60,0000} = -\frac{3}{512}C^{60}_{00,00} - \frac{1}{512}\sqrt{3}C^{60}_{00,20} + \frac{5}{512}C^{51}_{11,00} - \frac{1}{512}\sqrt{3}C^{51}_{11,20} - \frac{3}{512}C^{40}_{20,00} - \frac{1}{512}\sqrt{3}C^{40}_{20,20} - \frac{3C^{42}_{22,00}}{256\sqrt{5}} - \frac{1}{256}\sqrt{\frac{3}{5}}C^{42}_{22,20} + \frac{5}{512}C^{31}_{31,00} - \frac{1}{512}\sqrt{3}C^{31}_{31,20} + \frac{3}{256}\sqrt{\frac{3}{7}}C^{33}_{33,00} - \frac{9C^{33}_{33,20}}{1280\sqrt{7}},$$

$$C^{0000,1}_{60,0000} = \frac{1}{512}\sqrt{3}C^{60}_{00,00} - \frac{3}{512}C^{60}_{00,20} + \frac{1}{512}\sqrt{3}C^{51}_{11,00} - \frac{3}{512}C^{51}_{11,20} + \frac{1}{512}\sqrt{3}C^{40}_{20,00} - \frac{3}{512}C^{40}_{20,20} + \frac{1}{256}\sqrt{\frac{3}{5}}C^{42}_{22,00} - \frac{3C^{42}_{22,20}}{256\sqrt{5}} + \frac{1}{512}\sqrt{3}C^{31}_{31,00} - \frac{3}{512}C^{31}_{31,20} + \frac{9C^{33}_{33,00}}{1280\sqrt{7}} - \frac{9\sqrt{\frac{3}{7}}C^{33}_{33,20}}{1280},$$

$$C^{0000,0}_{40,2000} = \frac{21}{256}C^{60}_{00,00} + \frac{7}{256}\sqrt{3}C^{60}_{00,20} - \frac{35}{768}C^{51}_{11,00} + \frac{7C^{51}_{11,20}}{256\sqrt{3}} + \frac{5}{256}C^{40}_{20,00} + \frac{5C^{40}_{20,20}}{256\sqrt{3}} - \frac{7C^{42}_{22,00}}{128\sqrt{5}} - \frac{7C^{42}_{22,20}}{128\sqrt{15}} + \frac{5}{768}C^{31}_{31,00} - \frac{C^{31}_{31,20}}{256\sqrt{3}} + \frac{3}{128}\sqrt{21}C^{33}_{33,00} - \frac{9}{640}\sqrt{7}C^{33}_{33,20},$$

$$C^{0000,1}_{40,2000} = -\frac{7}{256}\sqrt{3}C^{60}_{00,00} + \frac{21}{256}C^{60}_{00,20} - \frac{7C^{51}_{11,00}}{256\sqrt{3}} + \frac{7}{256}C^{51}_{11,20} - \frac{5C^{40}_{20,00}}{256\sqrt{3}} + \frac{5}{256}C^{40}_{20,20} + \frac{7C^{42}_{22,00}}{128\sqrt{15}} - \frac{7C^{42}_{22,20}}{128\sqrt{5}} + \frac{C^{31}_{31,00}}{256\sqrt{3}} - \frac{1}{256}C^{31}_{31,20} + \frac{9}{640}\sqrt{7}C^{33}_{33,00} - \frac{9}{640}\sqrt{21}C^{33}_{33,20},$$

$$C^{0000,0}_{42,2202} = \frac{3}{64}\sqrt{5}C^{60}_{00,00} + \frac{1}{64}\sqrt{15}C^{60}_{00,20} - \frac{5}{192}\sqrt{5}C^{51}_{11,00} + \frac{1}{64}\sqrt{\frac{5}{3}}C^{51}_{11,20} - \frac{1}{64}\sqrt{5}C^{40}_{20,00} - \frac{1}{64}\sqrt{\frac{5}{3}}C^{40}_{20,20} + \frac{1}{64}C^{42}_{22,00} + \frac{C^{42}_{22,20}}{64\sqrt{3}} + \frac{5}{192}\sqrt{5}C^{31}_{31,00} - \frac{1}{64}\sqrt{\frac{5}{3}}C^{31}_{31,20} - \frac{3}{64}\sqrt{\frac{15}{7}}C^{33}_{33,00} + \frac{9C^{33}_{33,20}}{64\sqrt{35}},$$

$$C^{0000,1}_{42,2202} = -\frac{1}{64}\sqrt{15}C^{60}_{00,00} + \frac{3}{64}\sqrt{5}C^{60}_{00,20} - \frac{1}{64}\sqrt{\frac{5}{3}}C^{51}_{11,00} + \frac{1}{64}\sqrt{5}C^{51}_{11,20} + \frac{1}{64}\sqrt{\frac{5}{3}}C^{40}_{20,00} - \frac{1}{64}\sqrt{5}C^{40}_{20,20} - \frac{C^{42}_{22,00}}{64\sqrt{3}} + \frac{1}{64}C^{42}_{22,20} + \frac{1}{64}\sqrt{\frac{5}{3}}C^{31}_{31,00} - \frac{1}{64}\sqrt{5}C^{31}_{31,20} - \frac{9C^{33}_{33,00}}{64\sqrt{35}} + \frac{9}{64}\sqrt{\frac{3}{35}}C^{33}_{33,20},$$

$$C^{2000,0}_{00,4000} = \frac{21}{256}C^{60}_{00,00} + \frac{7}{256}\sqrt{3}C^{60}_{00,20} + \frac{35}{256}C^{51}_{11,00} - \frac{7}{256}\sqrt{3}C^{51}_{11,20} + \frac{21}{256}C^{40}_{20,00} + \frac{7}{256}\sqrt{3}C^{40}_{20,20} + \frac{21C^{42}_{22,00}}{128\sqrt{5}} + \frac{7}{128}\sqrt{\frac{3}{5}}C^{42}_{22,20} + \frac{35}{256}C^{31}_{31,00} - \frac{7}{256}\sqrt{3}C^{31}_{31,20} + \frac{3}{128}\sqrt{21}C^{33}_{33,00} - \frac{9}{640}\sqrt{7}C^{33}_{33,20},$$

$$C^{2000,1}_{00,4000} = -\frac{7}{256}\sqrt{3}C^{60}_{00,00} + \frac{21}{256}C^{60}_{00,20} + \frac{7}{256}\sqrt{3}C^{51}_{11,00} - \frac{21}{256}C^{51}_{11,20} - \frac{7}{256}\sqrt{3}C^{40}_{20,00} + \frac{21}{256}C^{40}_{20,20} - \frac{7}{128}\sqrt{\frac{3}{5}}C^{42}_{22,00} + \frac{21C^{42}_{22,20}}{128\sqrt{5}} + \frac{7}{256}\sqrt{3}C^{31}_{31,00} - \frac{21}{256}C^{31}_{31,20} + \frac{9}{640}\sqrt{7}C^{33}_{33,00} - \frac{9}{640}\sqrt{21}C^{33}_{33,20},$$

$$C^{2202,0}_{20,2202} = -\frac{7}{128}\sqrt{5}C^{60}_{00,00} - \frac{7}{128}\sqrt{\frac{5}{3}}C^{60}_{00,20} - \frac{35\sqrt{5}C^{51}_{11,00}}{1152} + \frac{7}{384}\sqrt{\frac{5}{3}}C^{51}_{11,20} - \frac{5}{384}\sqrt{5}C^{40}_{20,00} - \frac{5}{384}\sqrt{\frac{5}{3}}C^{40}_{20,20} + \frac{7}{192}C^{42}_{22,00} + \frac{7C^{42}_{22,20}}{192\sqrt{3}} + \frac{5\sqrt{5}C^{31}_{31,00}}{1152} - \frac{1}{384}\sqrt{\frac{5}{3}}C^{31}_{31,20} + \frac{1}{64}\sqrt{105}C^{33}_{33,00} -$$

$\frac{3}{64}\sqrt{\frac{7}{5}}C^{33}_{33,20}$,

$C^{2202,1}_{20,2202} = \frac{7}{128}\sqrt{\frac{5}{3}}C^{60}_{00,00} - \frac{7}{128}\sqrt{5}C^{60}_{00,20} - \frac{7}{384}\sqrt{\frac{5}{3}}C^{51}_{11,00} + \frac{7}{384}\sqrt{5}C^{51}_{11,20} + \frac{5}{384}\sqrt{\frac{5}{3}}C^{40}_{20,00} - \frac{5}{384}\sqrt{5}C^{40}_{20,20} - \frac{7C^{42}_{22,00}}{192\sqrt{3}} + \frac{7}{192}C^{42}_{22,20} + \frac{1}{384}\sqrt{\frac{5}{3}}C^{31}_{31,00} - \frac{1}{384}\sqrt{5}C^{31}_{31,20} + \frac{3}{64}\sqrt{\frac{7}{5}}C^{33}_{33,00} - \frac{3}{64}\sqrt{\frac{21}{5}}C^{33}_{33,20}$,

$C^{2202,0}_{22,2202} = -\frac{1}{64}\sqrt{35}C^{60}_{00,00} - \frac{1}{64}\sqrt{\frac{35}{3}}C^{60}_{00,20} - \frac{5}{576}\sqrt{35}C^{51}_{11,00} + \frac{1}{192}\sqrt{\frac{35}{3}}C^{51}_{11,20} + \frac{1}{192}\sqrt{35}C^{40}_{20,00} + \frac{1}{192}\sqrt{\frac{35}{3}}C^{40}_{20,20} - \frac{1}{192}\sqrt{7}C^{42}_{22,00} - \frac{1}{192}\sqrt{\frac{7}{3}}C^{42}_{22,20} + \frac{5}{576}\sqrt{35}C^{31}_{31,00} - \frac{1}{192}\sqrt{\frac{35}{3}}C^{31}_{31,20} - \frac{1}{64}\sqrt{15}C^{33}_{33,00} + \frac{3C^{33}_{33,20}}{64\sqrt{5}}$,

$C^{2202,1}_{22,2202} = \frac{1}{64}\sqrt{\frac{35}{3}}C^{60}_{00,00} - \frac{1}{64}\sqrt{35}C^{60}_{00,20} - \frac{1}{192}\sqrt{\frac{35}{3}}C^{51}_{11,00} + \frac{1}{192}\sqrt{35}C^{51}_{11,20} - \frac{1}{192}\sqrt{\frac{35}{3}}C^{40}_{20,00} + \frac{1}{192}\sqrt{35}C^{40}_{20,20} + \frac{1}{192}\sqrt{\frac{7}{3}}C^{42}_{22,00} - \frac{1}{192}\sqrt{7}C^{42}_{22,20} + \frac{1}{192}\sqrt{\frac{35}{3}}C^{31}_{31,00} - \frac{1}{192}\sqrt{35}C^{31}_{31,20} - \frac{3C^{33}_{33,00}}{64\sqrt{5}} + \frac{3}{64}\sqrt{\frac{3}{5}}C^{33}_{33,20}$,

$C^{1111,0}_{40,1111} = \frac{7}{256}C^{60}_{00,00} + \frac{35C^{60}_{00,20}}{256\sqrt{3}} - \frac{7}{256}\sqrt{\frac{3}{5}}C^{62}_{00,22} + \frac{7}{768}C^{51}_{11,00} - \frac{7C^{51}_{11,20}}{256\sqrt{3}} - \frac{7C^{51}_{11,22}}{256\sqrt{15}} + \frac{27\sqrt{7}C^{53}_{11,22}}{1280} + \frac{5}{768}C^{40}_{20,00} + \frac{25C^{40}_{20,20}}{768\sqrt{3}} - \frac{7C^{42}_{20,22}}{768\sqrt{15}} - \frac{7C^{42}_{22,00}}{384\sqrt{5}} - \frac{7}{384}\sqrt{\frac{5}{3}}C^{42}_{22,20} + \frac{17C^{40}_{22,22}}{768\sqrt{15}} + \frac{1}{384}\sqrt{\frac{35}{3}}C^{42}_{22,22} - \frac{3}{320}\sqrt{3}C^{44}_{22,22} - \frac{1}{768}C^{31}_{31,00} + \frac{C^{31}_{31,20}}{256\sqrt{3}} - \frac{23C^{31}_{31,22}}{256\sqrt{15}} + \frac{3\sqrt{7}C^{33}_{31,22}}{1280} - \frac{3}{640}\sqrt{21}C^{33}_{33,00} + \frac{9}{640}\sqrt{7}C^{33}_{33,20} - \frac{9}{320}\sqrt{\frac{21}{10}}C^{33}_{33,22}$,

$C^{1111,1}_{40,1111} = \frac{7}{256}\sqrt{3}C^{60}_{00,00} + \frac{7}{256}C^{60}_{00,20} + \frac{21C^{62}_{00,22}}{256\sqrt{5}} + \frac{7C^{51}_{11,00}}{256\sqrt{3}} + \frac{7}{768}C^{51}_{11,20} - \frac{7C^{51}_{11,22}}{768\sqrt{5}} + \frac{9\sqrt{21}C^{53}_{11,22}}{1280} + \frac{5C^{40}_{20,00}}{256\sqrt{3}} + \frac{5}{768}C^{40}_{20,20} + \frac{7C^{42}_{20,22}}{768\sqrt{5}} - \frac{7C^{42}_{22,00}}{128\sqrt{15}} - \frac{7C^{42}_{22,20}}{384\sqrt{5}} - \frac{17C^{40}_{22,22}}{768\sqrt{5}} - \frac{1}{384}\sqrt{35}C^{42}_{22,22} + \frac{9}{320}C^{44}_{22,22} - \frac{C^{31}_{31,00}}{256\sqrt{3}} - \frac{1}{768}C^{31}_{31,20} - \frac{23C^{31}_{31,22}}{768\sqrt{5}} + \frac{\sqrt{21}C^{33}_{31,22}}{1280} - \frac{9}{640}\sqrt{7}C^{33}_{33,00} - \frac{3}{640}\sqrt{21}C^{33}_{33,20} - \frac{9}{320}\sqrt{\frac{7}{10}}C^{33}_{33,22}$,

$C^{1111,0}_{42,1111} = -\frac{1}{128}\sqrt{5}C^{60}_{00,00} - \frac{5}{128}\sqrt{\frac{5}{3}}C^{60}_{00,20} + \frac{1}{128}\sqrt{3}C^{62}_{00,22} - \frac{1}{384}\sqrt{5}C^{51}_{11,00} + \frac{1}{128}\sqrt{\frac{5}{3}}C^{51}_{11,20} + \frac{C^{51}_{11,22}}{128\sqrt{3}} - \frac{27C^{53}_{11,22}}{128\sqrt{35}} + \frac{1}{384}\sqrt{5}C^{40}_{20,00} + \frac{5}{384}\sqrt{\frac{5}{3}}C^{40}_{20,20} - \frac{5C^{42}_{20,22}}{384\sqrt{3}} - \frac{1}{384}C^{42}_{22,00} - \frac{5C^{42}_{22,20}}{384\sqrt{3}} - \frac{11C^{40}_{22,22}}{384\sqrt{3}} + \frac{C^{42}_{22,22}}{12\sqrt{21}} + \frac{3}{224}\sqrt{\frac{3}{5}}C^{44}_{22,22} + \frac{1}{384}\sqrt{5}C^{31}_{31,00} - \frac{1}{128}\sqrt{\frac{5}{3}}C^{31}_{31,20} + \frac{5C^{31}_{31,22}}{128\sqrt{3}} + \frac{3}{128}\sqrt{\frac{5}{7}}C^{33}_{31,22} - \frac{3}{128}\sqrt{\frac{3}{35}}C^{33}_{33,00} + \frac{9C^{33}_{33,20}}{128\sqrt{35}} - \frac{9}{32}\sqrt{\frac{3}{14}}C^{33}_{33,22}$,

$C^{1111,1}_{42,1111} = -\frac{1}{128}\sqrt{15}C^{60}_{00,00} - \frac{1}{128}\sqrt{5}C^{60}_{00,20} - \frac{3}{128}C^{62}_{00,22} - \frac{1}{128}\sqrt{\frac{5}{3}}C^{51}_{11,00} - \frac{1}{384}\sqrt{5}C^{51}_{11,20} + \frac{1}{384}C^{51}_{11,22} - \frac{9}{128}\sqrt{\frac{3}{35}}C^{53}_{11,22} + \frac{1}{128}\sqrt{\frac{5}{3}}C^{40}_{20,00} + \frac{1}{384}\sqrt{5}C^{40}_{20,20} + \frac{5}{384}C^{42}_{20,22} - \frac{C^{42}_{22,00}}{128\sqrt{3}} - \frac{1}{384}C^{42}_{22,20} + \frac{11}{384}C^{40}_{22,22} - \frac{C^{42}_{22,22}}{12\sqrt{7}} - \frac{9C^{44}_{22,22}}{224\sqrt{5}} + \frac{1}{128}\sqrt{\frac{5}{3}}C^{31}_{31,00} + \frac{1}{384}\sqrt{5}C^{31}_{31,20} + \frac{5}{384}C^{31}_{31,22} + \frac{1}{128}\sqrt{\frac{15}{7}}C^{33}_{31,22} - \frac{9C^{33}_{33,00}}{128\sqrt{35}} - \frac{3}{128}\sqrt{\frac{3}{35}}C^{33}_{33,20} - \frac{9C^{33}_{33,22}}{32\sqrt{14}}$,

$C^{1111,0}_{20,3111} = -\frac{7}{64}C^{60}_{00,00} - \frac{35C^{60}_{00,20}}{64\sqrt{3}} + \frac{7}{64}\sqrt{\frac{3}{5}}C^{62}_{00,22} + \frac{7}{192}C^{51}_{11,00} - \frac{7C^{51}_{11,20}}{64\sqrt{3}} + \frac{7}{64}\sqrt{\frac{5}{3}}C^{51}_{11,22} - \frac{5}{192}C^{40}_{20,00} - \frac{25C^{40}_{20,20}}{192\sqrt{3}} + \frac{7C^{42}_{20,22}}{192\sqrt{15}} + \frac{7C^{42}_{22,00}}{96\sqrt{5}} + \frac{7}{96}\sqrt{\frac{5}{3}}C^{42}_{22,20} + \frac{7C^{40}_{22,22}}{192\sqrt{15}} - \frac{1}{48}\sqrt{\frac{7}{15}}C^{42}_{22,22} -$

$$\frac{3}{80}\sqrt{3}C^{44}_{22,22}-\frac{1}{192}C^{31}_{31,00}+\frac{C^{31}_{31,20}}{64\sqrt{3}}+\frac{7C^{31}_{31,22}}{64\sqrt{15}}-\frac{3}{80}\sqrt{7}C^{33}_{31,22}-\frac{3}{160}\sqrt{21}C^{33}_{33,00}+\frac{9}{160}\sqrt{7}C^{33}_{33,20}-\frac{9}{80}\sqrt{\frac{21}{10}}C^{33}_{33,22},$$

$$C^{1111,1}_{20,3111}=-\frac{7}{64}\sqrt{3}C^{60}_{00,00}-\frac{7}{64}C^{60}_{00,20}-\frac{21C^{62}_{00,22}}{64\sqrt{5}}+\frac{7C^{51}_{11,00}}{64\sqrt{3}}+\frac{7}{192}C^{51}_{11,20}+\frac{7}{192}\sqrt{5}C^{51}_{11,22}-\frac{5C^{40}_{20,00}}{64\sqrt{3}}-\frac{5}{192}C^{40}_{20,20}-\frac{7C^{42}_{20,22}}{192\sqrt{5}}+\frac{7C^{42}_{22,00}}{32\sqrt{15}}+\frac{7C^{42}_{22,20}}{96\sqrt{5}}-\frac{7C^{40}_{22,22}}{192\sqrt{5}}+\frac{1}{48}\sqrt{\frac{7}{5}}C^{42}_{22,22}+\frac{9}{80}C^{44}_{22,22}-\frac{C^{31}_{31,00}}{64\sqrt{3}}-\frac{1}{192}C^{31}_{31,20}+\frac{7C^{31}_{31,22}}{192\sqrt{5}}-\frac{1}{80}\sqrt{21}C^{33}_{31,22}-\frac{9}{160}\sqrt{7}C^{33}_{33,00}-\frac{3}{160}\sqrt{21}C^{33}_{33,20}-\frac{9}{80}\sqrt{\frac{7}{10}}C^{33}_{33,22},$$

$$C^{1111,0}_{22,3313}=-\frac{1}{48}\sqrt{\frac{7}{2}}C^{60}_{00,00}-\frac{5}{48}\sqrt{\frac{7}{6}}C^{60}_{00,20}+\frac{1}{16}\sqrt{\frac{7}{30}}C^{62}_{00,22}+\frac{1}{144}\sqrt{\frac{7}{2}}C^{51}_{11,00}-\frac{1}{48}\sqrt{\frac{7}{6}}C^{51}_{11,20}+\frac{1}{48}\sqrt{\frac{35}{6}}C^{51}_{11,22}+\frac{1}{144}\sqrt{\frac{7}{2}}C^{40}_{20,00}+\frac{5}{144}\sqrt{\frac{7}{6}}C^{40}_{20,20}-\frac{1}{144}\sqrt{\frac{35}{6}}C^{42}_{20,22}-\frac{1}{144}\sqrt{\frac{7}{10}}C^{42}_{22,00}-\frac{1}{144}\sqrt{\frac{35}{6}}C^{42}_{22,20}+\frac{1}{144}\sqrt{\frac{7}{30}}C^{40}_{22,22}+\frac{C^{42}_{22,22}}{18\sqrt{30}}+\frac{1}{80}\sqrt{\frac{3}{14}}C^{44}_{22,22}-\frac{1}{144}\sqrt{\frac{7}{2}}C^{31}_{31,00}+\frac{1}{48}\sqrt{\frac{7}{6}}C^{31}_{31,20}-\frac{1}{48}\sqrt{\frac{35}{6}}C^{31}_{31,22}+\frac{1}{80}\sqrt{\frac{3}{2}}C^{33}_{33,00}-\frac{3C^{33}_{33,20}}{80\sqrt{2}}+\frac{3}{32}\sqrt{\frac{3}{5}}C^{33}_{33,22},$$

$$C^{1111,1}_{22,3313}=-\frac{1}{16}\sqrt{\frac{7}{6}}C^{60}_{00,00}-\frac{1}{48}\sqrt{\frac{7}{2}}C^{60}_{00,20}-\frac{1}{16}\sqrt{\frac{7}{10}}C^{62}_{00,22}+\frac{1}{48}\sqrt{\frac{7}{6}}C^{51}_{11,00}+\frac{1}{144}\sqrt{\frac{7}{2}}C^{51}_{11,20}+\frac{1}{144}\sqrt{\frac{35}{2}}C^{51}_{11,22}+\frac{1}{48}\sqrt{\frac{7}{6}}C^{40}_{20,00}+\frac{1}{144}\sqrt{\frac{7}{2}}C^{40}_{20,20}+\frac{1}{144}\sqrt{\frac{35}{2}}C^{42}_{20,22}-\frac{1}{48}\sqrt{\frac{7}{30}}C^{42}_{22,00}-\frac{1}{144}\sqrt{\frac{7}{10}}C^{42}_{22,20}-\frac{1}{144}\sqrt{\frac{7}{10}}C^{40}_{22,22}-\frac{C^{42}_{22,22}}{18\sqrt{10}}-\frac{3C^{44}_{22,22}}{80\sqrt{14}}-\frac{1}{48}\sqrt{\frac{7}{6}}C^{31}_{31,00}-\frac{1}{144}\sqrt{\frac{7}{2}}C^{31}_{31,20}-\frac{1}{144}\sqrt{\frac{35}{2}}C^{31}_{31,22}+\frac{3C^{33}_{33,00}}{80\sqrt{2}}+\frac{1}{80}\sqrt{\frac{3}{2}}C^{33}_{33,20}+\frac{3C^{33}_{33,22}}{32\sqrt{5}},$$

$$C^{1111,0}_{00,5111}=\frac{3}{128}C^{60}_{00,00}+\frac{5}{128}\sqrt{3}C^{60}_{00,20}-\frac{3}{128}\sqrt{\frac{3}{5}}C^{62}_{00,22}-\frac{3}{128}C^{51}_{11,00}+\frac{3}{128}\sqrt{3}C^{51}_{11,20}-\frac{9}{128}\sqrt{\frac{3}{5}}C^{51}_{11,22}-\frac{81C^{53}_{11,22}}{640\sqrt{7}}+\frac{3}{128}C^{40}_{20,00}+\frac{5}{128}\sqrt{3}C^{40}_{20,20}-\frac{3}{128}\sqrt{\frac{3}{5}}C^{42}_{20,22}+\frac{3C^{42}_{22,00}}{64\sqrt{5}}+\frac{1}{64}\sqrt{15}C^{42}_{22,20}-\frac{3}{128}\sqrt{\frac{3}{5}}C^{40}_{22,22}-\frac{3}{64}\sqrt{\frac{3}{35}}C^{42}_{22,22}-\frac{9\sqrt{3}C^{44}_{22,22}}{1120}-\frac{3}{128}C^{31}_{31,00}+\frac{3}{128}\sqrt{3}C^{31}_{31,20}-\frac{9}{128}\sqrt{\frac{3}{5}}C^{31}_{31,22}-\frac{81C^{33}_{31,22}}{640\sqrt{7}}-\frac{9}{320}\sqrt{\frac{3}{7}}C^{33}_{33,00}+\frac{27C^{33}_{33,20}}{320\sqrt{7}}-\frac{27}{160}\sqrt{\frac{3}{70}}C^{33}_{33,22},$$

$$C^{1111,1}_{00,5111}=\frac{3}{128}\sqrt{3}C^{60}_{00,00}+\frac{3}{128}C^{60}_{00,20}+\frac{9C^{62}_{00,22}}{128\sqrt{5}}-\frac{3}{128}\sqrt{3}C^{51}_{11,00}-\frac{3}{128}C^{51}_{11,20}-\frac{9C^{51}_{11,22}}{128\sqrt{5}}-\frac{27}{640}\sqrt{\frac{3}{7}}C^{53}_{11,22}+\frac{3}{128}\sqrt{3}C^{40}_{20,00}+\frac{3}{128}C^{40}_{20,20}+\frac{9C^{42}_{20,22}}{128\sqrt{5}}+\frac{3}{64}\sqrt{\frac{3}{5}}C^{42}_{22,00}+\frac{3C^{42}_{22,20}}{64\sqrt{5}}+\frac{9C^{40}_{22,22}}{128\sqrt{5}}+\frac{9C^{42}_{22,22}}{64\sqrt{35}}+\frac{27C^{44}_{22,22}}{1120}-\frac{3}{128}\sqrt{3}C^{31}_{31,00}-\frac{3}{128}C^{31}_{31,20}-\frac{9C^{31}_{31,22}}{128\sqrt{5}}-\frac{27}{640}\sqrt{\frac{3}{7}}C^{33}_{31,22}-\frac{27C^{33}_{33,00}}{320\sqrt{7}}-\frac{9}{320}\sqrt{\frac{3}{7}}C^{33}_{33,20}-\frac{27C^{33}_{33,22}}{160\sqrt{70}},$$

$$C^{3111,0}_{00,3111}=\frac{21}{640}C^{60}_{00,00}+\frac{7}{128}\sqrt{3}C^{60}_{00,20}-\frac{21}{640}\sqrt{\frac{3}{5}}C^{62}_{00,22}-\frac{21}{640}C^{51}_{11,00}+\frac{21}{640}\sqrt{3}C^{51}_{11,20}-\frac{63}{640}\sqrt{\frac{3}{5}}C^{51}_{11,22}-\frac{81\sqrt{7}C^{53}_{11,22}}{3200}+\frac{21}{640}C^{40}_{20,00}+\frac{7}{128}\sqrt{3}C^{40}_{20,20}-\frac{21}{640}\sqrt{\frac{3}{5}}C^{42}_{20,22}+\frac{21C^{42}_{22,00}}{320\sqrt{5}}+\frac{7}{64}\sqrt{\frac{3}{5}}C^{42}_{22,20}-\frac{21}{640}\sqrt{\frac{3}{5}}C^{40}_{22,22}-\frac{3}{320}\sqrt{\frac{21}{5}}C^{42}_{22,22}-\frac{9}{800}\sqrt{3}C^{44}_{22,22}-\frac{21}{640}C^{31}_{31,00}+\frac{21}{640}\sqrt{3}C^{31}_{31,20}-\frac{63}{640}\sqrt{\frac{3}{5}}C^{31}_{31,22}-\frac{81\sqrt{7}C^{33}_{31,22}}{3200}-\frac{9\sqrt{21}C^{33}_{33,00}}{1600}+\frac{27\sqrt{7}C^{33}_{33,20}}{1600}-\frac{27}{800}\sqrt{\frac{21}{10}}C^{33}_{33,22},$$

$$C^{3111,1}_{00,3111}=\frac{21}{640}\sqrt{3}C^{60}_{00,00}+\frac{21}{640}C^{60}_{00,20}+\frac{63C^{62}_{00,22}}{640\sqrt{5}}-\frac{21}{640}\sqrt{3}C^{51}_{11,00}-\frac{21}{640}C^{51}_{11,20}-\frac{63C^{51}_{11,22}}{640\sqrt{5}}-\frac{27\sqrt{21}C^{53}_{11,22}}{3200}+\frac{21}{640}\sqrt{3}C^{40}_{20,00}+\frac{21}{640}C^{40}_{20,20}+\frac{63C^{42}_{20,22}}{640\sqrt{5}}+\frac{21}{320}\sqrt{\frac{3}{5}}C^{42}_{22,00}+$$

$$\frac{21C^{42}_{22,20}}{320\sqrt{5}}+\frac{63C^{40}_{22,22}}{640\sqrt{5}}+\frac{9}{320}\sqrt{\frac{7}{5}}C^{42}_{22,22}+\frac{27}{800}C^{44}_{22,22}-\frac{21}{640}\sqrt{3}C^{31}_{31,00}-\frac{21}{640}C^{31}_{31,20}-\frac{63C^{31}_{31,22}}{640\sqrt{5}}-\frac{27\sqrt{21}C^{33}_{31,22}}{3200}-\frac{27\sqrt{7}C^{33}_{33,00}}{1600}-\frac{9\sqrt{21}C^{33}_{33,20}}{1600}-\frac{27}{800}\sqrt{\frac{7}{10}}C^{33}_{33,22}.$$

2 out of the 24 sixth order coupling constants is dependent to the others and can be expressed as function of the independent ones. The choice of the set of independent coupling constants is not unique. We did the following choice,

$$C^{3111,0}_{00,3111}=\frac{7C^{1111,0}_{00,5111}}{5},$$

$$C^{3111,1}_{00,3111}=\frac{7C^{1111,1}_{00,5111}}{5}.$$

**22 sixth order parameters of the pseudopotential as function of the 22 independent coupling constants of the Galilean and spherical symmetric sixth-order EDF .**

$$C^{60}_{00,00}=\frac{2}{7}C^{2000,0}_{00,4000}-\frac{2C^{2000,1}_{00,4000}}{7\sqrt{3}}-\frac{3C^{2202,0}_{20,2202}}{\sqrt{5}}+\sqrt{\frac{3}{5}}C^{2202,1}_{20,2202}-\frac{12C^{2202,0}_{22,2202}}{\sqrt{35}}+4\sqrt{\frac{3}{35}}C^{2202,1}_{22,2202}+2C^{0000,0}_{40,2000}-\frac{2C^{0000,1}_{40,2000}}{\sqrt{3}}+\frac{4C^{0000,0}_{42,2202}}{\sqrt{5}}-\frac{4C^{0000,1}_{42,2202}}{\sqrt{15}}-4C^{0000,0}_{60,0000}+\frac{4C^{0000,1}_{60,0000}}{\sqrt{3}},$$

$$C^{60}_{00,20}=\frac{2C^{2000,0}_{00,4000}}{7\sqrt{3}}+\frac{2}{7}C^{2000,1}_{00,4000}-\sqrt{\frac{3}{5}}C^{2202,0}_{20,2202}-\frac{3C^{2202,1}_{20,2202}}{\sqrt{5}}-4\sqrt{\frac{3}{35}}C^{2202,0}_{22,2202}-\frac{12C^{2202,1}_{22,2202}}{\sqrt{35}}+\frac{2C^{0000,0}_{40,2000}}{\sqrt{3}}+2C^{0000,1}_{40,2000}+\frac{4C^{0000,0}_{42,2202}}{\sqrt{15}}+\frac{4C^{0000,1}_{42,2202}}{\sqrt{5}}-\frac{4C^{0000,0}_{60,0000}}{\sqrt{3}}-4C^{0000,1}_{60,0000},$$

$$C^{62}_{00,22}=\frac{4}{21}\sqrt{\frac{5}{3}}C^{2000,0}_{00,4000}-\frac{4}{21}\sqrt{5}C^{2000,1}_{00,4000}-\frac{2}{3}\sqrt{\frac{5}{3}}C^{1111,0}_{00,5111}+\frac{2}{3}\sqrt{5}C^{1111,1}_{00,5111}+\frac{16C^{2202,0}_{20,2202}}{35\sqrt{3}}-\frac{16}{35}C^{2202,1}_{20,2202}+\frac{34C^{1111,0}_{20,3111}}{7\sqrt{15}}-\frac{34C^{1111,1}_{20,3111}}{7\sqrt{5}}-\frac{8C^{2202,0}_{22,2202}}{5\sqrt{21}}+\frac{8C^{2202,1}_{22,2202}}{5\sqrt{7}}+4\sqrt{\frac{6}{35}}C^{1111,0}_{22,3313}-12\sqrt{\frac{2}{35}}C^{1111,1}_{22,3313}-4\sqrt{\frac{3}{5}}C^{1111,0}_{40,1111}+\frac{12C^{1111,1}_{40,1111}}{\sqrt{5}}-\frac{188C^{0000,0}_{40,2000}}{21\sqrt{15}}+\frac{188C^{0000,1}_{40,2000}}{21\sqrt{5}}+\frac{8C^{1111,0}_{42,1111}}{5\sqrt{3}}-\frac{8}{5}C^{1111,1}_{42,1111}-\frac{28C^{0000,0}_{42,2202}}{15\sqrt{3}}+\frac{28}{15}C^{0000,1}_{42,2202}+\frac{16}{3}\sqrt{\frac{5}{3}}C^{0000,0}_{60,0000}-\frac{16}{3}\sqrt{5}C^{0000,1}_{60,0000},$$

$$C^{51}_{11,00}=\frac{12}{7}C^{2000,0}_{00,4000}-\frac{4}{7}\sqrt{3}C^{2000,1}_{00,4000}-\frac{6C^{2202,0}_{20,2202}}{\sqrt{5}}+2\sqrt{\frac{3}{5}}C^{2202,1}_{20,2202}-\frac{24C^{2202,0}_{22,2202}}{\sqrt{35}}+8\sqrt{\frac{3}{35}}C^{2202,1}_{22,2202}-4C^{0000,0}_{40,2000}+\frac{4C^{0000,1}_{40,2000}}{\sqrt{3}}-\frac{8C^{0000,0}_{42,2202}}{\sqrt{5}}+\frac{8C^{0000,1}_{42,2202}}{\sqrt{15}}+24C^{0000,0}_{60,0000}-8\sqrt{3}C^{0000,1}_{60,0000},$$

$$C^{51}_{11,20}=\frac{4}{7}\sqrt{3}C^{2000,0}_{00,4000}-\frac{20}{7}C^{2000,1}_{00,4000}-2\sqrt{\frac{3}{5}}C^{2202,0}_{20,2202}+2\sqrt{5}C^{2202,1}_{20,2202}-8\sqrt{\frac{3}{35}}C^{2202,0}_{22,2202}+8\sqrt{\frac{5}{7}}C^{2202,1}_{22,2202}-\frac{4C^{0000,0}_{40,2000}}{\sqrt{3}}+\frac{20}{3}C^{0000,1}_{40,2000}-\frac{8C^{0000,0}_{42,2202}}{\sqrt{15}}+\frac{8}{3}\sqrt{5}C^{0000,1}_{42,2202}+8\sqrt{3}C^{0000,0}_{60,0000}-40C^{0000,1}_{60,0000},$$

$$C^{51}_{11,22}=\frac{8}{7}\sqrt{\frac{3}{5}}C^{2000,0}_{00,4000}+\frac{8C^{2000,1}_{00,4000}}{7\sqrt{5}}-4\sqrt{\frac{3}{5}}C^{1111,0}_{00,5111}-\frac{4C^{1111,1}_{00,5111}}{\sqrt{5}}-\frac{32}{25}\sqrt{3}C^{2202,0}_{20,2202}-\frac{32}{25}C^{2202,1}_{20,2202}+\frac{12}{5}\sqrt{\frac{3}{5}}C^{1111,0}_{20,3111}+\frac{12C^{1111,1}_{20,3111}}{5\sqrt{5}}-\frac{128}{25}\sqrt{\frac{3}{7}}C^{2202,0}_{22,2202}-\frac{128C^{2202,1}_{22,2202}}{25\sqrt{7}}+\frac{72}{5}\sqrt{\frac{6}{35}}C^{1111,0}_{22,3313}+\frac{72}{5}\sqrt{\frac{2}{35}}C^{1111,1}_{22,3313}-\frac{8}{5}\sqrt{\frac{3}{5}}C^{1111,0}_{40,1111}-\frac{8C^{1111,1}_{40,1111}}{5\sqrt{5}}+\frac{104C^{0000,0}_{40,2000}}{5\sqrt{15}}+\frac{104C^{0000,1}_{40,2000}}{15\sqrt{5}}+\frac{32}{25}\sqrt{3}C^{1111,0}_{42,1111}+\frac{32}{25}C^{1111,1}_{42,1111}+\frac{208C^{0000,0}_{42,2202}}{25\sqrt{3}}+\frac{208}{75}C^{0000,1}_{42,2202}-32\sqrt{\frac{3}{5}}C^{0000,0}_{60,0000}-\frac{32C^{0000,1}_{60,0000}}{\sqrt{5}},$$

$$C^{53}_{11,22}=\frac{16C^{2000,0}_{00,4000}}{9\sqrt{7}}+\frac{16C^{2000,1}_{00,4000}}{9\sqrt{21}}-\frac{8}{9}\sqrt{7}C^{1111,0}_{00,5111}-\frac{8}{9}\sqrt{\frac{7}{3}}C^{1111,1}_{00,5111}+\frac{832C^{2202,0}_{20,2202}}{45\sqrt{35}}+$$

$$\frac{832C^{2202,1}_{20,2202}}{45\sqrt{105}}+\frac{88C^{1111,0}_{20,3111}}{45\sqrt{7}}+\frac{88C^{1111,1}_{20,3111}}{45\sqrt{21}}+\frac{304C^{2202,0}_{22,2202}}{45\sqrt{5}}+\frac{304C^{2202,1}_{22,2202}}{45\sqrt{15}}-\frac{32}{15}\sqrt{2}C^{1111,0}_{22,3313}-\frac{32}{15}\sqrt{\frac{2}{3}}C^{1111,1}_{22,3313}+\frac{16}{5}\sqrt{7}C^{1111,0}_{40,1111}+\frac{16}{5}\sqrt{\frac{7}{3}}C^{1111,1}_{40,1111}-\frac{304C^{0000,0}_{40,2000}}{135\sqrt{7}}-\frac{304C^{0000,1}_{40,2000}}{135\sqrt{21}}-\frac{176}{45}\sqrt{\frac{7}{5}}C^{1111,0}_{42,1111}-\frac{176}{45}\sqrt{\frac{7}{15}}C^{1111,1}_{42,1111}-\frac{344}{135}\sqrt{\frac{7}{5}}C^{0000,0}_{42,2202}-\frac{344}{135}\sqrt{\frac{7}{15}}C^{0000,1}_{42,2202}-\frac{64}{9}\sqrt{7}C^{0000,0}_{60,0000}-\frac{64}{9}\sqrt{\frac{7}{3}}C^{0000,1}_{60,0000},$$

$$C^{40}_{20,00}=2C^{2000,0}_{00,4000}-\frac{2C^{2000,1}_{00,4000}}{\sqrt{3}}-\sqrt{5}C^{2202,0}_{20,2202}+\sqrt{\frac{5}{3}}C^{2202,1}_{20,2202}+4\sqrt{\frac{7}{5}}C^{2202,0}_{22,2202}-4\sqrt{\frac{7}{15}}C^{2202,1}_{22,2202}+\frac{10}{3}C^{0000,0}_{40,2000}-\frac{10C^{0000,1}_{40,2000}}{3\sqrt{3}}-\frac{28C^{0000,0}_{42,2202}}{3\sqrt{5}}+\frac{28C^{0000,1}_{42,2202}}{3\sqrt{15}}-28C^{0000,0}_{60,0000}+\frac{28C^{0000,1}_{60,0000}}{\sqrt{3}},$$

$$C^{40}_{20,20}=\frac{2C^{2000,0}_{00,4000}}{\sqrt{3}}+2C^{2000,1}_{00,4000}-\sqrt{\frac{5}{3}}C^{2202,0}_{20,2202}-\sqrt{5}C^{2202,1}_{20,2202}+4\sqrt{\frac{7}{15}}C^{2202,0}_{22,2202}+4\sqrt{\frac{7}{5}}C^{2202,1}_{22,2202}+\frac{10C^{0000,0}_{40,2000}}{3\sqrt{3}}+\frac{10}{3}C^{0000,1}_{40,2000}-\frac{28C^{0000,0}_{42,2202}}{3\sqrt{15}}-\frac{28C^{0000,1}_{42,2202}}{3\sqrt{5}}-\frac{28C^{0000,0}_{60,0000}}{\sqrt{3}}-28C^{0000,1}_{60,0000},$$

$$C^{42}_{20,22}=\frac{8}{7}\sqrt{\frac{5}{3}}C^{2000,0}_{00,4000}-\frac{8}{7}\sqrt{5}C^{2000,1}_{00,4000}-4\sqrt{\frac{5}{3}}C^{1111,0}_{00,5111}+4\sqrt{5}C^{1111,1}_{00,5111}-\frac{16C^{2202,0}_{20,2202}}{35\sqrt{3}}+\frac{16}{35}C^{2202,1}_{20,2202}+\frac{12}{7}\sqrt{\frac{3}{5}}C^{1111,0}_{20,3111}-\frac{36C^{1111,1}_{20,3111}}{7\sqrt{5}}+\frac{128C^{2202,0}_{22,2202}}{5\sqrt{21}}-\frac{128C^{2202,1}_{22,2202}}{5\sqrt{7}}-24\sqrt{\frac{6}{35}}C^{1111,0}_{22,3313}+72\sqrt{\frac{2}{35}}C^{1111,1}_{22,3313}-\frac{8C^{1111,0}_{40,1111}}{\sqrt{15}}+\frac{8C^{1111,1}_{40,1111}}{\sqrt{5}}-\frac{232C^{0000,0}_{40,2000}}{21\sqrt{15}}+\frac{232C^{0000,1}_{40,2000}}{21\sqrt{5}}+\frac{32C^{1111,0}_{42,1111}}{5\sqrt{3}}-\frac{32}{5}C^{1111,1}_{42,1111}+\frac{208C^{0000,0}_{42,2202}}{15\sqrt{3}}-\frac{208}{15}C^{0000,1}_{42,2202}+32\sqrt{\frac{5}{3}}C^{0000,0}_{60,0000}-32\sqrt{5}C^{0000,1}_{60,0000},$$

$$C^{42}_{22,00}=\frac{8}{7}\sqrt{5}C^{2000,0}_{00,4000}-\frac{8}{7}\sqrt{\frac{5}{3}}C^{2000,1}_{00,4000}+4C^{2202,0}_{20,2202}-\frac{4C^{2202,1}_{20,2202}}{\sqrt{3}}-\frac{8C^{2202,0}_{22,2202}}{\sqrt{7}}+\frac{8C^{2202,1}_{22,2202}}{\sqrt{21}}-\frac{8}{3}\sqrt{5}C^{0000,0}_{40,2000}+\frac{8}{3}\sqrt{\frac{5}{3}}C^{0000,1}_{40,2000}+\frac{8}{3}C^{0000,0}_{42,2202}-\frac{8C^{0000,1}_{42,2202}}{3\sqrt{3}}-16\sqrt{5}C^{0000,0}_{60,0000}+16\sqrt{\frac{5}{3}}C^{0000,1}_{60,0000},$$

$$C^{42}_{22,20}=\frac{8}{7}\sqrt{\frac{5}{3}}C^{2000,0}_{00,4000}+\frac{8}{7}\sqrt{5}C^{2000,1}_{00,4000}+\frac{4C^{2202,0}_{20,2202}}{\sqrt{3}}+4C^{2202,1}_{20,2202}-\frac{8C^{2202,0}_{22,2202}}{\sqrt{21}}-\frac{8C^{2202,1}_{22,2202}}{\sqrt{7}}-\frac{8}{3}\sqrt{\frac{5}{3}}C^{0000,0}_{40,2000}-\frac{8}{3}\sqrt{5}C^{0000,1}_{40,2000}+\frac{8C^{0000,0}_{42,2202}}{3\sqrt{3}}+\frac{8}{3}C^{0000,1}_{42,2202}-16\sqrt{\frac{5}{3}}C^{0000,0}_{60,0000}-16\sqrt{5}C^{0000,1}_{60,0000},$$

$$C^{40}_{22,22}=\frac{4C^{2000,0}_{00,4000}}{\sqrt{15}}-\frac{4C^{2000,1}_{00,4000}}{\sqrt{5}}-\frac{14C^{1111,0}_{00,5111}}{\sqrt{15}}+\frac{14C^{1111,1}_{00,5111}}{\sqrt{5}}-\frac{32C^{2202,0}_{20,2202}}{25\sqrt{3}}+\frac{32}{25}C^{2202,1}_{20,2202}-\frac{6}{5}\sqrt{\frac{3}{5}}C^{1111,0}_{20,3111}+\frac{18C^{1111,1}_{20,3111}}{5\sqrt{5}}-\frac{104}{25}\sqrt{\frac{7}{3}}C^{2202,0}_{22,2202}+\frac{104}{25}\sqrt{7}C^{2202,1}_{22,2202}+\frac{12}{5}\sqrt{\frac{42}{5}}C^{1111,0}_{22,3313}-\frac{36}{5}\sqrt{\frac{14}{5}}C^{1111,1}_{22,3313}+\frac{68C^{1111,0}_{40,1111}}{5\sqrt{15}}-\frac{68C^{1111,1}_{40,1111}}{5\sqrt{5}}+\frac{76C^{0000,0}_{40,2000}}{15\sqrt{15}}-\frac{76C^{0000,1}_{40,2000}}{15\sqrt{5}}-\frac{392C^{1111,0}_{42,1111}}{25\sqrt{3}}+\frac{392}{25}C^{1111,1}_{42,1111}-\frac{868C^{0000,0}_{42,2202}}{75\sqrt{3}}+\frac{868}{75}C^{0000,1}_{42,2202}+\frac{112C^{0000,0}_{60,0000}}{\sqrt{15}}-\frac{112C^{0000,1}_{60,0000}}{\sqrt{5}},$$

$$C^{42}_{22,22}=\frac{16}{7}\sqrt{\frac{5}{21}}C^{2000,0}_{00,4000}-\frac{16}{7}\sqrt{\frac{5}{7}}C^{2000,1}_{00,4000}-8\sqrt{\frac{5}{21}}C^{1111,0}_{00,5111}+8\sqrt{\frac{5}{7}}C^{1111,1}_{00,5111}-\frac{16C^{2202,0}_{20,2202}}{\sqrt{21}}+\frac{16C^{2202,1}_{20,2202}}{\sqrt{7}}+\frac{32C^{2202,0}_{22,2202}}{7\sqrt{3}}-\frac{32}{7}C^{2202,1}_{22,2202}+16\sqrt{\frac{5}{21}}C^{1111,0}_{40,1111}-16\sqrt{\frac{5}{7}}C^{1111,1}_{40,1111}-\frac{16}{3}\sqrt{\frac{5}{21}}C^{0000,0}_{40,2000}+\frac{16}{3}\sqrt{\frac{5}{7}}C^{0000,1}_{40,2000}+\frac{32C^{1111,0}_{42,1111}}{\sqrt{21}}-\frac{32C^{1111,1}_{42,1111}}{\sqrt{7}}+\frac{16C^{0000,0}_{42,2202}}{3\sqrt{21}}-\frac{16C^{0000,1}_{42,2202}}{3\sqrt{7}}+64\sqrt{\frac{5}{21}}C^{0000,0}_{60,0000}-64\sqrt{\frac{5}{7}}C^{0000,1}_{60,0000},$$

$$C^{44}_{22,22}=\frac{16C^{2000,0}_{00,4000}}{21\sqrt{3}}-\frac{16}{21}C^{2000,1}_{00,4000}-\frac{8C^{1111,0}_{00,5111}}{3\sqrt{3}}+\frac{8}{3}C^{1111,1}_{00,5111}+\frac{256C^{2202,0}_{20,2202}}{15\sqrt{15}}-\frac{256C^{2202,1}_{20,2202}}{15\sqrt{5}}-\frac{56C^{1111,0}_{20,3111}}{15\sqrt{3}}+\frac{56}{15}C^{1111,1}_{20,3111}-\frac{176C^{2202,0}_{22,2202}}{15\sqrt{105}}+\frac{176C^{2202,1}_{22,2202}}{15\sqrt{35}}+\frac{4}{5}\sqrt{\frac{14}{3}}C^{1111,0}_{22,3313}-\frac{4}{5}\sqrt{14}C^{1111,1}_{22,3313}-\frac{16}{5}\sqrt{3}C^{1111,0}_{40,1111}+\frac{48}{5}C^{1111,1}_{40,1111}+\frac{592C^{0000,0}_{40,2000}}{45\sqrt{3}}-\frac{592}{45}C^{0000,1}_{40,2000}-\frac{64C^{1111,0}_{42,1111}}{15\sqrt{15}}+\frac{64C^{1111,1}_{42,1111}}{15\sqrt{5}}-\frac{256C^{0000,0}_{42,2202}}{45\sqrt{15}}+\frac{256C^{0000,1}_{42,2202}}{45\sqrt{5}}+\frac{64C^{0000,0}_{60,0000}}{3\sqrt{3}}-\frac{64}{3}C^{0000,1}_{60,0000},$$

$$C^{31}_{31,00} = \tfrac{12}{5}C^{2000,0}_{00,4000} - \tfrac{4}{5}\sqrt{3}C^{2000,1}_{00,4000} + \frac{6C^{2202,0}_{20,2202}}{5\sqrt{5}} - \tfrac{2}{5}\sqrt{\tfrac{3}{5}}C^{2202,1}_{20,2202} + \tfrac{24}{5}\sqrt{\tfrac{7}{5}}C^{2202,0}_{22,2202} - \tfrac{8}{5}\sqrt{\tfrac{21}{5}}C^{2202,1}_{22,2202} + \tfrac{4}{5}C^{0000,0}_{40,2000} - \frac{4C^{0000,1}_{40,2000}}{5\sqrt{3}} + \frac{56C^{0000,0}_{42,2202}}{5\sqrt{5}} - \frac{56C^{0000,1}_{42,2202}}{5\sqrt{15}} + \tfrac{168}{5}C^{0000,0}_{60,0000} - \tfrac{56}{5}\sqrt{3}C^{0000,1}_{60,0000},$$

$$C^{31}_{31,20} = \tfrac{4}{5}\sqrt{3}C^{2000,0}_{00,4000} - 4C^{2000,1}_{00,4000} + \tfrac{2}{5}\sqrt{\tfrac{3}{5}}C^{2202,0}_{20,2202} - \frac{2C^{2202,1}_{20,2202}}{\sqrt{5}} + \tfrac{8}{5}\sqrt{\tfrac{21}{5}}C^{2202,0}_{22,2202} - 8\sqrt{\tfrac{7}{5}}C^{2202,1}_{22,2202} + \frac{4C^{0000,0}_{40,2000}}{5\sqrt{3}} - \tfrac{4}{3}C^{0000,1}_{40,2000} + \frac{56C^{0000,0}_{42,2202}}{5\sqrt{15}} - \frac{56C^{0000,1}_{42,2202}}{3\sqrt{5}} + \tfrac{56}{5}\sqrt{3}C^{0000,0}_{60,0000} - 56C^{0000,1}_{60,0000},$$

$$C^{31}_{31,22} = \tfrac{8}{5}\sqrt{\tfrac{3}{5}}C^{2000,0}_{00,4000} + \frac{8C^{2000,1}_{00,4000}}{5\sqrt{5}} - \tfrac{28}{5}\sqrt{\tfrac{3}{5}}C^{1111,0}_{00,5111} - \frac{28C^{1111,1}_{00,5111}}{5\sqrt{5}} - \tfrac{256}{125}\sqrt{3}C^{2202,0}_{20,2202} - \tfrac{256}{125}C^{2202,1}_{20,2202} + \tfrac{36}{25}\sqrt{\tfrac{3}{5}}C^{1111,0}_{20,3111} + \frac{36C^{1111,1}_{20,3111}}{25\sqrt{5}} + \tfrac{128}{125}\sqrt{21}C^{2202,0}_{22,2202} + \tfrac{128}{125}\sqrt{7}C^{2202,1}_{22,2202} - \tfrac{72}{25}\sqrt{\tfrac{42}{5}}C^{1111,0}_{22,3313} - \tfrac{72}{25}\sqrt{\tfrac{14}{5}}C^{1111,1}_{22,3313} - \tfrac{184}{25}\sqrt{\tfrac{3}{5}}C^{1111,0}_{40,1111} - \frac{184C^{1111,1}_{40,1111}}{25\sqrt{5}} + \frac{472C^{0000,0}_{40,2000}}{25\sqrt{15}} + \frac{472C^{0000,1}_{40,2000}}{75\sqrt{5}} - \tfrac{224}{125}\sqrt{3}C^{1111,0}_{42,1111} - \tfrac{224}{125}C^{1111,1}_{42,1111} - \frac{1456C^{0000,0}_{42,2202}}{125\sqrt{3}} - \tfrac{1456}{375}C^{0000,1}_{42,2202} - \tfrac{224}{5}\sqrt{\tfrac{3}{5}}C^{0000,0}_{60,0000} - \frac{224C^{0000,1}_{60,0000}}{5\sqrt{5}},$$

$$C^{33}_{31,22} = \frac{16C^{2000,0}_{00,4000}}{5\sqrt{7}} + \frac{16C^{2000,1}_{00,4000}}{5\sqrt{21}} - \tfrac{8}{5}\sqrt{7}C^{1111,0}_{00,5111} - \tfrac{8}{5}\sqrt{\tfrac{7}{3}}C^{1111,1}_{00,5111} + \frac{608C^{2202,0}_{20,2202}}{25\sqrt{35}} + \frac{608C^{2202,1}_{20,2202}}{25\sqrt{105}} - \frac{248C^{1111,0}_{20,3111}}{25\sqrt{7}} - \frac{248C^{1111,1}_{20,3111}}{25\sqrt{21}} - \frac{304C^{2202,0}_{22,2202}}{25\sqrt{5}} - \frac{304C^{2202,1}_{22,2202}}{25\sqrt{15}} + \tfrac{96}{25}\sqrt{2}C^{1111,0}_{22,3313} + \tfrac{32}{25}\sqrt{6}C^{1111,1}_{22,3313} + \tfrac{16}{25}\sqrt{7}C^{1111,0}_{40,1111} + \tfrac{16}{25}\sqrt{\tfrac{7}{3}}C^{1111,1}_{40,1111} - \frac{2096C^{0000,0}_{40,2000}}{75\sqrt{7}} - \frac{2096C^{0000,1}_{40,2000}}{75\sqrt{21}} + \tfrac{176}{25}\sqrt{\tfrac{7}{5}}C^{1111,0}_{42,1111} + \tfrac{176}{25}\sqrt{\tfrac{7}{15}}C^{1111,1}_{42,1111} + \tfrac{344}{75}\sqrt{\tfrac{7}{5}}C^{0000,0}_{42,2202} + \tfrac{344}{75}\sqrt{\tfrac{7}{15}}C^{0000,1}_{42,2202} - \tfrac{64}{5}\sqrt{7}C^{0000,0}_{60,0000} - \tfrac{64}{5}\sqrt{\tfrac{7}{3}}C^{0000,1}_{60,0000},$$

$$C^{33}_{33,00} = \frac{8C^{2000,0}_{00,4000}}{3\sqrt{21}} - \frac{8C^{2000,1}_{00,4000}}{9\sqrt{7}} + 4\sqrt{\tfrac{7}{15}}C^{2202,0}_{20,2202} - \tfrac{4}{3}\sqrt{\tfrac{7}{5}}C^{2202,1}_{20,2202} - \frac{8C^{2202,0}_{22,2202}}{\sqrt{15}} + \frac{8C^{2202,1}_{22,2202}}{3\sqrt{5}} + \tfrac{8}{3}\sqrt{\tfrac{7}{3}}C^{0000,0}_{40,2000} - \tfrac{8}{9}\sqrt{7}C^{0000,1}_{40,2000} - \tfrac{8}{3}\sqrt{\tfrac{7}{15}}C^{0000,0}_{42,2202} + \tfrac{8}{9}\sqrt{\tfrac{7}{5}}C^{0000,1}_{42,2202} + \tfrac{16}{3}\sqrt{\tfrac{7}{3}}C^{0000,0}_{60,0000} - \tfrac{16}{9}\sqrt{7}C^{0000,1}_{60,0000},$$

$$C^{33}_{33,20} = \frac{8C^{2000,0}_{00,4000}}{9\sqrt{7}} - \frac{40C^{2000,1}_{00,4000}}{9\sqrt{21}} + \tfrac{4}{3}\sqrt{\tfrac{7}{5}}C^{2202,0}_{20,2202} - \tfrac{4}{3}\sqrt{\tfrac{35}{3}}C^{2202,1}_{20,2202} - \frac{8C^{2202,0}_{22,2202}}{3\sqrt{5}} + \tfrac{8}{3}\sqrt{\tfrac{5}{3}}C^{2202,1}_{22,2202} + \tfrac{8}{9}\sqrt{7}C^{0000,0}_{40,2000} - \tfrac{40}{9}\sqrt{\tfrac{7}{3}}C^{0000,1}_{40,2000} - \tfrac{8}{9}\sqrt{\tfrac{7}{5}}C^{0000,0}_{42,2202} + \tfrac{8}{9}\sqrt{\tfrac{35}{3}}C^{0000,1}_{42,2202} + \tfrac{16}{9}\sqrt{7}C^{0000,0}_{60,0000} - \tfrac{80}{9}\sqrt{\tfrac{7}{3}}C^{0000,1}_{60,0000},$$

$$C^{33}_{33,22} = \tfrac{16}{9}\sqrt{\tfrac{2}{105}}C^{2000,0}_{00,4000} + \tfrac{16}{27}\sqrt{\tfrac{2}{35}}C^{2000,1}_{00,4000} - \tfrac{8}{9}\sqrt{\tfrac{14}{15}}C^{1111,0}_{00,5111} - \tfrac{8}{27}\sqrt{\tfrac{14}{5}}C^{1111,1}_{00,5111} - \tfrac{32}{75}\sqrt{\tfrac{14}{3}}C^{2202,0}_{20,2202} - \tfrac{32}{225}\sqrt{14}C^{2202,1}_{20,2202} - \tfrac{8}{15}\sqrt{\tfrac{14}{15}}C^{1111,0}_{20,3111} - \tfrac{8}{45}\sqrt{\tfrac{14}{5}}C^{1111,1}_{20,3111} + \tfrac{112}{75}\sqrt{\tfrac{2}{3}}C^{2202,0}_{22,2202} + \tfrac{112}{225}\sqrt{2}C^{2202,1}_{22,2202} + \frac{8C^{1111,0}_{22,3313}}{5\sqrt{15}} + \frac{8C^{1111,1}_{22,3313}}{15\sqrt{5}} - \tfrac{16}{5}\sqrt{\tfrac{14}{15}}C^{1111,0}_{40,1111} - \tfrac{16}{15}\sqrt{\tfrac{14}{5}}C^{1111,1}_{40,1111} - \tfrac{16}{45}\sqrt{\tfrac{14}{15}}C^{0000,0}_{40,2000} - \tfrac{16}{135}\sqrt{\tfrac{14}{5}}C^{0000,1}_{40,2000} - \tfrac{128}{75}\sqrt{\tfrac{14}{3}}C^{1111,0}_{42,1111} - \tfrac{128}{225}\sqrt{14}C^{1111,1}_{42,1111} - \tfrac{32}{225}\sqrt{\tfrac{14}{3}}C^{0000,0}_{42,2202} - \tfrac{32}{675}\sqrt{14}C^{0000,1}_{42,2202} - \tfrac{64}{9}\sqrt{\tfrac{14}{15}}C^{0000,0}_{60,0000} - \tfrac{64}{27}\sqrt{\tfrac{14}{5}}C^{0000,1}_{60,0000}.$$
