# Supplementary material for: Effective pseudopotential for energy density functionals with higher order derivatives
Source: arXiv:1103.0682 ancillary file (2011-04-17)
Supplement: Supplementary file 5 [file README.tex.pdf]

**Contents Description of the Supplemental Material for the paper**  
*Effective pseudopotential for energy density functionals with higher order derivatives*

The Supplemental Material is given in three different formats (T<sub>E</sub>X, Mathematica<sup>®</sup>, and Fortran) displaying the same results. In the filenames is included the format of the content of the file (F for Fortran, M for Mathematica<sup>®</sup>, T for T<sub>E</sub>X) and the section of the paper where the results included in the file are referred to: for instance, the results contained in the file **Suppl\_F\_Section\_IIIA.txt** are explicitly cited in the Section IIIA of the paper and are displayed in Fortran form.

**Some remarks about the extensions of the files included in the Supplemental Material**

- T<sub>E</sub>X files: all the T<sub>E</sub>X files are named as **Suppl\_T\_filename.tex** and they can be directly processed by T<sub>E</sub>X.
- Mathematica<sup>®</sup> files: all the Mathematica<sup>®</sup> files are named **Suppl\_M\_filename.txt** and they can be processed after changing the extension of the files into **.nb**, which is the correct extension for the files to be processed in the Mathematica<sup>®</sup>.
- Fortran files: all the Fortran files are named **Suppl\_F\_filename.txt** and they can be compiled after changing the extension of the files into **.f90**, which is the correct extension for the files to be processed in Fortran. The matrices of the coefficients are given explicitly in Subroutines, which can be included in a main program. They display the numerical coefficients of the formulas in which the EDF coupling constants are expressed through the pseudopotential parameters or *vice versa*. In the list of contents below, we will make explicit the structure of the matrices using the standard notation of the systems of linear equation,  $\mathbf{b} = A\mathbf{x}$ , denoting with  $\mathbf{x}$  the column vector multiplying the coefficients matrix A and with  $\mathbf{b}$  the resulting column vector.

**Complete list of the files included in the Supplemental Material**

- T<sub>E</sub>X files:
  1. **Suppl\_T\_Section\_III.tex**
  2. **Suppl\_T\_Section\_IIIA.tex**
  3. **Suppl\_T\_Section\_IIIB.tex**
  4. **Suppl\_T\_Section\_IV.tex**
- Mathematica<sup>®</sup> files:
  1. **Suppl\_M\_Section\_III.txt**

2. Suppl\_M.Section.IIIA.txt
3. Suppl\_M.Section.IIIB.txt
4. Suppl\_M.Section.IV.txt

- Fortran files:

1. Suppl\_F.Section.III.txt:

$A \equiv MatrixFourth(90, 15),$

$\mathbf{x} \equiv (C_{00,00}^{40}, C_{00,20}^{40}, C_{00,22}^{42}, C_{11,00}^{31}, C_{11,11}^{31}, C_{11,20}^{31}, C_{11,22}^{31}, C_{11,22}^{33}, C_{20,00}^{20},$   
 $C_{20,20}^{20}, C_{20,22}^{22}, C_{22,00}^{22}, C_{22,11}^{22}, C_{22,20}^{22}, C_{22,22}^{22}) ,$

$\mathbf{b} \equiv (C_{00,2000}^{2000,0}, C_{00,2000}^{2000,1}, C_{00,2011}^{2011,0}, C_{00,2011}^{2011,1}, C_{00,2202}^{2202,0}, C_{00,2202}^{2202,1}, C_{00,2211}^{2011,0}, C_{00,2211}^{2011,1},$   
 $C_{00,2211}^{2211,0}, C_{00,2211}^{2211,1}, C_{00,2212}^{2212,0}, C_{00,2212}^{2212,1}, C_{00,2213}^{2213,0}, C_{00,2213}^{2213,1}, C_{00,3101}^{1101,0}, C_{00,3101}^{1101,1}, C_{00,3110}^{1110,0},$   
 $C_{00,3110}^{1110,1}, C_{00,3111}^{1111,0}, C_{00,3111}^{1111,1}, C_{00,3112}^{1112,0}, C_{00,3112}^{1112,1}, C_{00,3312}^{1112,0}, C_{00,3312}^{1112,1}, C_{00,4000}^{0000,0}, C_{00,4000}^{0000,1},$   
 $C_{00,4011}^{0011,0}, C_{00,4011}^{0011,1}, C_{00,4211}^{0011,0}, C_{00,4211}^{0011,1}, C_{11,0011}^{3101,0}, C_{11,0011}^{3101,1}, C_{11,1111}^{2000,0}, C_{11,1111}^{2000,1}, C_{11,1111}^{2202,0},$   
 $C_{11,1111}^{2202,1}, C_{11,1112}^{2202,0}, C_{11,1112}^{2202,1}, C_{11,2011}^{1101,0}, C_{11,2011}^{1101,1}, C_{11,2211}^{1101,0}, C_{11,2211}^{1101,1}, C_{11,2212}^{1101,0}, C_{11,2212}^{1101,1},$   
 $C_{0000,0}^{1111,0}, C_{0000,0}^{1111,1}, C_{1101,0}^{1101,0}, C_{1101,0}^{1101,1}, C_{1110,0}^{1110,0}, C_{1110,0}^{1110,1}, C_{1111,0}^{1111,0}, C_{1111,0}^{1111,1}, C_{1112,0}^{1112,0},$   
 $C_{1112,0}^{1112,1}, C_{0000,0}^{0000,0}, C_{0000,0}^{0000,1}, C_{0011,0}^{0011,0}, C_{0011,0}^{0011,1}, C_{0011,0}^{0011,1}, C_{0011,0}^{0011,1}, C_{1101,0}^{1101,0}, C_{1101,0}^{1101,1},$   
 $C_{1111,0}^{1111,0}, C_{1111,0}^{1111,1}, C_{1110,0}^{1110,0}, C_{1110,0}^{1110,1}, C_{1111,0}^{1111,0}, C_{1111,0}^{1111,1}, C_{1112,0}^{1112,0}, C_{1112,0}^{1112,1}, C_{0011,0}^{0011,0},$   
 $C_{0011,0}^{0011,1}, C_{0000,0}^{0000,0}, C_{0000,0}^{0000,1}, C_{0011,0}^{0011,0}, C_{0011,0}^{0011,1}, C_{0011,0}^{0011,1}, C_{0011,0}^{0011,1}, C_{0011,0}^{0011,1}, C_{0011,0}^{0011,1},$   
 $C_{1101,0}^{1101,0}, C_{1101,0}^{1101,1}, C_{0000,0}^{0000,0}, C_{0000,0}^{0000,1}, C_{0000,0}^{0000,1}, C_{0000,0}^{0000,1}, C_{40,0011}^{0011,0}, C_{40,0011}^{0011,1}, C_{42,0011}^{0011,0},$   
 $C_{42,0011}^{0011,1}) ;$

$A \equiv MatrixSixth(258, 26),$

$\mathbf{x} \equiv (C_{00,00}^{60}, C_{00,20}^{60}, C_{00,22}^{62}, C_{11,00}^{51}, C_{11,11}^{51}, C_{11,20}^{51}, C_{11,22}^{51}, C_{11,22}^{53}, C_{20,00}^{40}, C_{20,20}^{40},$   
 $C_{20,22}^{42}, C_{22,00}^{42}, C_{22,11}^{42}, C_{22,20}^{42}, C_{22,22}^{42}, C_{22,22}^{44}, C_{31,00}^{31}, C_{31,11}^{31}, C_{31,20}^{31},$   
 $C_{31,22}^{31}, C_{31,22}^{33}, C_{33,00}^{33}, C_{33,11}^{33}, C_{33,20}^{33}, C_{33,22}^{33}) ,$

$\mathbf{b} \equiv (C_{00,3101}^{3101,0}, C_{00,3101}^{3101,1}, C_{00,3110}^{3110,0}, C_{00,3110}^{3110,1}, C_{00,3111}^{3111,0}, C_{00,3111}^{3111,1}, C_{00,3112}^{3112,0},$   
 $C_{00,3112}^{3112,1}, C_{00,3303}^{3303,0}, C_{00,3303}^{3303,1}, C_{00,3312}^{3312,0}, C_{00,3312}^{3312,1}, C_{00,3312}^{3312,0}, C_{00,3312}^{3312,1},$   
 $C_{00,3313}^{3313,0}, C_{00,3313}^{3313,1}, C_{00,3314}^{3314,0}, C_{00,3314}^{3314,1}, C_{00,4000}^{2000,0}, C_{00,4000}^{2000,1}, C_{00,4011}^{2011,0},$   
 $C_{00,4011}^{2011,1}, C_{00,4011}^{2211,0}, C_{00,4011}^{2211,1}, C_{00,4202}^{2202,0}, C_{00,4202}^{2202,1}, C_{00,4211}^{2011,0}, C_{00,4211}^{2011,1},$   
 $C_{00,4211}^{2211,0}, C_{00,4211}^{2211,1}, C_{00,4212}^{2212,0}, C_{00,4212}^{2212,1}, C_{00,4213}^{2213,0}, C_{00,4213}^{2213,1}, C_{00,4413}^{2213,0},$   
 $C_{00,4413}^{2213,1}, C_{00,5101}^{1101,0}, C_{00,5101}^{1101,1}, C_{00,5110}^{1110,0}, C_{00,5110}^{1110,1}, C_{00,5111}^{1111,0}, C_{00,5111}^{1111,1},$   
 $C_{00,5112}^{1112,0}, C_{00,5112}^{1112,1}, C_{00,5312}^{1112,0}, C_{00,5312}^{1112,1}, C_{00,6000}^{0000,0}, C_{00,6000}^{0000,1}, C_{00,6011}^{0011,0},$   
 $C_{00,6011}^{0011,1}, C_{00,6211}^{0011,0}, C_{00,6211}^{0011,1}, C_{11,0011}^{5101,0}, C_{11,0011}^{5101,1}, C_{11,1111}^{4000,0}, C_{11,1111}^{4000,1},$   
 $C_{4202,0}^{4202,0}, C_{4202,0}^{4202,1}, C_{3101,0}^{3101,0}, C_{3101,0}^{3101,1}, C_{11,1111}^{3101,0}, C_{11,1111}^{3101,1}, C_{11,2211}^{3101,0},$   
 $C_{11,2211}^{3101,1}, C_{11,2212}^{3101,0}, C_{11,2212}^{3101,1}, C_{11,2212}^{3303,0}, C_{11,2212}^{3303,1}, C_{11,2213}^{3303,0}, C_{11,2213}^{3303,1},$   
 $C_{2000,0}^{2000,0}, C_{2000,0}^{2000,1}, C_{2202,0}^{2202,0}, C_{2202,0}^{2202,1}, C_{2202,0}^{2202,0}, C_{2202,0}^{2202,1}, C_{11,3111}^{11,3111}, C_{11,3111}^{11,3112},$   
 $C_{2202,1}^{2202,0}, C_{2202,1}^{2202,1}, C_{1101,0}^{1101,0}, C_{1101,0}^{1101,1}, C_{1101,0}^{1101,0}, C_{1101,0}^{1101,1}, C_{11,4211}^{11,4211},$   
 $C_{1101,0}^{1101,0}, C_{1101,0}^{1101,1}, C_{0000,0}^{0000,0}, C_{0000,0}^{0000,1}, C_{2000,0}^{2000,0}, C_{2000,0}^{2000,1}, C_{2011,0}^{2011,0},$   
 $C_{11,4212}^{11,4212}, C_{11,4212}^{11,5111}, C_{11,5111}^{11,5111}, C_{20,2000}^{20,2000}, C_{20,2000}^{20,2011}, C_{20,2011}^{20,2011}) ,$



$A \equiv \text{MatrixSixthInvT0}(26, 26),$

$$\begin{aligned} \mathbf{x} \equiv & (C_{00,3303}^{3303,0}, C_{00,3313}^{3313,0}, C_{00,6211}^{0011,0}, C_{11,2212}^{3101,0}, C_{20,2011}^{2011,0}, C_{20,2202}^{2202,0}, C_{20,2211}^{2011,0}, C_{22,3112}^{1110,0}, \\ & C_{22,3112}^{1111,0}, C_{22,3303}^{1101,0}, C_{22,3313}^{1111,0}, C_{22,4212}^{0011,0}, C_{22,4212}^{2202,0}, C_{31,1112}^{1101,0}, C_{33,2213}^{1101,0}, C_{40,1101}^{1112,0}, C_{40,1112}^{1112,0}, \\ & C_{40,2211}^{0011,0}, C_{42,1101}^{1101,0}, C_{42,1111}^{1111,0}, C_{42,1112}^{1110,0}, C_{42,2212}^{0011,0}, C_{44,2213}^{0011,0}, C_{51,0011}^{1101,0}, C_{60,0000}^{0000,0}, \\ & C_{60,0011}^{0011,0}, C_{62,0011}^{0011,0}), \\ \mathbf{b} \equiv & (C_{00,00}^{60}, C_{00,20}^{60}, C_{00,22}^{62}, C_{11,00}^{51}, C_{11,11}^{51}, C_{11,20}^{51}, C_{11,22}^{51}, C_{11,22}^{53}, C_{20,00}^{40}, \\ & C_{20,20}^{40}, C_{20,22}^{42}, C_{22,00}^{42}, C_{22,11}^{42}, C_{22,20}^{40}, C_{22,22}^{42}, C_{22,22}^{44}, C_{22,22}^{44}, C_{31,00}^{31}, \\ & C_{31,11}^{31}, C_{31,20}^{31}, C_{31,22}^{31}, C_{31,22}^{33}, C_{33,00}^{33}, C_{33,11}^{33}, C_{33,20}^{33}, C_{33,22}^{33}); \end{aligned}$$

$A \equiv \text{MatrixSixthInvT1}(26, 26),$

$$\begin{aligned} \mathbf{x} \equiv & (C_{00,3303}^{3303,1}, C_{00,3313}^{3313,1}, C_{00,6211}^{0011,1}, C_{11,2212}^{3101,1}, C_{20,2011}^{2011,1}, C_{20,2202}^{2202,1}, C_{20,2211}^{2011,1}, C_{22,3112}^{1110,1}, \\ & C_{22,3112}^{1111,1}, C_{22,3303}^{1101,1}, C_{22,3313}^{1111,1}, C_{22,4212}^{0011,1}, C_{22,4212}^{2202,1}, C_{31,1112}^{1101,1}, C_{33,2213}^{1101,1}, C_{40,1101}^{1112,1}, C_{40,1112}^{1112,1}, \\ & C_{40,2211}^{0011,1}, C_{42,1101}^{1101,1}, C_{42,1111}^{1111,1}, C_{42,1112}^{1110,1}, C_{42,2212}^{0011,1}, C_{44,2213}^{0011,1}, C_{51,0011}^{1101,1}, C_{60,0000}^{0000,1}, \\ & C_{60,0011}^{0011,1}, C_{62,0011}^{0011,1}), \\ \mathbf{b} \equiv & (C_{00,00}^{60}, C_{00,20}^{60}, C_{00,22}^{62}, C_{11,00}^{51}, C_{11,11}^{51}, C_{11,20}^{51}, C_{11,22}^{51}, C_{11,22}^{53}, C_{20,00}^{40}, \\ & C_{20,20}^{40}, C_{20,22}^{42}, C_{22,00}^{42}, C_{22,11}^{42}, C_{22,20}^{40}, C_{22,22}^{42}, C_{22,22}^{44}, C_{22,22}^{44}, C_{31,00}^{31}, \\ & C_{31,11}^{31}, C_{31,20}^{31}, C_{31,22}^{31}, C_{31,22}^{33}, C_{33,00}^{33}, C_{33,11}^{33}, C_{33,20}^{33}, C_{33,22}^{33}). \end{aligned}$$

### 3. Suppl\_F\_Section IIIB.txt:

$A \equiv \text{Matrix4thCouplConst}(15, 15),$

$$\begin{aligned} \mathbf{x} \equiv & (C_{00,4211}^{0011,0}, C_{20,1101}^{1101,0}, C_{20,2211}^{0011,0}, C_{22,1101}^{1111,0}, C_{22,1112}^{1112,0}, C_{22,1112}^{1112,0}, C_{22,2213}^{0011,0}, C_{40,0000}^{0000,0}, \\ & C_{40,0011}^{0011,0}, C_{42,0011}^{0011,0}, C_{00,2202}^{2202,0}, C_{00,2212}^{2212,0}, C_{20,2011}^{0011,0}, C_{11,2212}^{1101,0}, C_{31,0011}^{1101,0}), \\ \mathbf{b} \equiv & (C_{00,2202}^{2202,1}, C_{00,2212}^{2212,1}, C_{00,4211}^{0011,1}, C_{40,0000}^{0000,1}, C_{40,0011}^{0011,1}, C_{42,0011}^{0011,1}, C_{20,1101}^{1101,1}, C_{22,1101}^{1101,1}, \\ & C_{20,2011}^{0011,1}, C_{20,2211}^{0011,1}, C_{22,1112}^{1111,1}, C_{22,1112}^{1112,1}, C_{22,2213}^{0011,1}, C_{31,0011}^{1101,1}, C_{11,2212}^{1101,1}); \end{aligned}$$

$A \equiv \text{Matrix6thCouplConst}(26, 26),$

$$\begin{aligned} \mathbf{x} \equiv & (C_{00,3303}^{3303,0}, C_{00,3313}^{3313,0}, C_{00,6211}^{0011,0}, C_{11,2212}^{3101,0}, C_{20,2011}^{2011,0}, C_{20,2202}^{2202,0}, C_{20,2211}^{2011,0}, C_{22,3112}^{1110,0}, \\ & C_{22,3112}^{1111,0}, C_{22,3303}^{1101,0}, C_{22,3313}^{1111,0}, C_{22,4212}^{0011,0}, C_{40,1101}^{1112,0}, C_{40,1112}^{1112,0}, C_{40,2211}^{0011,0}, C_{31,1112}^{2202,0}, \\ & C_{33,2213}^{1101,0}, C_{42,1101}^{1111,0}, C_{42,1111}^{1111,0}, C_{42,1112}^{1110,0}, C_{42,2212}^{0011,0}, C_{44,2213}^{0011,0}, C_{51,0011}^{1101,0}, C_{60,0000}^{0000,0}, \\ & C_{60,0011}^{0011,0}, C_{62,0011}^{0011,0}), \\ \mathbf{b} \equiv & (C_{60,0000}^{0000,1}, C_{60,0011}^{0011,1}, C_{62,0011}^{0011,1}, C_{00,3303}^{3303,1}, C_{00,6211}^{0011,1}, C_{00,3313}^{3313,1}, C_{20,2202}^{2202,1}, C_{42,1112}^{1110,1}, \\ & C_{22,3112}^{1110,1}, C_{42,1111}^{1111,1}, C_{22,3112}^{1111,1}, C_{22,3313}^{1111,1}, C_{40,1112}^{1112,1}, C_{40,1101}^{1101,1}, C_{42,1101}^{1101,1}, C_{22,3303}^{1101,1}, \\ & C_{1101,1}^{1101,1}, C_{2202,1}^{2202,1}, C_{1101,1}^{1101,1}, C_{3101,1}^{3101,1}, C_{0011,1}^{0011,1}, C_{0011,1}^{0011,1}, C_{0011,1}^{0011,1}, C_{2011,1}^{2011,1}, \\ & C_{2011,1}^{2011,1}, C_{22,4212}^{22,4212}). \end{aligned}$$

### 4. Suppl\_F\_Section IV.txt:

$A \equiv \text{Matrix4thSpherical}(14, 13),$

$$\begin{aligned} \mathbf{x} \equiv & (C_{00,00}^{40}, C_{00,20}^{40}, C_{00,22}^{42}, C_{11,00}^{31}, C_{11,20}^{31}, C_{11,22}^{31}, C_{11,22}^{33}, C_{20,00}^{20}, C_{20,20}^{20}, \\ & C_{20,22}^{22}, C_{22,00}^{22}, C_{22,20}^{22}, C_{22,22}^{22}), \end{aligned}$$

$$\mathbf{b} \equiv (C_{40,0000}^{0000,0}, C_{40,0000}^{0000,1}, C_{20,2000}^{0000,0}, C_{20,2000}^{0000,1}, C_{22,2202}^{0000,0}, C_{22,2202}^{0000,1}, C_{00,2202}^{2202,0}, C_{00,2202}^{2202,1}, C_{20,1111}^{1111,0}, C_{20,1111}^{1111,1}, C_{22,1111}^{1111,0}, C_{22,1111}^{1111,1}, C_{00,3111}^{1111,0}, C_{00,3111}^{1111,1});$$

$$\begin{aligned} A &\equiv \text{Matrix4thSphericalInv}(13, 13), \\ \mathbf{x} &\equiv (C_{00,2202}^{2202,0}, C_{00,2202}^{2202,1}, C_{00,3111}^{1111,0}, C_{00,3111}^{1111,1}, C_{20,1111}^{1111,0}, C_{20,1111}^{1111,1}, C_{22,1111}^{1111,0}, C_{22,1111}^{1111,1}, C_{20,2000}^{0000,0}, C_{20,2000}^{0000,1}, C_{22,2202}^{0000,0}, C_{22,2202}^{0000,1}, C_{40,0000}^{0000,0}, C_{40,0000}^{0000,1}), \\ \mathbf{b} &\equiv (C_{00,00}^{40}, C_{00,20}^{40}, C_{00,22}^{42}, C_{11,00}^{31}, C_{11,20}^{31}, C_{11,22}^{31}, C_{11,22}^{33}, C_{20,00}^{20}, C_{20,20}^{20}, C_{20,22}^{22}, C_{22,00}^{22}, C_{22,20}^{22}, C_{22,22}^{22}), \end{aligned}$$

$$\begin{aligned} A &\equiv \text{Matrix6thSpherical}(24, 22), \\ \mathbf{x} &\equiv (C_{00,00}^{60}, C_{00,20}^{60}, C_{00,22}^{62}, C_{11,00}^{51}, C_{11,20}^{51}, C_{11,22}^{51}, C_{11,22}^{53}, C_{20,00}^{40}, C_{20,20}^{40}, C_{20,22}^{42}, C_{22,00}^{42}, C_{22,20}^{42}, C_{22,22}^{42}, C_{22,22}^{44}, C_{31,00}^{31}, C_{31,20}^{31}, C_{31,22}^{31}, C_{31,22}^{33}, C_{33,00}^{33}, C_{33,20}^{33}, C_{33,22}^{33}), \\ \mathbf{b} &\equiv (C_{60,0000}^{0000,0}, C_{60,0000}^{0000,1}, C_{40,2000}^{0000,0}, C_{40,2000}^{0000,1}, C_{42,2202}^{0000,0}, C_{42,2202}^{0000,1}, C_{00,4000}^{2000,0}, C_{00,4000}^{2000,1}, C_{20,2202}^{2202,0}, C_{20,2202}^{2202,1}, C_{22,2202}^{2202,0}, C_{22,2202}^{2202,1}, C_{40,1111}^{1111,0}, C_{40,1111}^{1111,1}, C_{42,1111}^{1111,0}, C_{42,1111}^{1111,1}, C_{20,3111}^{1111,0}, C_{20,3111}^{1111,1}, C_{22,3313}^{1111,0}, C_{22,3313}^{1111,1}, C_{00,5111}^{1111,0}, C_{00,5111}^{1111,1}, C_{00,3111}^{3111,0}, C_{00,3111}^{3111,1}), \\ \end{aligned}$$

$$\begin{aligned} A &\equiv \text{Matrix6thSphericalInv}(22, 22), \\ \mathbf{x} &\equiv (C_{00,4000}^{2000,0}, C_{00,4000}^{2000,1}, C_{00,5111}^{1111,0}, C_{00,5111}^{1111,1}, C_{20,2202}^{2202,0}, C_{20,2202}^{2202,1}, C_{20,3111}^{1111,0}, C_{20,3111}^{1111,1}, C_{22,2202}^{2202,0}, C_{22,2202}^{2202,1}, C_{22,3313}^{1111,0}, C_{22,3313}^{1111,1}, C_{40,1111}^{1111,0}, C_{40,1111}^{1111,1}, C_{40,2000}^{0000,0}, C_{40,2000}^{0000,1}, C_{42,1111}^{1111,0}, C_{42,1111}^{1111,1}, C_{42,2202}^{0000,0}, C_{42,2202}^{0000,1}, C_{60,0000}^{0000,0}, C_{60,0000}^{0000,1}), \\ \mathbf{b} &\equiv (C_{00,00}^{60}, C_{00,20}^{60}, C_{00,22}^{62}, C_{11,00}^{51}, C_{11,20}^{51}, C_{11,22}^{51}, C_{11,22}^{53}, C_{20,00}^{40}, C_{20,20}^{40}, C_{20,22}^{42}, C_{22,00}^{42}, C_{22,20}^{42}, C_{22,22}^{42}, C_{22,22}^{44}, C_{31,00}^{31}, C_{31,20}^{31}, C_{31,22}^{31}, C_{31,22}^{33}, C_{33,00}^{33}, C_{33,20}^{33}, C_{33,22}^{33}). \end{aligned}$$
